# Supplementary material for: Your Policy Regularizer is Secretly an Adversary
Source: arXiv:2203.12592 source file (2022-07-08)
Supplement: Supplementary file 1 [file 1_norm_conj.tex]

\section{Conjugate Function Derivations for KL and $\alpha$-Divergences}\label{app:conjugates}
\textcolor{red}{In this appendix, we distinguish between the conjugate function $\alphaconjn$ derived using optimization over policies $\pi(a|s) \in \simplex$ with a normalization constraint, and conjugate functions $\alphaconjmu$ with optimization over the full state-action occupancy measure $\mu(a,s)$. We treat the latter case in further detail in \myapp{perturb_pf}, and will show that these essentially differ by only an outer expectation over $\mu(s)$.}\RB{How to handle this?}

In this section, we focus on $\alphaconjn$, which specifies the optimal value function and appears in soft value aggregation or the regularized Bellman optimality operator \citep{geist2019theory}.  See \myapp{soft_value} for additional background and discussion.

We first review well-known conjugate derivations for the \textsc{kl} divergence.  In \myapp{alpha_conj_all}, we provide background on the $\alpha$-divergence, including its relation to the Tsallis entropy.   We derive the conjugate function for the $\alpha$-divergence, and will further inspect its properties in \myapp{alpha_results}.

\subsection{KL Divergence}
\label{app:kl_conj_all}
While the $\alpha$-divergence is often written over unnormalized measures, it is less common to consider an extended \kl divergence where the inputs need not be normalized \citep{zhang2004divergence}.   We consider the following definition, which occurs from the limiting behavior of \cref{eq:alpha_div_app} below as $\alpha \rightarrow 1$.% or $\alpha \rightarrow 1$.
\begin{align}
   \KL[\tpi(a|s):\tpi_0(a|s)] = \sum \limits_{a \in \mathcal{A}} \tpi(a|s) \log \frac{\tpi(a|s)}{\tpi_0(a|s)} - \sum \limits_{a \in \mathcal{A}} \tpi(a|s)  + \sum \limits_{a \in \mathcal{A}} \tpi_0(a|s) \label{eq:ukl_def_app}
\end{align}

Note that $\KL[\tpi(a|s):\tpi_0(a|s)]$ matches the standard $\KL[\pi(a|s):\pi_0(a|s)]$ for normalized inputs $\tpi, \tpi_0 \in \simplex$. 

We will find this definition useful when introducing a Lagrange multiplier to enforce the normalization constraint $\pi(a|s) \in \Delta^{|\mathcal{A}|}$ in the conjugate optimization below.   In order to evaluate this relaxation,  the regularizer $\Omega_{\pi_0}(\pi)$ should be able to take unnormalized $\tpi(a|s) \not \in \Delta^{|\mathcal{A}|}$ as input.   
\begin{align}
    \klconjpi(\dualvar) = \max \limits_{\tpi \in \fnspace_+} \blangle \tpi(a|s), \dualvar(a,s) \brangle - \klomegatpi - \lambda \left(\sum \limits_{a \in \mathcal{A}} \tpi(a|s) - 1 \right) \label{eq:conj_kl_opt_app}
\end{align} 
where $\fnspace_+$ is the space of non-negative density functions.
We can then derive the convex conjugate as follows.
\begin{proposition} (a)  The conjugate function $\klconjpi(\dualvar)$ of the \kl divergence $\klomegatpi = \frac{1}{\beta}\KL[\tpi(a|s):\tpi_0(a|s)]$, with restriction to normalized $\pi(a|s) \in \simplex$, has the closed form
\begin{align}
\klconjpi(\dualvar) = \frac{1}{\beta} \log \sum \limits_{a \in \mathcal{A}} \pi_0(a|s) \expof{ \beta \cdot \dualvar(a,s) } \label{eq:app_conj_kl}
\end{align}
(b)  The \KL divergence may then be written using the conjugate representation 
\begin{align}
   \frac{1}{\beta}\KL[\pi(a|s):\pi_0(a|s)] = \max \limits_{\dualvar \in \fnspace} \blangle \pi(a|s), \dualvar(a,s) \brangle  - \frac{1}{\beta} \log \sum \limits_{a \in \mathcal{A}} \pi_0(a|s) \expof{ \beta \cdot \dualvar(a,s) } .
\end{align}
\end{proposition}
\begin{proof}
To derive a closed form for the conjugate, consider 
\begin{align}
    \frac{1}{\beta} \Omega^{*}_{\tpi_0, \beta}(\dualvar) = \max \limits_{\tpi \in \densityfnspacea} \, \blangle \tpi(a|s), \dualvar(a,s) \brangle - \frac{1}{\beta} \left( \sum \limits_{a \in \mathcal{A}} \tpi(a|s) \log \frac{\tpi(a|s)}{\tpi_0(a|s)} - \sum \limits_{a \in \mathcal{A}} \tpi(a|s)  + \sum \limits_{a \in \mathcal{A}} \tpi_0(a|s) \right) - \lambda \left(\sum \limits_{a \in \mathcal{A}} \tpi(a|s) - 1 \right) \,. 
    \nonumber 
    % \label{eq:app_conj_kl_opt}
\end{align}
Differentiating yields a condition $\dualvar(a,s) = \nabla_{\pi} \klomegapi$ which can be inverted analytically to solve for the optimizing argument $\pi_*(a|s)$  
\begin{align}
    \dualvar(a,s) &=  \frac{1}{\beta} \left( \log \frac{\tpi(a|s)}{\tpi_0(a|s)} + {\tpi(a|s) \cdot \frac{1}{\tpi(a|s)} - 1} \right) + \lambda \nonumber \\[1.25ex]
    \implies  \, \, \piopt(a|s) &= \pi_0(a|s) \expof{ \beta \cdot \big( \dualvar(a,s) - \lambda \big) } \label{eq:optimizing_policy_kl_app}
\end{align}
Using \cref{eq:optimizing_policy_kl_app}, we can define $\psi(s;\beta) := \lambda$ as $\psi(s;\beta) = \frac{1}{\beta} \log \sum \limits_{a \in \mathcal{A}} \pi_0(a|s) \expof{ \beta \cdot \dualvar(a,s) } $.
%We can see from \cref{eq:optimizing_policy_kl_app} that 
% \begin{align}
%     \psi(s;\beta) = \frac{1}{\beta} \log \sum \limits_{a \in \mathcal{A}} \pi_0(a|s) \expof{ \beta \cdot \dualvar(a,s) } \nonumber
% \end{align}
Plugging this argument back into the conjugate optimization \cref{eq:app_conj_kl}, 
% the expectation term vanishes, with 
\tiny \begin{align}
   \klconjpi(\dualvar) = \langle \pi_0(a|s) \expof{ \beta \cdot \big( \dualvar(a,s) - \psi(s;\beta) \big) }, \dualvar(a,s) \rangle - \frac{1}{\beta} \sum \limits_{a \in \mathcal{A}} \pi_0(a|s) \expof{ \beta \cdot \big( \dualvar(a,s) - \psi(s;\beta) \big) } \cdot \log \frac{\tpi_0(a|s)}{\tpi_0(a|s)} \expof{ \beta \cdot \big( \dualvar(a,s) - \psi(s;\beta) \big) } \nonumber \, ,
\end{align}
\normalsize 
where the expectation terms vanish to leave the normalization constant $\psi(s;\beta)$ as the conjugate
% , which does not depend on $a$.   
% We finally obtain the conjugate
\begin{align}
    \klconjpi(\dualvar) = \psi(s;\beta) = \frac{1}{\beta} \log \sum \limits_{a \in \mathcal{A}} \pi_0(a|s) \expof{ \beta \cdot \dualvar(a,s) } \nonumber
\end{align}
Note that for the $\alpha$-divergence, we will have $\frac{1}{\beta} \Omega^{* (\alpha)}_{\pi_0, \beta}(\dualvar) \neq \psi_{\alpha}(s;\beta)$.  

Part (b), the conjugate expansion of the (scaled) \KL divergence in terms of its conjugate $\klconjpi$, follows from the definition in \cref{eq:conjomega}.
\end{proof}

\subsection{Reverse KL Divergence \RB{TO DO} }\label{app:kl_conj_rev}
The reverse \kl divergence, extended to unnormalized density functions as input, corresponds to the limiting behavior of the $\alpha$-divergence in \cref{eq:alpha_div_app} as $\alpha \rightarrow 0$.
\begin{align}
   \KL[\tpi_0(a|s):\tpi(a|s)] = \sum \limits_{a \in \mathcal{A}} \tpi_0(a|s) \log \frac{\tpi_0(a|s)}{\tpi(a|s)} -  \sum \limits_{a \in \mathcal{A}} \tpi_0(a|s) + \sum \limits_{a \in \mathcal{A}} \tpi(a|s)  \label{eq:urkl_def_app}
\end{align}
The convex conjugate representation of the reverse \kl divergence is as follows.
\begin{proposition} (a)  The conjugate function $\rklconjpi(\dualvar)$ of the reverse \kl divergence $\rklomegatpi = \frac{1}{\beta}\KL[\tpi_0(a|s):\tpi(a|s)]$, with restriction to normalized $\pi(a|s) \in \simplex$, has the closed form
\begin{align}
\rklconjpi(\dualvar) = \frac{1}{\beta} \blangle \pi_0(a|s), \frac{\dualvar(a,s)}{1 - \big((\dualvar(a,s) - \psi_0(s;\beta) \big) } \brangle - \frac{1}{\beta}
   \log \left[ 1- \big((\dualvar(a,s) - \psi_0(s;\beta) \big) \right] \label{eq:app_conj_rkl}
\end{align}
(b)  The reverse \kl divergence may then be written using the conjugate representation 
\footnotesize
\begin{align}
   \frac{1}{\beta}\KL[\pi_0(a|s):\pi(a|s)] = \max \limits_{\dualvar \in \fnspace} \blangle \pi(a|s), \dualvar(a,s) \brangle  - \frac{1}{\beta} \blangle \pi_0(a|s), \frac{\dualvar(a,s)}{1 - \big((\dualvar(a,s) - \psi_0(s;\beta) \big)} \brangle - \frac{1}{\beta}
   \log \left[ 1 - \big((\dualvar(a,s) - \psi_0(s;\beta) \big) \right] . \nonumber
\end{align}
\normalsize
\end{proposition}
\begin{proof}
% First, differentiating 
\end{proof}

\subsection{$\alpha$-Divergence}\label{app:alpha_conj_all}
We first recall the definition of the $\alpha$-divergence over unnormalized measures \citep{zhang2004divergence, amari2016information}.  For simplicity, we use notation $\alpha = \frac{1+\alpha\tick}{2}$ and $1-\alpha = \frac{1-\alpha\tick}{2}$ which differs from the more common use of $\alpha \tick$ in the information geometry literature
\begin{align}
 D_{\alpha}[\tpi_0(a):\tpi(a) ]& = \small \frac{1}{\alpha(1-\alpha)} \bigg( (1-\alpha)  \sum \limits_{a \in \mathcal{A}} \tpi_0(a) + \alpha  \sum \limits_{a \in \mathcal{A}} \tpi(a)  - \sum \limits_{a \in \mathcal{A}} \tpi_0(a)^{1-\alpha} \, \tpi(a)^{\alpha}  \bigg) . \label{eq:alpha_div_app}
\end{align}
When both $\sum \limits_{a \in \mathcal{A}} \tpi_0(a) = \sum \limits_{a \in \mathcal{A}} \tpi(a) = 1$, we can write the $\alpha$-divergence over normalized distributions as 
\begin{align}
    D_{\alpha}[\pi_0(a):\pi(a)]& = \frac{1}{\alpha(1-\alpha)} \bigg( 1- \sum \limits_{a \in \mathcal{A}} \pi_0(a)^{1-\alpha} \, \pi(a)^{\alpha}  \bigg) . \label{eq:alpha_norm}
\end{align}
Note that $D_{\alpha}[\pi_0: \pi] \rightarrow \KL[\pi:\pi_0]$ as $\alpha \rightarrow 1$, recovering the \kl divergence most commonly used in policy regularization.  As $\alpha \rightarrow 0$, we have $D_{\alpha}[\pi_0: \pi] \rightarrow \KL[\pi_0:\pi]$.   Due to convex duality, we have that $D_{\alpha}[\tpi_0(a) : \tpi(a)] = D_{1-\alpha}[\tpi(a) : \tpi_0(a)]$ \citep{zhang2004divergence}, which can be easily confirmed algebraically for both normalized and unnormalized arguments.   
We continue to write $D_{\alpha}[\tpi_0(a) : \tpi(a)]$ for simplicity, but emphasize that this is analogous to the case of $\KL[\pi(a):\pi_0(a)]$ as $\alpha \rightarrow 1$ despite the fact that the arguments appear to be reversed.

\subsubsection{Relation to Tsallis Entropy, $q$-exponential}\label{app:tsallis}
We analyze the $\alpha$-divergence in \cref{eq:alpha_div_app}-(\ref{eq:alpha_norm}) as a generalization of Tsallis entropy regularization \citep{lee2019tsallis}.
To show a relationship with the Tsallis entropy, we first define the $q$-exponential function $\log_q$ \citep{tsallis2009introduction}.   We define $\log_{\alpha}(u)$, with $\alpha = 2-q$, so that our use of $\log_{\alpha}(u)$ matches \citet{lee2019tsallis} Eq. (5)
\begin{align}
  \log_{q}(u) = \frac{1}{1-q} \bigg( u^{1-q} - 1\bigg) \qquad   \log_{\alpha}(u) = \frac{1}{\alpha -1} \bigg( u^{\alpha-1} - 1\bigg) = \log_{2-q}(u)
    %\log_{q}(u) = \frac{1}{q -1} \bigg( u^{q-1} - 1\bigg)
\end{align}
% Again, we use slightly non-standard notation to match \citet{lee2019tsallis}, where our $ \alpha = q = 2- q\tick$ for more standard definitions of the $q$-exponential. in terms of $q\tick$ with $1-q$ exponents.
The Tsallis entropy \citep{tsallis2009introduction, naudts2011generalised}, is defined as 
\begin{align}
    H^T_{q}[\pi(a)] = \frac{1}{q-1} \bigg( 1 -  \sum \limits_{a \in \mathcal{A}}  \pi(a)^{q} \bigg) =  \sum \limits_{a \in \mathcal{A}} \pi(a) \log_q\big( \frac{1}{\pi(a)} \big)\label{eq:tsallis1}
\end{align}
%since the latter expression contains a product of $\pi(a) \cdot \pi(a)^{-(1-q)}$. 
However, we may also express the Tsallis entropy of order $q$ in terms of $\log_{2-q}$, which is analogous to our reparameterization of $\log_{\alpha}$ using $\alpha = 2-q$ as above,  
% but $ H^T_{q}[\pi(a)] =  H^T_{\alpha}[\pi(a)]$.   
\begin{align}
     H^T_{q}[\pi(a)] = \frac{1}{q-1} \bigg( 1- \sum \limits_{a \in \mathcal{A}} \pi(a)^{q} \bigg) =   - \sum \limits_{a \in \mathcal{A}} \pi(a) \cdot \log_{2-q} \big(\pi(a) \big) \label{eq:tsallis2}
\end{align}
%since the latter expression contains a product of $\pi(a) \cdot \pi(a)^{\alpha-1}$. 
\cref{eq:tsallis1} and \cref{eq:tsallis2} mirror the two equivalent ways of writing the Shannon entropy $H_1[\pi(a)] = \sum \pi(a) \log \frac{1}{\pi(a)} =-\sum \pi(a) \log \pi(a)$, with $q=2-q$ for $q=1$.

\paragraph{$\alpha$-Divergence and Tsallis Entropy}
\RB{Change to use the constant 1 as the reference $\pi_0(a)$?}
To connect the Tsallis entropy and the $\alpha$-divergence in \cref{eq:alpha_norm}, we can consider the $\alpha$-divergence to a uniform distribution over actions $D_{\alpha}[u(a):\pi(a)]$
\begin{align}
    D_{\alpha}[u(a):\pi(a)] = \frac{1}{\alpha(1-\alpha)} \left(1 - \frac{1}{|\mathcal{A}|}^{1-\alpha} \sum \limits_{a \in \mathcal{A}} \pi(a|s)^{\alpha} \right) = \frac{-1}{\alpha}\frac{1}{|\mathcal{A}|}^{1-\alpha} H^T_{\alpha}[\pi(a)] + c
\end{align}
where $c = \frac{1}{\alpha(1-\alpha)}(1-\frac{1}{|\mathcal{A}|}^{1-\alpha})$ reverts the rescaling of the constant term.
The negative sign arises from changing an $\alpha-1$ to $1-\alpha$, or because entropies are defined to be concave and divergences are taken to be convex.  
% see that $-\frac{1}{\alpha}  H^T_{\alpha}[\pi(a)] = D_{\alpha}[u(a):\pi(a)] + c$ where $u(a)$ is the uniform distribution over actions which only affects the divergence via a constant term.  The negative sign arises from the fact that entropies are defined to be concave, while divergences are taken to be convex.   
Similarly, a Tsallis divergence \citep{naudts2011generalised} can be defined with respect to an arbitrary reference distribution $\pi_0(a)$
\begin{align}
    D^T_{\alpha}[\pi_0(a):\pi(a)] := - \bigg( - \sum \limits_{a \in \mathcal{A}} \pi(a) \cdot \log_{\alpha} \bigg(\frac{\pi(a)}{\pi_0(a)} \bigg) \bigg) = \frac{1}{1-\alpha} \bigg( 1 -  \sum \limits_{a \in \mathcal{A}} \pi_0(a)^{1-\alpha} \pi(a)^{\alpha} \bigg) \label{eq:tsallis_alpha_div}
\end{align}
where the $\alpha$-divergence $D_{\alpha}[\pi_0(a):\pi(a)]  = \frac{1}{\alpha} D^T_{\alpha}[\pi_0(a):\pi(a)]$ includes an additional $\frac{1}{\alpha}$ scaling factor compared to the Tsallis divergence.  We will see that including this constant factor by regularizing with Amari's $\alpha$-divergence allows us to avoid an inconvenient $1/\alpha$ factor in optimal policy solutions (\cref{eq:alpha_opt_policy} and \cref{eq:optimizing_policy_na_app}) compared with Eq. 8 and 10 of \citet{lee2019tsallis}, where our use of $\alpha$ is equivalent to their parameter $q$. 

% Compared with Amari's definition of the $\alpha$-divergence $D_{\alpha}[\pi_0(a):\pi(a)]$ in \cref{eq:alpha_norm}, the Tsallis divergence $D^T_{\alpha}$ is identical apart from missing the $1/\alpha$ constant.  We will see that \textit{including} this constant by regularizing with Amari's $\alpha$-divergence allows us to avoid an inconvenient $1/\alpha$ factor in optimal policy solutions (\cref{eq:optimizing_policy_ua_app} and \cref{eq:optimizing_policy_na_app}) compared with Eq. 8 and 10 of \citet{lee2019tsallis}, where our use of $\alpha$ is equivalent to their parameter $q$.
% $H^T_{\alpha}[\pi(a)]$ differs by a negative sign which simply reflects that entropies are defined to be concave while divergences are taken to be convex.  The $\alpha$-divergence includes an additional scaling constant, which above allowed us to recover the \KL divergence in either direction as special cases.   We will see that constant this allows us to avoid dividing by $1/q$ in optimal solutions to $\alpha$-divergence minimization, compared with, e.g. Eq. 8 and 10 of \citet{lee2019tsallis}.

% The Tsallis divergence to a more general base distribution $\pi_0(a) \neq u(a)$ may be defined in similar fashion using \cref{eq:alpha_norm}, along with extensions to unnormalized measures.   We continue to focus on Amari's $\alpha$-divergence, with the only difference being the additional constant factor $\frac{1}{\alpha}$.

\paragraph{$\alpha$-Divergence as an $f$-divergence}
Recall the definition of the $f$-divergence
\begin{align}
    D_{f}[\pi_0:\pi] = \sum \limits_{a \in \mathcal{A}} \pi(a|s) f \left( \frac{\pi_0(a|s)}{\pi(a|s)} \right) \, .
\end{align}
We can see that the $\alpha$-divergence, over either normalized or unnormalized densities, is an $f$-divergence with generator functions equal to 
%For the normalized case, the generator function is
\begin{align}
\begin{aligned}
    f_{\alpha}(u) = \frac{1}{\alpha(1-\alpha)} \left( u - u^{1-\alpha} \right)
\end{aligned}\hspace*{.15\textwidth}
\begin{aligned}
    f_{\alpha}(\tilde{u}) = \frac{1}{\alpha(1-\alpha)} \left( \alpha -  (1-\alpha)\tilde{u} - \tilde{u}^{1-\alpha} \right)
\end{aligned}
\end{align}
where $f_{\alpha}(\tilde{u})$ is for the divergence over unnormalized measures.

\paragraph{Pointwise Regularization}  
Just as in \cref{eq:tsallis_alpha_div}, the $\alpha$-divergence can be written using the expectation of the $\alpha$-logarithm, but including a constant $\frac{1}{\alpha}$ which vanishes for the \kl divergence at $\alpha =1$.
\begin{align}
    D_{\alpha}[\pi_0(a):\pi(a)] =  \frac{1}{\alpha} \sum \limits_{a \in \mathcal{A}} \pi(a) \cdot \log_{\alpha} \bigg(\frac{\pi(a)}{\pi_0(a)} \bigg) = \frac{1}{\alpha (1-\alpha)} \bigg( 1 -  \sum \limits_{a \in \mathcal{A}} \pi_0(a)^{1-\alpha} \pi(a)^{\alpha} \bigg)
\end{align}
where we have assumed that $\sum_a \pi(a) = 1$.   This way of writing highlights the connection between the $\alpha$-divergence and $\alpha$- or $q$-logarithm.

\subsubsection{Convex Conjugate of $\alpha$-Divergence (with Restriction to Normalized Policies)}\label{app:alpha_conj_norm}
As in \cref{app:kl_conj_all}, we consider the conjugate optimization with a Lagrange multiplier $\lambda$ enforcing normalization of the policy
\begin{align}
    \alphaconjn(\dualvar) = \max \limits_{\tpi \in \fnspace_+} \blangle \tpi(a|s), \dualvar(a,s) \brangle - \omegatpi - \lambda \left(\sum \limits_{a \in \mathcal{A}} \tpi(a|s) - 1 \right)  \, . \label{eq:conj_alpha_opt_app} 
\end{align}
\begin{proposition} \label{prop:alpha_conj_app}
(a) 
% With $\alphan = D_{\alpha}[\pi_0(a|s):\pi(a|s)]$, the conjugate function has the closed form
% The conjugate function of 
The conjugate function $\alphaconjn(\dualvar)$ of the $\alpha$-divergence $\omegatpi = D_{\alpha}[\tpi_0(a|s): \tpi(a|s)]$ in \cref{eq:alpha_div_app}, with restriction to normalized $\pi(a|s) \in \simplex$, has the closed form
% {$\alphaconjn(\dualvar) = \max \limits_{\pi \in \simplex} \langle \pi, \dualvar \rangle - \alphan$} 
\begin{align}
 \alphaconjn(\dualvar) &=    \frac{\alpha-1}{\alpha} \bigg \langle \pi_0(a|s) \big[ 1+ \beta (\alpha-1) \cdot \big(\dualvar(a,s) - \psi_{\alpha}(s;\beta)\big)  \big]^{\frac{1}{\alpha-1}}, \, \dualvar(a,s) \bigg \rangle  + \frac{1}{\alpha}  \psi_{\alpha}(s;\beta)   \label{eq:app_conj_norm} %- \frac{1}{\beta} \frac{1}{\alpha(1-\alpha)}
 \end{align}
(b)  The $\alpha$-divergence may then be written using the conjugate representation 
\small 
\begin{align}
   \frac{1}{\beta}D_{\alpha}[\pi_0:\pi] &= \max \limits_{\dualvar \in \fnspace} \, \blangle \pi(a|s), \dualvar(a,s) \brangle  - \frac{\alpha-1}{\alpha} \blangle \pi_0(a|s) \big[ 1+  \beta (\alpha-1) \cdot \big(\dualvar(a,s) - \psi_{\alpha}(s;\beta)\big)  \big]^{\frac{1}{\alpha-1}}, \, \dualvar(a,s) \brangle -  \frac{1}{\alpha}  \psi_{\alpha}(s;\beta) \nonumber %\\
   %& \phantom{===}-  \frac{1}{\alpha}  \psi_{\alpha}(s;\beta)   %+ \frac{1}{\beta} \frac{1}{\alpha(1-\alpha)}
\end{align}
\normalsize
\end{proposition}
\textcolor{red}{Include Lagrange multiplier for $\pi(a|s) \geq 0$}
\begin{proof}
Considering the conjugate optimization with normalization constraint,
\begin{align}
    \alphaconjn(\dualvar) = \max \limits_{\pi \in \simplex} \, \blangle \pi(a|s), \dualvar(a,s) \brangle - \frac{1}{\beta} D_{\alpha}[\tpi_0(a|s):\tpi(a|s)] + \lambda \big( \sum \limits_{a \in \mathcal{A}} \pi(a|s) -1 \big) \label{eq:app_conj_ukl_opt}
\end{align}
Differentiating yields a condition $\dualvar(a,s) = \frac{1}{\beta}\nabla_{\tpi} D_{\alpha}[\tpi_0(a|s):\tpi(a|s) ]$, %$\dualvar(a,s) = \nabla_{\tpi} \frac{1}{\beta} D_{\alpha}[\tpi(a|s):\tpi_0(a|s)]$, but unlike the case of the \KL divergence, this expression can not be easily inverted to solve for $\pi(a|s)$
%which can be inverted analytically to solve for the optimizing argument $\tpi_*(a|s)$  
\begin{align}
    \dualvar(a,s) &= \nabla_{\pi} \frac{1}{\beta} \frac{1}{\alpha(1-\alpha)} \bigg(   \sum \limits_{a \in \mathcal{A}} (1-\alpha) \, \pi_0(a|s) + \alpha \, \pi(a|s) - \pi_0(a|s)^{1-\alpha} \, \pi(a|s)^{\alpha}  \bigg) \\
    &= \frac{1}{\beta}\frac{1}{1-\alpha} - \frac{1}{\beta}\frac{1}{1-\alpha}  \pi_0(a|s)^{1-\alpha} \, \pi(a|s)^{\alpha-1}   + \lambda \, .\nonumber %\\[1.25ex]
\end{align}
Inverting this expression to solve for the optimizing argument $\pi_*(a|s)$, 
\begin{align}
 \piopt(a|s) = \pi_0(a|s) \big[1 + \beta (\alpha-1) \cdot \big( \dualvar(a,s) - \normalizeralpha \big)  \big]^{\frac{1}{\alpha-1}} \label{eq:optimizing_policy_na_app}
\end{align}
where $\normalizeralpha = \lambda$ enforces normalization.   Plugging this argument back into \cref{eq:app_conj_ukl_opt}, we can again rewrite $\sum_a \pi_0(a)^{1-\alpha} \pi(a)^\alpha = \sum_a \pi(a) \frac{\pi(a)}{\pi_0(a)}^{\alpha-1}$,  allowing for cancellation of the exponent in \cref{eq:optimizing_policy_na_app}
%\scriptsize
\small
\begin{align}
    \alphaconjn(\dualvar)  &= \bigg \langle  \pi_0(a|s) \big[  1+ \beta (\alpha-1) \cdot \big(\dualvar(a,s) - \psi_{\alpha}(s;\beta)\big)  \big]^{\frac{1}{\alpha-1}}, \, \dualvar(a,s) \bigg \rangle - \frac{1}{\beta} \frac{1}{\alpha(1-\alpha)} \\
    &\phantom{====} + \frac{1}{\beta} \frac{1}{\alpha(1-\alpha)}  \sum \limits_{a \in \mathcal{A}} \pi_0(a|s) \big[  1+\beta (\alpha-1) \cdot \big(\dualvar(a,s) - \psi_{\alpha}(s;\beta)\big) \big]^{\frac{1}{\alpha-1}}\cdot 1 \nonumber \\
    &\phantom{====}  + \frac{1}{\beta} \frac{1}{\alpha(1-\alpha)} \sum \limits_{a \in \mathcal{A}}  \pi_0(a|s) \big[  1+\beta (\alpha-1) \cdot \big(\dualvar(a,s) - \psi_{\alpha}(s;\beta)\big) \big]^{\frac{1}{\alpha-1}} \cdot  \beta (\alpha -1) \cdot \big(\dualvar(a,s) - \psi_{\alpha}(s;\beta)\big) \nonumber % \\[1.25ex]
    % & \phantom{==} + \bigg( \frac{1}{\beta} \frac{1}{\alpha(1-\alpha)} - \frac{1}{\beta} \frac{1}{1-\alpha} \bigg) \sum \limits_{a \in \mathcal{A}}  \tpi_0(a|s) \big[ 1 +  \beta (\alpha-1) \cdot \dualvar(a,s)  \big]^{\frac{1}{\alpha-1}} \nonumber 
\end{align}
\normalsize
Noting that $\sum \limits_{a \in \mathcal{A}} \pi_0(a|s) \big[  1+\beta (\alpha-1) \cdot \big(\dualvar(a,s) - \psi_{\alpha}(s;\beta)\big) \big]^{\frac{1}{\alpha-1}}$ is normalized and that we have a change in sign in the third line due to $(\alpha-1)/(1-\alpha)$, the above simplifies to a closed form for the conjugate $\alphaconjn$ 
% in terms of $\dualvar$
\begin{align} 
 \alphaconjn(\dualvar) &=     \frac{\alpha-1}{\alpha}  \bigg \langle \pi_0(a|s) \big[  \beta (\alpha-1) \cdot \big(\dualvar(a,s) - \psi_{\alpha}(s;\beta)\big)  \big]^{\frac{1}{\alpha-1}}, \, \dualvar(a,s) \bigg \rangle   +  \frac{1}{\alpha}  \psi_{\alpha}(s;\beta) 
 %- \frac{1}{\beta} \frac{1}{\alpha(1-\alpha)} \nonumber
\end{align}
%as desired.   
The conjugate representation of $D_{\alpha}[\pi_0(a|s):\pi(a|s)]$ then follows by definition. 
\end{proof}
