# Supplementary material for: Your Policy Regularizer is Secretly an Adversary
Source: arXiv:2203.12592 source file (2022-07-08)
Supplement: Supplementary file 2 [file 3_perturb_pf.tex]

\section{Worst-Case Reward Perturbations}\label{app:perturb_pf}
In this section, we derive the worst-case reward perturbations for the adversary associated with a particular policy (\cref{eq:pedro_form}, \myprop{optimal_perturbations}) and show that they preserve the value of the regularized objective in \cref{app:preserve}.  In contrast to \mysec{conj_examples} and \myapp{conjugates}, we consider the conjugate $\alphaconjmu$ with optimization over the full state-action occupancy measure $\mu(a,s)$.   
However, when analyzing the optimal policy $\piopt(a|s)$ in \myapp{advantage_pf}, we will find that this approach sheds insight into the relationship between $V_*(s)$ and $\normalizeralpha$, which both appear in the conjugate with optimization over $\pi(a|s)$ in 
\cref{eq:alpha_conj_norm_main} and \myprop{alpha_conj_app}.

% For now, see \myapp{joint_derivation} 
\subsection{Derivation of Worst-Case Reward Perturbations (Proof of \myprop{optimal_perturbations})}\label{app:perturb_pf_sub} 
\textcolor{red}{Compared with the main text, note that we include a Lagrange multiplier $\lambdazero$ enforcing $\mu(a,s) \geq 0$.   For $\mu(a,s)>0$ or $\pi(a|s)>0$, we have $\lambdazero= 0$ by complementary slackness \citep{boyd2004convex}. }
\optimalperturbations*
\begin{proof}
Recall from the conjugacy conditions in \mysec{conj_intro} that $\propt(a,s) = \nabla \omegamu = (\nabla \alphaconjmu)^{-1}(\mu)$.   We will derive the optimal reward perturbations via the first equality  $\propt(a,s) = \nabla \omegamu$ for convenience, since we will see that the conjugate $\alphaconjmu$ can be difficult to manipulate directly.  

We consider the conjugate optimization over $\mu(a,s)$, and include a Lagrange multiplier $\lambdazero$ to enforce $\mu(a,s) \geq 0$. We justify ignoring normalization constraints below, and write the optimization as
% Expressing the conjugate function
% \begin{align}
\begin{align}
    \alphaconjmu(\pr) &= \max \limits_{\mu(a,s)} \blangle \mu(a,s), \pr(a,s) \brangle - \alphanmu - \lambdazero \label{eq:mu_as_conj}
\end{align}
% where we do not include a normalization constraint since, for the optimal value function $V_*(s)$, the Bellman flow constraints imply 
where we treat the conditional regularization $\alphanmu= \mathbb{E}_{\mu(s)}\big[ D_{\alpha}[\pi_0(a|s): \frac{\mu(a,s)}{\mu(s)}] \big]$ as a function of the full state-action occupancy measure $\mu(a,s)$, with $\pi(a|s) = \mu(a,s) / \mu(s)$ and
\begin{align}
    \alphanmu 
    % &= \mathbb{E}_{\mu(s)}\big[ D_{\alpha}[\pi_0(a|s): \underbrace{\frac{\mu(a,s)}{\mu(s)}}_{\pi(a|s)}] \big] \nonumber \\
     &= \frac{1}{\beta}\frac{1}{\alpha (1-\alpha)} \left( (1-\alpha) \sum \limits_{a,s} \mu(s) \pi_0(a|s) + \alpha \sum \limits_{a,s} \mu(a,s) - \sum \limits_{a,s} \mu(s) \pi_0(a|s)^{1-\alpha} \left(\frac{\mu(a,s)}{\mu(s)}\right)^{\alpha} \right) \label{eq:joint_div}
    % &= \frac{1}{\beta}\frac{1}{\alpha (1-\alpha)} \left( 1 - \sum \limits_{a,s} \mu(s) \pi_0(a|s)^{1-\alpha} \left(\frac{\mu(a,s)}{\mu(s)}\right)^{\alpha} \right) \label{eq:joint_div}
\end{align}
% \end{align}
% \begin{align}
% \alphaconjn(\pr) &= \max \limits_{\mu(a,s)} \blangle \mu(a,s), \pr(a,s) \brangle - \alphanmu ,
% \end{align}
After rearranging the exponents in the second term of  \cref{eq:joint_div},
we can solve for the optimal $\mu(a,s)$ by differentiating \cref{eq:joint_div} with respect to $\mu$.  
We explicitly denote the arguments of differentiation and summation to highlight the care needed to differentiating the marginal $\mu(s\tick)$ with respect to $\mu(a,s)$, with $\sum_{s\tick} \frac{d}{d\mu(a,s)}\mu(s\tick) = \sum_{s\tick, a\tick} \frac{d}{d\mu(a,s)} \mu(a\tick, s\tick) = \sum_{s\tick, a\tick} \delta(a\tick,s\tick = a,s) = 1$.  See \citet{neu2017unified}, \citet{lee2019tsallis} for similar derivations.
% using the condition $\propt(a,s) &= \nabla_{\mu} \alphanmu$, with
\begin{align}
\pr&(a,s) = \nabla_{\mu} \alphanmu  - \lambdazero \label{eq:pr_equals_grad} \\
% &= \frac{1}{\beta}\frac{1}{\alpha(1-\alpha)} \sum \limits_{a\tick,s\tick}  \frac{d}{d\mu(a,s)} \mu(s\tick)^{1-\alpha} \pi_0(a\tick|s\tick)^{1-\alpha} \mu(a\tick,s\tick)^{\alpha} \\
&= \frac{1}{\beta}\frac{1}{\alpha(1-\alpha)}  \sum \limits_{a\tick,s\tick}  \frac{d}{d\mu(a,s)} \bigg( (1-\alpha) \mu(s\tick)\pi_0(a\tick|s\tick) + \alpha \mu(a\tick, s\tick) - \mu(s\tick)^{1-\alpha} \pi_0(a\tick|s\tick)^{1-\alpha} \mu(a\tick,s\tick)^{\alpha} \bigg)  - \lambdazero \nonumber \\
&=  - \lambdazero + \frac{1}{\beta}\frac{1}{\alpha(1-\alpha)} \bigg( 
(1-\alpha) \sum \limits_{s\tick} \underbrace{\frac{d \sum_{a\tick} \mu(a\tick, s\tick)}{d\mu(a,s)}}_{\delta(s = s\tick)} \sum \limits_{a\tick} \pi_0(a\tick|s)  + \alpha 
\sum \limits_{a\tick,s\tick} \underbrace{\frac{d\mu(a\tick,s\tick)}{d\mu(a,s)}}_{\delta(a\tick,s\tick = a,s)}  - 
 \\ %phantom{= \frac{1}{\beta}\frac{1}{(1-\alpha)} \bigg(}
&\phantom{==} -\sum \limits_{a\tick,s\tick}  \alpha \mu(a\tick,s\tick)^{\alpha-1} \underbrace{\frac{d\mu(a\tick,s\tick)}{d\mu(a,s)}}_{\delta(a\tick,s\tick = a,s)} \mu(s\tick)^{1-\alpha} \pi_0(a\tick|s\tick)^{1-\alpha}- (1-\alpha) \sum \limits_{a\tick,s\tick} \mu(s\tick)^{-\alpha} \underbrace{\frac{d \sum_{a\tick} \mu(a\tick, s\tick)}{d\mu(a,s)}}_{\delta(s = s\tick)} \cdot \pi_0(a\tick|s\tick)^{1-\alpha} \mu(a\tick,s\tick)^{\alpha} \bigg) \nonumber \\
&= \frac{1}{\beta}\frac{1}{\alpha(1-\alpha)} \bigg( (1-\alpha) \textcolor{red}{\sum_{a} \pi_0(a|s)} + \alpha - \alpha \left(\frac{\mu(a,s)}{\mu(s) \pi_0(a|s)} \right)^{\alpha-1} - (1-\alpha) \sum \limits_{a\tick}   \pi_0(a|s)^{1-\alpha}\left(\frac{\mu(a,s)}{\mu(s)} \right)^{\alpha}  \bigg)  - \lambdazero \nonumber
\end{align}
% where 

Finally, with this optimality condition, we substitute $\pi_*(a|s) = \frac{\mu(a,s)}{\mu(s)}$ to obtain
\begin{align}
   \pr(a,s) = 
\textcolor{red}{\frac{1}{\beta}\frac{1}{\alpha} \sum_{a} \pi_0(a|s) + \frac{1}{\beta}\frac{1}{1-\alpha}}
%   \frac{1}{\beta}\frac{1}{\alpha (1-\alpha)}
   - \frac{1}{\beta}\frac{1}{1-\alpha} \left(\frac{\pi_*(a|s)}{\pi_0(a|s)} \right)^{\alpha-1} - \frac{1}{\beta}\frac{1}{\alpha} \sum \limits_{a} \pi_0(a|s)^{1-\alpha} \pi_*(a|s)^{\alpha}  - \lambdazero\label{eq:propt_intermediate}
\end{align}
\sout{Using $\frac{1}{\beta}\frac{1}{\alpha(1-\alpha)} = -\frac{1}{\beta}\frac{1}{\alpha(\alpha-1)} = \frac{1}{\beta}\frac{1}{(\alpha-1)} - \frac{1}{\beta}\frac{1}{\alpha}$, we split the constant into two terms, which allows us to recognize a $\log_{\alpha}\frac{\pi(a|s)}{\pi_0(a|s)}$ term and $-\myconst$ term in \cref{eq:propt_intermediate} for $\sum \limits_{a} \pi_0(a|s) = 1$. }
 We first notice that \cref{eq:propt_intermediate} contains terms which combine to yield $\frac{1}{\beta} \log_{\alpha}\frac{\pi(a|s)}{\pi_0(a|s)}$.   Further, if we assume that $\sum \limits_{a} \pi_0(a|s) = 1$ and notice that $\sum \limits_{a} \pi(a|s) = \sum \limits_{a} \frac{\mu(a,s)}{\sum \limits_a \mu(a,s)} = 1$, then we can also recognize a term of $-\myconst$ term,
\begin{align}
   \pr(a,s) = \frac{1}{\beta}\underbrace{ \frac{1}{\alpha-1}  \bigg( \left(\frac{\pi(a|s)}{\pi_0(a|s)} \right)^{\alpha-1} - 1 }_{\log_{\alpha}\frac{\pi(a|s)}{\pi_0(a|s)}}\bigg) -  \frac{1}{\beta}\bigg( \underbrace{\frac{1}{\alpha}  \sum \limits_{a} \pi_0(a|s)^{1-\alpha} \pi(a|s)^{\alpha} - \frac{1}{\alpha}\sum \limits_{a} \pi_0(a|s)}_{-\myconst} \bigg)  - \lambdazero \, .\label{eq:worst_case_reward_perturba}
\end{align}
As desired, we obtain
\begin{align}
    \pr(a,s) = \frac{1}{\beta}\log_{\alpha}\frac{\pi(a|s)}{\pi_0(a|s)} + \frac{1}{\beta} \myconst  - \lambdazero\, . \label{eq:worst_case_reward_perturb}
\end{align}
By complementary slackness, we know that $\lambdazero=0$ when $\mu(a,s) > 0$, so that the perturbations are not affected for state-action pairs with non-zero probability.   In subsequent derivations, we will frequently consider expectations of the form $\langle \pi(a|s), \propt(a,s) \rangle$.   Note that we can ignore the contribution of $\lambdazero$ in these expressions, since either $\lambdazero = 0$ or $\mu(a,s) = 0$ and $\pi(a|s) = 0$.
% where the negative sign in $-\myconst$ 
\end{proof}

\subsubsection{Conjugate Function using $\mu(a,s)$ Optimization}\label{app:conjugate_mu}
We can use the above derivations to obtain the conjugate function $\alphaconjmu$, which treats the $\alpha$-divergence as a function of $\mu(a,s)$.   This proposition will allow us to show that the conjugate preserves the value of the objective in \myapp{preserve}.  
% and derive the feasible set of adversarial perturbations in \myapp{feasible_pf}.

\begin{restatable}[\textbf{Conjugate Function using $\mu(a,s)$ Optimization}]{proposition}{conjugatemu}\label{prop:conjugate_mu}
The conjugate $\alphaconjmu(\dualvar)$ of the $\alpha$-divergence $\omegamu = \mathbb{E}_{\mu(s)}\big[ D_{\alpha}[\pi_0(a|s): \pi(a|s)] \big]$ in \cref{eq:alpha_div_app} as a function of $\mu(a,s)$, can be written 
\begin{align}
    \hspace*{-.2cm} \alphaconjmu(\pr) = \frac{\alpha-1}{\alpha} \blangle \mur(s) \pir(a|s), \pr(a,s) \brangle + \frac{1}{\alpha} \normalizerpr \label{eq:conj_alpha_mu_app}
    % - \frac{\alpha-1}{\alpha}\blangle \mur(s), D_{\alpha}[\pi_0:\pir] \brangle= \frac{\alpha-1}{\alpha} \mathbb{E}_{\mu(s)}\bigg[ \alphaconjn(\pr)\bigg] \nonumber
\end{align}
\RB{RESTATE / CLARIFY}
where $\pir(a|s)=\frac{\mur(a,s)}{\mur(s)}$, which is a function of $\pr(a,s)$, is the policy derived from the state-action occupancy measure that corresponds to $\pr$ via the conjugacy conditions
$\mur(a,s) = \nabla \alphaconjmu(\dualvar) = (\nabla \Omega^{(\alpha)}_{\pi_0, \mu})^{-1}(\dualvar)$
\begin{align}
    \pir(a|s) = \pi_0(a|s) \big[ 1 +  \beta (\alpha-1) \cdot \big( \pr(a,s) -\normalizerpr \big) \big]_+^{\frac{1}{\alpha-1}} \label{eq:policy_for_perturbed}
    % \pir(a|s) = \pi_0(a|s) \bigg[ 1 +  \beta (\alpha-1) \cdot \big( \pr(a,s) - \frac{1}{\beta}\mydiv{\pir} \big) \bigg] \label{eq:policy_for_perturbed}
\end{align}
\end{restatable}
\begin{proof}
Starting from \cref{eq:worst_case_reward_perturba}, we can solve for $\pir(a|s)$ in self-consistent fashion, since $\mydiv{\pir}$ depends on $\pir(a|s)$, to obtain \eqref{eq:policy_for_perturbed}.   Note that we substitute $\normalizerpr = \frac{1}{\beta}(1-\alpha)D_{\alpha}[\pi_0:\pir]$ in order to emphasize that $\normalizerpr$ should be treated as a constant and solved for numerically, thus avoiding recursive substitution of $\pir$ terms.  

\textcolor{red}{This notation also highlights the role of $\normalizerpr = \frac{1}{\beta}(1-\alpha)D_{\alpha}[\pi_0:\pir]$ as a normalization constant that is different than $\normalizeralpha$ (which normalizes the policy for the conjugate $\alphaconjn(Q)$ with $Q$-values as inputs, as in \mysec{conj_examples} and \myapp{conjugates}).   } \RB{REDO THIS... TOTALLY UNCLEAR}
% \begin{align}
%     \pi_*(a|s) = \pi_0(a|s) \bigg[1 + \beta (\alpha-1) \cdot \big( \pr(a,s) - \frac{1}{\beta} \myconst  \big) \bigg]_+^{\frac{1}{\alpha-1}} \label{eq:opt_pi_joint_alpha}
% \end{align}
If $\mur(a,s)$ is normalized, note that $\pir(a|s)= \mur(a,s) / \sum_a \mur(a,s)$ is normalized by construction \textcolor{red}{(see proof that $\mu \in \mathcal{M}$ is normalized)}.  When plotting the feasible sets in \myapp{feasible}, we confirm that \cref{eq:policy_for_perturbed} is normalized for the single-step setting, with $\normalizerpr$ matching $\frac{1}{\beta}(1-\alpha)D_{\alpha}[\pi_0:\pir]$ and the normalization constant of \cref{eq:policy_for_perturbed} obtained by numerical optimization.

Plugging this optimizing argument $\pir(a|s)$ back into \cref{eq:mu_as_conj}, we obtain an expression for the conjugate $\alphaconjmu$, which matches the form of the conjugate $\alphaconjn$ with optimization over $\pi(a|s)\in \simplex$ in \cref{eq:alpha_conj_norm_main} and \cref{eq:app_conj_norm}.
\begin{align}
\alphaconjmu(\pr) &= \blangle \mur(s) \pir(a|s), \pr(a,s) \brangle - \frac{1}{\beta}\frac{1}{\alpha(1-\alpha)} +\frac{1}{\beta}\frac{1}{\alpha(1-\alpha)} \blangle \pir(a|s),  \left( \frac{\pir(a|s)}{\pi_0(a|s)}\right)^{\alpha-1} \brangle \\
&=\blangle \mur(s) \pir(a|s), \pr(a,s) \brangle - \frac{1}{\beta}\frac{1}{\alpha(1-\alpha)} +\frac{1}{\beta}\frac{1}{\alpha(1-\alpha)} \blangle \pir(a|s), 1\brangle \\
&\phantom{====} +  \frac{1}{\alpha} \frac{\beta}{\beta}\frac{(\alpha-1)}{(1-\alpha)}  \blangle \pir(a|s), \pr(a,s) \brangle - \frac{1}{\alpha} \frac{\beta}{\beta}\frac{(\alpha-1)}{(1-\alpha)} \normalizerpr \nonumber \\
&= \frac{\alpha-1}{\alpha} \blangle \mur(s) \pir(a|s), \pr(a,s) \brangle + \frac{1}{\alpha} \normalizerpr
\end{align}
\end{proof}

\subsection{Worst-Case Reward Perturbations Preserve Value of the Objective}\label{app:preserve}
We now confirm that the conjugate optimization matches the value of the regularization function $\omegamu = \max_{\pr} \langle \mu(a,s), \pr(a,s) \rangle - \alphaconjmu(\pr)$ when evaluated with the worst-case reward perturbations $\propt(a,s)$, as we would expect from the definition in \cref{eq:conjomega}. 

We first show that $\alphaconjmu(\propt)=0 \, \forall \alpha$ in the following proposition, which will also be useful in deriving the feasible set in \myapp{feasible}.    %we then use to confirm the conjugate identity.    This proposition
% Solving \cref{eq:worst_case_reward_perturba} for the policy $\pir(a|s)$ instead, we obtain
% \begin{align}
%     \pir(a|s) = \pi_0(a|s) \bigg[ 1 +  \beta (\alpha-1) \cdot \big( \pr(a,s) - \frac{1}{\beta}\mydiv{\pir} \big) \bigg]_+^{\frac{1}{\alpha-1}} \label{eq:policy_for_perturbed}
% \end{align}
\begin{restatable}{proposition}{conjugatezero} \label{prop:conjugatezero}
For the worst-case reward perturbation $\propt(a,s)$ associated with a given policy $\pi(a|s)$ or occupancy measure $\mu(a,s)$, evaluating the conjugate function, for any $\alpha$, yields
\begin{align}
  \alphaconjmu = 0
\end{align}
\end{restatable}
\begin{proof}
Treating the conjugate function $\alphaconjmu(\pr)$ as a function of $\pr$, we substitute the worst-case reward perturbations $\propt(a,s)$ from \myprop{optimal_perturbations} and \cref{eq:optimal_perturbations}.  Note that $\propt(a,s)$ is a function of the original $\pi(a|s)$.  We would like to show that $\omegamu = \langle \mu(s)\pir(a|s), \propt(a,s) \rangle - \alphaconjmu(\propt)$.

First, we can simplify the expression for $\pir(a,s)$ in \cref{eq:policy_for_perturbed}, using 
\begin{align*}
    \pir(a|s) &= \pi_0(a|s) \big[ 1 +  \beta (\alpha-1) \cdot \big( \pr(a,s) -\normalizerpr \big) \big]_+^{\frac{1}{\alpha-1}} \nonumber \\
    &= \pi_0(a|s) \big[ 1 +  \beta (\alpha-1) \cdot \big( \frac{1}{\beta}\frac{1}{\alpha-1}\big( \frac{\pi(a|s)}{\pi_0(a|s)} \big)^{\alpha-1} - \frac{1}{\beta}\frac{1}{\alpha-1} + \frac{1}{\beta}(1-\alpha) D_{\alpha}[\pi_0:\pi] - \underbrace{\frac{1}{\beta}(1-\alpha) D_{\alpha}[\pi_0:\pi]}_{\normalizerpr} \big) \big]_+^{\frac{1}{\alpha-1}} \nonumber \\
    &= \pi(a|s) \nonumber
\end{align*}
which is to be expected since $\pi(a|s)$ (or $\pir(a|s)$) and $\propt(a|s)$ are in dual correspondence.
Plugging this into \myprop{conjugate_mu} \cref{eq:conj_alpha_mu_app},
\begin{align*}
    \hspace*{-.2cm} \alphaconjmu(\pr) &= \frac{\alpha-1}{\alpha} \blangle \mu(s) \pi(a|s), \pr(a,s) \brangle + \frac{1}{\alpha} \normalizerpr \\
    &= \frac{\alpha-1}{\alpha} \blangle \mu(s) \pi(a|s), \frac{1}{\beta}\frac{1}{\alpha-1} \frac{\pi(a|s)}{\pi_0(a|s)}^{\alpha-1} - \frac{1}{\beta}\frac{1}{\alpha-1}\brangle  +  \frac{\alpha-1}{\alpha}\frac{1}{\beta}(1-\alpha)D_{\alpha}[\pi_0:\pi] + \frac{1}{\alpha} \normalizerpr \nonumber \\
    &\overset{(1)}{=}  -\frac{1}{\beta}(1-\alpha)D_{\alpha}[\pi_0:\pi] +  \left( \frac{\alpha-1}{\alpha} +\frac{1}{\alpha} \right) \frac{1}{\beta}(1-\alpha)D_{\alpha}[\pi_0:\pi]  \\
    &= 0
\end{align*}
where, in $(1)$, we have used $\normalizerpr:=\frac{1}{\beta}(1-\alpha)D_{\alpha}[\pi_0:\pi]$ and noted that a negative sign is necessary to obtain $(1-\alpha) D_{\alpha}[\pi_0:\pi] = \frac{1}{\alpha}(1 - \sum \pi_0(a|s)^{1-\alpha}\pi(a|s)^{\alpha}$ in the first term. 
\end{proof}

\begin{restatable}{corollary}{preserves}\label{cor:preserves}
For the worst-case reward perturbations $\propt(a,s)$ associated with a given policy $\pi(a|s)$, the conjugate expansion does not change the value of the objective function in \cref{eq:dual_lagrangian}.  In other words, we confirm
\begin{align}
    \omegamu  = \langle \pi(a|s), \propt(a,s) \rangle - \alphaconjmu(\propt) \, .
\end{align}
\end{restatable}
\begin{proof}
We have shown in \myprop{conjugatezero} that $\alphaconjmu(\propt) = 0$.   Substituting the reward perturbations $\propt(a,s)$, we can follow similar derivations to confirm
\begin{align*}
     \omegamu  &= \langle \mu(s) \pi(a|s), \propt(a,s) \rangle - \langle \mu(s), \alphaconjmu(\propt) \rangle \\
     &= \blangle \mu(s) \pi(a|s), \frac{1}{\beta}\frac{1}{\alpha-1} \frac{\pi(a|s)}{\pi_0(a|s)}^{\alpha-1} - \frac{1}{\beta}\frac{1}{\alpha-1}\brangle  +  \blangle \mu(s), \frac{1}{\beta}(1-\alpha)D_{\alpha}[\pi_0:\pi] \brangle - 0 \\
     &= \blangle \mu(s), \frac{1}{\beta}\,\alpha\, D_{\alpha}[\pi_0:\pi] \brangle + \blangle \mu(s), \frac{1}{\beta}(1-\alpha)D_{\alpha}[\pi_0:\pi] \brangle \\
     &=  \blangle \mu(s), \frac{1}{\beta} D_{\alpha}[\pi_0:\pi] \brangle = \omegamu \, .
\end{align*} 
\end{proof}

\subsection{Relationship with Advantage Function (Proof of \myprop{advantage})}\label{app:advantage_pf}
We now prove the relationship between the worst-case reward perturbations and the advantage function.   Our derivations assume optimal values, with $Q_*(a,s) = r(a,s) + \gamma \transitionvstar$ and $V_*(s) = \max \limits_{\pi \in \simplex} \langle \pi(a|s), Q(a,s) \blangle - \omegamu$.   We prove the following proposition from \mysec{optimal_policy}.
\advantage*
\begin{proof}
We begin by considering the Lagrangian dual of the regularized objective in \cref{eq:dual_lagrangian}
\begin{align}
   \max \limits_{\mu(a,s)} \min \limits_{V(s)} & \, (1-\gamma) \big\langle \nu_0(s), V(s) \big  \rangle  
     + \blangle \mu(a,s), r(a,s) +  \gamma \transitionv -V(s)\brangle - \omegamu \, . \nonumber
     % \label{eq:dual_lagrangian}
\end{align}{}
Eliminating $\mu(a,s)$ by setting $\frac{d}{d\mu}=0$, we can reuse our derivations in \cref{eq:pr_equals_grad}-(\ref{eq:propt_intermediate}) to show that 
\begin{align}
     r(a,s) +  &\gamma \transitionv -V(s) - \nabla \omegamu = 0 \label{eq:kkt} \\
     r(a,s) +  & \gamma \transitionv -V(s) - \frac{1}{\beta} \frac{1}{\alpha-1} \big( \frac{\pi(a|s)}{\pi_0(a|s)}^{\alpha-1} - 1 \big) - \frac{1}{\beta}(1-\alpha) D_{\alpha}[\pi_0:\pi] = 0 \\
     \implies \pi(a|s) &= \pi_0(a|s) [ 1 + \beta (\alpha-1) ( r(a,s) +  \gamma \transitionv -V(s) - \frac{1}{\beta}(1-\alpha) D_{\alpha}[\pi_0:\pi]) ]_+^{\frac{1}{\alpha-1}} \label{eq:opt_alpha_pol_app}
     % \implies \mu(a,s)
\end{align}
Recall that the optimal Lagrange multipliers $V_*(s)$ enforce the Bellman flow constraints in \cref{eq:dual_lagrangian} which, for normalized $\nu_0(s) \in \Delta^{|\mathcal{S}|}$, implies that $\mu(a,s) \in \Delta^{|\mathcal{S}| \times |\mathcal{A}|}$ and thus $\pi(a|s) \in \Delta^{|\mathcal{A}|}$ are normalized.  
Plugging in the optimal $V_*(s)$ and $Q_*(a,s) = r(a,s) + \gamma \transitionvstar$, we can thus consider the second two terms to be the normalization constant for the optimal policy $\piopt(a|s)$.    As in \mysec{conj_examples} and \myapp{conjugates}, we denote this normalizer as $\normalizeralpha$, with 
\begin{align}
\normalizeralpha =  V_*(s) + \frac{1}{\beta}(1-\alpha) D_{\alpha}[\pi_0:\piopt] \, . \label{eq:psidentity_app}
\end{align}
See \citet{lee2019tsallis} App. D2 for similar reasoning.   Note that $\normalizeralpha$ also corresponds to the normalization constant for the optimal policy in the conjugate optimization $\alphaconjn(Q) = \max_{\pi \in \simplex} \langle \pi, Q \rangle - \omegapi$.   
\textcolor{red}{Further, note that \cref{eq:psidentity_app} is a self-consistent equation since all three terms interact via the policy $\piopt(a|s)$.
}

While we found this identity useful in our simplified exposition in \mysec{optimal_policy}, it is not strictly necessary in the below proof.   
 % it is not directly necessary in what follows.
Substituting the optimal values into the policy in \cref{eq:opt_alpha_pol_app}, we have
\begin{align}
\piopt(a|s) &= \pi_0(a|s) [ 1 + \beta (\alpha-1) ( Q_{*}(a,s) \underbrace{- V_*(s) - \frac{1}{\beta}(1-\alpha) D_{\alpha}[\pi_0:\piopt])}_{-\normalizeralpha} ]_+^{\frac{1}{\alpha-1}}  \\
&= \pi_0(a|s) \exp_{\alpha}\big\{ \beta \cdot \big(  Q_{*}(a,s) - V_*(s) - \frac{1}{\beta}(1-\alpha) D_{\alpha}[\pi_0:\piopt] \big) \big\} 
\end{align}
Finally, we can rewrite the worst-case reward perturbations $\propt(a,s)$ (\cref{eq:optimal_perturbations} or \cref{eq:worst_case_reward_perturb}) for this optimal policy as follows
\begin{align}
\propt(a,s) &= \frac{1}{\beta}\log_{\alpha}\frac{\pi(a|s)}{\pi_0(a|s)} + \frac{1}{\beta}(1-\alpha) D_{\alpha}[\pi_0:\piopt] \\
&= Q_{*}(a,s) - V_*(s) - \frac{1}{\beta}(1-\alpha) D_{\alpha}[\pi_0:\piopt]  +\frac{1}{\beta} D_{\alpha}[\pi_0:\piopt] \\
&= Q_{*}(a,s) - V_*(s) 
\end{align}
which demonstrates that the worst-case reward perturbations $\propt(a,s)$ for the optimal policy $\piopt(a|s)$ correspond to the (optimal) advantage function $\propt(a,s) =  Q_{*}(a,s) - V_*(s)$.
\end{proof}

\begin{figure*}
\begin{minipage}{\textwidth}
\vspace*{-.2cm}
% \begin{subfigure}{0.25\textwidth}\includegraphics[width=\textwidth]{figs/conj_by_alpha_confirm/value_norm_beta01_vert.pdf}
% \caption{$\beta=0.1$}\label{fig:value_agg}\end{subfigure}
\begin{subfigure}{0.24\textwidth}\includegraphics[width=\textwidth]{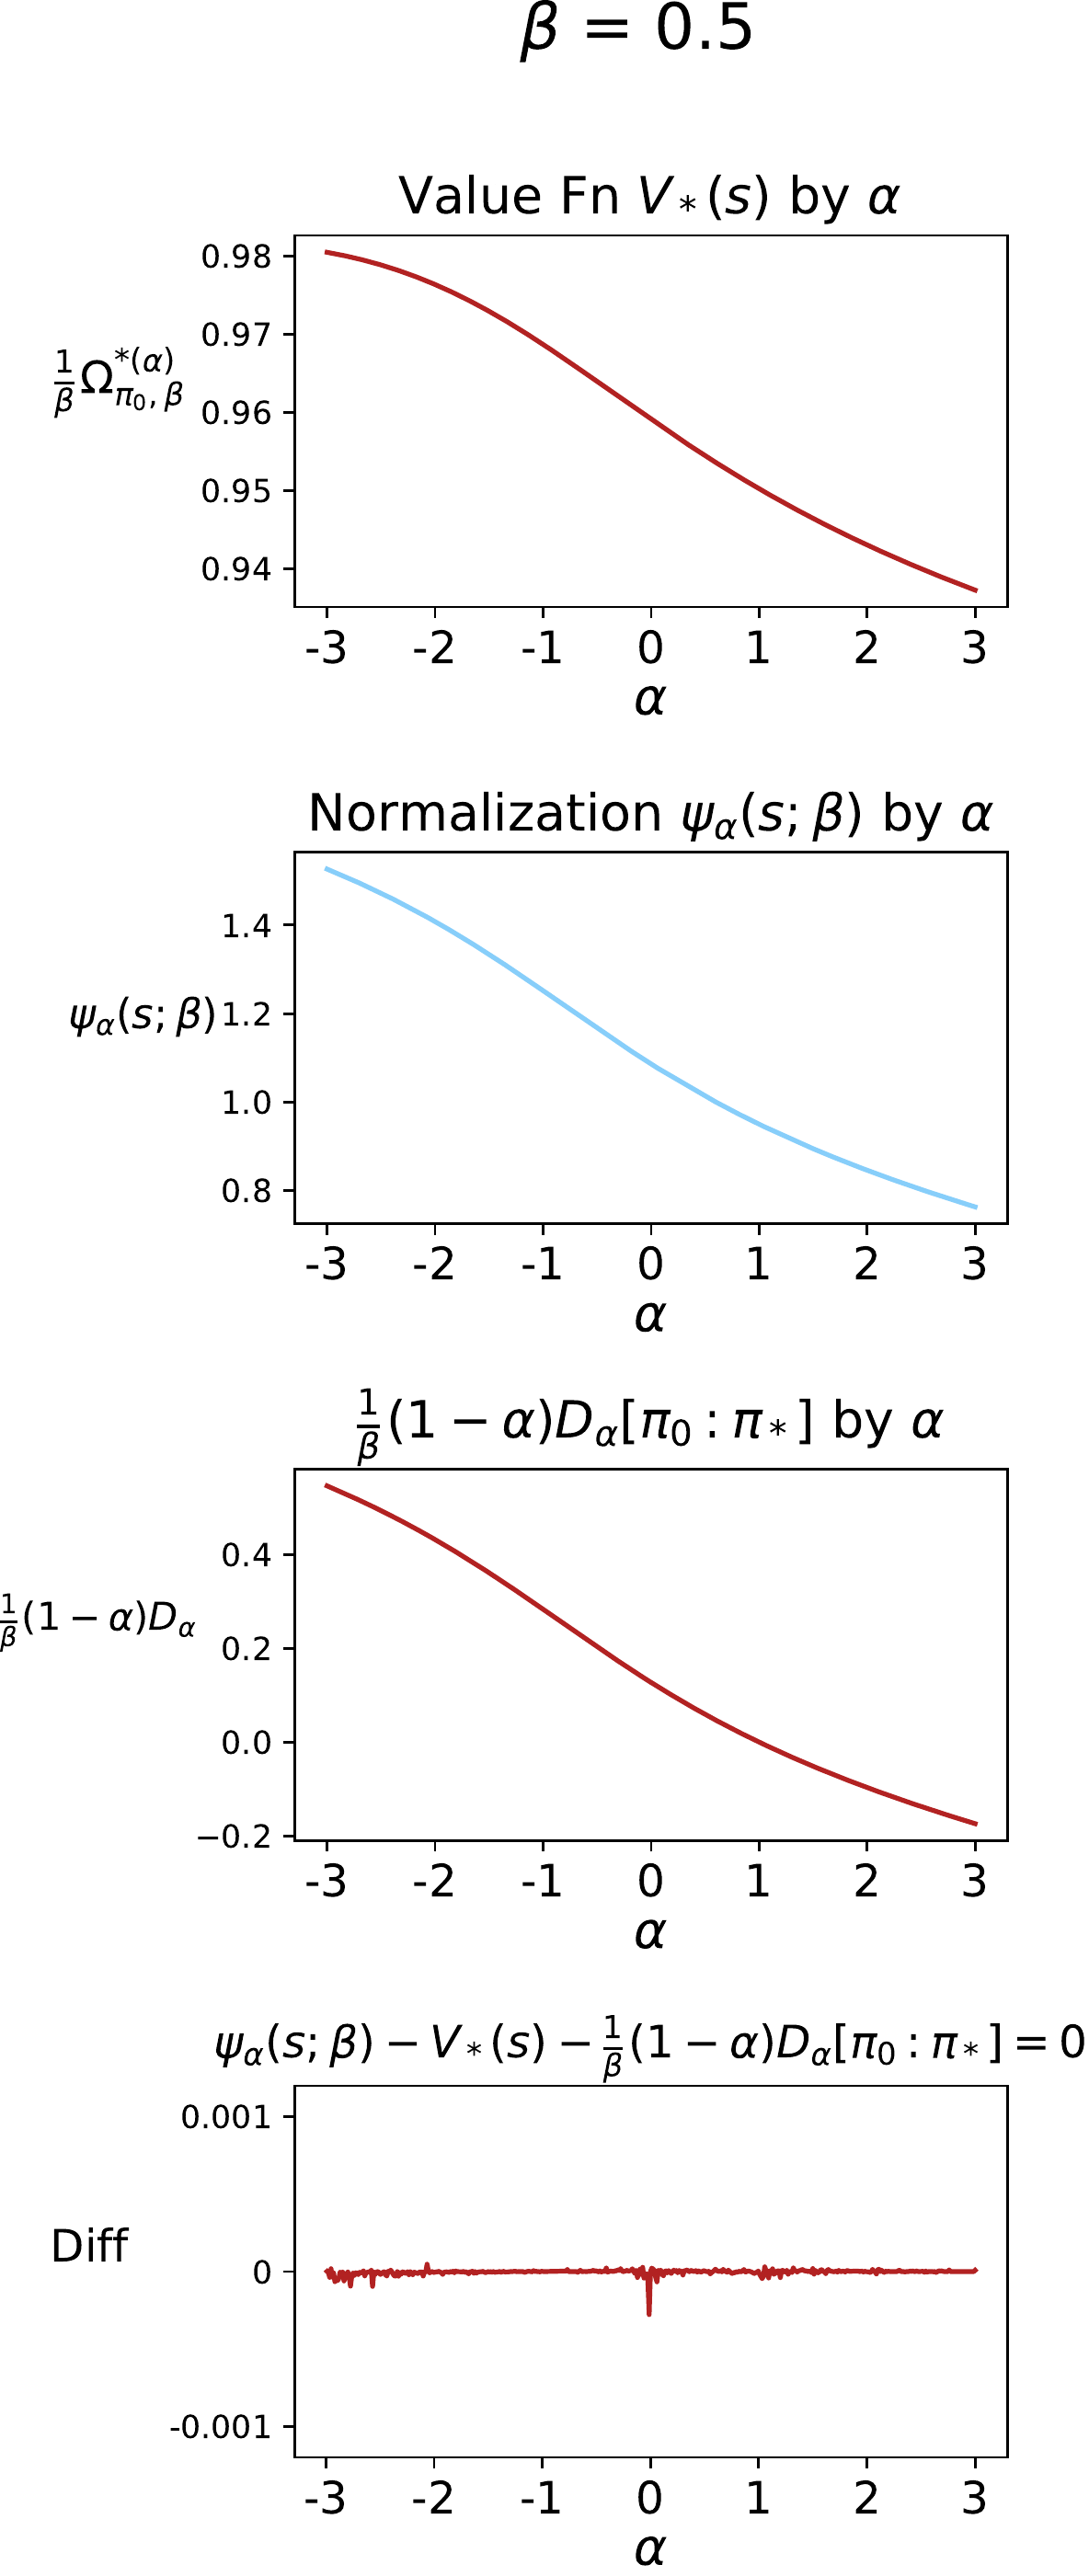}
\caption{$\beta=0.5$}\end{subfigure}
\begin{subfigure}{0.24\textwidth}\includegraphics[width=\textwidth]{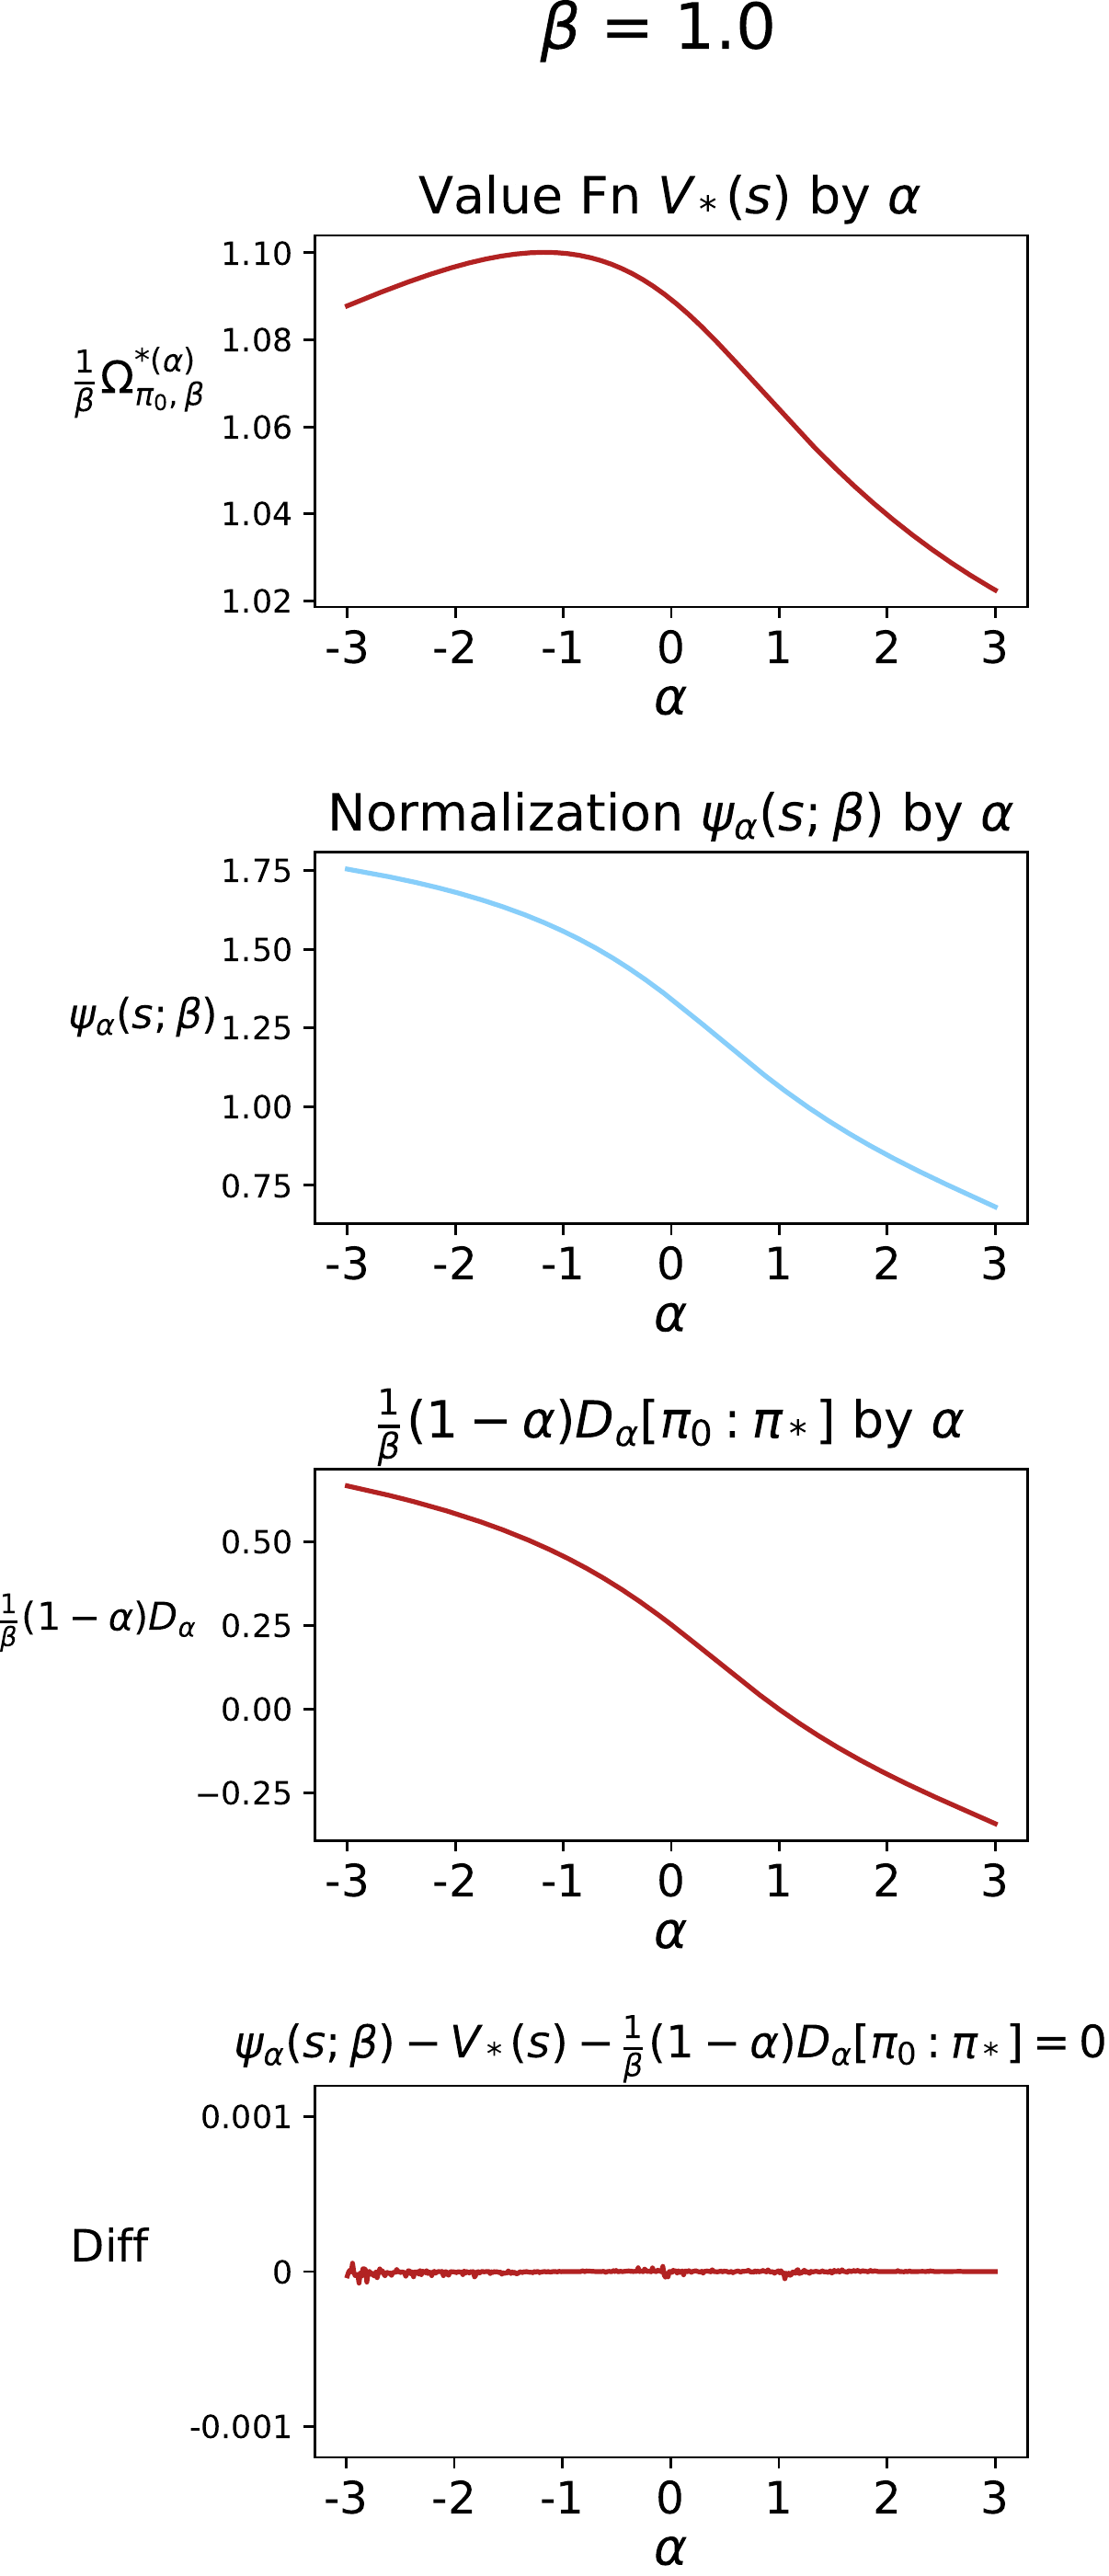}
\caption{$\beta=1$}\end{subfigure}
\begin{subfigure}{0.24\textwidth}\includegraphics[width=\textwidth]{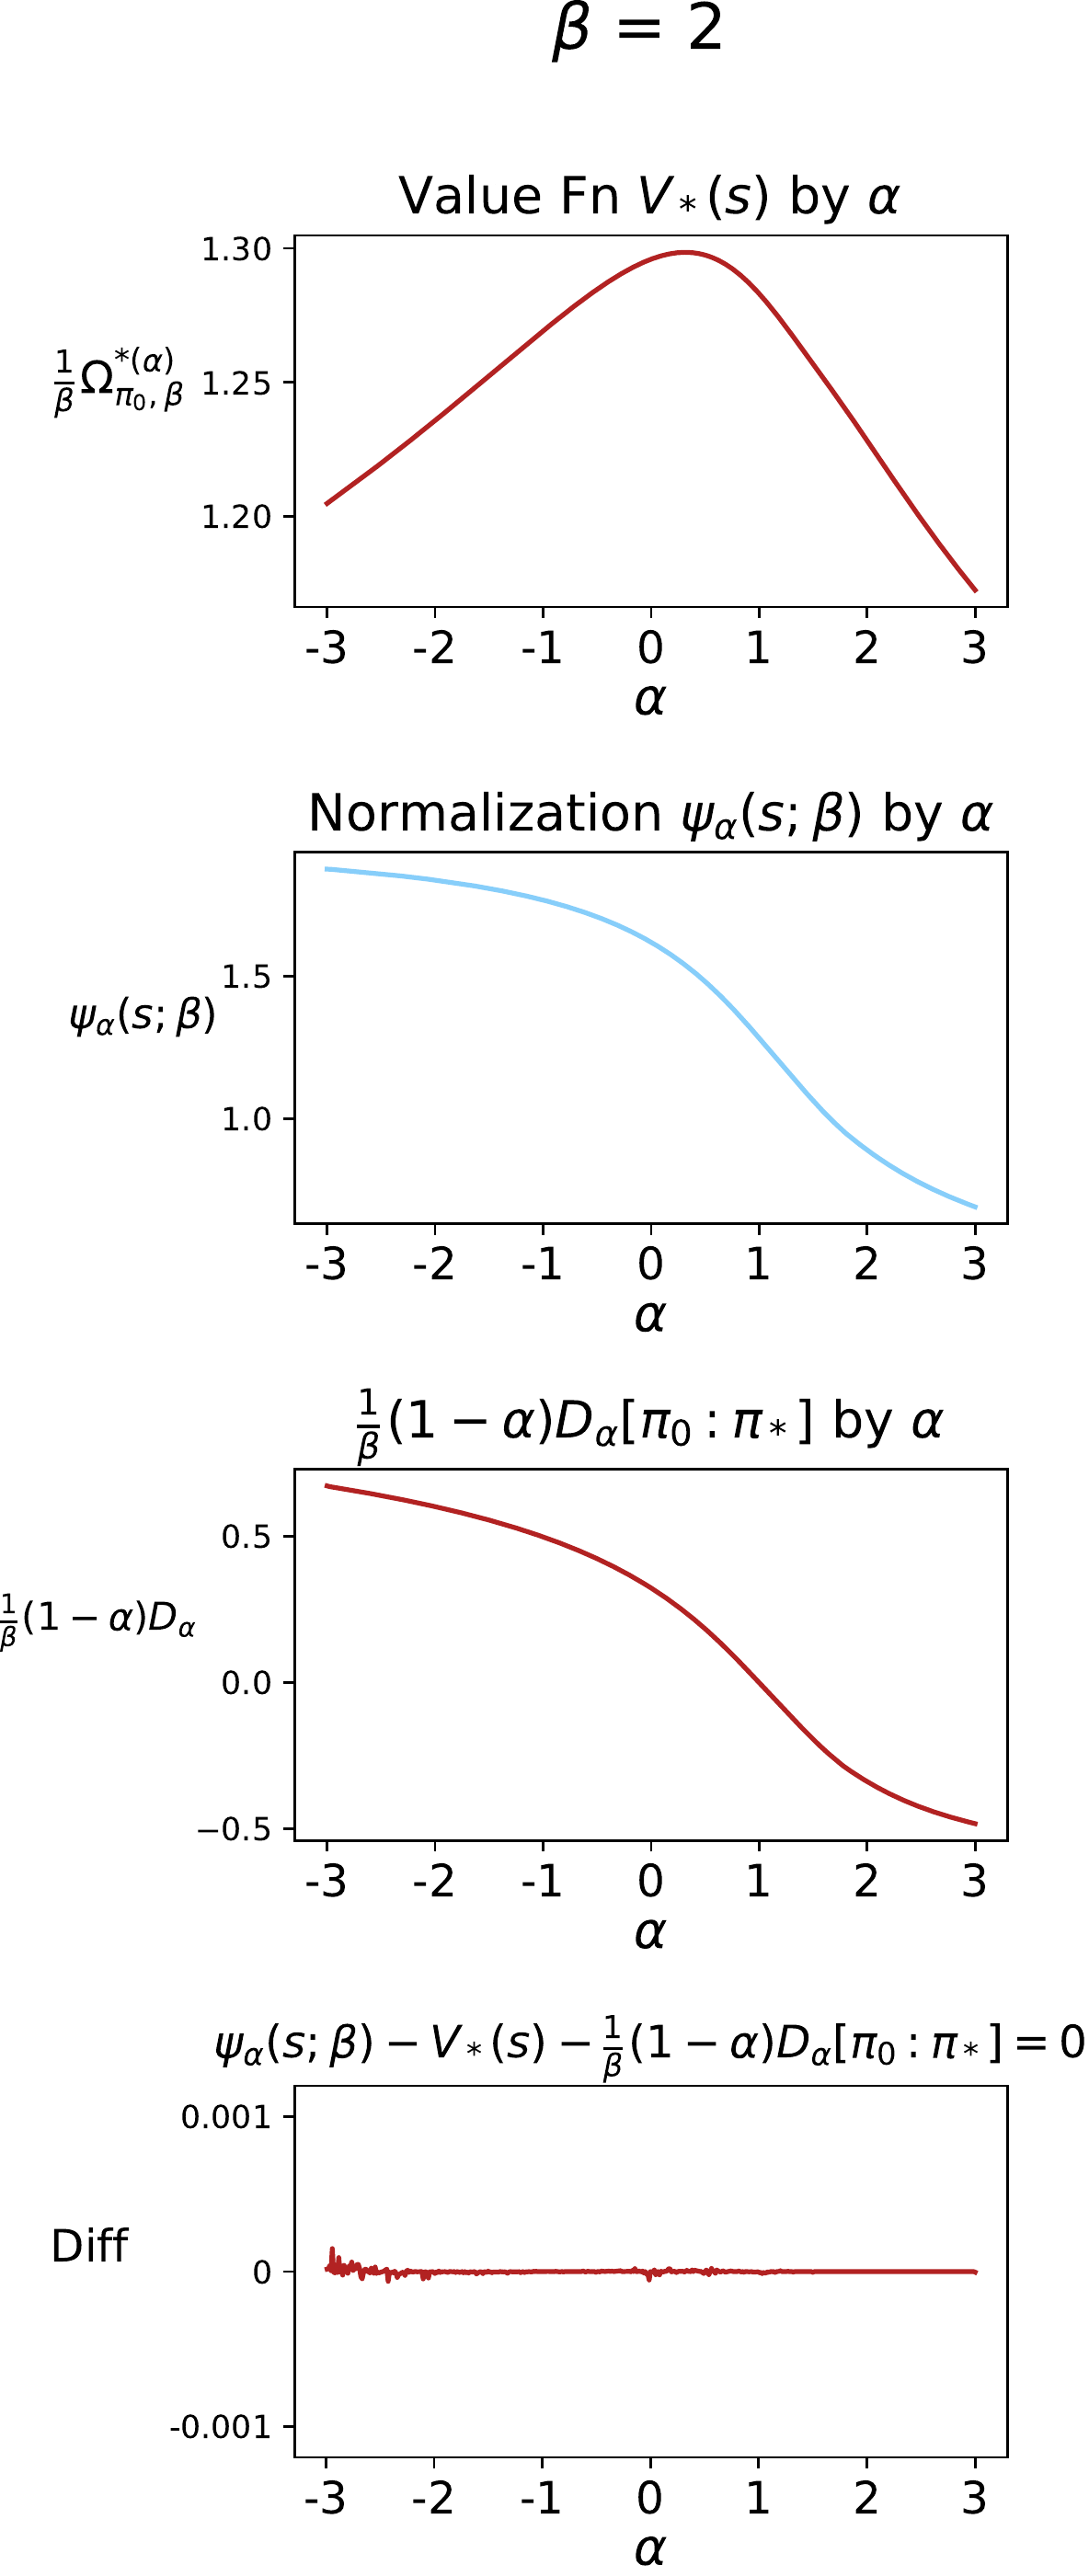}
\caption{$\beta=2$}\end{subfigure}
\begin{subfigure}{0.24\textwidth}\includegraphics[width=\textwidth]{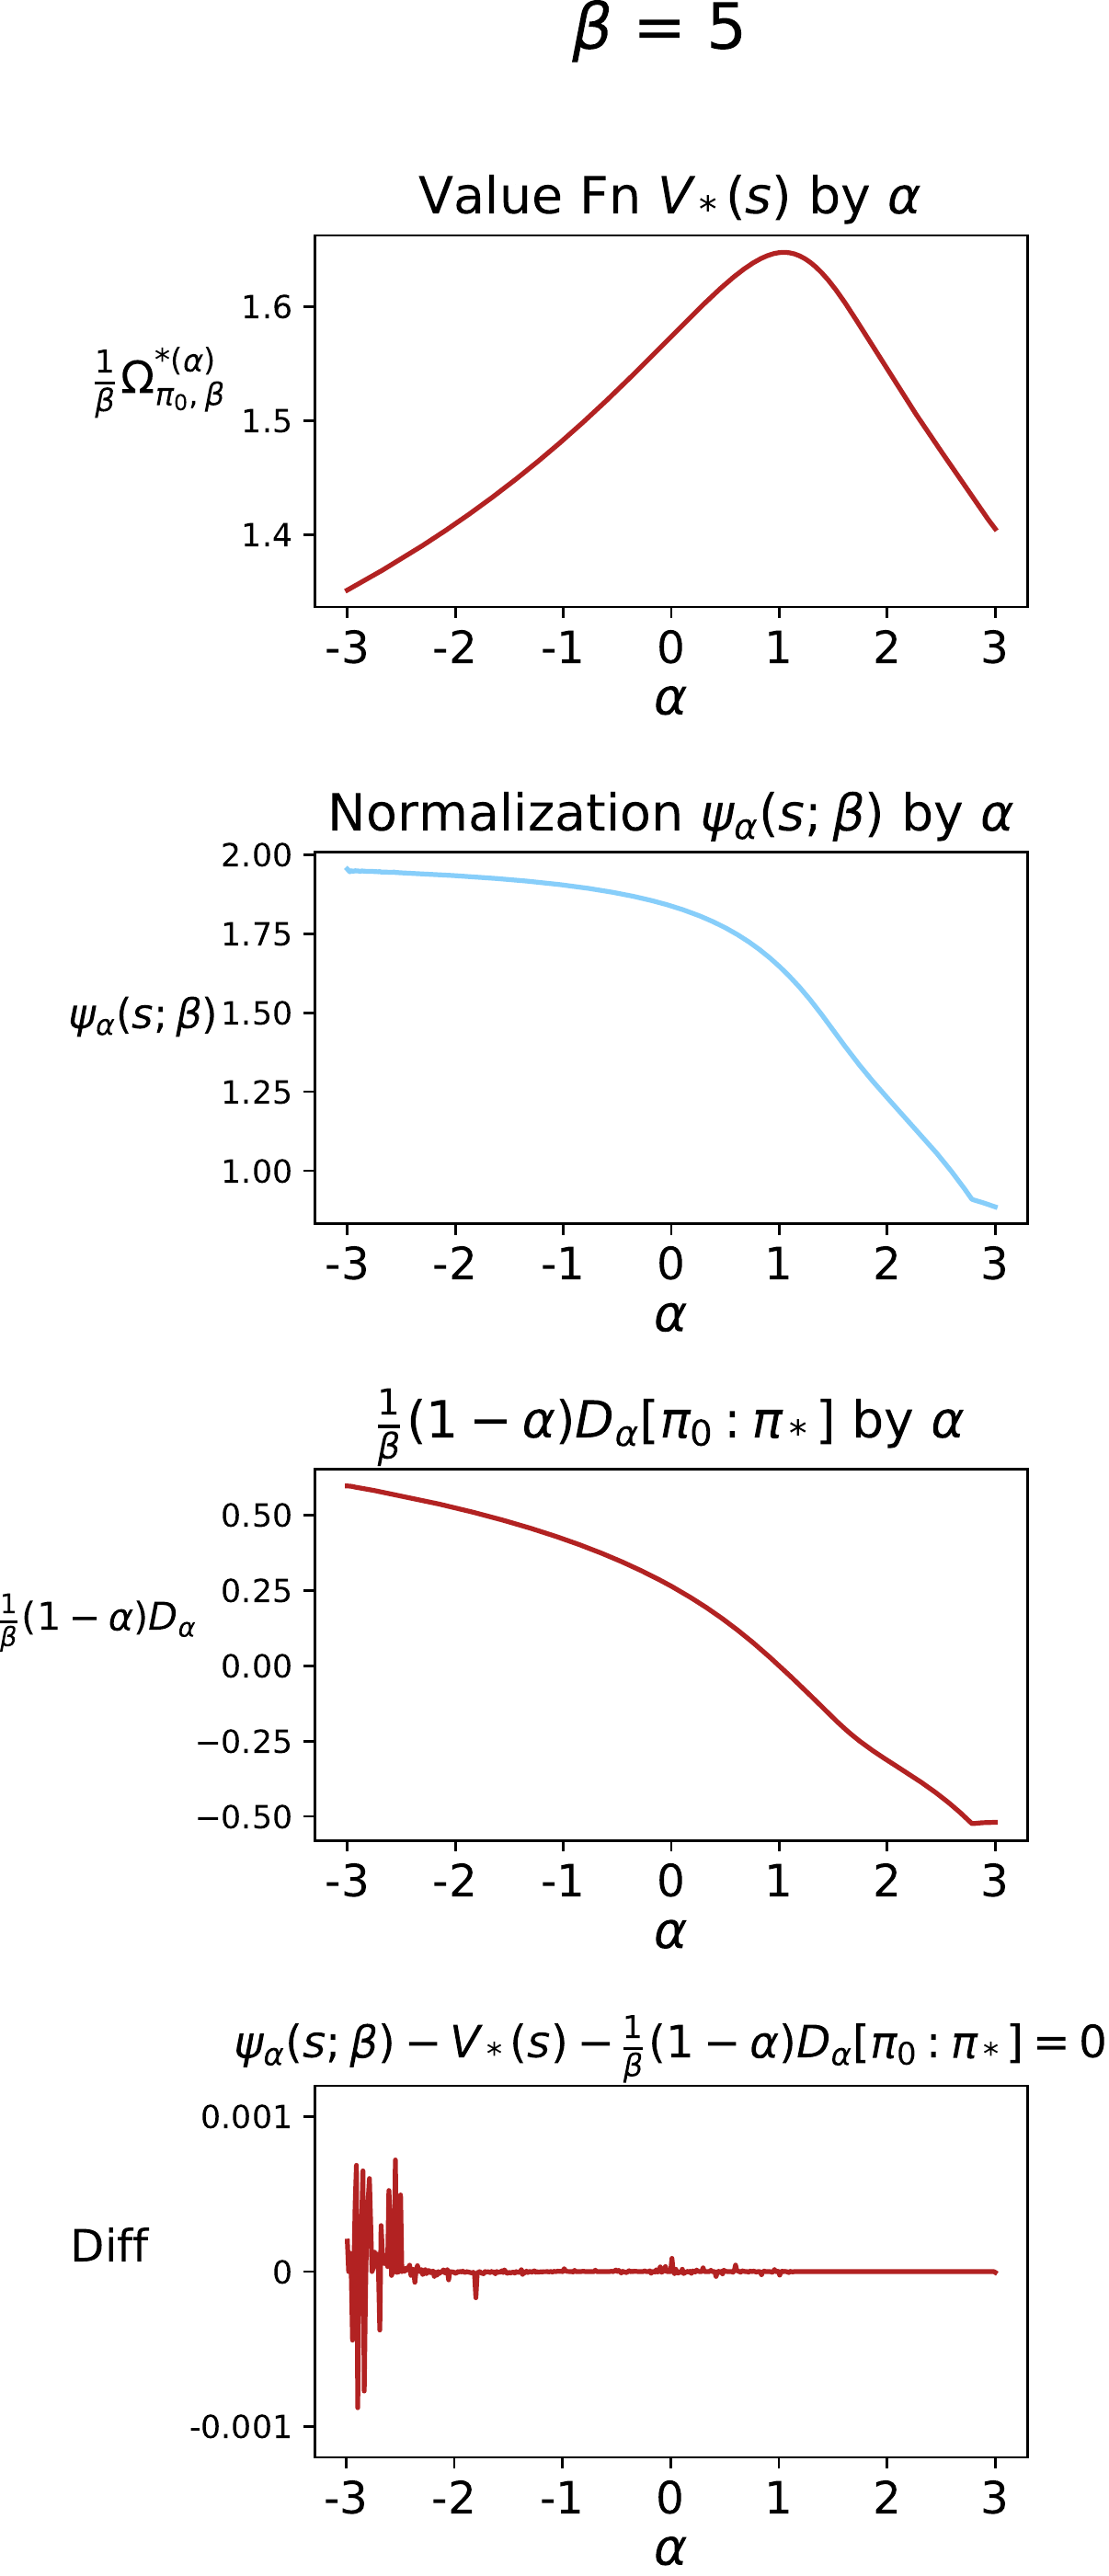}
\caption{$\beta=5$}\end{subfigure}
\caption{ Value Function $V_*(s) = \alphaconjn(Q_*)$ (first row) and Normalization Constant $\psiqopt$ (second row) as a function of $\alpha$ for various regularization strengths $\beta$.   We use the same rewards as in  \myfig{perturb_opt} and \myfig{value_agg_main} and a uniform reference.
We plot $\psipr = \frac{1}{\beta}(1-\alpha)D_{\alpha}[\pi_0:\piopt]$ in the third row, and confirm the identity $V_*(s) = \psiqopt - \psipr$ from \cref{eq:value_and_normalizers} and (\ref{eq:subtractive_relationship}) in the last row.   We find that this equality holds for all $\alpha$ up to small optimization errors on the order of $10^{-3}$.
% Recall that $V(s)= \alphaconjn(Q) = \frac{\alpha-1}{\alpha}   \langle \piopt(a|s), \, Q(a,s)  \rangle   +  \textcolor{red}{\psi_Q(s;\beta)}$ where $\psi_Q(s;\beta)$ is the normalization constant for the optimizing argument $\piopt(a|s) = \pi_0(a|s)[1+(\alpha-1) \beta \big(Q(a,s) - \psi_Q(s;\beta) \big)]_+^{\frac{1}{\alpha-1}}$.  For $\alpha =1$, $V_*(s) = \psi(s;\beta)$ and $\piopt(a|s) = \pi_0(a|s)\exp\{\beta \big(r(a,s) - \normalizerexp \big)\}$. We use the same rewards as in \cref{fig:perturb_opt} and \cref{fig:value_agg_main}.  We emphasize the smaller scale of the $y$-axis in the top row for $V_*(s)$ plots and in the fourth row for confirming \textcolor{red}{$V_*(s) - \normalizeralpha = \frac{1}{\beta}(1-\alpha)D_{\alpha}[\pi_0:\piopt]$.}   We find that this equality holds for all $\alpha$, apart from numerical optimization errors on the order of $10^{-3}$ for $\beta =5$ and $\alpha \approx -3$.
}\label{fig:conj_by_alpha_app}
\end{minipage}
\begin{minipage}{\textwidth}
\vspace*{1cm}
\centering
\begin{subfigure}{0.4\columnwidth}\includegraphics[width=.676\textwidth]{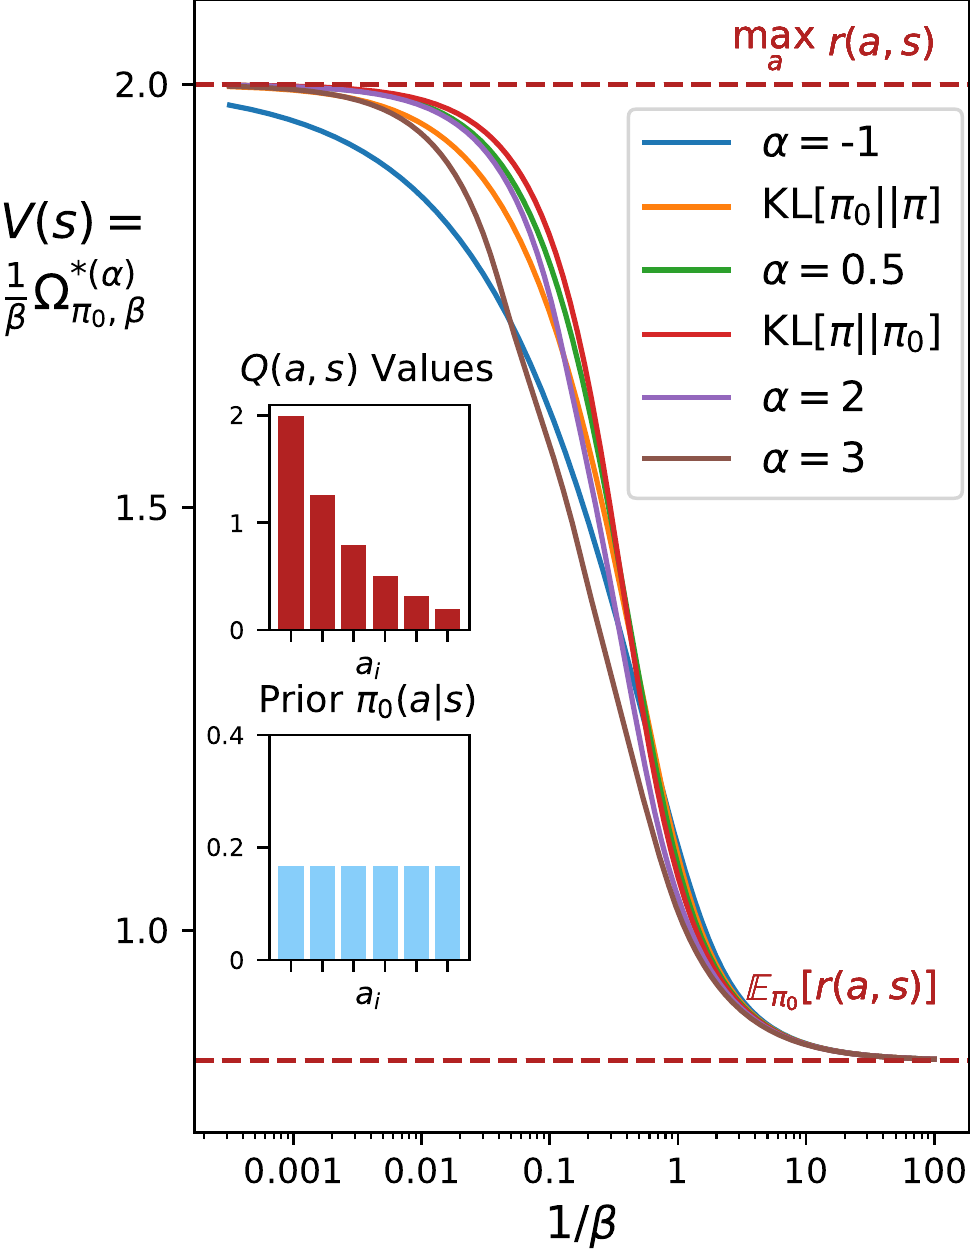}
\caption{Uniform $\pi_0(a|s)$}
% \label{fig:value_agga}
\end{subfigure}\hspace*{.01\columnwidth}
\begin{subfigure}{0.4\columnwidth} 
% \vspace*{-.12cm}\includegraphics[scale=.3]{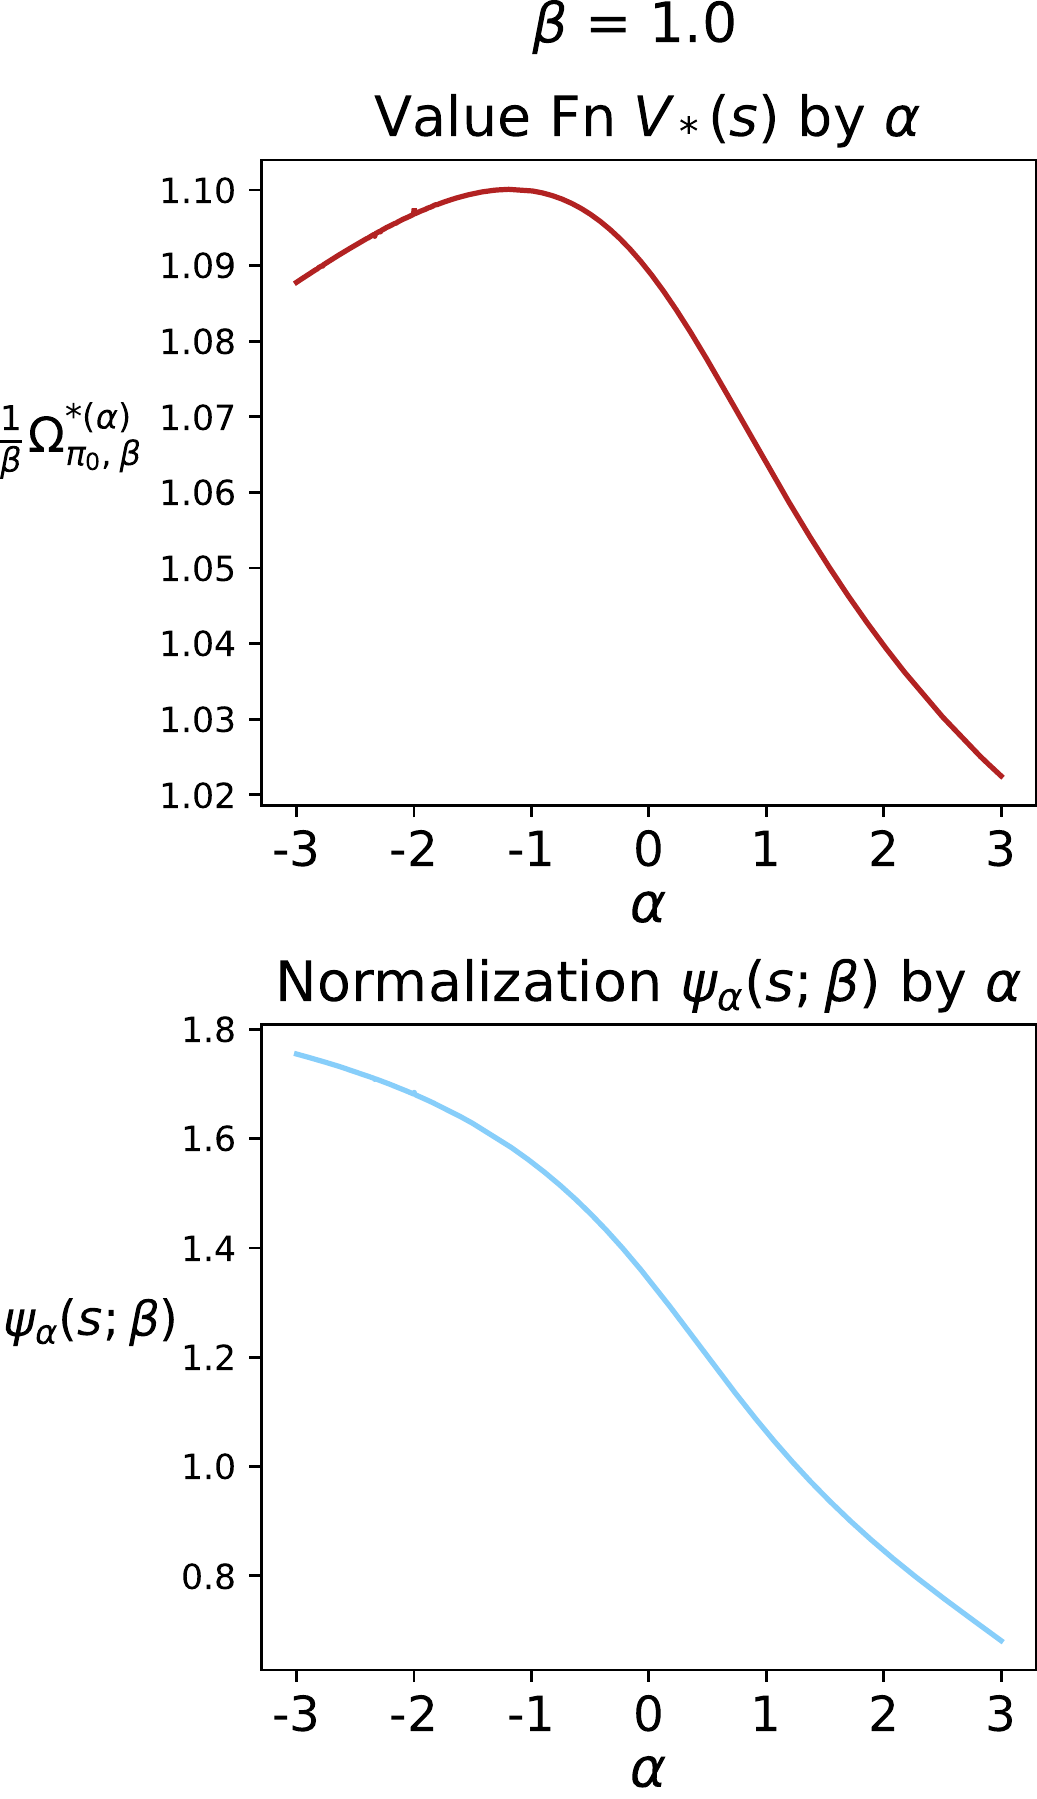}
% \vspace*{-.1cm}\includegraphics[width=.96\textwidth]{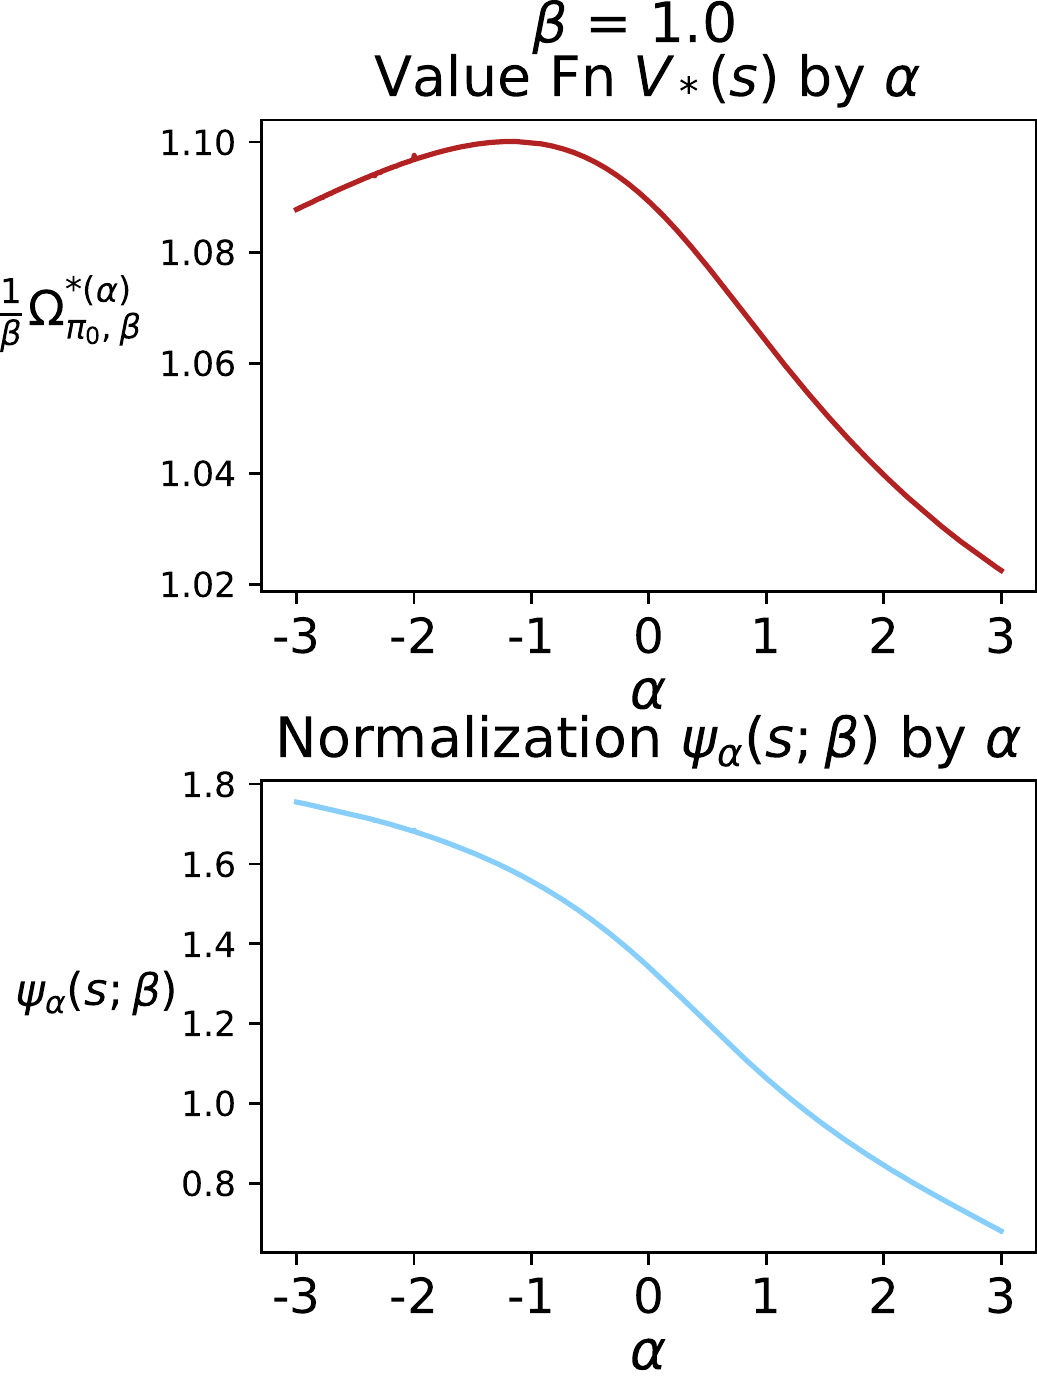}
% \caption{$V(s)$ and $\psi_{\alpha}(s)$ as a function of $\alpha$ for $\beta=1$}\label{fig:value_aggb}\end{subfigure}
\vspace*{-.1cm}\includegraphics[width=.676\textwidth]{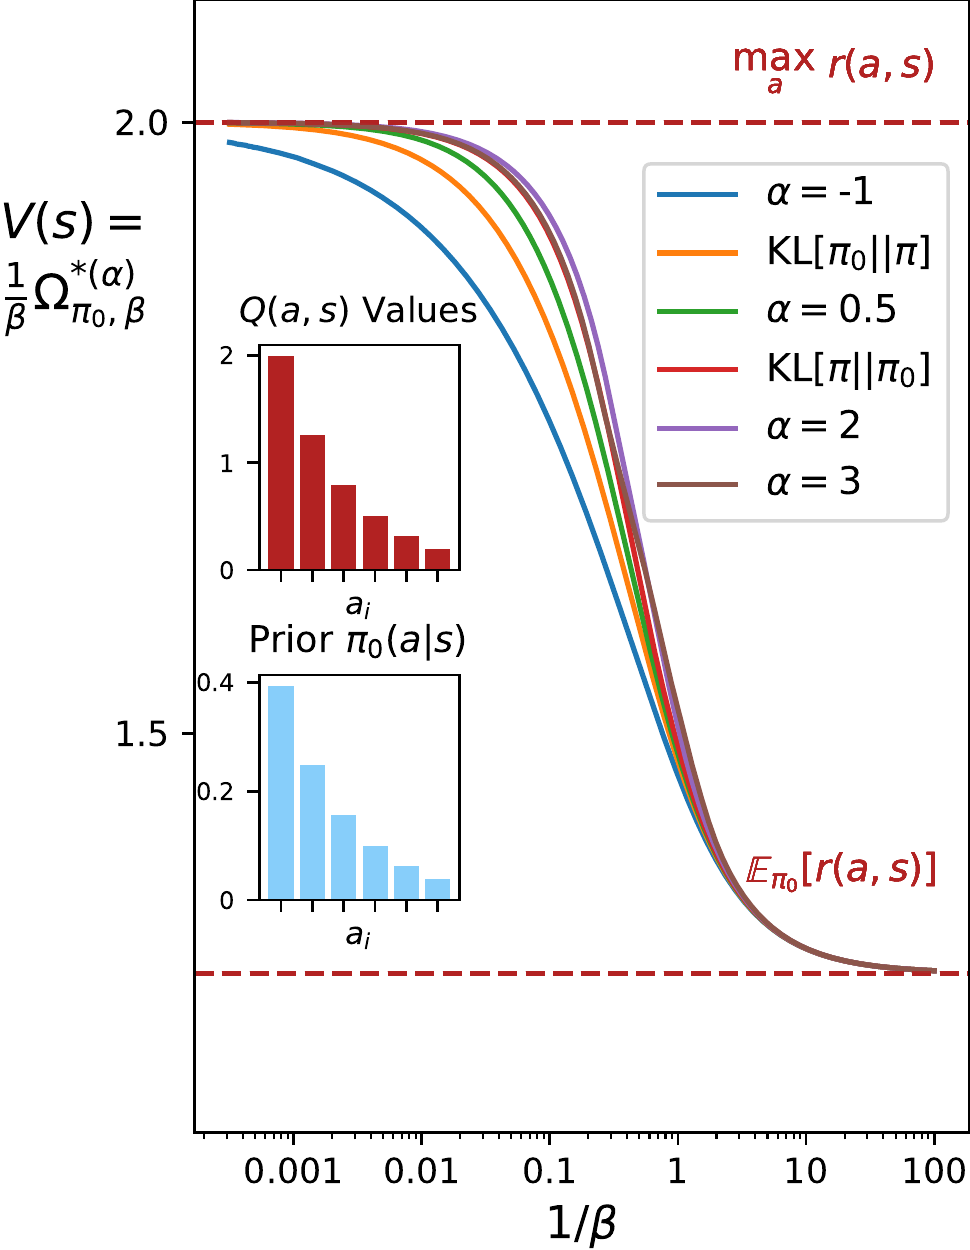}
\caption{$\pi_0(a|s) \propto r(a,s) $}
% \label{fig:value_agga}
\end{subfigure}
\captionof{figure}{Value function $V(s) = \alphaconjm(Q)$ as a function of $\beta$ (x-axis) and $\alpha$ (colored lines), using $Q(a,s)$ and $\pi_0(a|s)$ from the left inset.   See \cref{eq:kl_bellman} and \cref{eq:alpha_bellman} for closed forms.}\label{fig:value_agg_main} %and normalization constant $\psi_{\alpha}(s)$
\end{minipage}
\end{figure*}
\subsection{Confirming the Relationship between Normalization and Value Function}\label{app:advantage_confirm}
It is known that $V_*(s) = \normalizerexp$ in the case of \textsc{kl} divergence regularization \citep{ortega2013thermodynamics, fox2016taming,haarnoja17a}.  However, the relationship between $V_*(s)$ and $\normalizeralpha$ for general $\alpha$-divergences is less well-understood.   In \myfig{conj_by_alpha_app}, we plot both $V_*(s)$ and $\normalizeralpha$ for various values of $\alpha$ (x-axis) and $\beta$ (in each panel).     We also plot the value of $\frac{1}{\beta}(1-\alpha) D_{\alpha}[\pi_0:\piopt]$ in the third row, and confirm the identity in \cref{eq:psidentity_app} in the fourth row.

 As we also observed in \myfig{value_agga}, the soft value function or certainty equivalent $V_*(s) = \alphaconjn(Q)$ is not monotonic in $\alpha$ for this set of single-step rewards (the same $r(a,s)$ as in \myfig{perturb_opt} or \myfig{value_agga}). 

While it can be shown that $\normalizeralpha$ is convex as a function of $\beta$ \citep{amari2011q}, we see that $\normalizeralpha$ is not necessarily convex in $\alpha$ and appears to be monotonically decreasing in $\alpha$.   Finally, we find that the identity in \cref{eq:psidentity_app} holds empirically, with only small numerical optimization issues.
 % for high $\beta$ and $\alpha \approx -3$.
