# Supplementary material for: Your Policy Regularizer is Secretly an Adversary
Source: arXiv:2203.12592 source file (2022-07-08)
Supplement: Supplementary file 3 [file 6_feasible_pf.tex]

\section{Feasible Set (Proof of \myprop{feasible})}\label{app:feasible_pf}\label{app:feasible}
In this section, we derive a constrained optimization corresponding to the Lagrangian relaxation in \cref{eq:pedro_form} of the main text.  This allows us to characterize the feasible set of reward perturbations, which represents both the possible strategies of the adversary and the reward function changes to which a particular policy is robust.   Finally, we detail our approach to construct the feasible set plots in \myfig{feasible_set_main} and \myfig{feasible_set_uniform_app}-\ref{fig:feasible_set_nonuniform_app}.

% \begin{restatable}[(\citet{husain2021regularized} App. 7 and 7.8.1)]{lemma}{increasing}
% \label{lemma:increasing}
% The conjugate function $\alphaconjmu$ is increasing in $\pr(a,s)$, in the sense that if $\pr_1(a,s) \geq \pr_2(a,s)$ for all $a \in \mathcal{A}, s \in \mathcal{S}$, then $\alphaconjmu(\pr_1) \geq \alphaconjmu(\pr_2)$.
% \end{restatable}
% \citet{husain2021regularized} show this result for arbitrary $f$-divergences, 
% with the $\alpha$-divergence included as a special case (see \myapp{tsallis}).  
\feasible*
\begin{proof}
The proof \footnote{\textcolor{red}{Our proof differs from the intuitive arguments given in the main text. Note that $\alphaconjmu(\pr)$ increasing \textit{does not} imply the constraint $\alphaconjmu(\pr)\leq 0$ based on the optimization in \cref{eq:pedro_form}.     The fact that the conjugate function $\alphaconjmu$ is increasing in $\pr(a,s)$, in the sense that if $\pr_1(a,s) \geq \pr_2(a,s)$ for all $a \in \mathcal{A}, s \in \mathcal{S}$ then $\alphaconjmu(\pr_1) \geq \alphaconjmu(\pr_2)$, is shown for general $f$-divergences in \citet{husain2021regularized} App. 7.8.1, which includes the $\alpha$-divergence as a special case.}} is closely related to the result in  \myapp{preserve} \myprop{conjugatezero} that $\alphaconjmu(\propt)=0 \, \forall \alpha$ for the worst-case reward perturbations $\propt(a,s)$ associated with a particular policy $\pi(a|s)$ or occupancy measure $\mu(a,s)$.   

Considering the unconstrained optimization over $\pr(a,s)$ in \cref{eq:pedro_form}
% We can now use \mylemma{increasing} to show that perturbations with $\alphaconjmu \leq 0$ will be feasible for an adversary which minimizes the objective
\small
\begin{align}
    \hspace*{-.2cm} & \quad \max \limits_{\mu(a,s)} \min \limits_{V(s)} \min \limits_{\textcolor{\highlight}{\perturbr(a,s)}}  \big \langle {\mu(a,s)}, {r(a,s) +\gamma \transitionv - V(s) - \textcolor{\highlight}{\perturbr(a,s)}} \brangle + \alphaconjmu \big( \textcolor{\highlight}{\perturbr} \big) + (1-\gamma) \blangle \nu_0(s), V(s) \brangle \, ,  \, \label{eq:pedro_form4}
\end{align}
\normalsize
Informed by the result in \myprop{conjugatezero}, we can recognize $\frac{1}{\beta}$ as a Lagrange multiplier enforcing a constraint on the conjugate $\alphaconjmu( {\perturbr}) \leq 0$.   Note that no additional constants are required to enforce the inequality constraint.   Since $\frac{1}{\beta} > 0$ by assumption, we can see that $\alphaconjmu( {\perturbr}) > 0$ incurs a penalty in the minimization objective.   Finally, the complementary slackness condition \citep{boyd2004convex} suggests that, at optimality, we will have $\alphaconjmu( {\perturbr}) = 0$ as in \myprop{conjugatezero}.
Thus, the constrained optimization corresponding to \cref{eq:pedro_form4} becomes
\begin{align}
     \quad \max \limits_{\mu(a,s)} \min \limits_{V(s)} \min \limits_{\textcolor{\highlight}{\perturbr(a,s)}}  \big \langle {\mu(a,s)}, &{r(a,s) +\gamma \transitionv - V(s) - \textcolor{\highlight}{\perturbr(a,s)}} \brangle  + (1-\gamma) \blangle \nu_0(s), V(s) \brangle \quad \label{eq:pedro_form_constrained} \\
     &\text{subj. to } \,\, \alphaconjmu \big( \textcolor{\highlight}{\perturbr} \big) \leq 0 \nonumber \, 
\end{align}
For the \textsc{kl} divergence, we confirm that $\klconjmu(\pr)$ takes a form which is analogous to  the conjugate derived using optimization over $\pi(a|s)$ in \myapp{kl_conj_all}.  
To do so, we plug the policy $\pir(a|s) = \pi_0 \exp \{ \beta \cdot (\pr(a,s) - \psi(\pr, s;\beta)) \}$ that corresponds a particular reward perturbation into the conjugate optimization
\begin{align}
    \klconjmu &= \blangle \mu(s) \pir(a|s), \pr(a,s) \brangle - \frac{1}{\beta} \blangle \mu(s) \pir(a|s), \cancel{\log \exp} \{ \beta \cdot (\pr(a,s) - \psi(\pr, s;\beta)) \}\brangle \\
    &= \blangle \mu(s), \psi(\pr, s;\beta) \brangle = \blangle \mu(s), \frac{1}{\beta} \log \sum \limits_{a \in \mathcal{A}} \pi_0(a|s) \exp \{ \beta \cdot \pr(a,s) \} \brangle
\end{align}

We consider plotting the feasible set for the single step case in the next section, \cref{fig:feasible_set_main}, and \myfig{feasible_set_uniform_app}-\ref{fig:feasible_set_nonuniform_app}.   In this case, we can ignore the possibility that we have both positive and negative $\log \sum_{a} \pi_0(a|s) \exp \{ \beta \cdot \pr(a,s) \} \lessgtr 0$ in various $s \in \mathcal{S}$, but that averaging over $\mu(s)$ would still fulfill the constraint.  
Simplifying the constraint $\klconjpi \leq 0$ at each $s \in \mathcal{S}$, we remove the $\frac{1}{\beta}$ constant factor and exponentiate both sides to obtain \cref{eq:kl_feasible}
\begin{align}
     \sum\limits_{a \in \mathcal{A}} \pi_0(a|s) \expof{\beta \cdot \pr(a,s)} \leq 1 \, .
\end{align}
\end{proof}

\subsection{Plotting the $\alpha$-Divergence Feasible Set}\label{app:feasible_plot}
To plot boundary of the feasible set for the \textsc{kl} divergence regularization in two dimensions, we can simply solve for the $\pr(a_2,s)$ which satisfies the constraints for a given $\pr(a_1,s)$
\begin{align}
    \pr(a_2,s) = \frac{1}{\beta} \log \frac{1}{\pi_0(a_2|s)}(1- \pi_0(a_1|s) \expof{\beta \cdot \pr(a_1,s)}) \, .
\end{align}
The interior of the feasible set contains $\pr(a_1,s)$ and $\pr(a_2,s)$ that are greater than or equal to these values.

However,  we cannot analytically solve for the feasible set boundary for general $\alpha$-divergences, since the conjugate function $\alphaconjmu$ in \cref{eq:policy_for_perturbed} is defined in self-consistent fashion due to the normalization constant of $\pir(a,s)$.
Instead, we perform exhaustive search over a range of $\pr(a_1, s)$ and $\pr(a_2,s)$ values.  For each pair of candidate reward perturbations, we use \textsc{cvx-py} \citep{diamond2016cvxpy} to solve the optimization
\begin{align}
    \alphaconjn(\pr) = \max \limits_{\pi(a|s)} \blangle \pi(a|s), \pr(a,s) \brangle - \omegapi \,  \label{eq:feasible_set_opt}
\end{align}
which yields the policy $\pir(a|s)$ corresponding to this choice of $\pr(a,s)$.   We also obtain a value for the conjugate function  $\alphaconjn(\pr)$ by evaluating  \cref{eq:feasible_set_opt} at this $\pir(a|s)$.
We can terminate our exhaustive search and record the boundary of the feasible set when we find that $\alphaconjn(\pr) = 0$ within appropriate precision.     
Note that, in the single step case, we do not have to consider the marginal state visitation distribution $\mu(s)$ for either \textsc{kl} or $\alpha$-divergence regularization.
% Note that we are able to avoid optimization over $\mu(s)$
% We can further derive the normalization constant $\normalizerpr$ from the closed form for the policy $\pir(a,s) = \pi_0(a|s) [ 1+\beta(\alpha-1) (\pr(a,s) - \normalizerpr)]_+^{\frac{1}{\alpha-1}}$.  
% Finally, we evaluate the conjugate function $\alphaconjmu(\pr)$ \RB{REFERENCE... WHERE is this written?} for each candidate $\pr(a,s)$.  We can terminate our exhaustive search and record the boundary of the feasible set when we find that $\alphaconjmu(\pr) = 0$ within appropriate precision.

% \subsection{Limiting Behavior for the Feasible Set}\label{app:feasible_plot}
