# Supplementary material for: Your Policy Regularizer is Secretly an Adversary
Source: arXiv:2203.12592 source file (2022-07-08)
Supplement: Supplementary file 4 [file addl_feasible.tex]

\newcommand{\sidefeasible}{.12}
\newcommand{\mainfeasible}{.26}
\begin{figure*}[!t]
\centering
% \begin{minipage}{\textwidth}%{0.8\textwidth}
% \centering
\begin{center}
\[\arraycolsep=.01\textwidth
\begin{array}{cccc} %[width=40mm]
 \begin{subfigure}{\sidefeasible\textwidth}  \phantom{ \includegraphics[width=\textwidth]
 {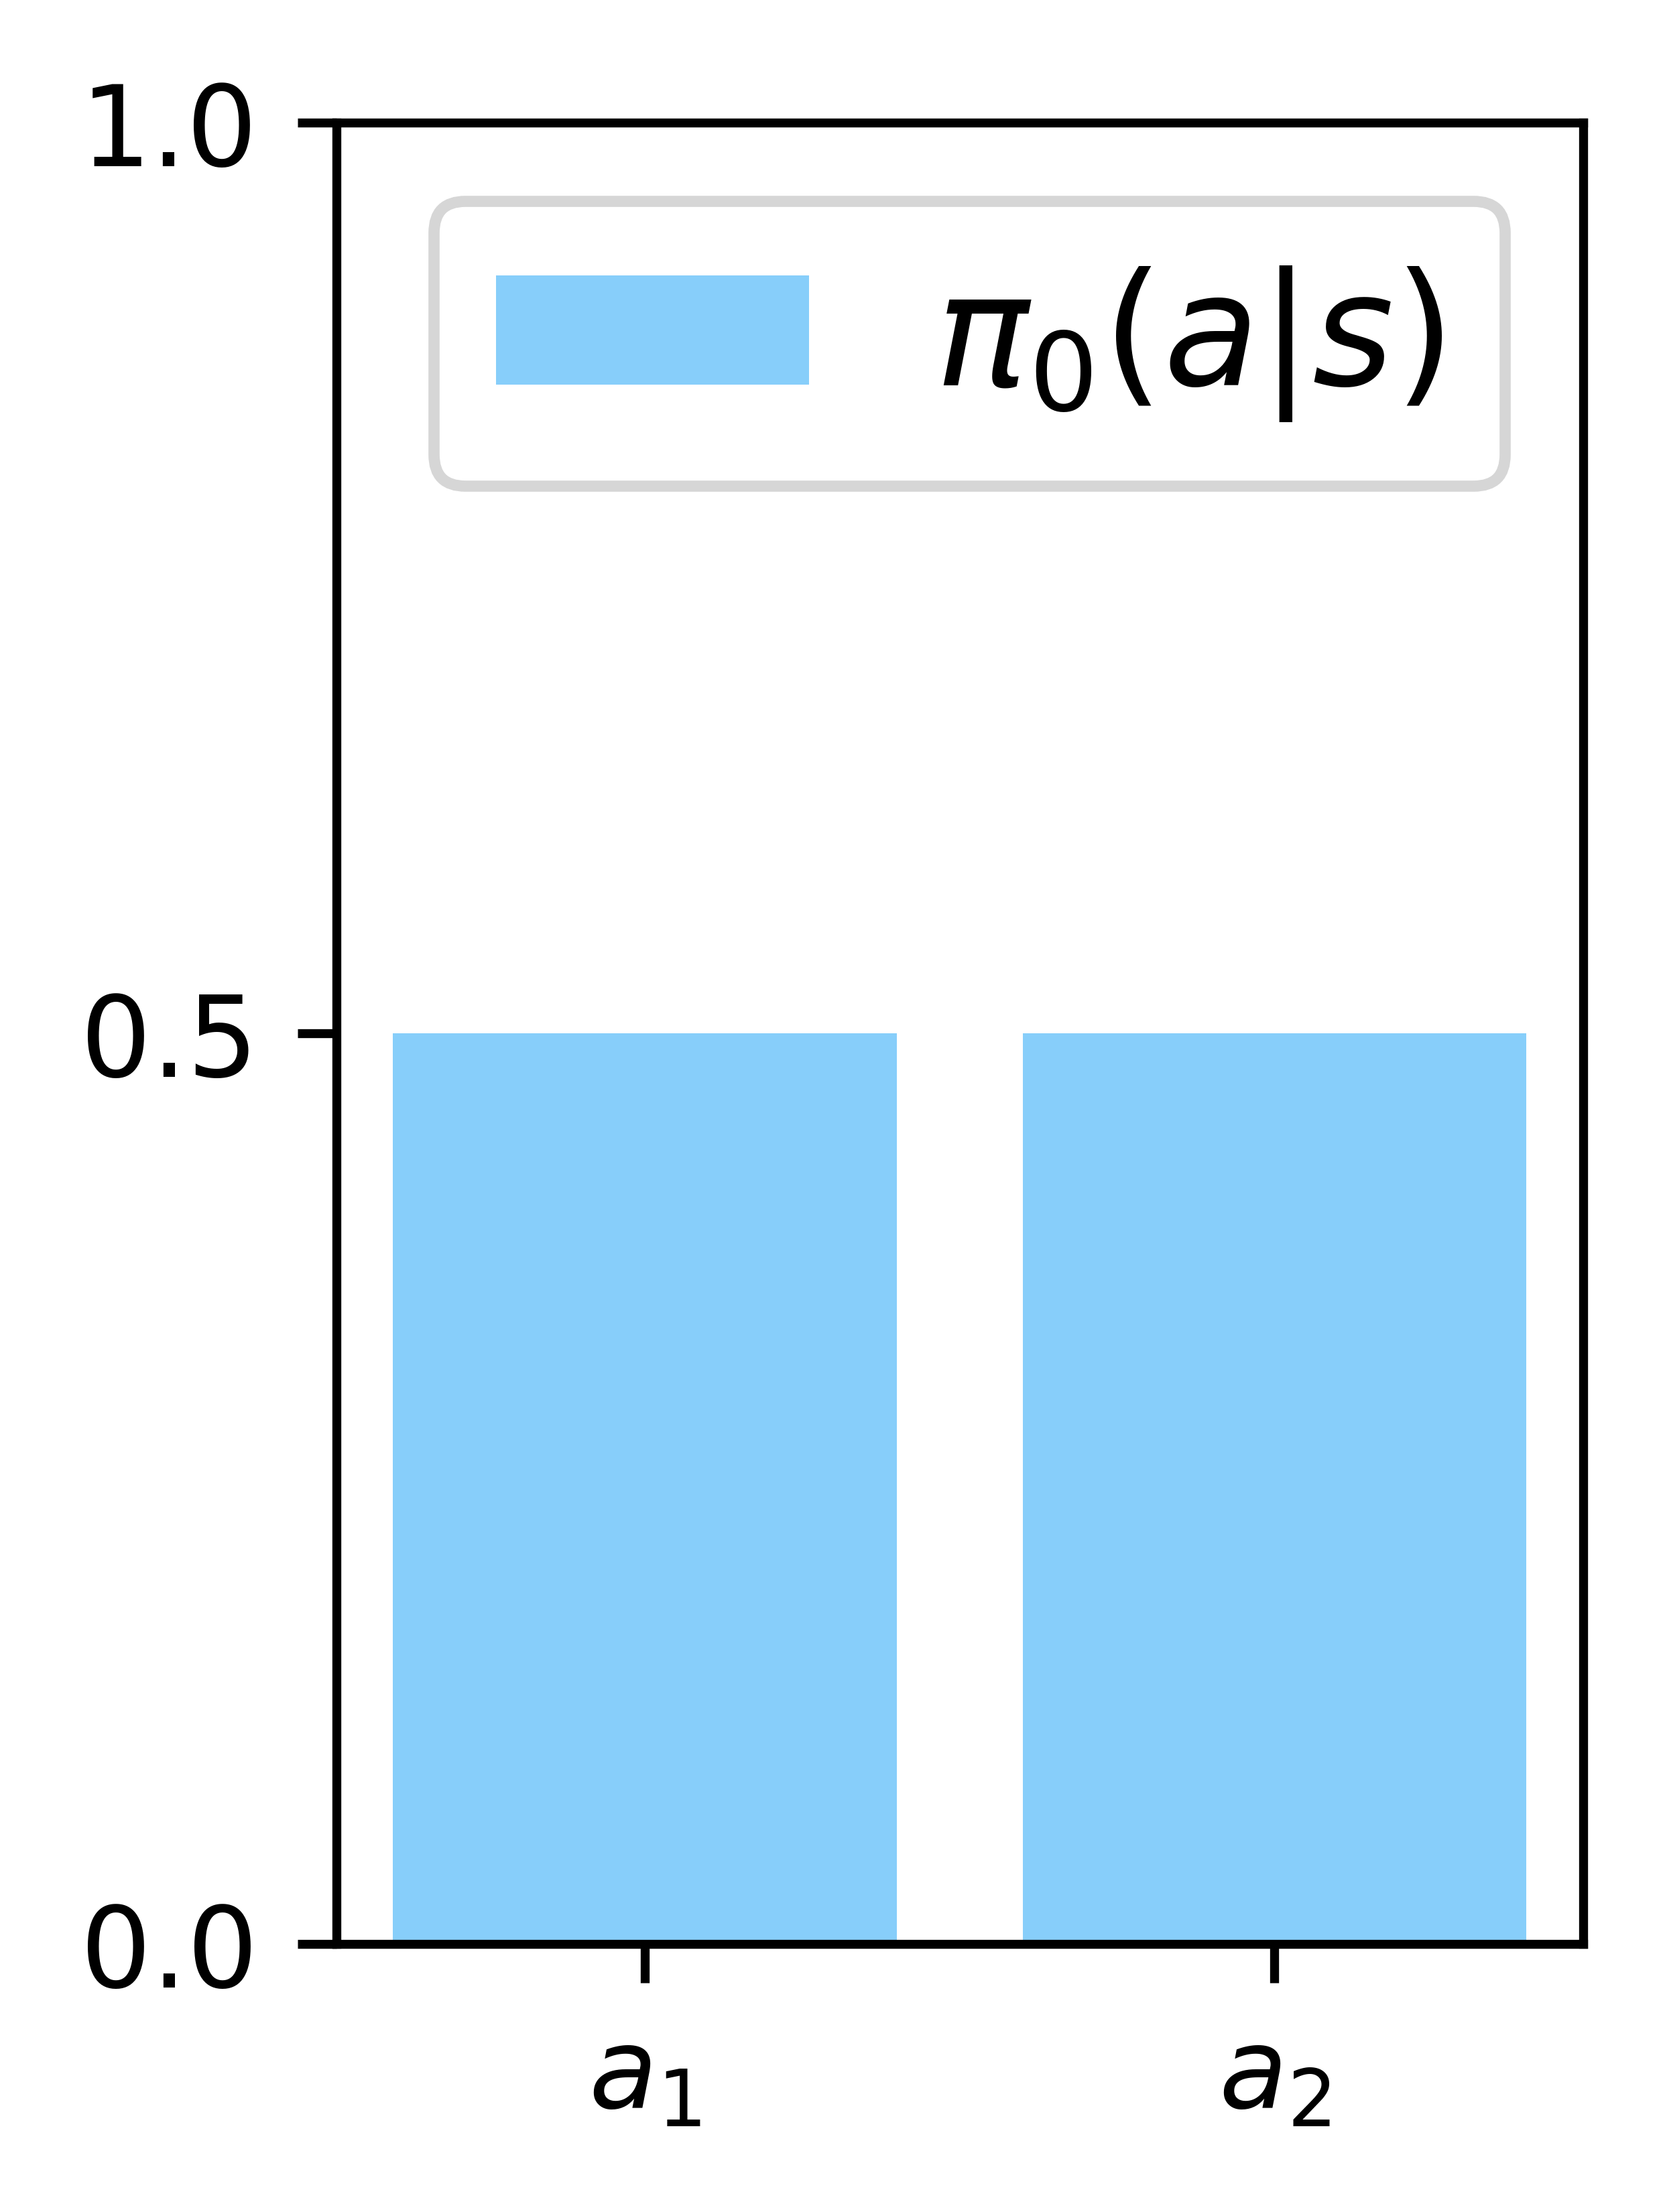}} \end{subfigure} & \begin{subfigure}{\mainfeasible\textwidth}\includegraphics[width=\textwidth, trim= 0 0 0 0, clip]
% {figs/feasible/alpha-1/alpha_neg1_beta1_uniform.png} 
{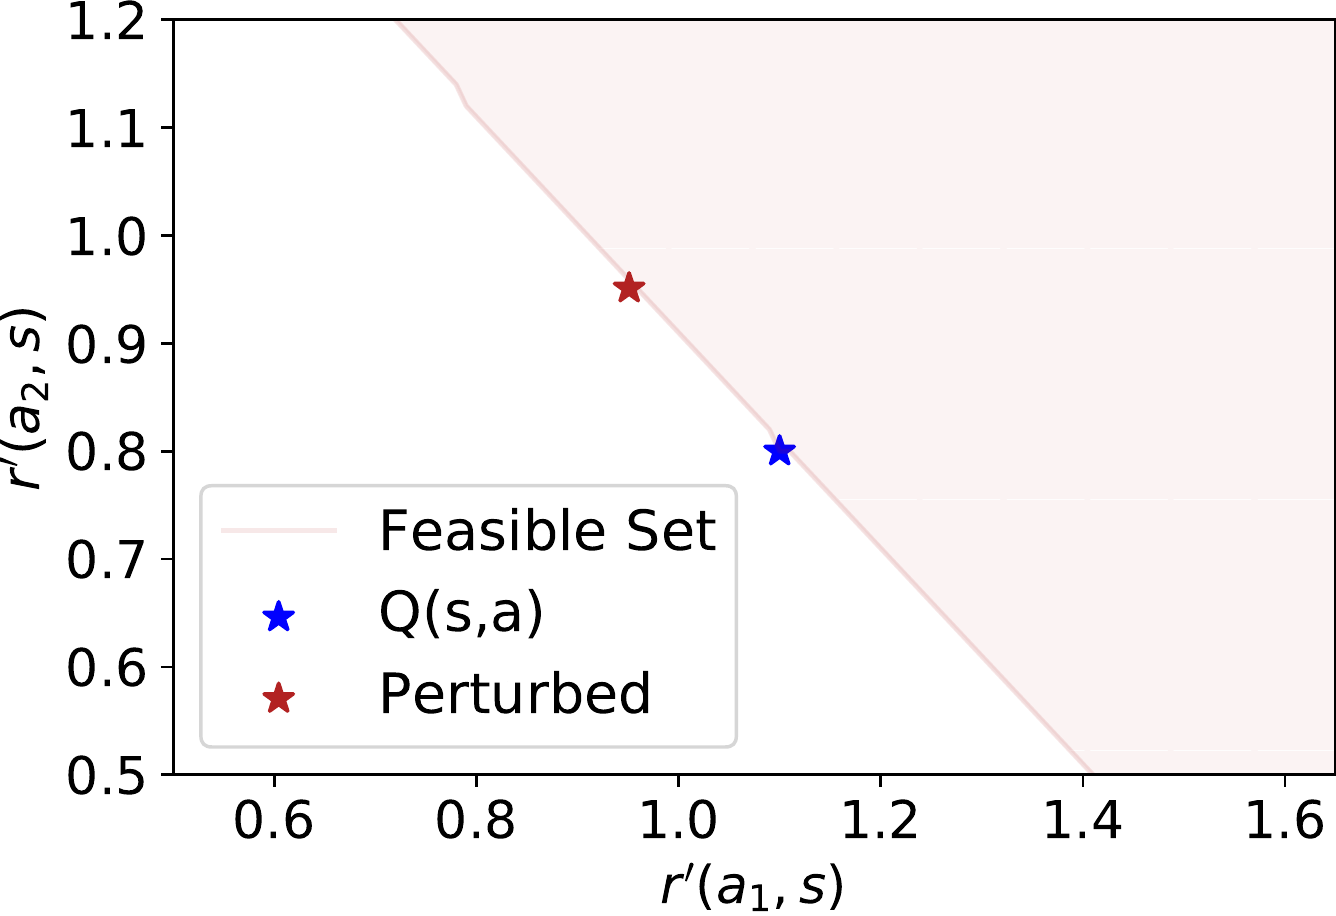}
\caption{ \centering \small $\alpha = -1, \beta = 0.1$}\end{subfigure}&
\begin{subfigure}{\mainfeasible\textwidth}\includegraphics[width=\textwidth, trim= 0 0 0 0, clip]
{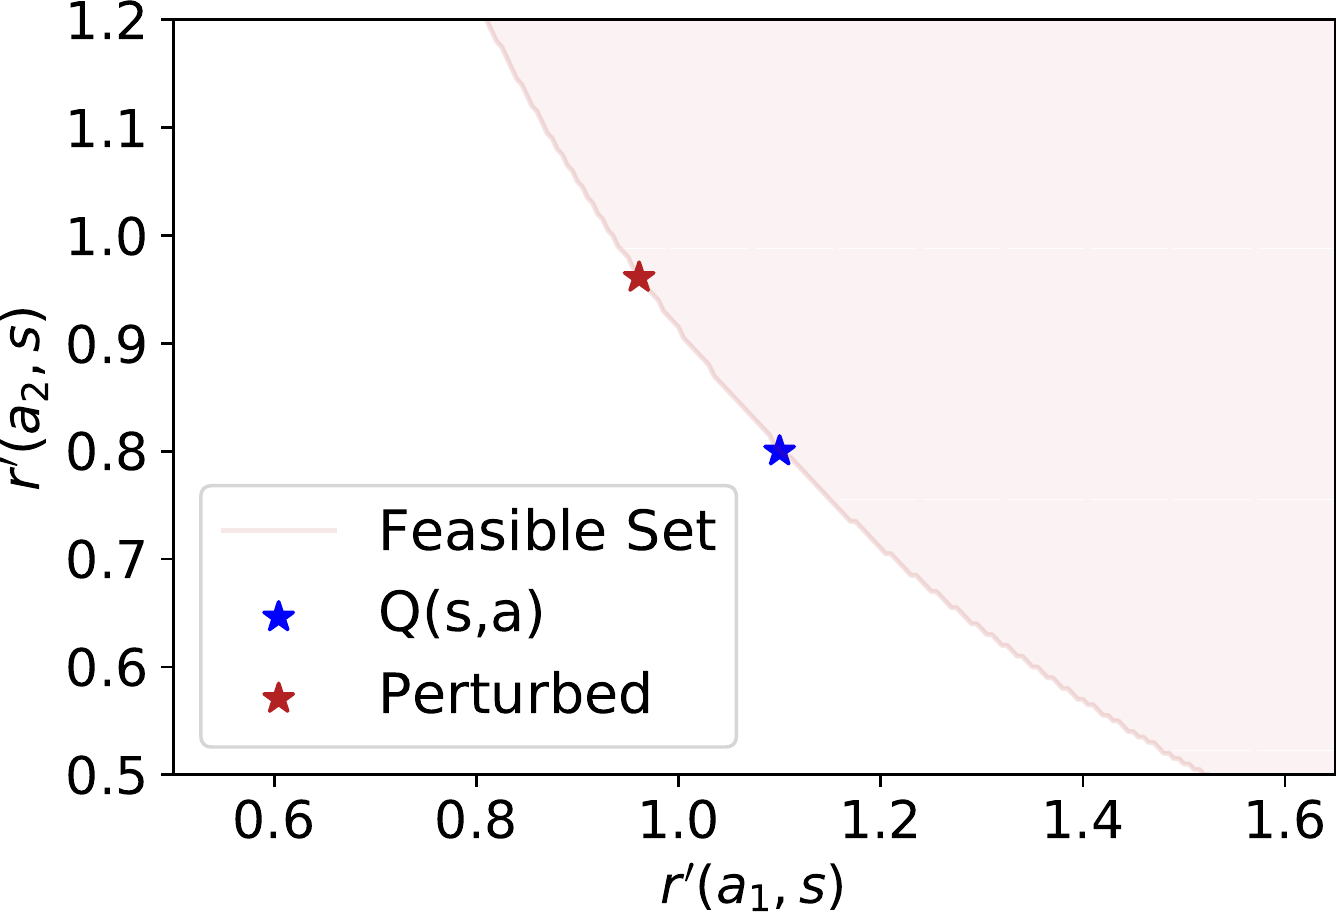}
\caption{ \centering \small $\alpha = -1, \beta = 1$}\end{subfigure} &
\begin{subfigure}{\mainfeasible\textwidth}\includegraphics[width=\textwidth, trim= 0 0 0 0, clip]
{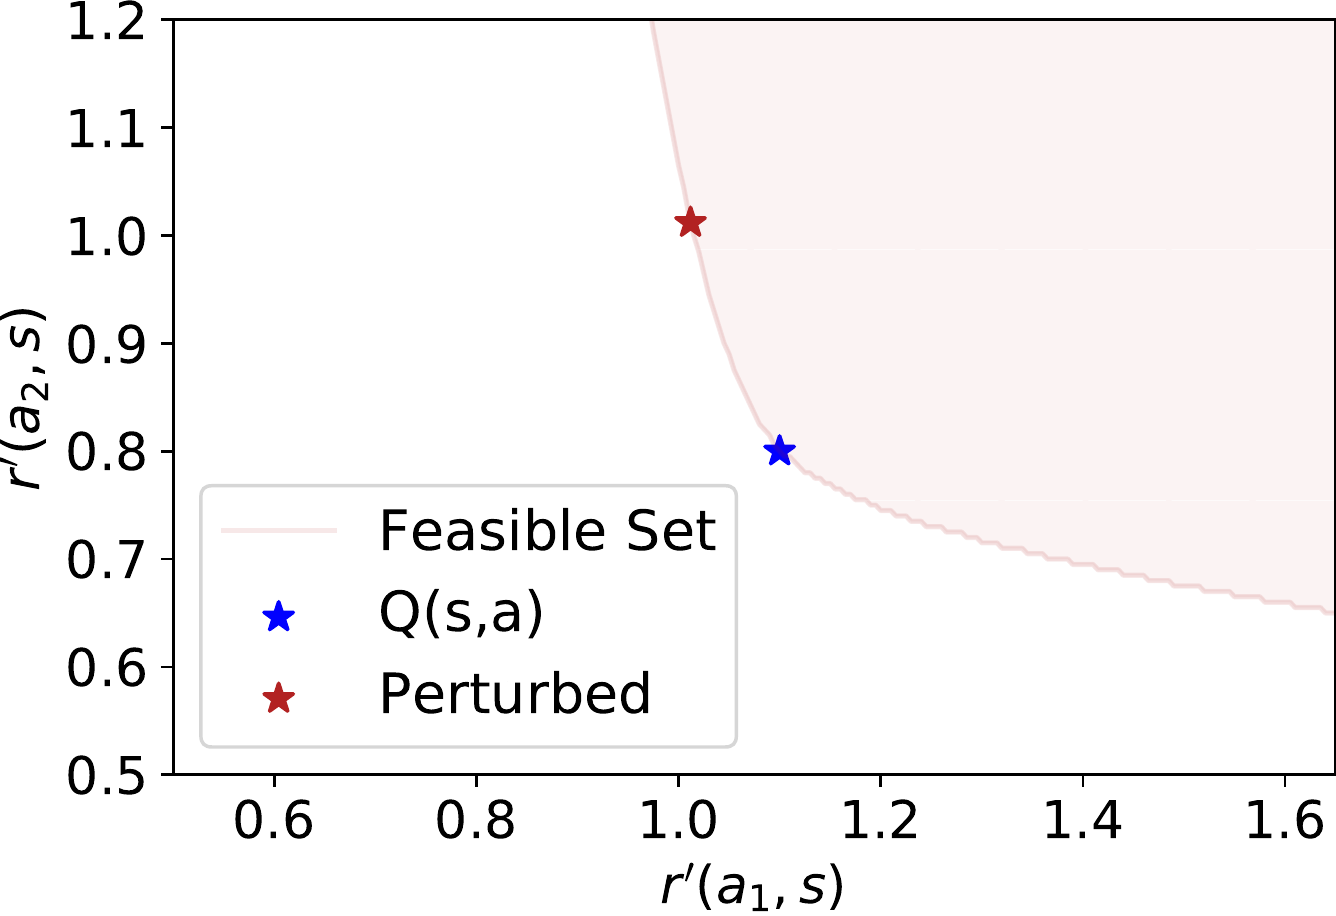}
\caption{ \centering \small $\alpha = -1, \beta = 10$}\end{subfigure} \\
 \begin{subfigure}{\sidefeasible\textwidth}  \includegraphics[width=0.9\textwidth]
 {figs/feasible/uniform_prior.png} \end{subfigure} & 
\begin{subfigure}{\mainfeasible\textwidth}\includegraphics[width=\textwidth, trim= 0 0 0 0, clip]
% {figs/feasible/kl_uniform_01.png}
{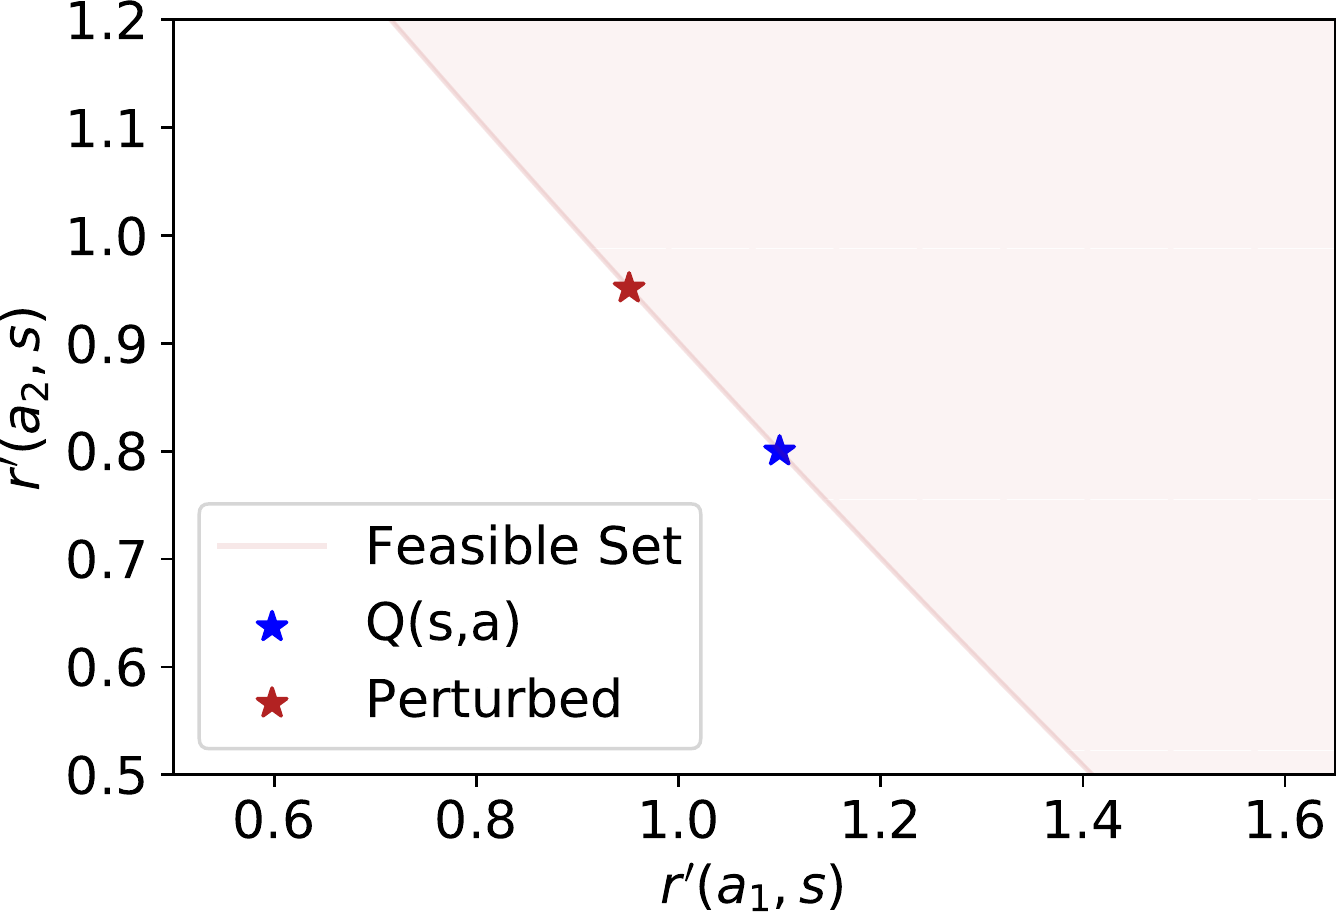}
\caption{ \centering \small $D_{KL}, \beta = 0.1$} \end{subfigure} & 
\begin{subfigure}{\mainfeasible\textwidth}\includegraphics[width=\textwidth, trim= 0 0 0 0, clip]{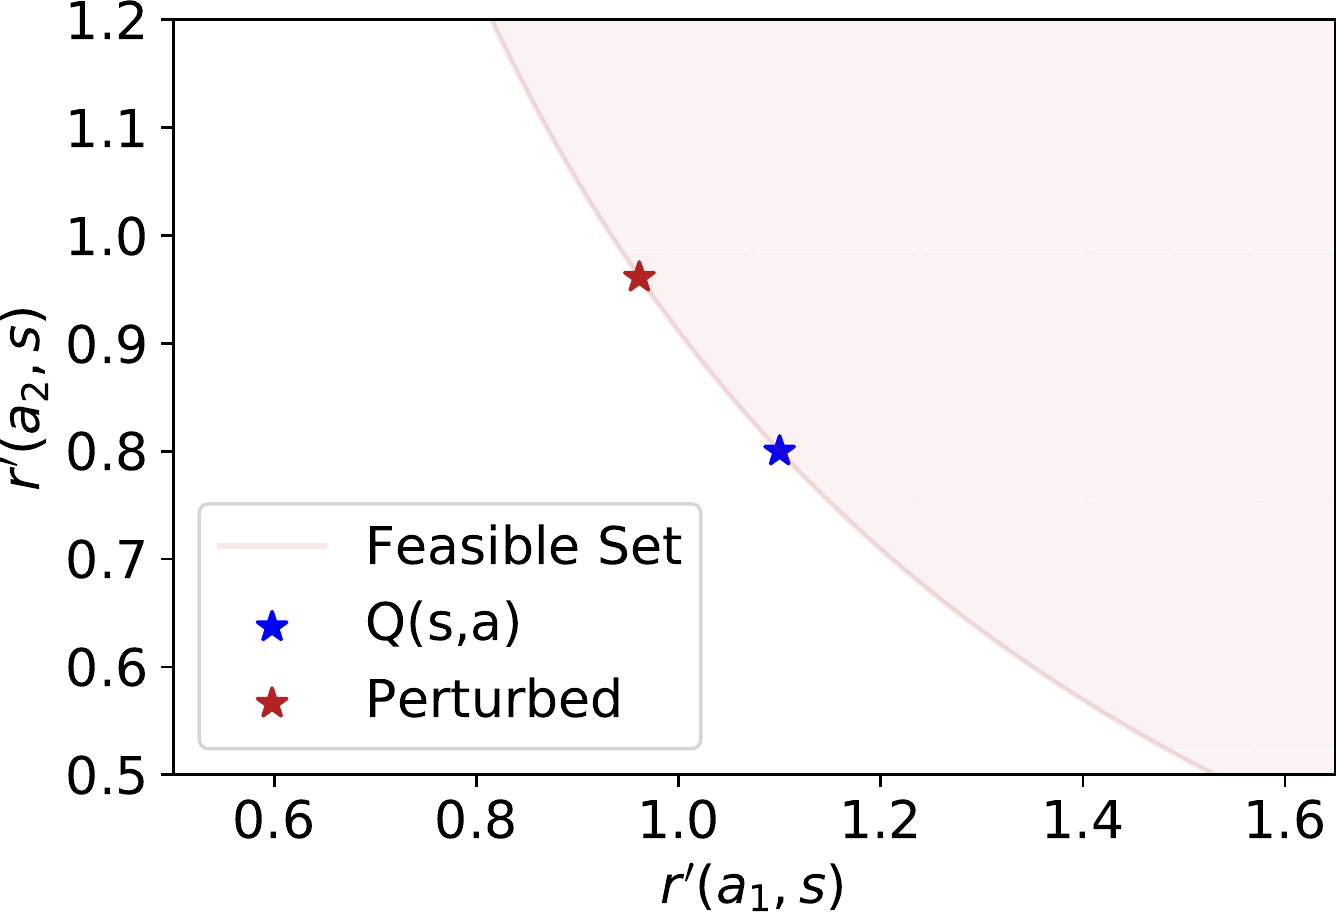}
\caption{\centering  $D_{KL}, \beta = 1$}\end{subfigure} &
\begin{subfigure}{\mainfeasible\textwidth}\includegraphics[width=\textwidth, trim= 0 0 0 0, clip]
% {figs/feasible/kl_uniform_10.png} 
{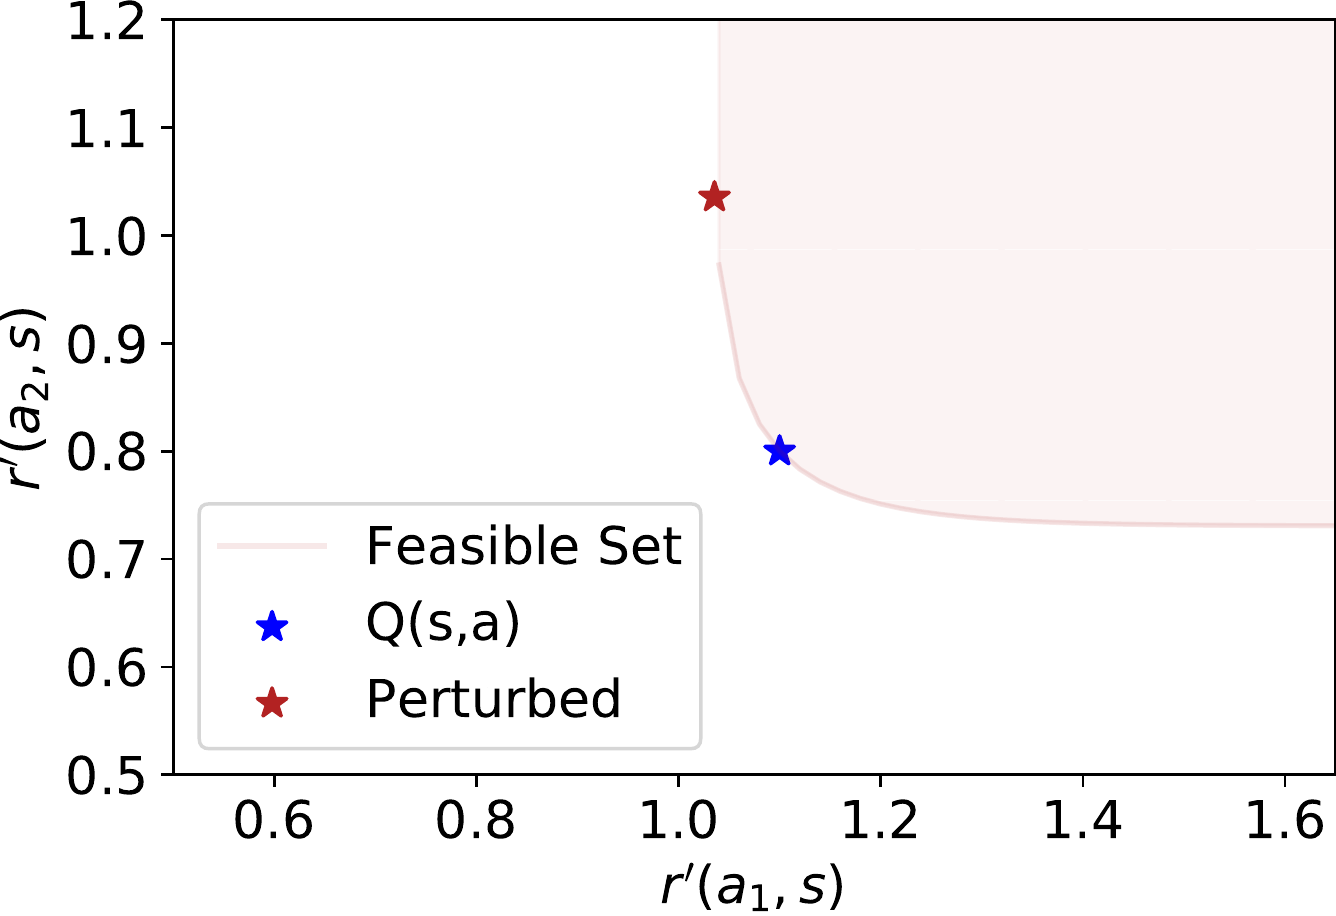}
\caption{ \centering \small $D_{KL}, \beta = 10$}\end{subfigure} \\
 \begin{subfigure}{\sidefeasible\textwidth} \phantom{ \includegraphics[width=\textwidth]
 {figs/feasible/uniform_prior.png}} \end{subfigure} & \begin{subfigure}{\mainfeasible\textwidth}\includegraphics[width=\textwidth, trim= 0 0 0 0, clip]
% {figs/feasible/alpha-1/alpha_neg1_beta1_uniform.png} 
{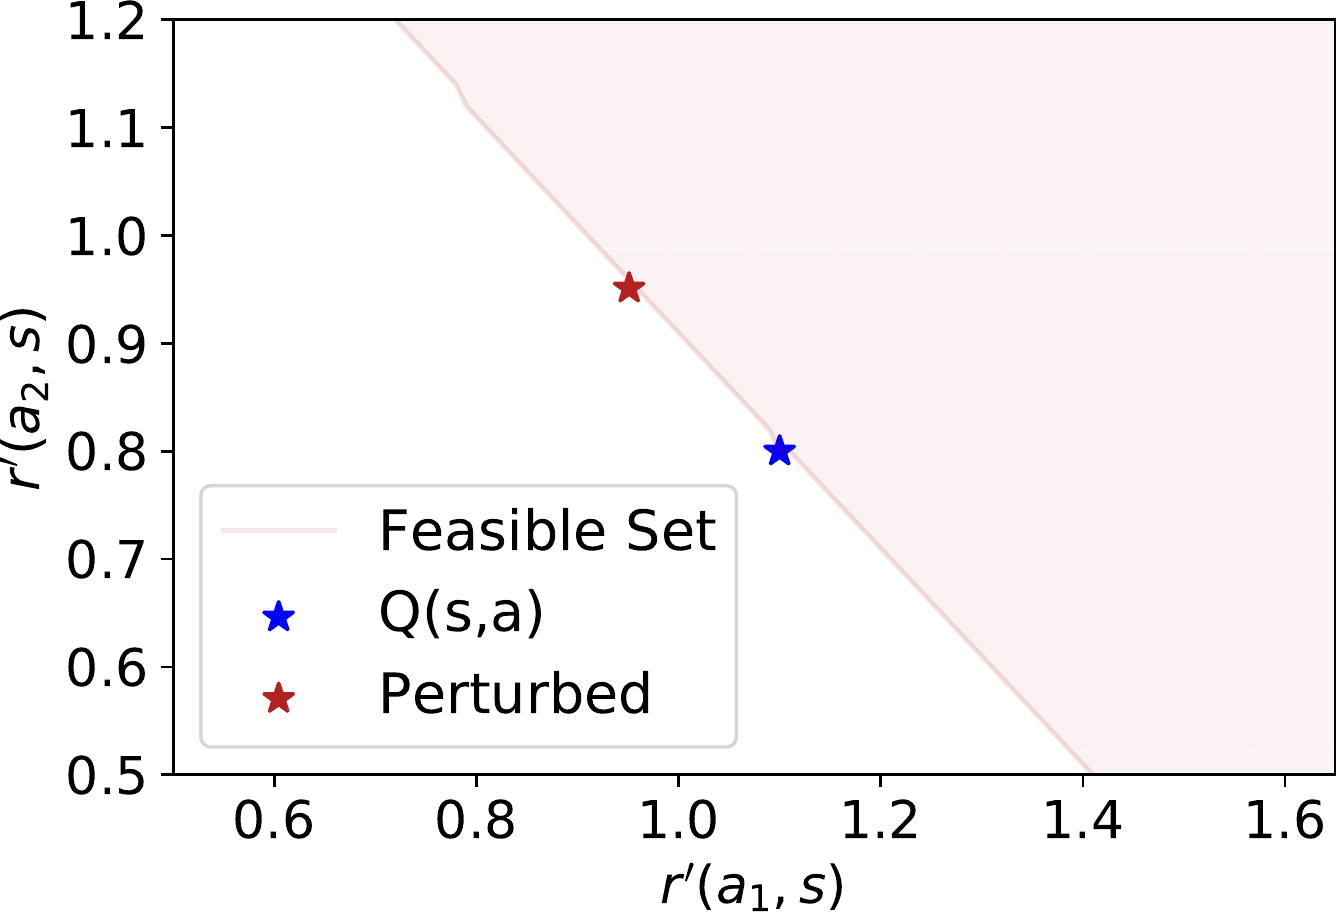}
\caption{ \centering \small $\alpha = 2, \beta = 0.1$}\end{subfigure}&
\begin{subfigure}{\mainfeasible\textwidth}\includegraphics[width=\textwidth, trim= 0 0 0 0, clip]
{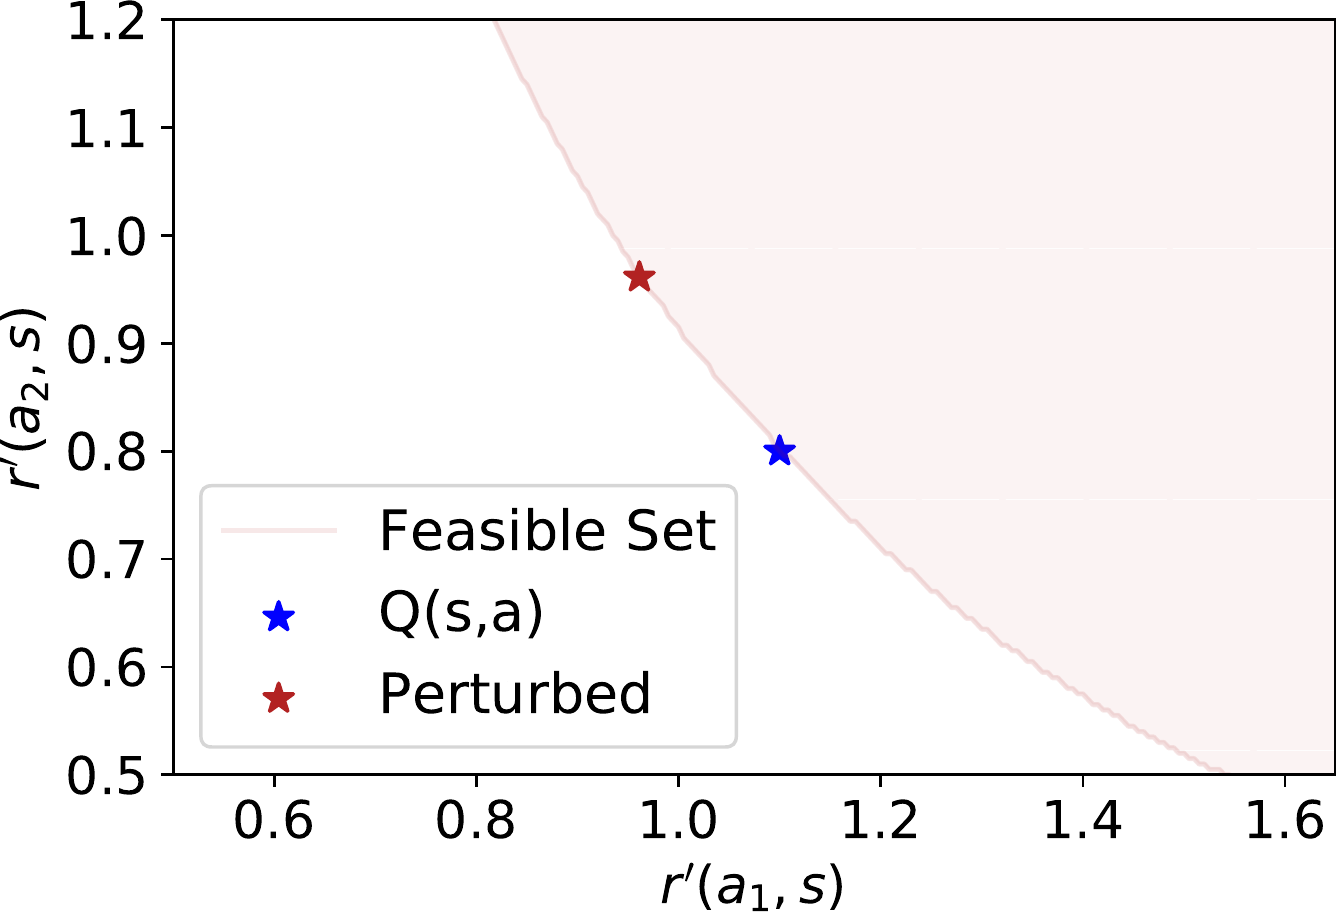}
\caption{ \centering \small $\alpha = 2, \beta = 1$}\end{subfigure}&
\begin{subfigure}{\mainfeasible\textwidth}\includegraphics[width=\textwidth, trim= 0 0 0 0, clip]
{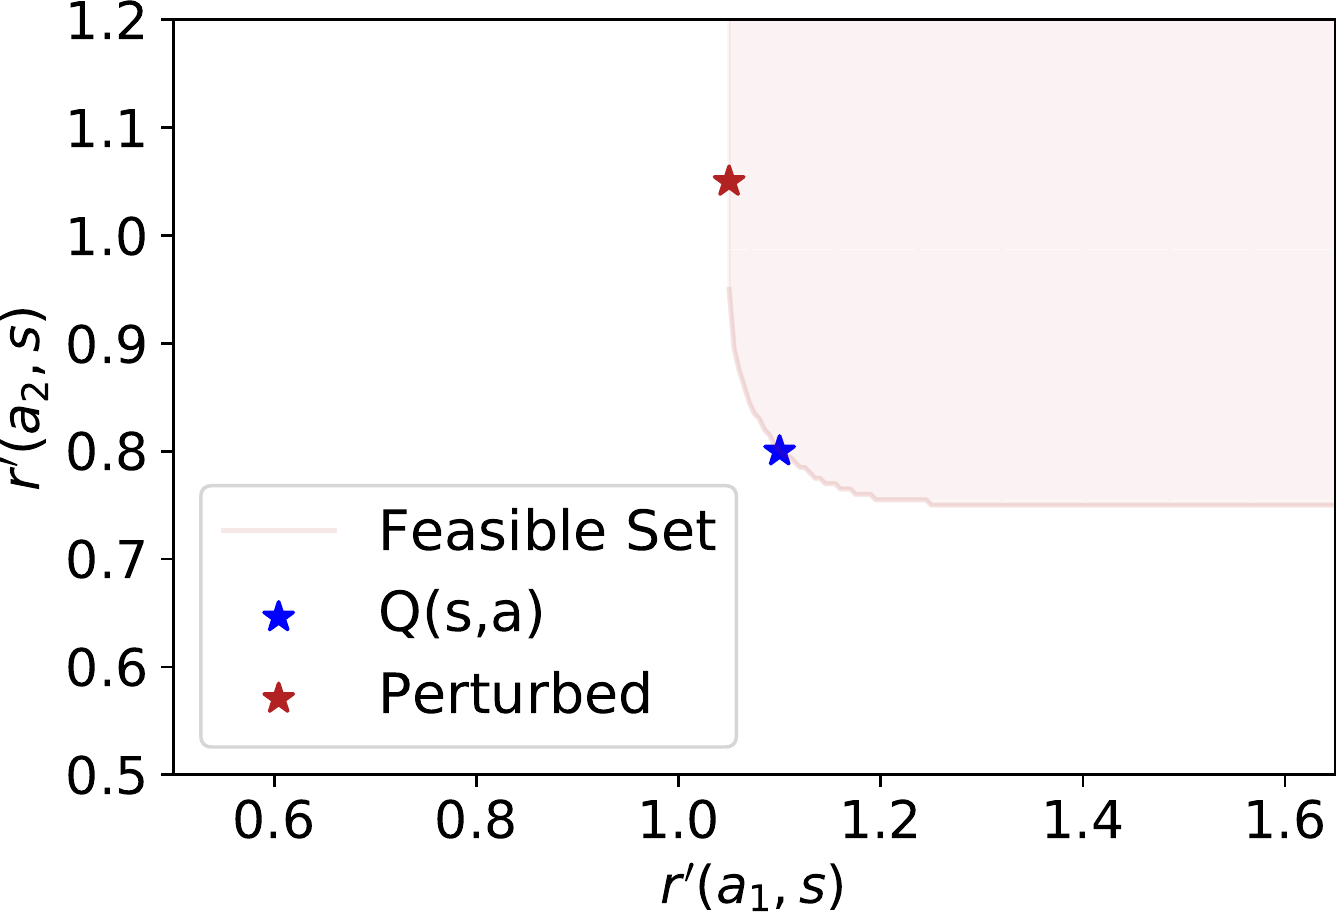}
\caption{ \centering \small $\alpha = 2, \beta = 10$}\end{subfigure} \\
\begin{subfigure}{\sidefeasible\textwidth} \phantom{ \includegraphics[width=\textwidth]
 {figs/feasible/uniform_prior.png}} \end{subfigure} & \begin{subfigure}{\mainfeasible\textwidth}\includegraphics[width=\textwidth, trim= 0 0 0 0, clip]
% {figs/feasible/alpha-1/alpha_neg1_beta1_uniform.png} 
{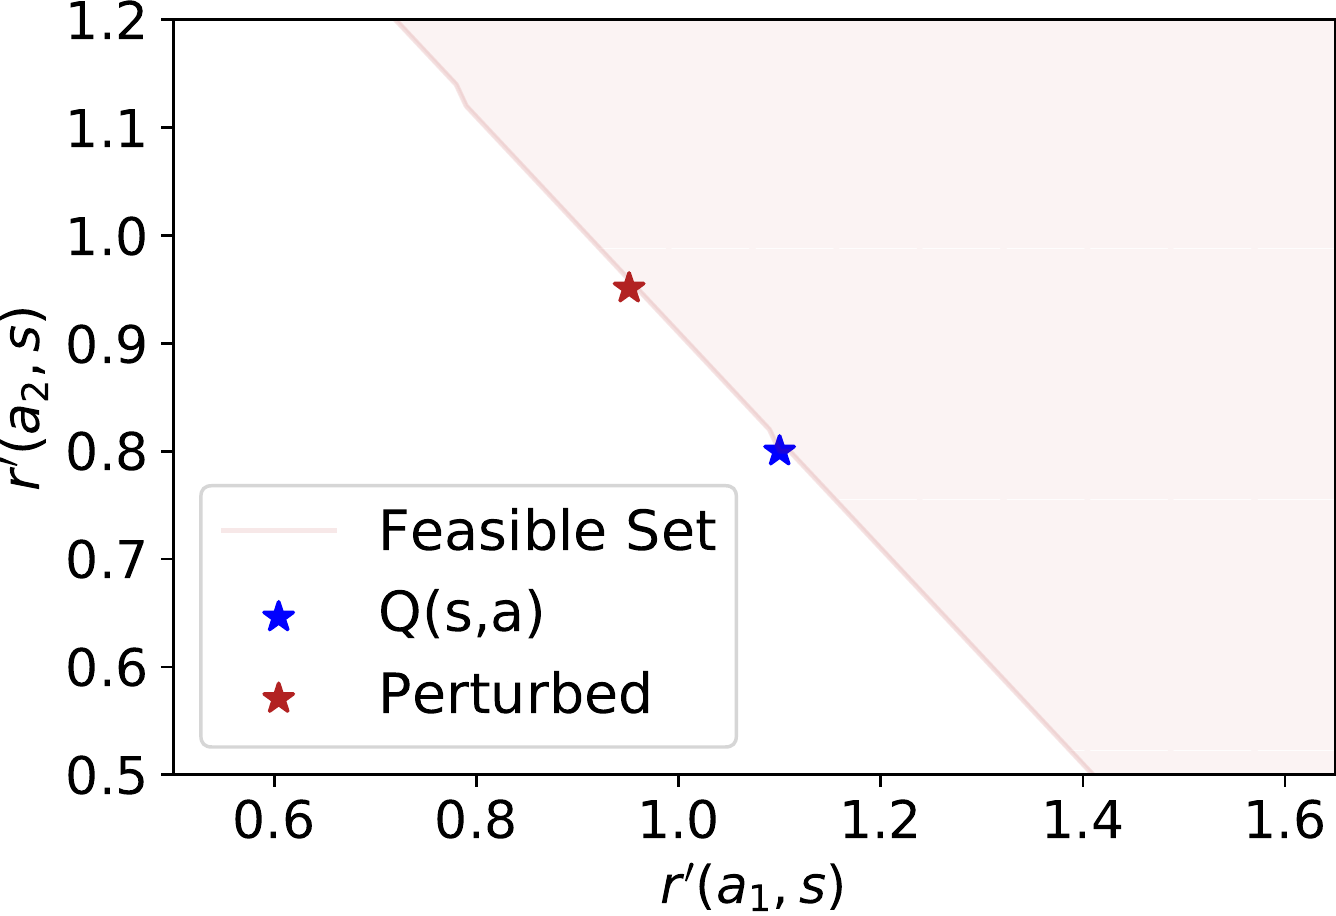}
\caption{\centering \small $\alpha = 3, \beta = 0.1$}\end{subfigure}&
\begin{subfigure}{\mainfeasible\textwidth}\includegraphics[width=\textwidth, trim= 0 0 0 0, clip]
{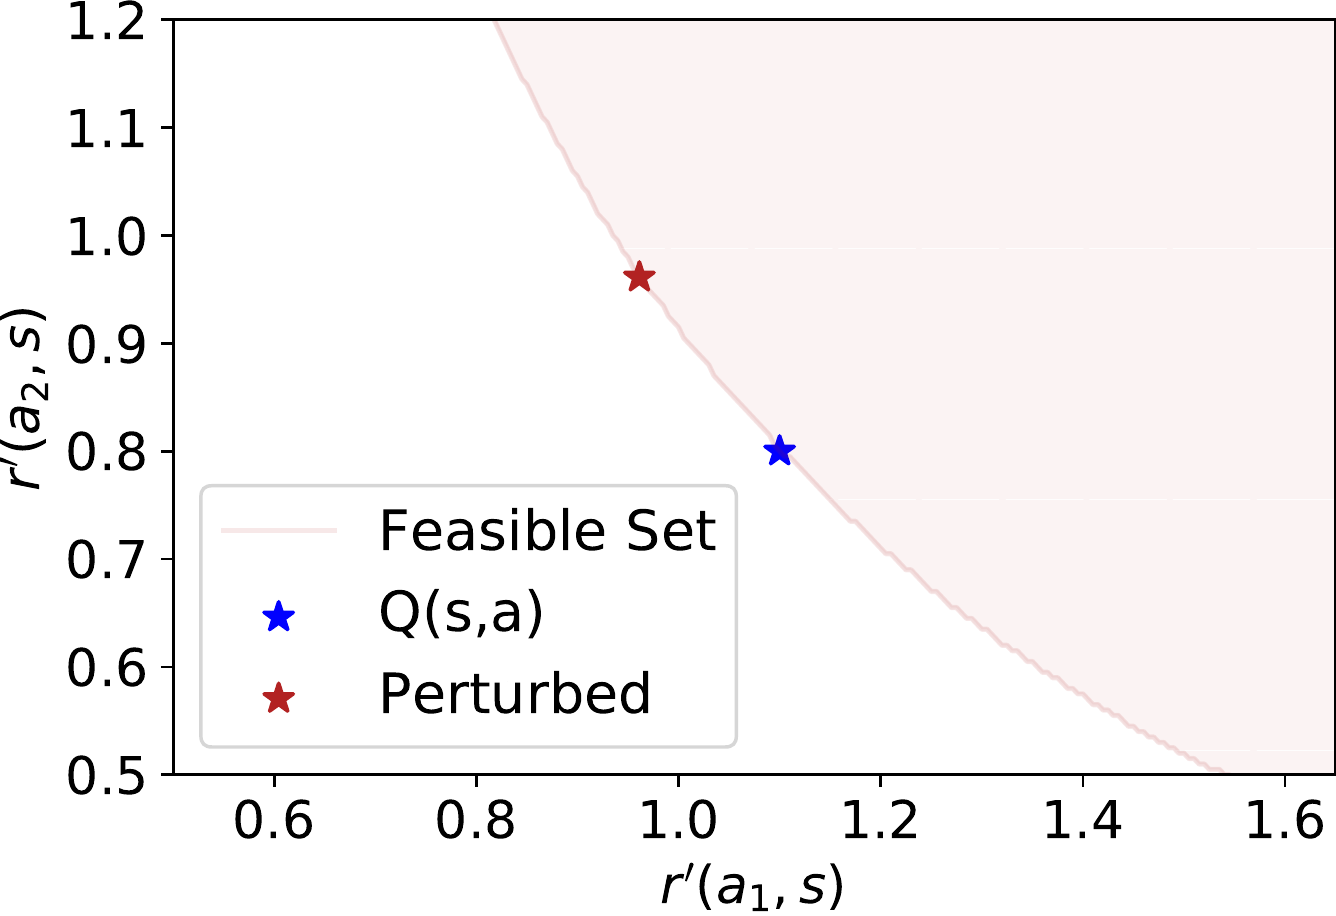}
\caption{ \centering \small $\alpha = 3, \beta = 1$}\end{subfigure}&
\begin{subfigure}{\mainfeasible\textwidth}\includegraphics[width=\textwidth, trim= 0 0 0 0, clip]
{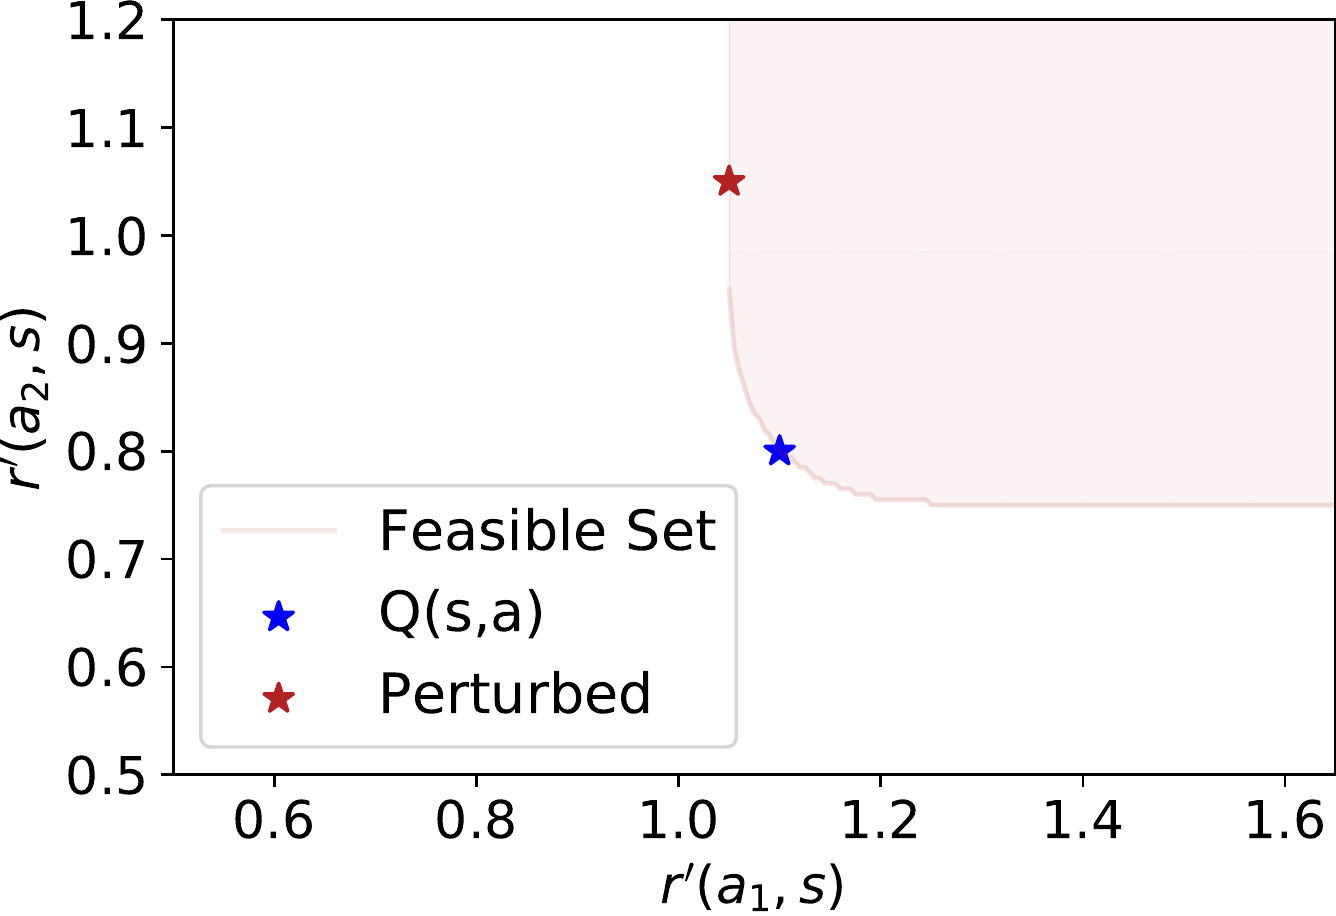}
\caption{ \centering \small $\alpha = 3, \beta = 10$}\end{subfigure}
\\ %&\hspace*{.2cm}\\
% \begin{subfigure}{\sidefeasible\textwidth}\vspace*{-.24cm} \includegraphics[width=\textwidth]{figs/feasible/nonuniform_prior.png}\end{subfigure}& %\qquad \hspace*{.2cm}
% \begin{subfigure}{\mainfeasible\textwidth}\includegraphics[width=\textwidth, trim= 5 0 5 0, clip]
% % {figs/feasible/kl_73_01.png}
% {figs/feasible/kl/beta01alpha1nonuniform.pdf}
% \caption{\label{fig:tabd} \centering \small $D_{KL}, \beta = 0.1$}\end{subfigure}& %\qquad \hspace*{.2cm}
% \begin{subfigure}{\mainfeasible\textwidth}\includegraphics[width=\textwidth, trim= 5 0 5 0, clip]
% % {figs/feasible/kl_73_1.png}
% {figs/feasible/kl/beta1alpha1nonuniform.pdf}
% \caption{\label{fig:tabe} \centering \small $D_{KL}, \beta = 1$}\end{subfigure}& %\qquad \hspace*{.2cm}
% \begin{subfigure}{\mainfeasible\textwidth}\includegraphics[width=\textwidth, trim= 5 0 5 0, clip]
% % {figs/feasible/kl_73_10.png} 
% {figs/feasible/kl/beta10alpha1nonuniform.pdf}
% \caption{\label{fig:tabf} \centering \small $D_{KL}, \beta = 10$}\end{subfigure}
\end{array}
\] 
\end{center}
% \end{minipage}
\caption{Feasible Set (red region) of rewards available to the adversary, for \textsc{kl} divergence (at various $\beta$) and $\alpha$-divergence ($\alpha=\{-1, 1, 2, 3\}$) regularization and fixed $Q_*(a,s) = r(a,s)$ values (blue star).  Red star indicates optimal perturbed reward $\mrpiopt = r - \prpiopt$, for the optimal $\pi_*(a|s)$ associated with regularization parameters $\alpha, \beta, \pi_0$ and the given $Q$-values.
% (see \cref{eq:alpha_opt_policy} and (\ref{eq:kl_opt_policy})). 
Top row:  reference distribution $\pi_0=(\frac{1}{2},\frac{1}{2})$, bottom row: $\pi_0 = (\frac{2}{3}, \frac{1}{3})$.  
% Red dot indicates $Q(a,s)$ associated with policy $\pi(a|s)$
}\label{fig:feasible_set_uniform_app}
\end{figure*}

\begin{figure*}[!t]
\centering
% \begin{minipage}{\textwidth}%{0.8\textwidth}
% \centering
\begin{center}
\[\arraycolsep=.01\textwidth
\begin{array}{cccc} %[width=40mm]
 \begin{subfigure}{\sidefeasible\textwidth}  \phantom{ \includegraphics[width=\textwidth]
 {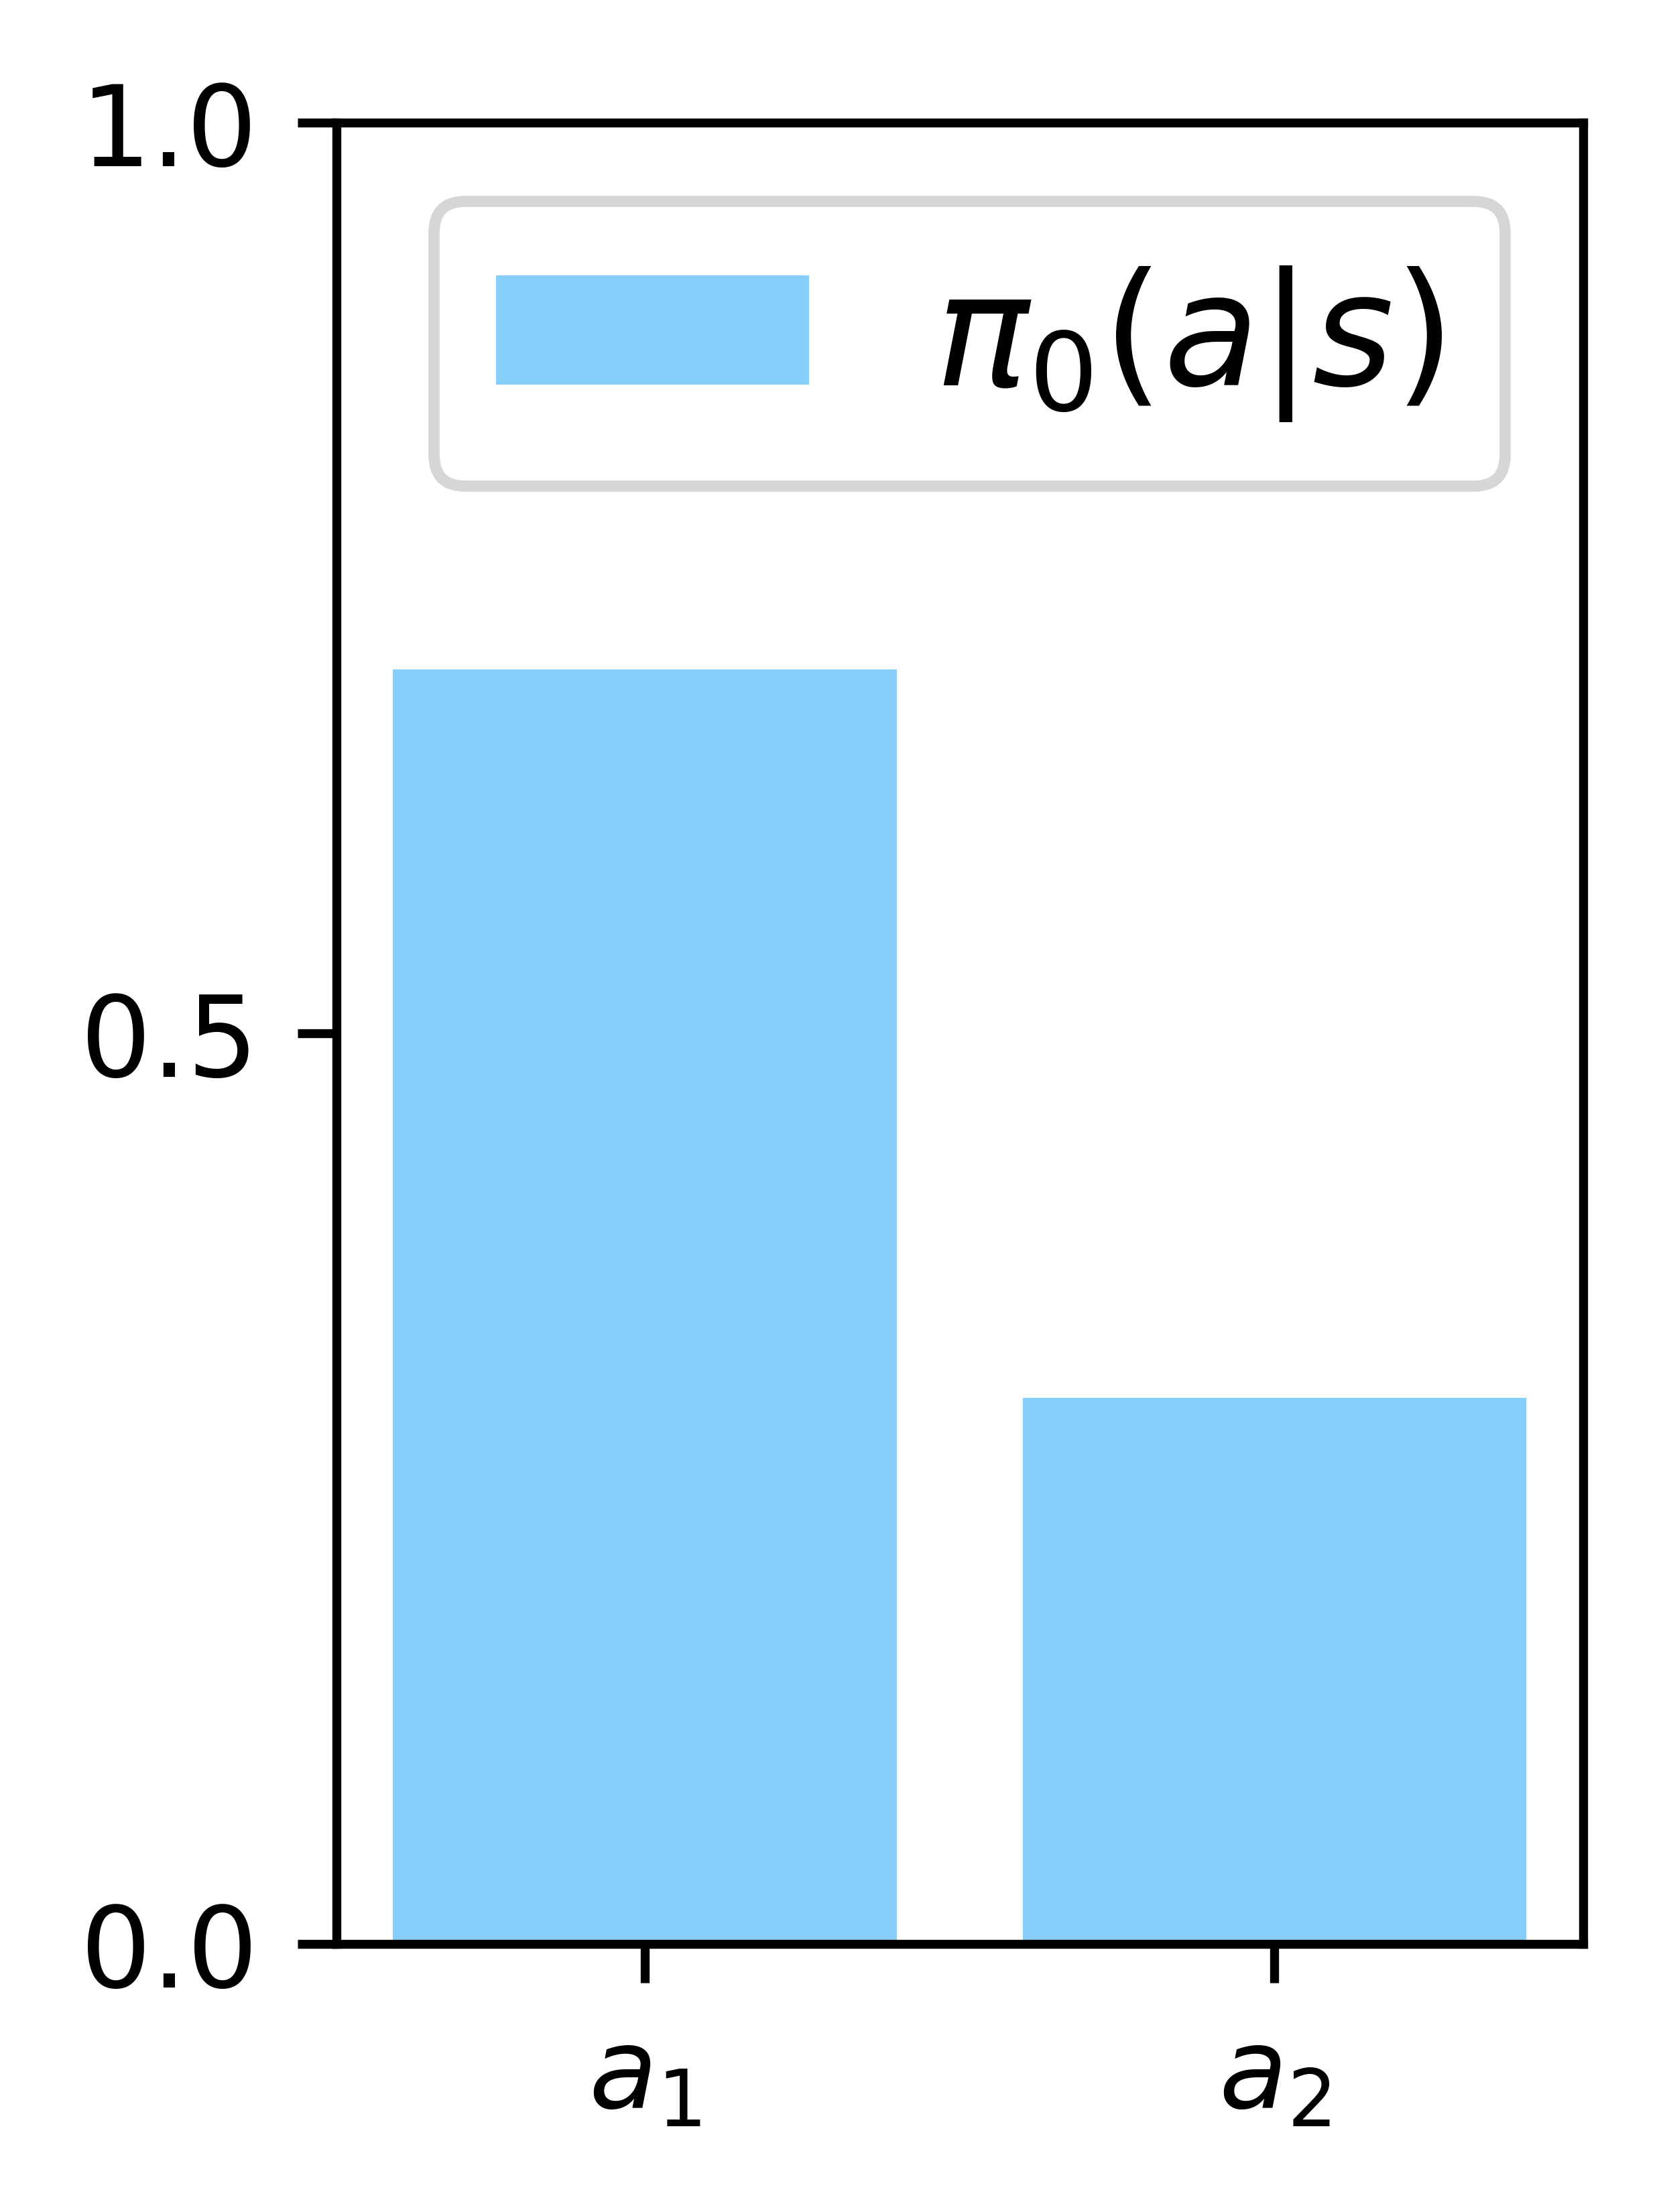}} \end{subfigure} & \begin{subfigure}{\mainfeasible\textwidth}\includegraphics[width=\textwidth, trim= 0 0 0 0, clip]
% {figs/feasible/alpha-1/alpha_neg1_beta1_uniform.png} 
{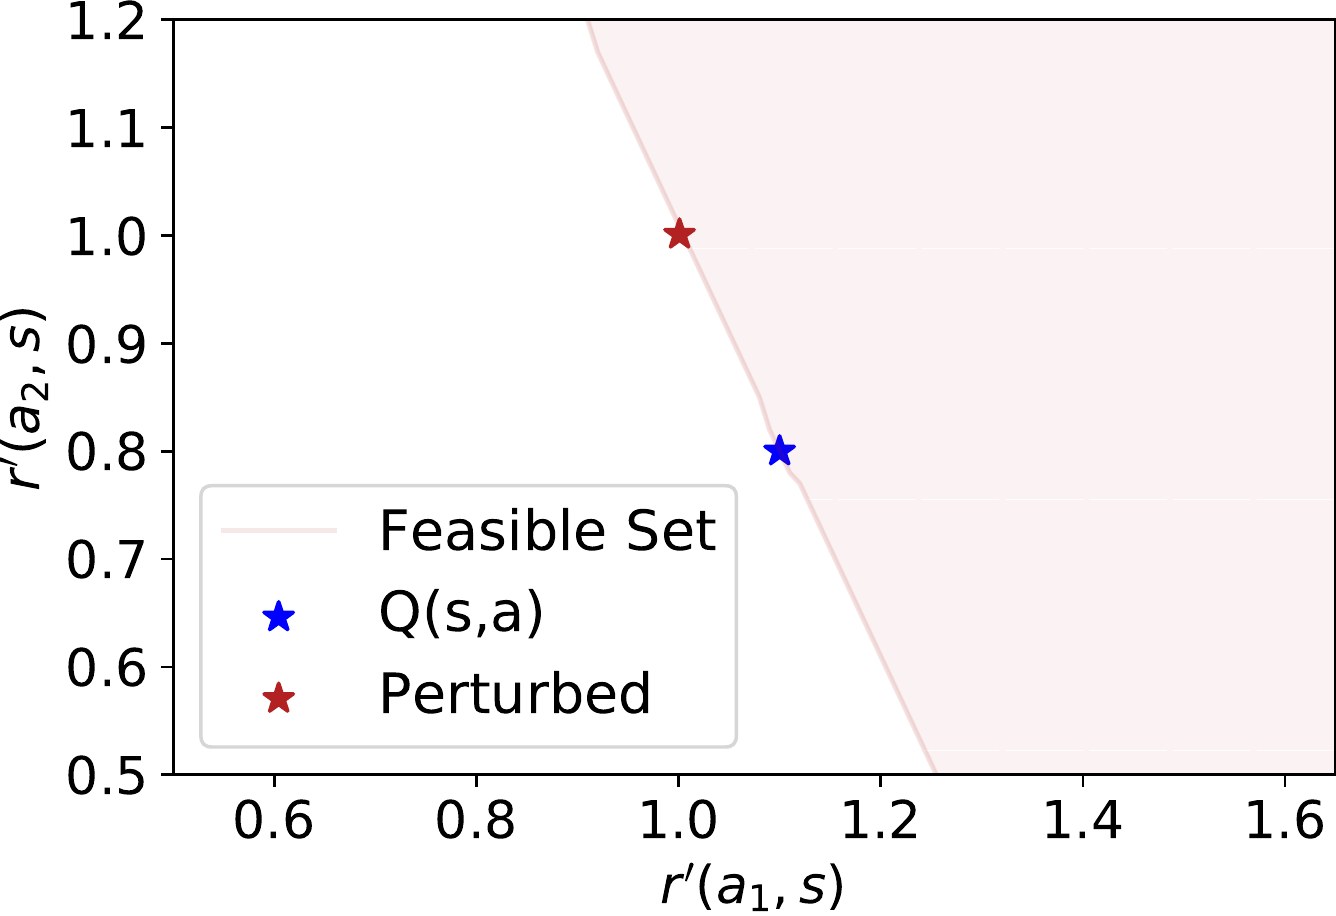}
\caption{ \centering \small $\alpha = -1, \beta = 0.1$}\end{subfigure}&
\begin{subfigure}{\mainfeasible\textwidth}\includegraphics[width=\textwidth, trim= 0 0 0 0, clip]
{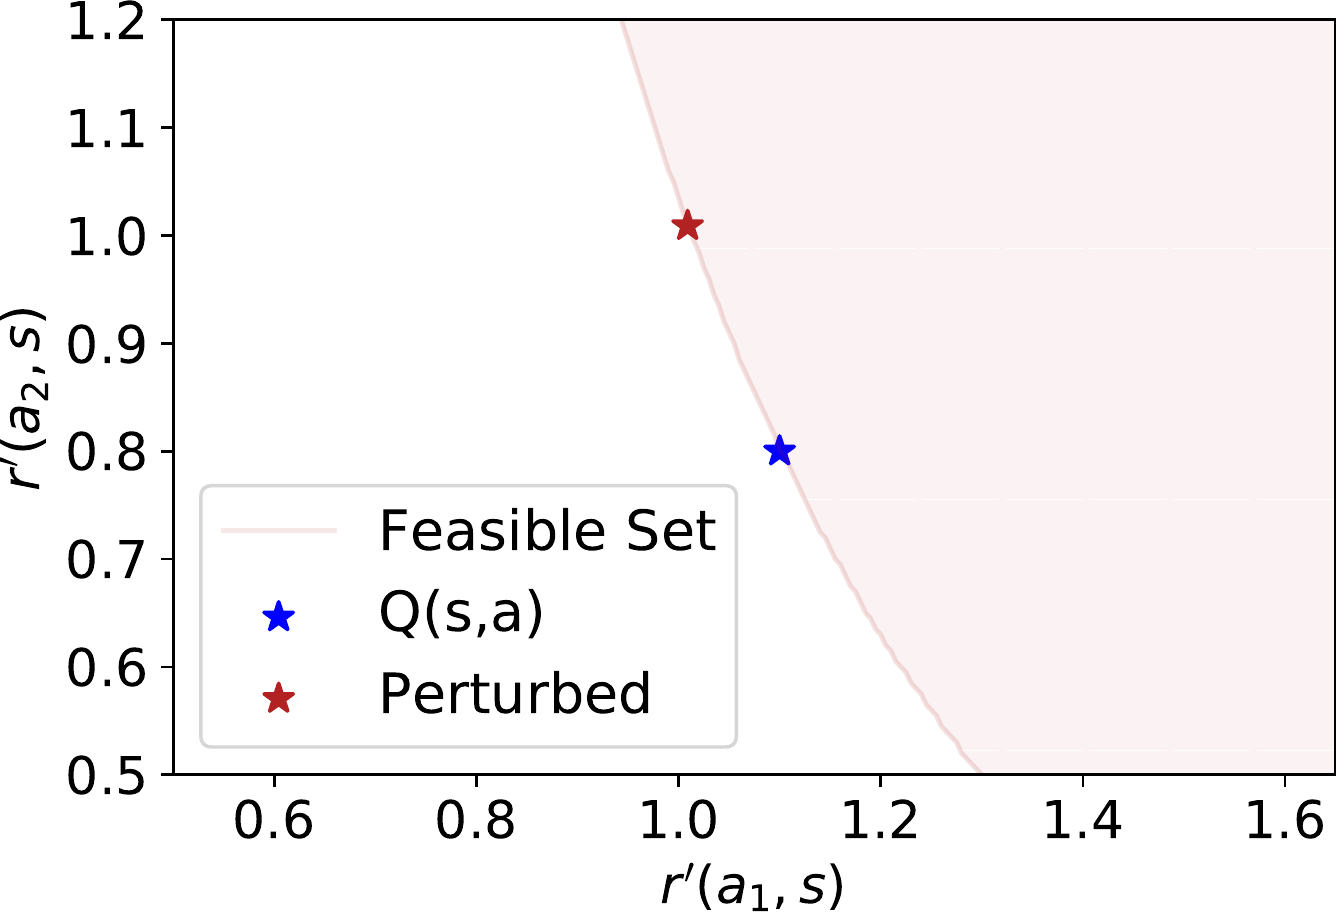}
\caption{ \centering \small $\alpha = -1, \beta = 1$}\end{subfigure} &
\begin{subfigure}{\mainfeasible\textwidth}\includegraphics[width=\textwidth, trim= 0 0 0 0, clip]
{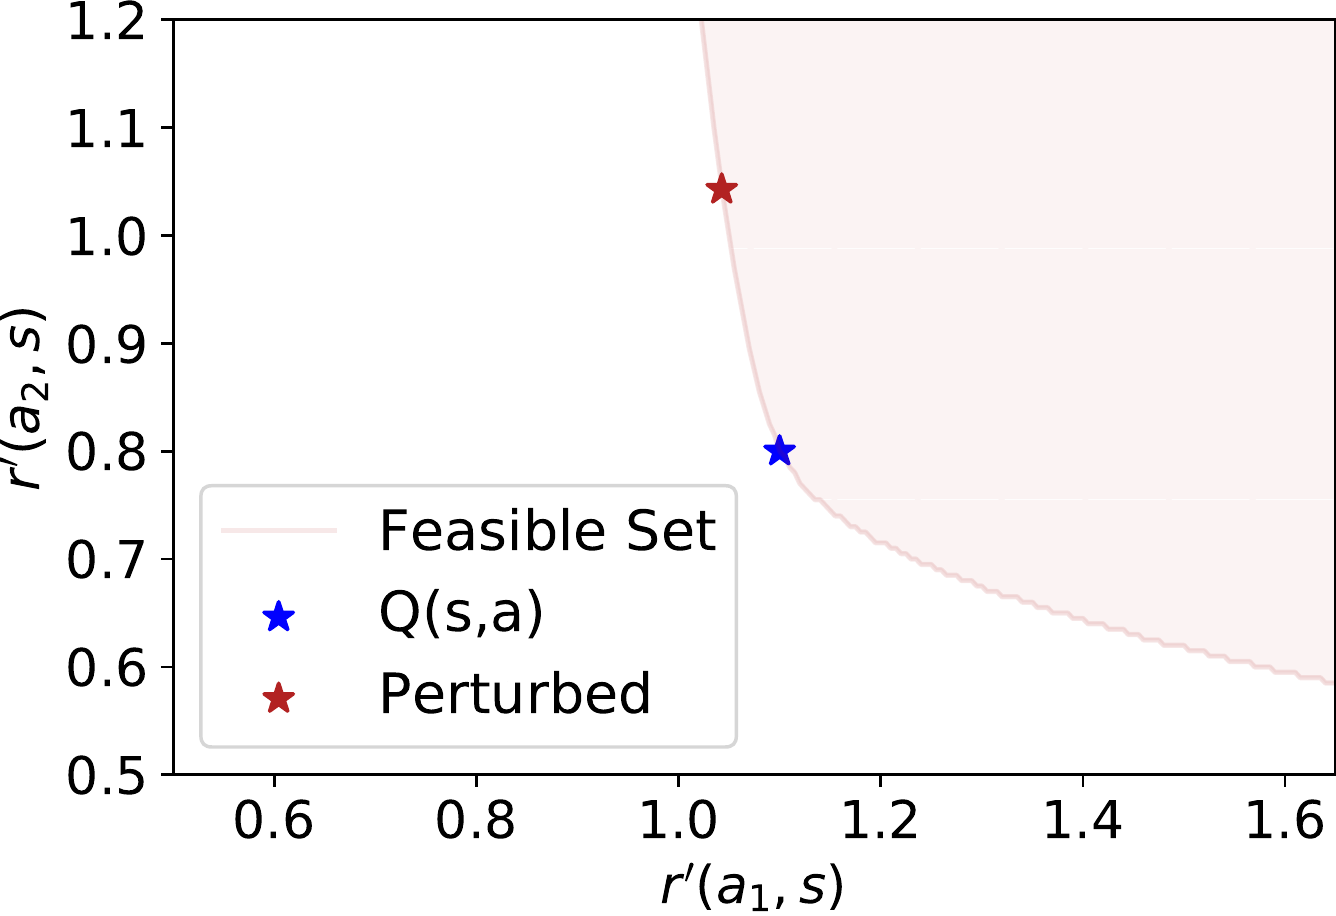}
\caption{ \centering \small $\alpha = -1, \beta = 10$}\end{subfigure} \\
 \begin{subfigure}{\sidefeasible\textwidth}  \includegraphics[width=0.9\textwidth]
 {figs/feasible/nonuniform_prior.png} \end{subfigure} & 
\begin{subfigure}{\mainfeasible\textwidth}\includegraphics[width=\textwidth, trim= 0 0 0 0, clip]
% {figs/feasible/kl_uniform_01.png}
{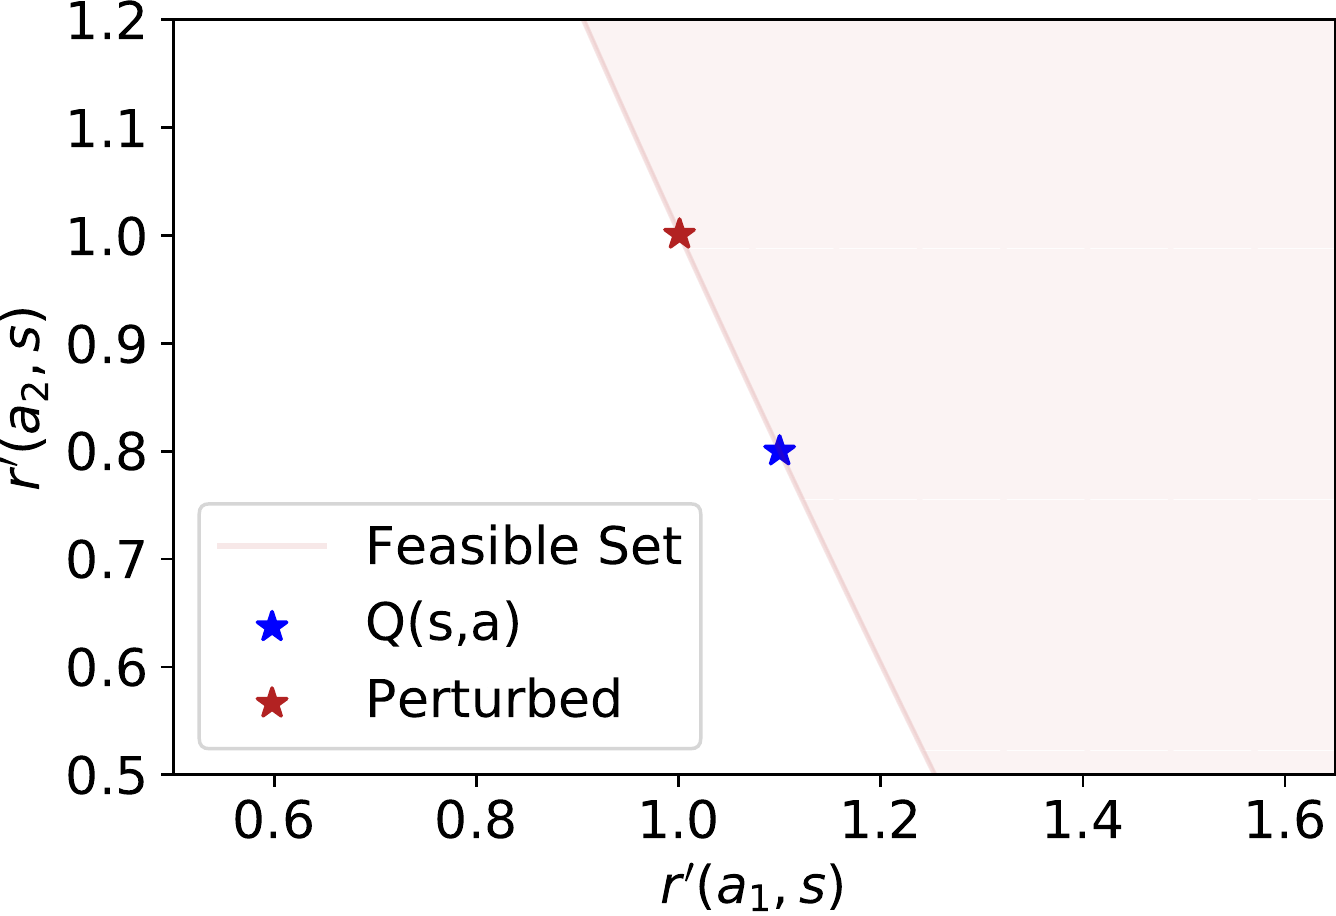}
\caption{ \centering \small $D_{KL}, \beta = 0.1$} \end{subfigure} & 
\begin{subfigure}{\mainfeasible\textwidth}\includegraphics[width=\textwidth, trim= 0 0 0 0, clip]{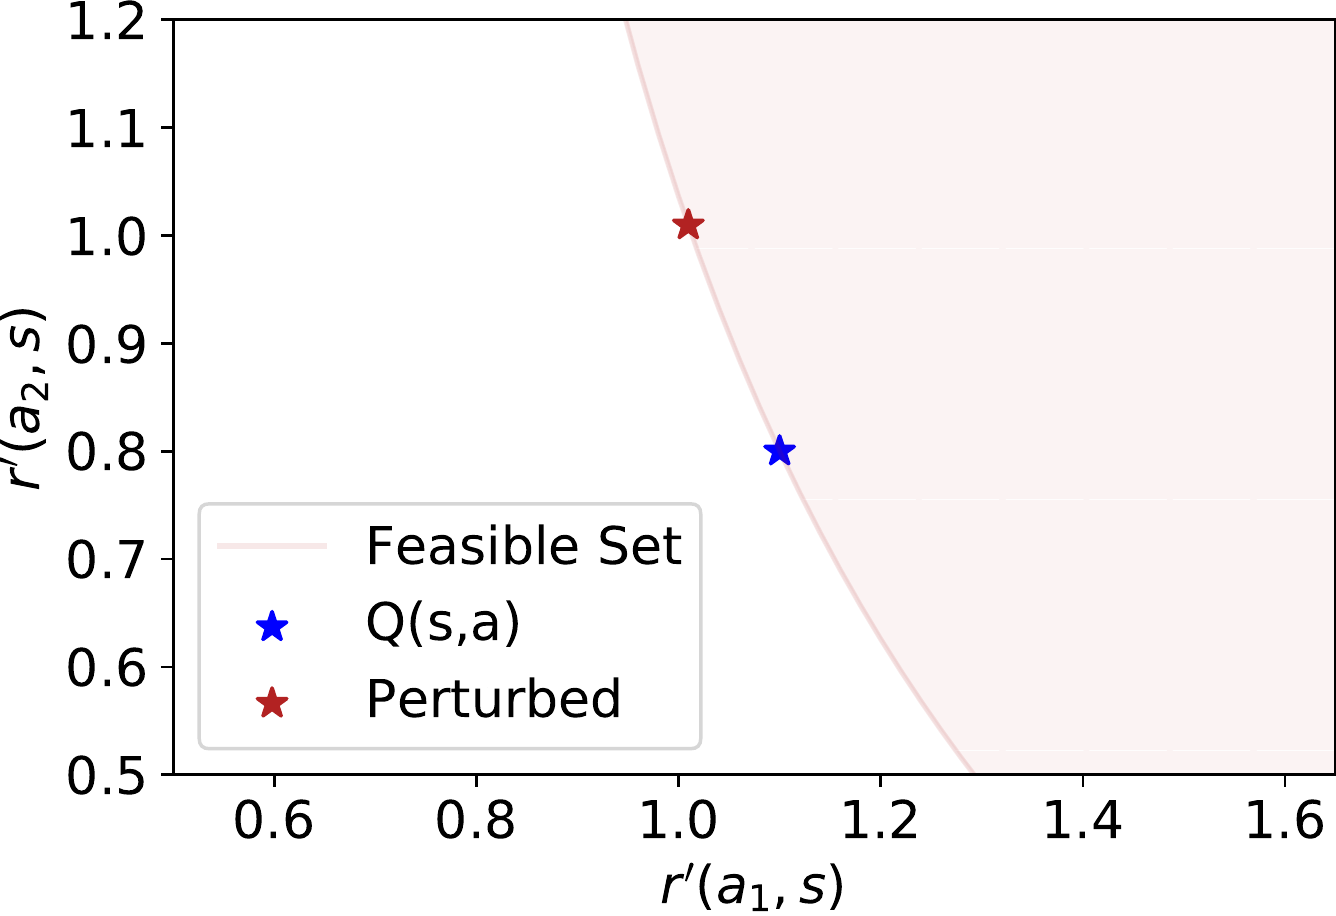}
\caption{ \centering  $D_{KL}, \beta = 1$}\end{subfigure} &
\begin{subfigure}{\mainfeasible\textwidth}\includegraphics[width=\textwidth, trim= 5 0 5 0, clip]
% {figs/feasible/kl_uniform_10.png} 
{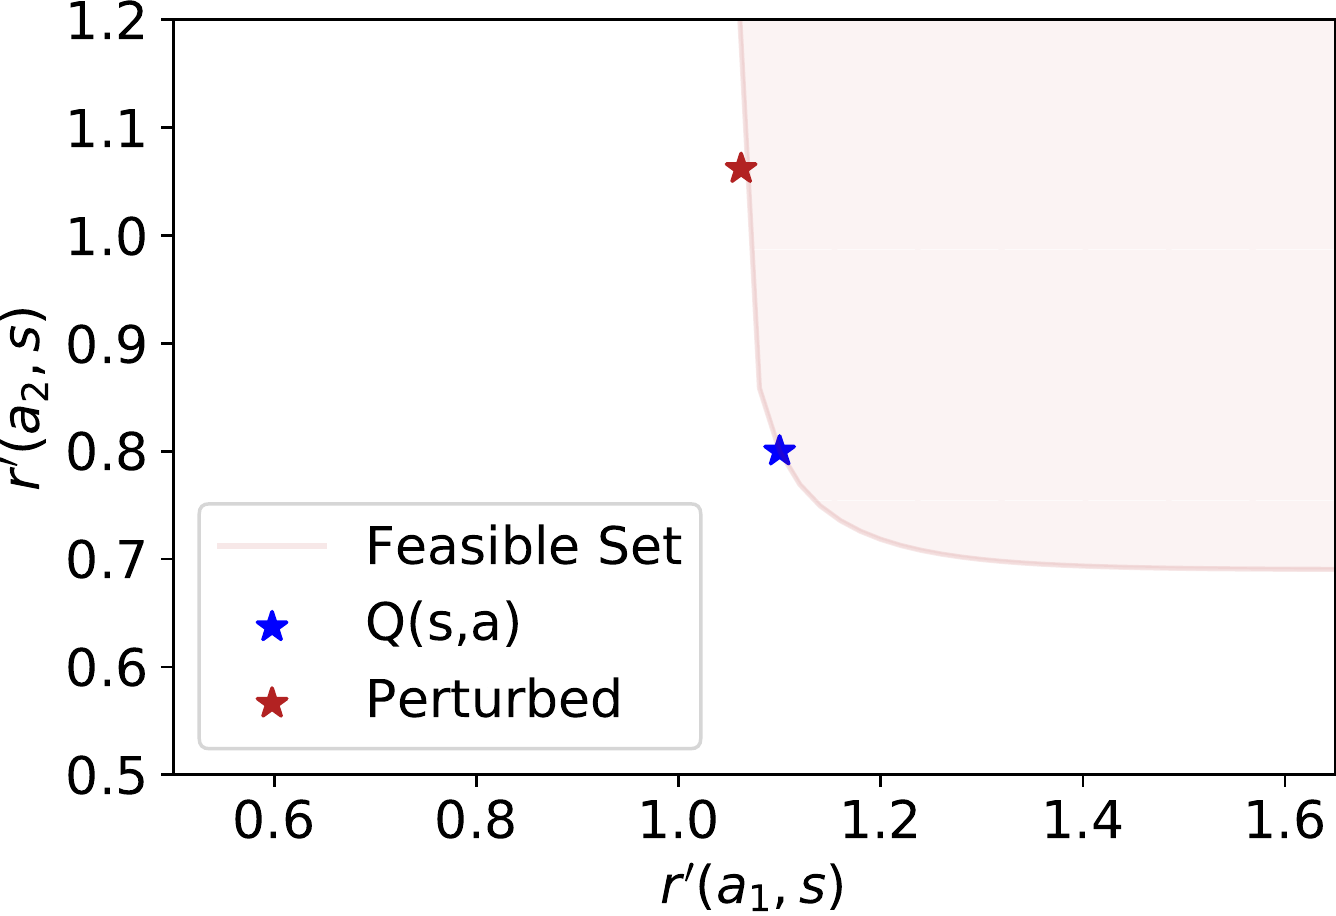}
\caption{ \centering \small $D_{KL}, \beta = 10$}\end{subfigure} \\
 \begin{subfigure}{\sidefeasible\textwidth} \phantom{ \includegraphics[width=\textwidth]
 {figs/feasible/nonuniform_prior.png}} \end{subfigure} & \begin{subfigure}{\mainfeasible\textwidth}\includegraphics[width=\textwidth, trim= 0 0 0 0, clip]
% {figs/feasible/alpha-1/alpha_neg1_beta1_uniform.png} 
{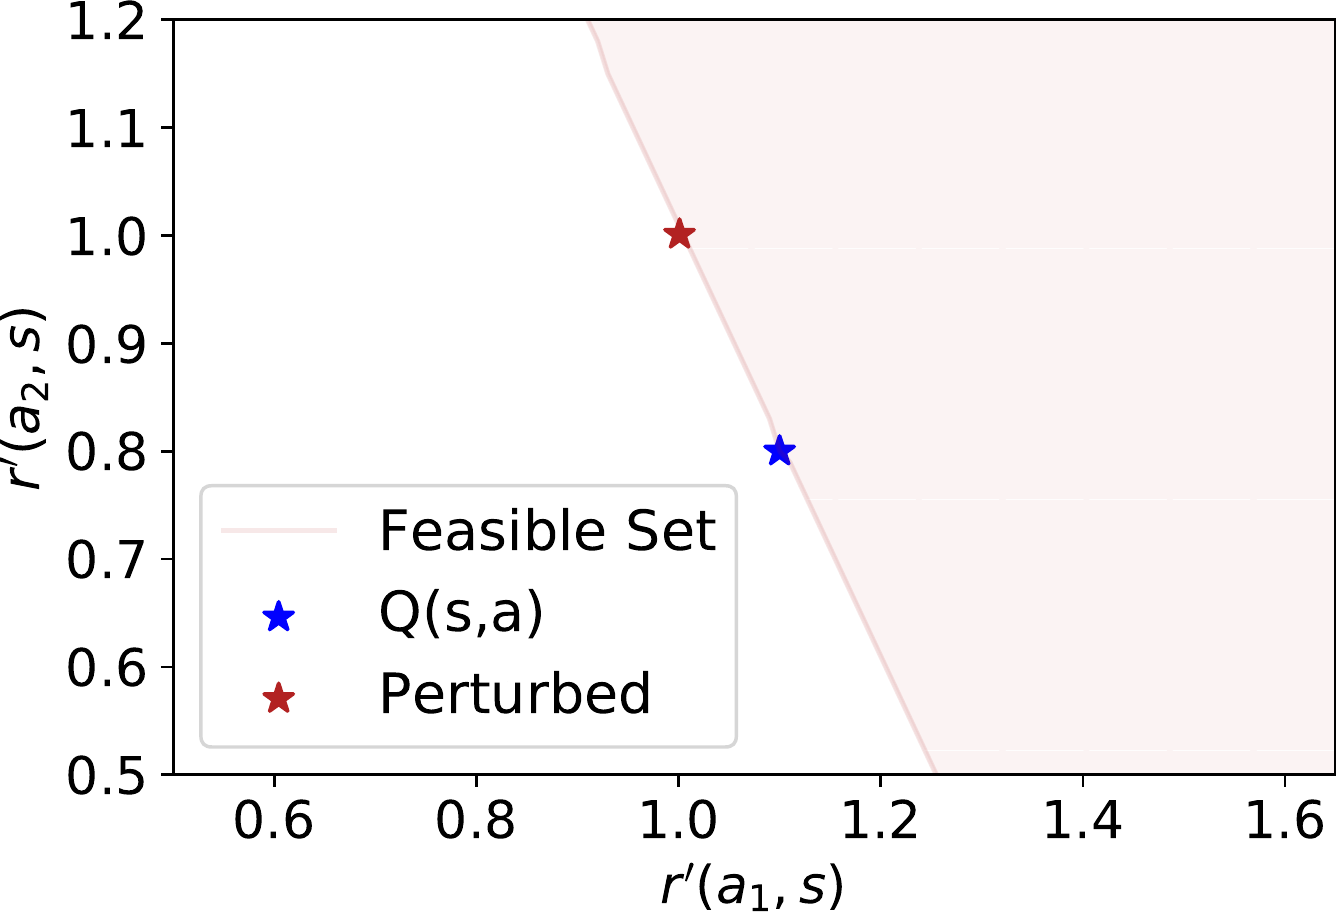}
\caption{ \centering \small $\alpha = 2, \beta = 0.1$}\end{subfigure}&
\begin{subfigure}{\mainfeasible\textwidth}\includegraphics[width=\textwidth, trim= 0 0 0 0, clip]
{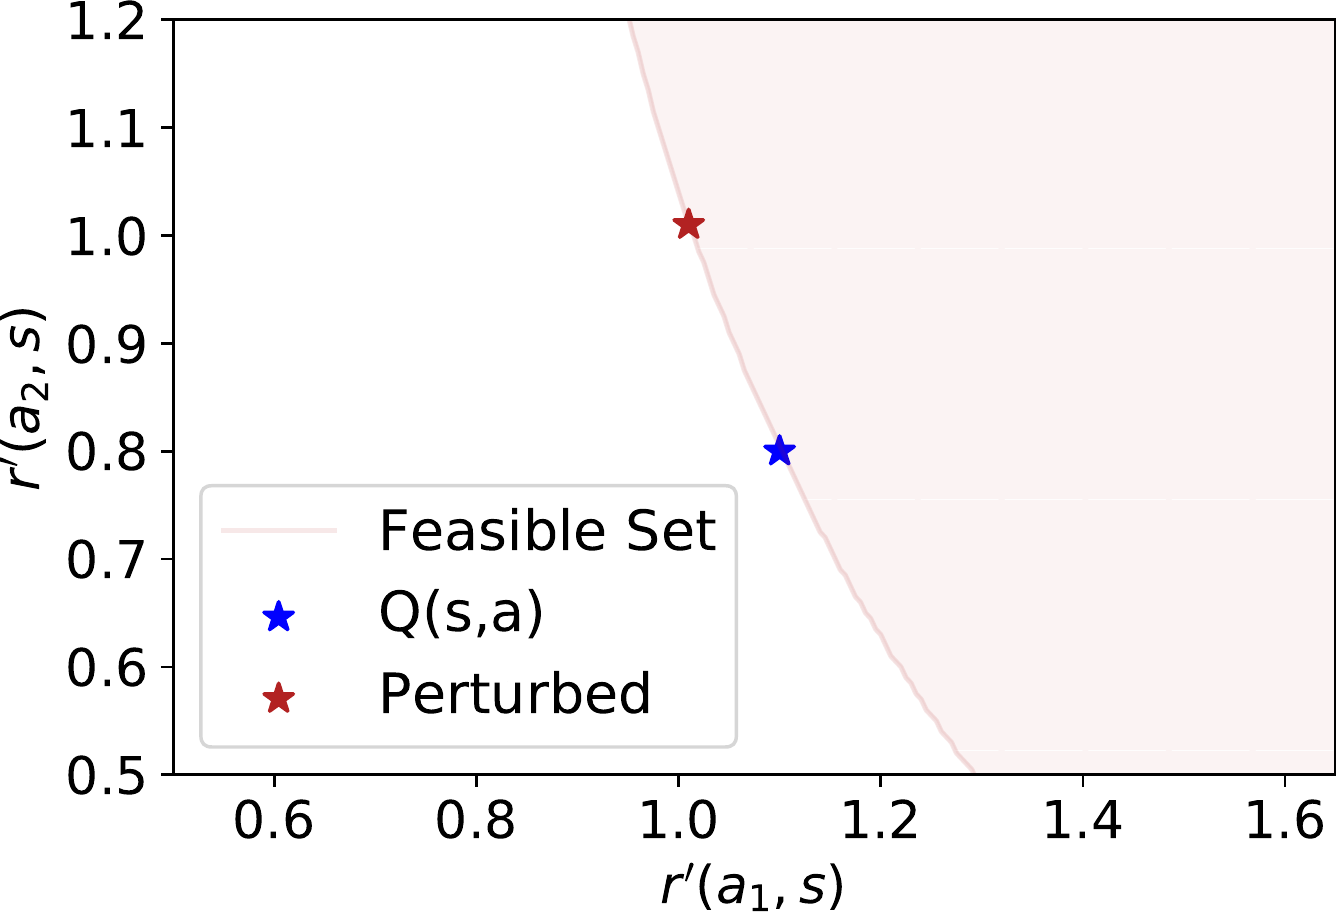}
\caption{ \centering \small $\alpha = 2, \beta = 1$}\end{subfigure} &
\begin{subfigure}{\mainfeasible\textwidth}\includegraphics[width=\textwidth, trim= 0 0 0 0, clip]
{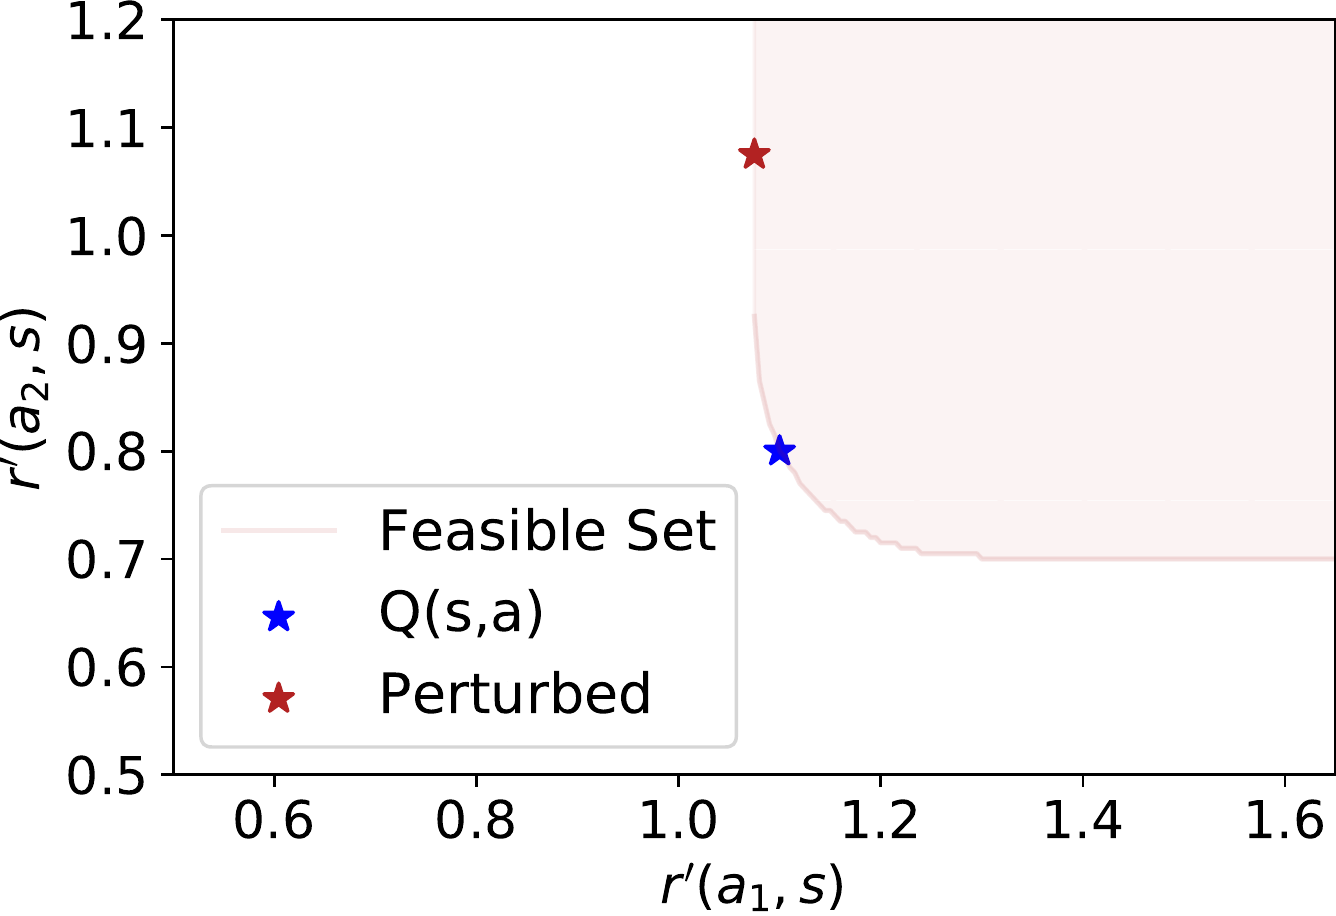}
\caption{ \centering \small $\alpha = 2, \beta = 10$}\end{subfigure} \\
\begin{subfigure}{\sidefeasible\textwidth} \phantom{ \includegraphics[width=\textwidth]
 {figs/feasible/nonuniform_prior.png}} \end{subfigure} & \begin{subfigure}{\mainfeasible\textwidth}\includegraphics[width=\textwidth, trim= 0 0 0 0, clip]
% {figs/feasible/alpha-1/alpha_neg1_beta1_uniform.png} 
{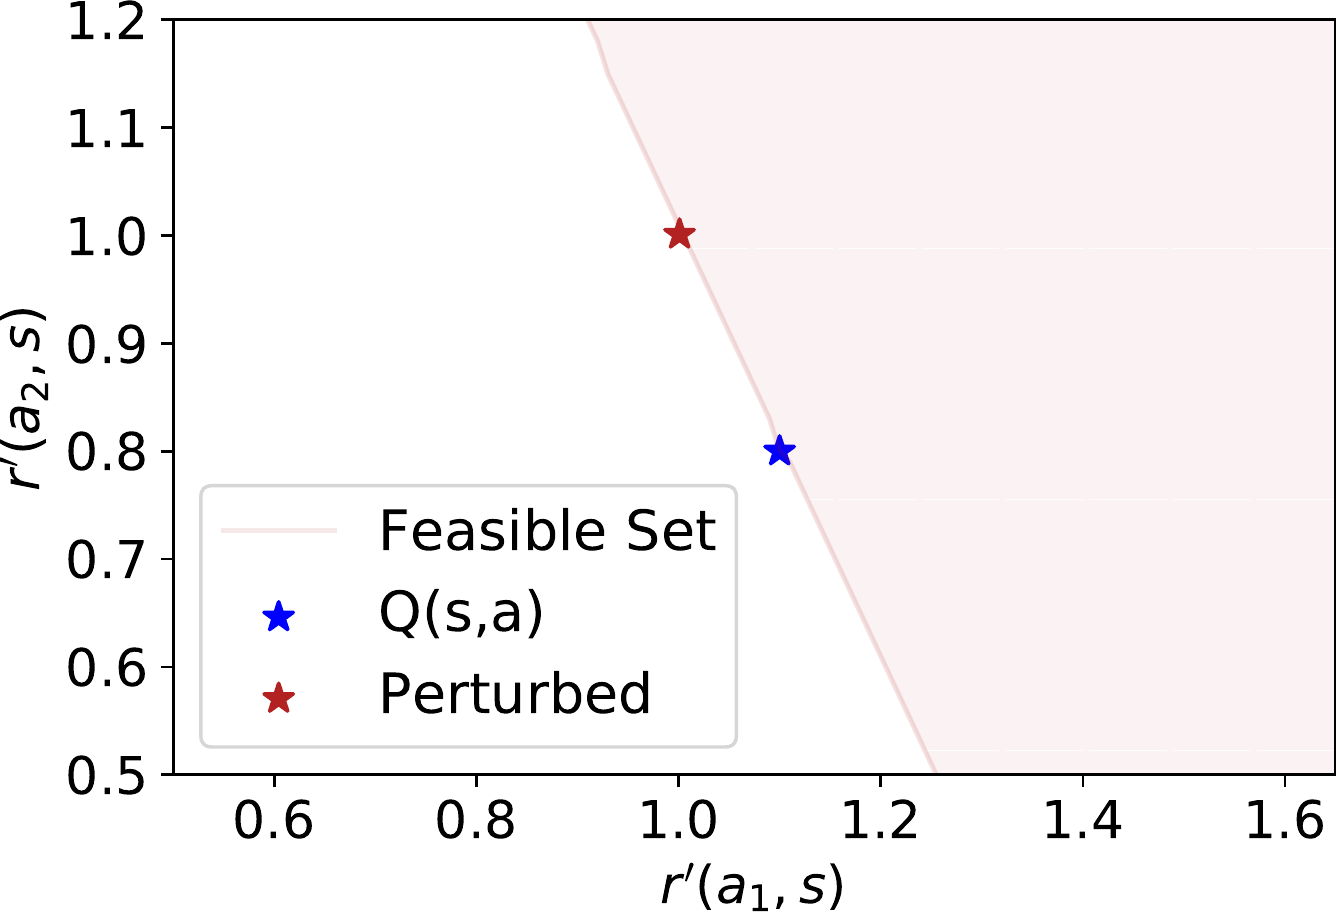}
\caption{ \centering \small $\alpha = 3, \beta = 0.1$}\end{subfigure}&
\begin{subfigure}{\mainfeasible\textwidth}\includegraphics[width=\textwidth, trim= 0 0 0 0, clip]
{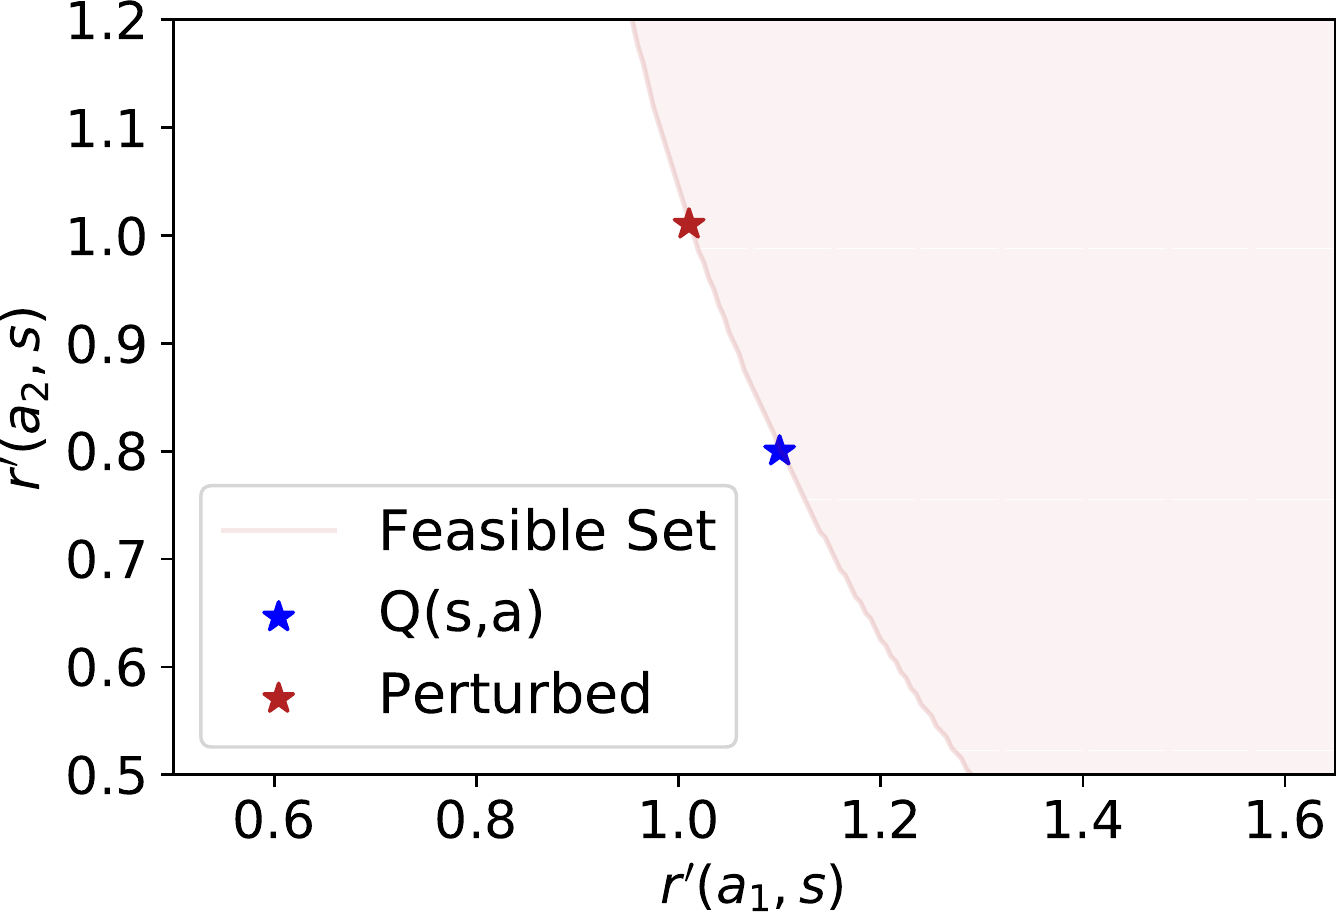}
\caption{ \centering \small $\alpha = 3, \beta = 1$}\end{subfigure}&
\begin{subfigure}{\mainfeasible\textwidth}\includegraphics[width=\textwidth, trim= 0 0 0 0, clip]
{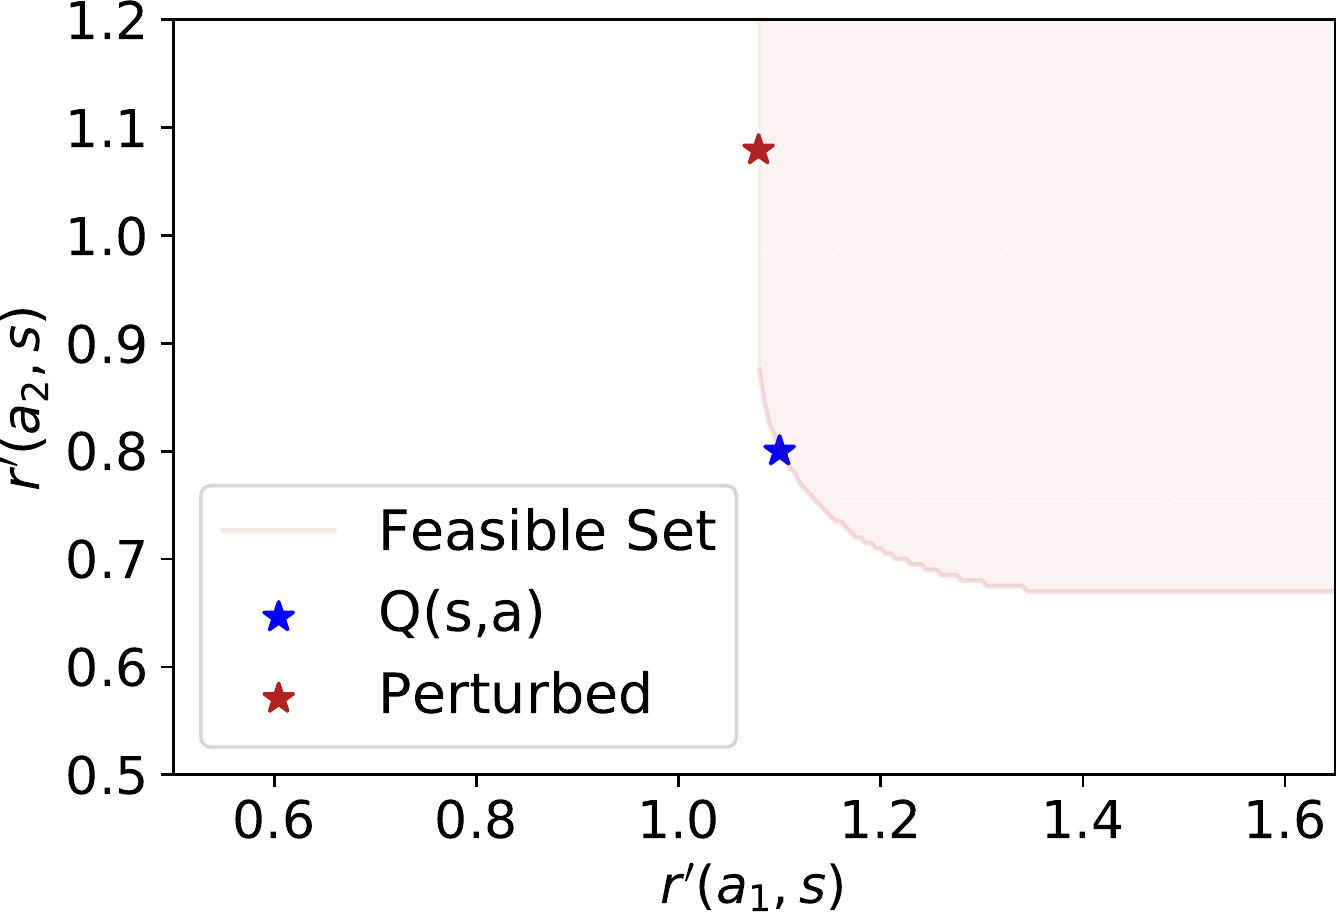}
\caption{\centering \small $\alpha = 3, \beta = 10$}\end{subfigure}
\\ %&\hspace*{.2cm}\\
% \begin{subfigure}{\sidefeasible\textwidth}\vspace*{-.24cm} \includegraphics[width=\textwidth]{figs/feasible/nonuniform_prior.png}\end{subfigure}& %\qquad \hspace*{.2cm}
% \begin{subfigure}{\mainfeasible\textwidth}\includegraphics[width=\textwidth, trim= 5 0 5 0, clip]
% % {figs/feasible/kl_73_01.png}
% {figs/feasible/kl/beta01alpha1nonuniform.pdf}
% \caption{\label{fig:tabd} \centering \small $D_{KL}, \beta = 0.1$}\end{subfigure}& %\qquad \hspace*{.2cm}
% \begin{subfigure}{\mainfeasible\textwidth}\includegraphics[width=\textwidth, trim= 5 0 5 0, clip]
% % {figs/feasible/kl_73_1.png}
% {figs/feasible/kl/beta1alpha1nonuniform.pdf}
% \caption{\label{fig:tabe} \centering \small $D_{KL}, \beta = 1$}\end{subfigure}& %\qquad \hspace*{.2cm}
% \begin{subfigure}{\mainfeasible\textwidth}\includegraphics[width=\textwidth, trim= 5 0 5 0, clip]
% % {figs/feasible/kl_73_10.png} 
% {figs/feasible/kl/beta10alpha1nonuniform.pdf}
% \caption{\label{fig:tabf} \centering \small $D_{KL}, \beta = 10$}\end{subfigure}
\end{array}
\] 
\end{center}
% \end{minipage}
\caption{Feasible Set (red region) of rewards available to the adversary, for \textsc{kl} divergence (at various $\beta$) and $\alpha$-divergence ($\alpha=\{-1, 1, 2, 3\}$) regularization and fixed $Q_*(a,s)$ values (blue star).  Red star indicates optimal perturbed reward $\mrpiopt = r - \prpiopt$, for the optimal $\pi_*(a|s)$ associated with regularization parameters $\alpha, \beta, \pi_0$ and the given $Q$-values. 
% (see \cref{eq:alpha_opt_policy} and (\ref{eq:kl_opt_policy})). 
Top row:  reference distribution $\pi_0=(\frac{1}{2},\frac{1}{2})$, bottom row: $\pi_0 = (\frac{2}{3}, \frac{1}{3})$.  
% Red dot indicates $Q(a,s)$ associated with policy $\pi(a|s)$
}\label{fig:feasible_set_nonuniform_app}
\end{figure*}
