# Supplementary material for: Your Policy Regularizer is Secretly an Adversary
Source: arXiv:2203.12592 source file (2022-07-08)
Supplement: Supplementary file 6 [file addl_single_step.tex]

\begin{figure*}[h]
\vspace*{-.3cm}
\centering
\begin{minipage}{.48\textwidth}
\subfloat[Optimal Policy]{
\[\arraycolsep=.005\textwidth
\begin{array}{cccc} %[width=40mm]
%\begin{subfigure}{.16\columnwidth}
 & \multicolumn{3}{c}{\text{(i) }\alpha=-1,  \beta = 0.1} \\[.5ex]
\multirow{3}{\WidthMM}{\includegraphics[width=\WidthM, height=\HeightS, trim=5 0 5 0]{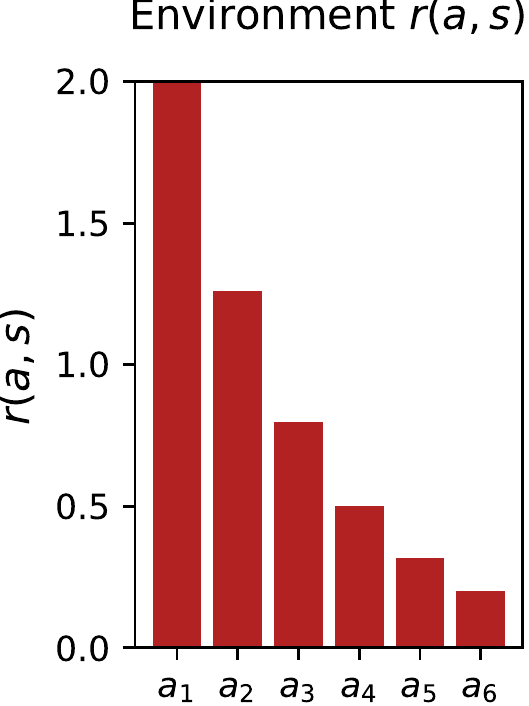} \\[4ex] \includegraphics[width=\WidthM, height=\HeightS, trim=5 0 5 0]{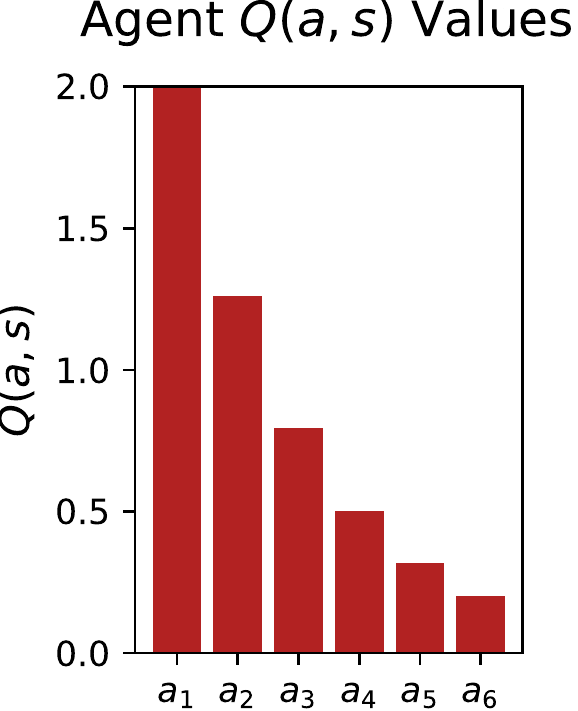}} &
%\end{subfigure}&\qquad  \hspace*{.2cm}
%\begin{subfigure}{0.33\columnwidth} 
\includegraphics[width=\WidthS, height=\HeightS, trim=5 0 5 0]{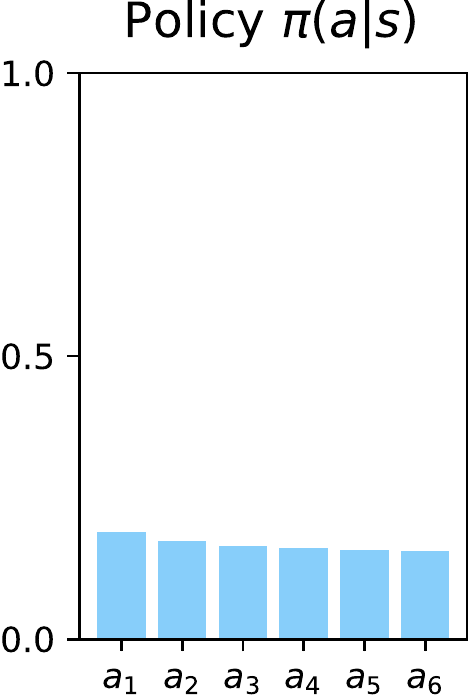} & 
%\caption{\centering \small $D_{KL}, \beta = 0.1$}\label{fig:taba}\end{subfigure}& \qquad \hspace*{.2cm}
%\begin{subfigure}{0.33\columnwidth} 
\includegraphics[width=\WidthM, height=\HeightM, trim=5 0 5 0]{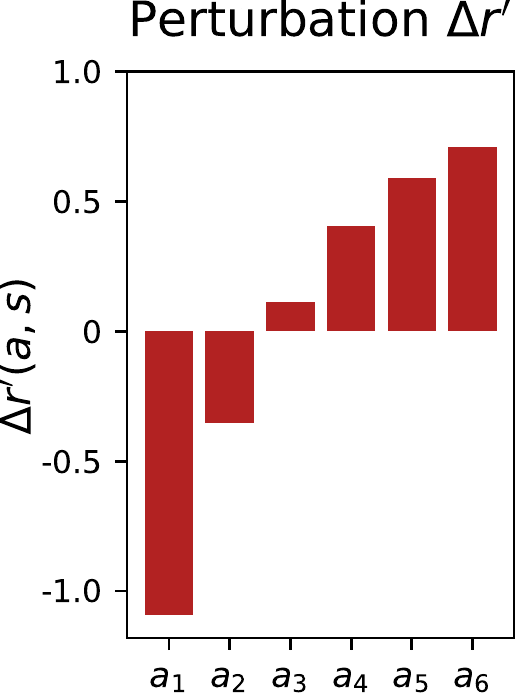} & 
%\caption{\centering  $D_{KL}, \beta = 1.0$}\label{fig:tabb}\end{subfigure}&\qquad \hspace*{.2cm}
%\begin{subfigure}{0.33\columnwidth} 
\includegraphics[width=\WidthM, height=\HeightM, trim=5 0 5 0]{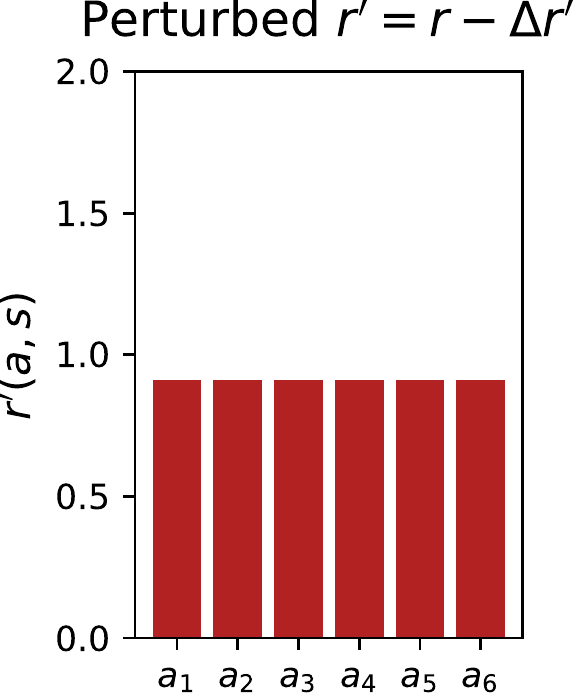}  \\[.25ex]
 & \multicolumn{3}{c}{\text{(ii) }\alpha=-1,  \beta =1.0} \\[.5ex]
%\caption{\centering \small $D_{KL}, \beta = 10$}\label{fig:tabc}\end{subfigure}&\hspace*{.2cm}\\
& % NEXT LINE for multi-row
%\includegraphics[width=\WidthM, height=\HeightS, trim=5 0 5 0]{figs/perturbed/opt_agent.pdf} &
%\end{subfigure}&\qquad  \hspace*{.2cm}
%\begin{subfigure}{0.33\columnwidth} 
\includegraphics[width=\WidthS, height=\HeightS, trim=5 0 5 0]{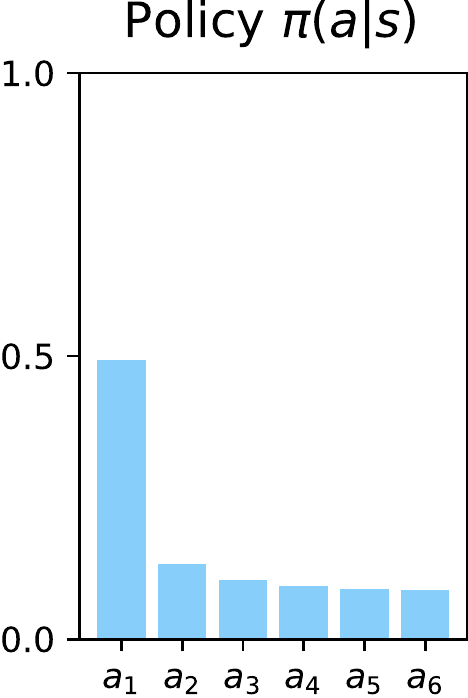} & 
%\caption{\centering \small $D_{KL}, \beta = 0.1$}\label{fig:taba}\end{subfigure}& \qquad \hspace*{.2cm}
%\begin{subfigure}{0.33\columnwidth} 
\includegraphics[width=\WidthM, height=\HeightM, trim=5 0 5 0]{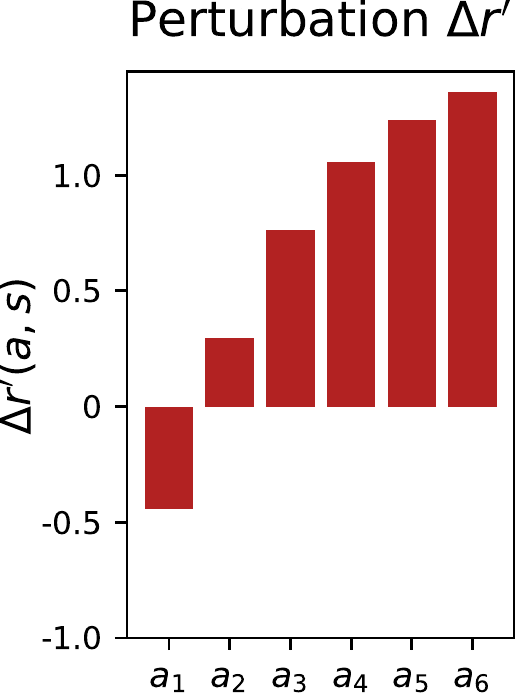} & 
%\caption{\centering  $D_{KL}, \beta = 1.0$}\label{fig:tabb}\end{subfigure}&\qquad \hspace*{.2cm}
%\begin{subfigure}{0.33\columnwidth} 
\includegraphics[width=\WidthM, height=\HeightM, trim=5 0 5 0]{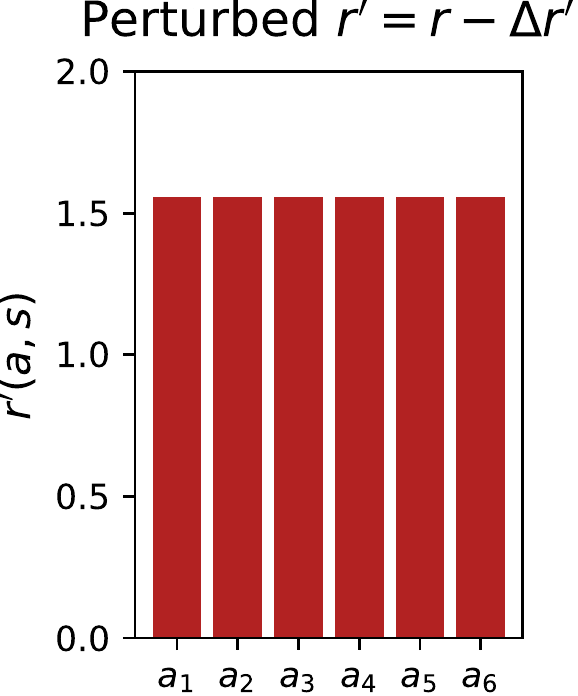} \\[.25ex]
 & \multicolumn{3}{c}{\text{(iii) } \alpha=-1,  \beta =10} \\[.25ex]
&
%\end{subfigure}&\qquad  \hspace*{.2cm}
%\begin{subfigure}{0.33\columnwidth} 
\includegraphics[width=\WidthS, height=\HeightS, trim=5 0 5 0]{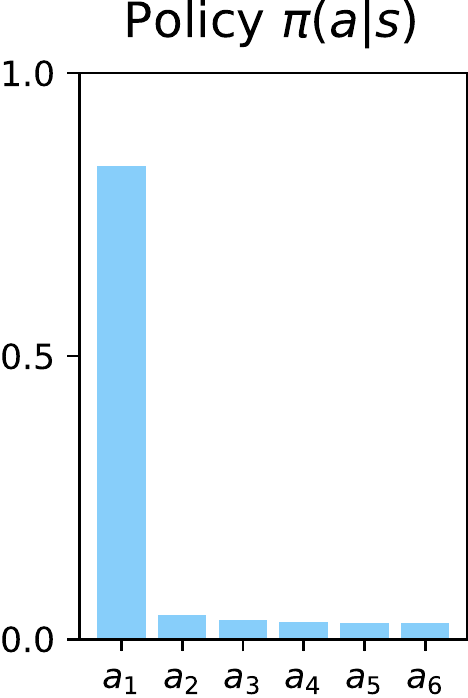} & 
%\caption{\centering \small $D_{KL}, \beta = 0.1$}\label{fig:taba}\end{subfigure}& \qquad \hspace*{.2cm}
%\begin{subfigure}{0.33\columnwidth} 
\includegraphics[width=\WidthM, height=\HeightM, trim=5 0 5 0]{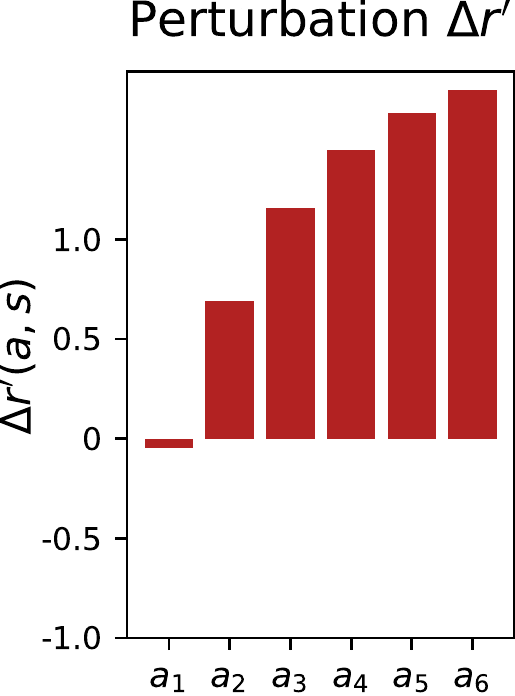} & 
%\caption{\centering  $D_{KL}, \beta = 1.0$}\label{fig:tabb}\end{subfigure}&\qquad \hspace*{.2cm}
%\begin{subfigure}{0.33\columnwidth} 
\includegraphics[width=\WidthM, height=\HeightM, trim=5 0 5 0]{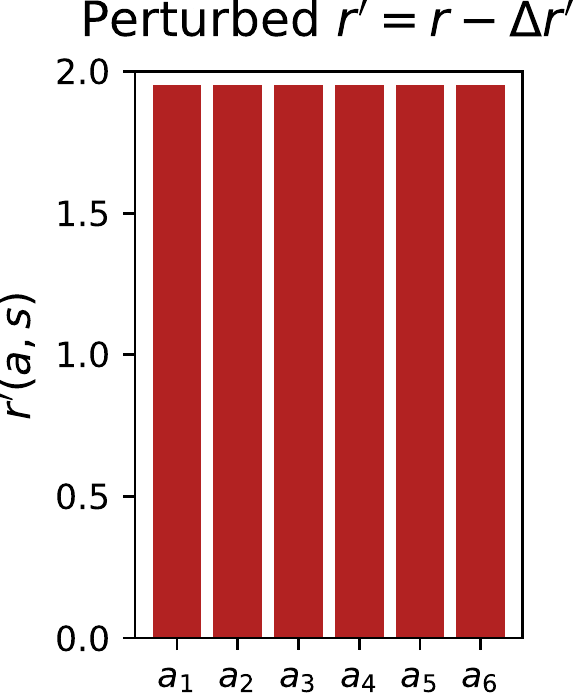} \\[.25ex]
\end{array}
\]
} %\hspace*{0.25cm}
%\label{subfig:subfig}
\end{minipage}\hspace{.02\textwidth} %{\quad \vline width 1pt}&
%&\\[2ex] \midrule
\begin{minipage}{.48\textwidth}
\subcaptionbox{Suboptimal Policy}{
\[\arraycolsep=.005\textwidth
\begin{array}{cccc} %[width=40mm]
%\begin{subfigure}{.16\columnwidth}
 & \multicolumn{3}{c}{\text{(i) } \alpha=-1,  \beta =0.1} \\[.5ex]
\multirow{3}{\WidthMM}{\includegraphics[width=\WidthM, height=\HeightS, trim=5 0 5 0]{figs/perturbed/env.pdf} \\[4ex] \includegraphics[width=\WidthM, height=\HeightS, trim=5 0 5 0]{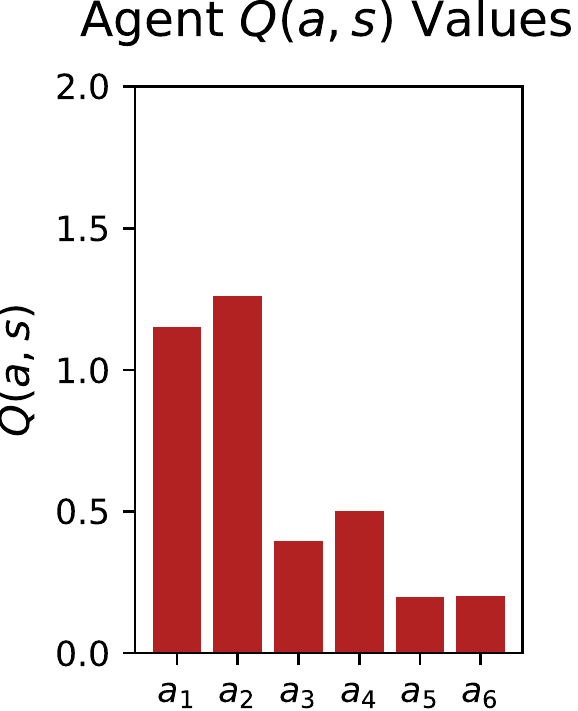}} &
%\end{subfigure}&\qquad  \hspace*{.2cm}
%\begin{subfigure}{0.33\columnwidth} 
\includegraphics[width=\WidthS, height=\HeightS, trim=5 0 5 0]{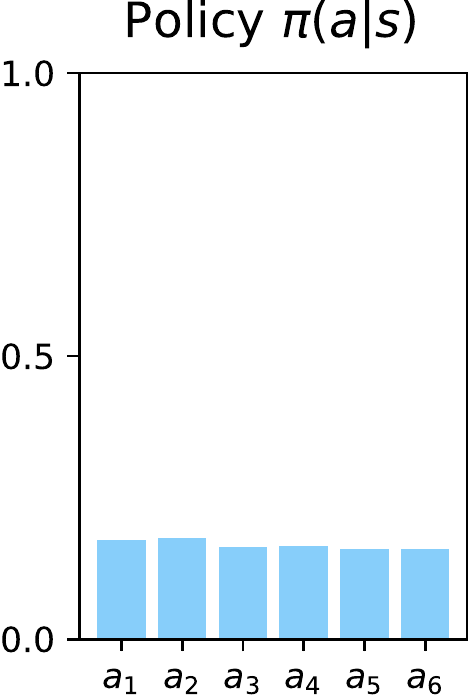} & 
%\caption{\centering \small $D_{KL}, \beta = 0.1$}\label{fig:taba}\end{subfigure}& \qquad \hspace*{.2cm}
%\begin{subfigure}{0.33\columnwidth} 
\includegraphics[width=\WidthM, height=\HeightM, trim=5 0 5 0]{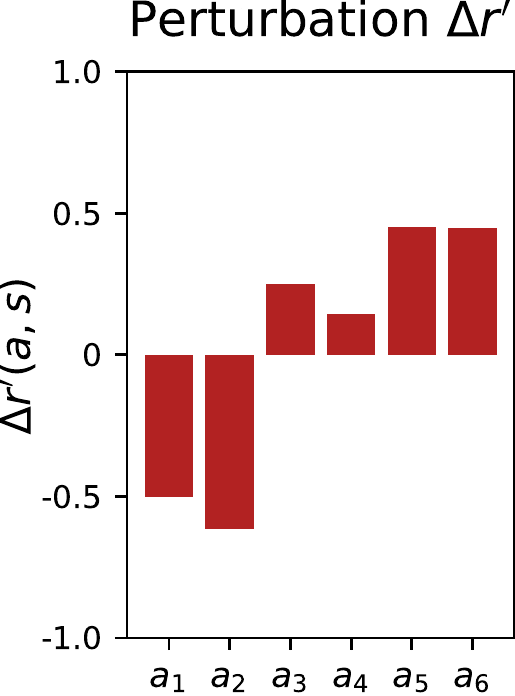} & 
%\caption{\centering  $D_{KL}, \beta = 1.0$}\label{fig:tabb}\end{subfigure}&\qquad \hspace*{.2cm}
%\begin{subfigure}{0.33\columnwidth} 
\includegraphics[width=\WidthM, height=\HeightM, trim=5 0 5 0]{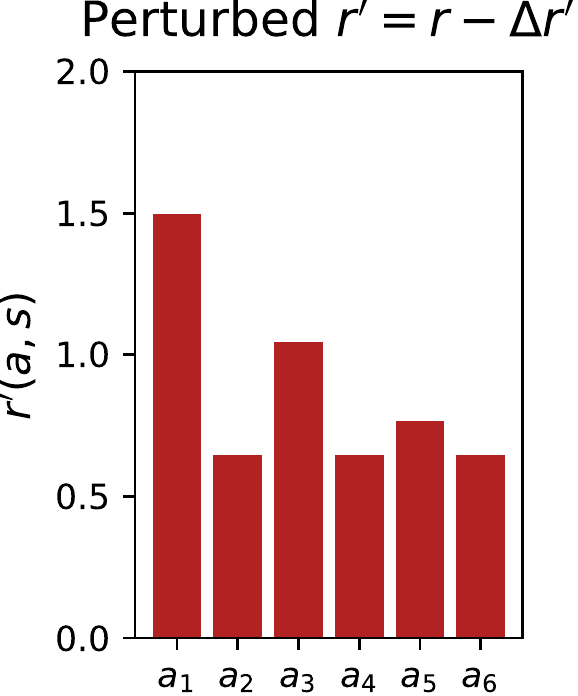}  \\[.25ex]
 & \multicolumn{3}{c}{\text{(ii) } \alpha=-1,  \beta =1.0} \\[.5ex]
%\caption{\centering \small $D_{KL}, \beta = 10$}\label{fig:tabc}\end{subfigure}&\hspace*{.2cm}\\
& % NEXT LINE for multi-row
%\includegraphics[width=\WidthM, height=\HeightS, trim=5 0 5 0]{figs/perturbed/agent.pdf} &
%\end{subfigure}&\qquad  \hspace*{.2cm}
%\begin{subfigure}{0.33\columnwidth} 
\includegraphics[width=\WidthS, height=\HeightS, trim=5 0 5 0]{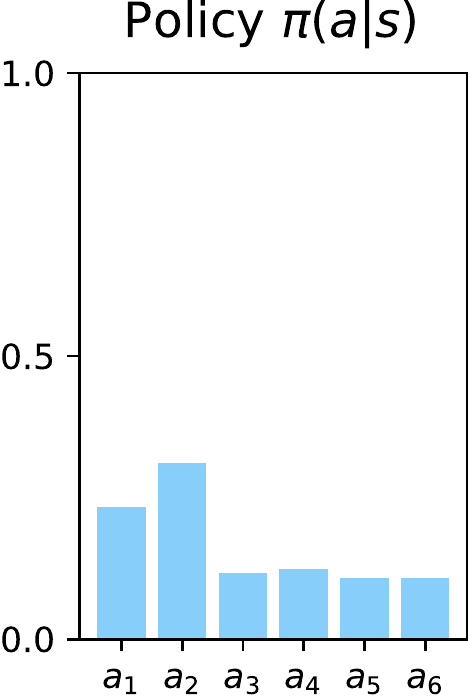} & 
%\caption{\centering \small $D_{KL}, \beta = 0.1$}\label{fig:taba}\end{subfigure}& \qquad \hspace*{.2cm}
%\begin{subfigure}{0.33\columnwidth} 
\includegraphics[width=\WidthM, height=\HeightM, trim=5 0 5 0]{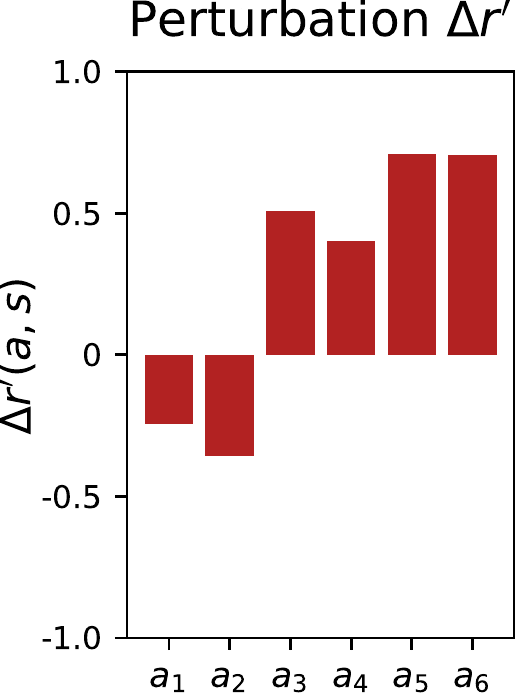} & 
%\caption{\centering  $D_{KL}, \beta = 1.0$}\label{fig:tabb}\end{subfigure}&\qquad \hspace*{.2cm}
%\begin{subfigure}{0.33\columnwidth} 
\includegraphics[width=\WidthM, height=\HeightM, trim=5 0 5 0]{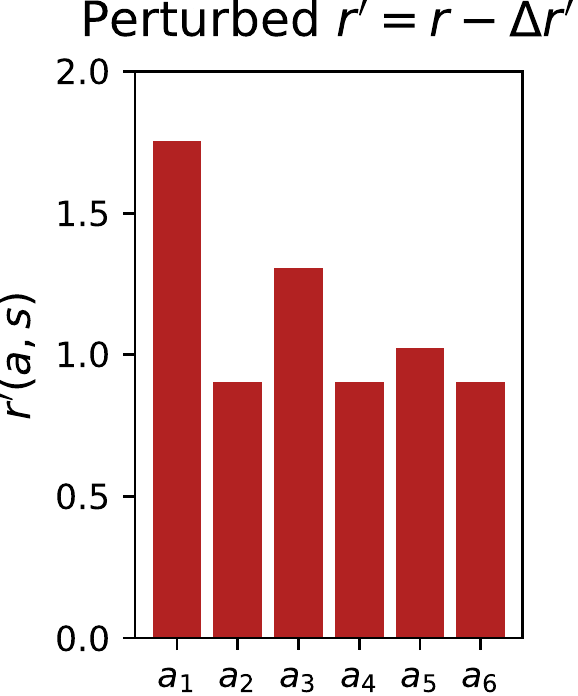} \\[.25ex]
 & \multicolumn{3}{c}{\text{(iii) } \alpha=-1,  \beta =10} \\[.5ex]
&
%\end{subfigure}&\qquad  \hspace*{.2cm}
%\begin{subfigure}{0.33\columnwidth} 
\includegraphics[width=\WidthS, height=\HeightS, trim=5 0 5 0]{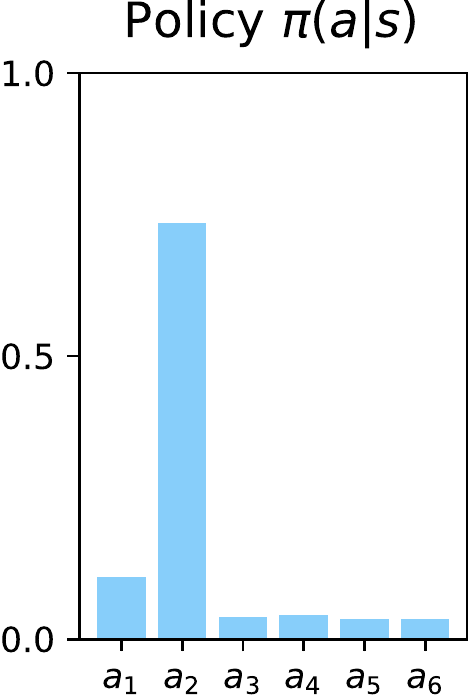} & 
%\caption{\centering \small $D_{KL}, \beta = 0.1$}\label{fig:taba}\end{subfigure}& \qquad \hspace*{.2cm}
%\begin{subfigure}{0.33\columnwidth} 
\includegraphics[width=\WidthM, height=\HeightM, trim=5 0 5 0]{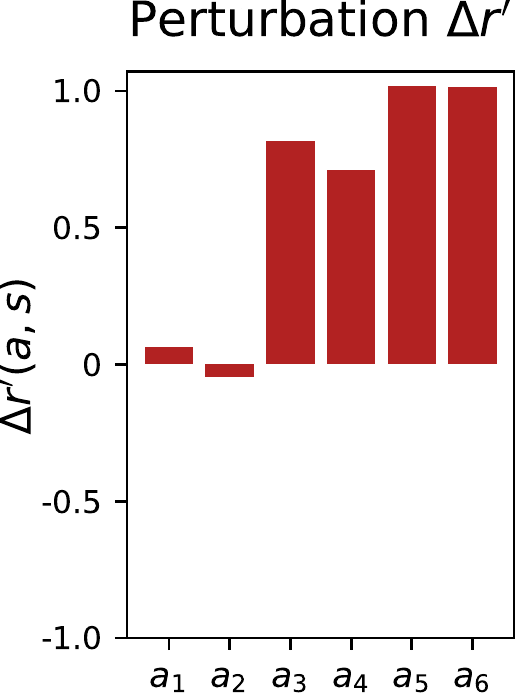} & 
%\caption{\centering  $D_{KL}, \beta = 1.0$}\label{fig:tabb}\end{subfigure}&\qquad \hspace*{.2cm}
%\begin{subfigure}{0.33\columnwidth} 
\includegraphics[width=\WidthM, height=\HeightM, trim=5 0 5 0]{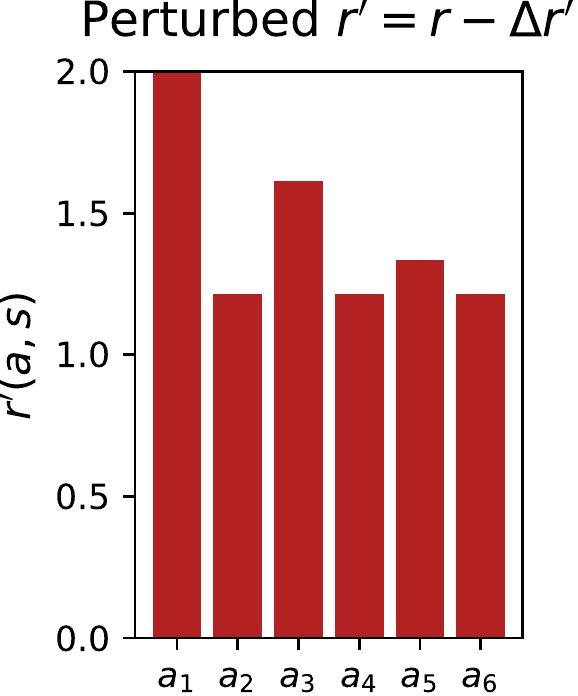} \\[.25ex]
\end{array}
\]
}
\end{minipage}
\caption{ Single-Step Reward Perturbations for $\alpha = -1 $.  Agent $Q$-values are used for each $\beta$ in columns 2-4.  }\label{fig:perturb_opt_alpha05}
\end{figure*}%
\begin{figure*}[h]
\centering
\begin{minipage}{.48\textwidth}
\subfloat[Optimal Policy]{
\[\arraycolsep=.005\textwidth
\begin{array}{cccc} %[width=40mm]
%\begin{subfigure}{.16\columnwidth}
 & \multicolumn{3}{c}{\text{(i) }\alpha=0,  \beta = 0.1} \\[.5ex]
\multirow{3}{\WidthMM}{\includegraphics[width=\WidthM, height=\HeightS, trim=5 0 5 0]{figs/perturbed/env.pdf} \\[4ex] \includegraphics[width=\WidthM, height=\HeightS, trim=5 0 5 0]{figs/perturbed/opt_agent.pdf}} &
%\end{subfigure}&\qquad  \hspace*{.2cm}
%\begin{subfigure}{0.33\columnwidth} 
\includegraphics[width=\WidthS, height=\HeightS, trim=5 0 5 0]{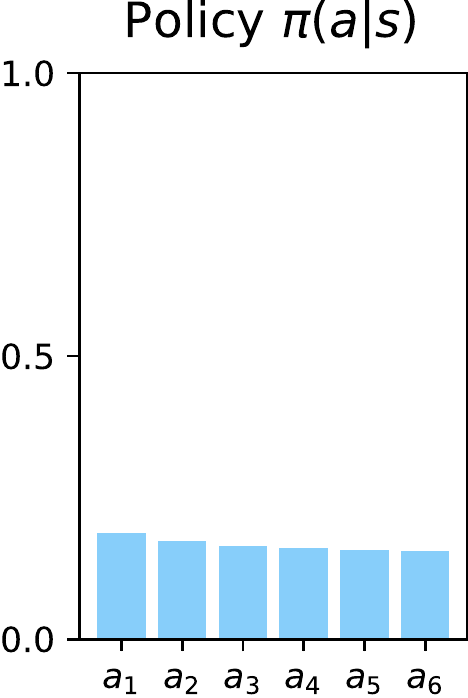} & 
%\caption{\centering \small $D_{KL}, \beta = 0.1$}\label{fig:taba}\end{subfigure}& \qquad \hspace*{.2cm}
%\begin{subfigure}{0.33\columnwidth} 
\includegraphics[width=\WidthM, height=\HeightM, trim=5 0 5 0]{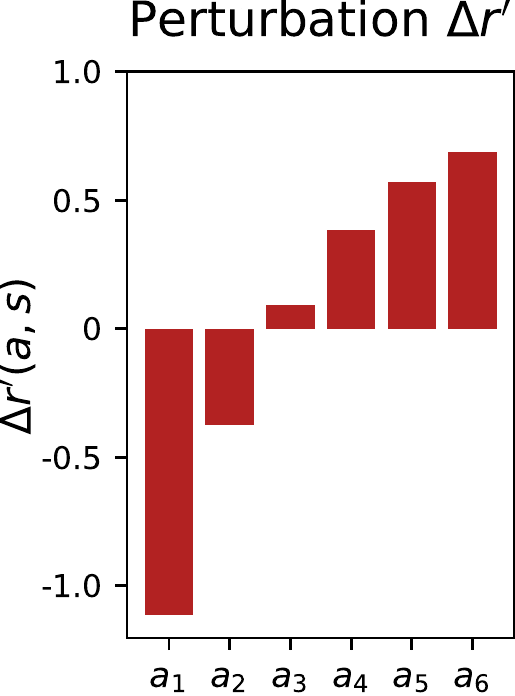} & 
%\caption{\centering  $D_{KL}, \beta = 1.0$}\label{fig:tabb}\end{subfigure}&\qquad \hspace*{.2cm}
%\begin{subfigure}{0.33\columnwidth} 
\includegraphics[width=\WidthM, height=\HeightM, trim=5 0 5 0]{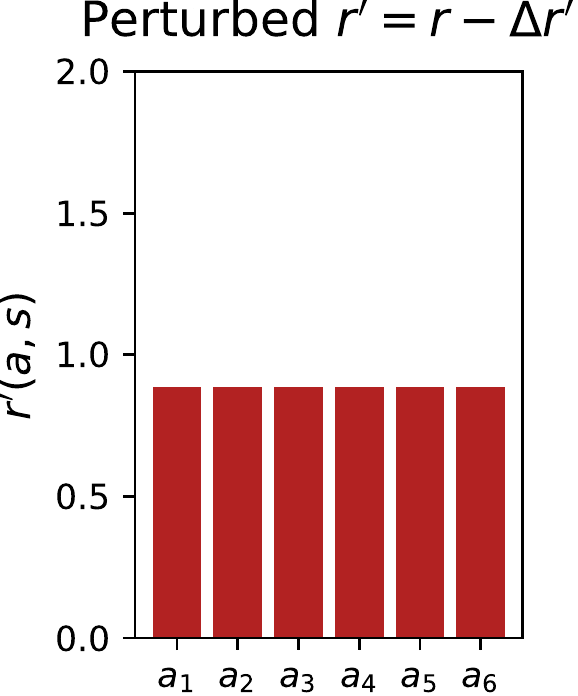}  \\[.25ex]
 & \multicolumn{3}{c}{\text{(ii) }\alpha=0,  \beta =1.0} \\[.5ex]
%\caption{\centering \small $D_{KL}, \beta = 10$}\label{fig:tabc}\end{subfigure}&\hspace*{.2cm}\\
& % NEXT LINE for multi-row
%\includegraphics[width=\WidthM, height=\HeightS, trim=5 0 5 0]{figs/perturbed/opt_agent.pdf} &
%\end{subfigure}&\qquad  \hspace*{.2cm}
%\begin{subfigure}{0.33\columnwidth} 
\includegraphics[width=\WidthS, height=\HeightS, trim=5 0 5 0]{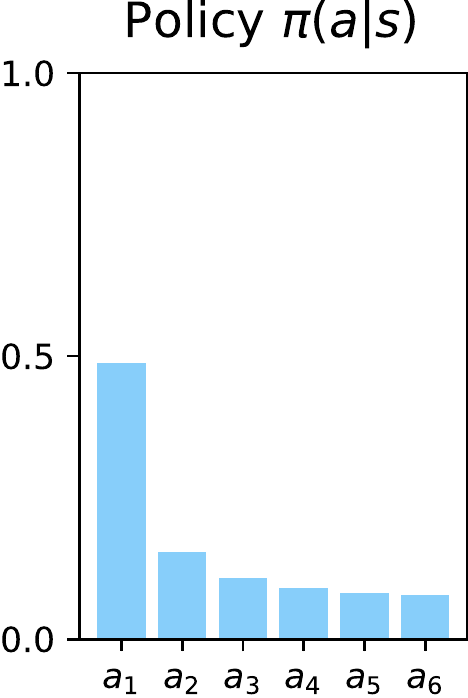} & 
%\caption{\centering \small $D_{KL}, \beta = 0.1$}\label{fig:taba}\end{subfigure}& \qquad \hspace*{.2cm}
%\begin{subfigure}{0.33\columnwidth} 
\includegraphics[width=\WidthM, height=\HeightM, trim=5 0 5 0]{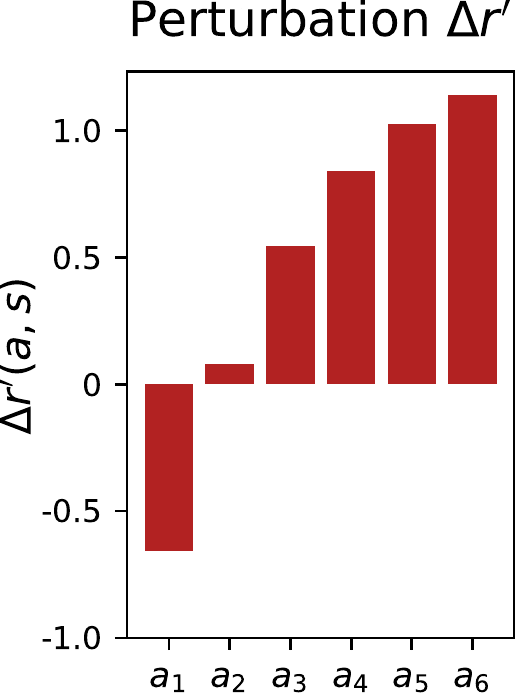} & 
%\caption{\centering  $D_{KL}, \beta = 1.0$}\label{fig:tabb}\end{subfigure}&\qquad \hspace*{.2cm}
%\begin{subfigure}{0.33\columnwidth} 
\includegraphics[width=\WidthM, height=\HeightM, trim=5 0 5 0]{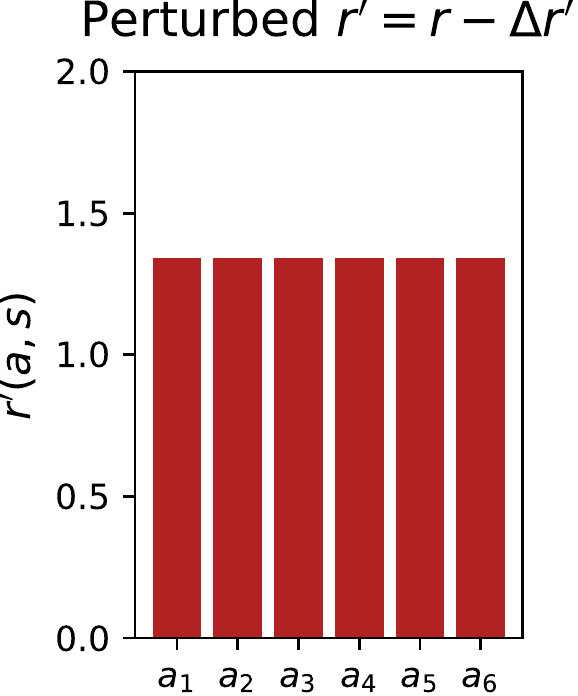} \\[.25ex]
 & \multicolumn{3}{c}{\text{(iii) } \alpha=0,  \beta =10} \\[.25ex]
&
%\end{subfigure}&\qquad  \hspace*{.2cm}
%\begin{subfigure}{0.33\columnwidth} 
\includegraphics[width=\WidthS, height=\HeightS, trim=5 0 5 0]{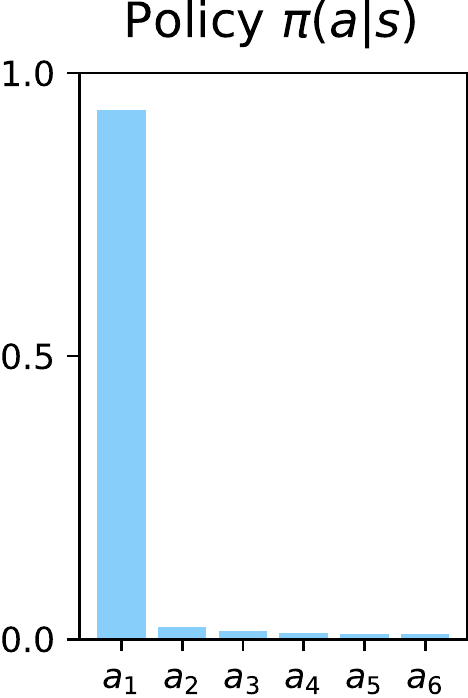} & 
%\caption{\centering \small $D_{KL}, \beta = 0.1$}\label{fig:taba}\end{subfigure}& \qquad \hspace*{.2cm}
%\begin{subfigure}{0.33\columnwidth} 
\includegraphics[width=\WidthM, height=\HeightM, trim=5 0 5 0]{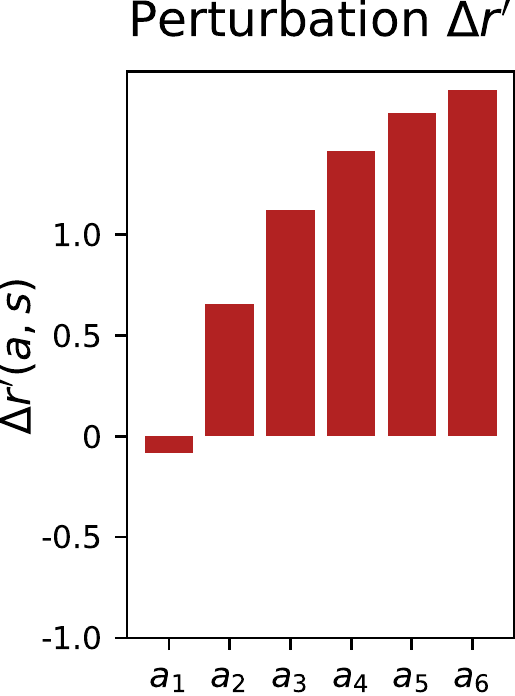} & 
%\caption{\centering  $D_{KL}, \beta = 1.0$}\label{fig:tabb}\end{subfigure}&\qquad \hspace*{.2cm}
%\begin{subfigure}{0.33\columnwidth} 
\includegraphics[width=\WidthM, height=\HeightM, trim=5 0 5 0]{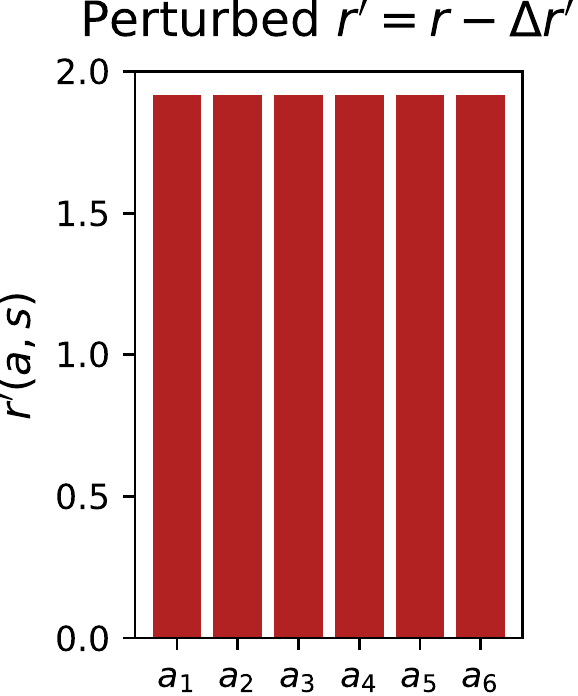} \\[.25ex]
\end{array}
\]
} %\hspace*{0.25cm}
%\label{subfig:subfig}
\end{minipage}\hspace{.02\textwidth} %{\quad \vline width 1pt}&
%&\\[2ex] \midrule
\begin{minipage}{.48\textwidth}
\subcaptionbox{Suboptimal Policy}{
\[\arraycolsep=.005\textwidth
\begin{array}{cccc} %[width=40mm]
%\begin{subfigure}{.16\columnwidth}
 & \multicolumn{3}{c}{\text{(i) } \alpha=0,  \beta =0.1} \\[.5ex]
\multirow{3}{\WidthMM}{\includegraphics[width=\WidthM, height=\HeightS, trim=5 0 5 0]{figs/perturbed/env.pdf} \\[4ex] \includegraphics[width=\WidthM, height=\HeightS, trim=5 0 5 0]{figs/perturbed/subopt_agent.pdf}} &
%\end{subfigure}&\qquad  \hspace*{.2cm}
%\begin{subfigure}{0.33\columnwidth} 
\includegraphics[width=\WidthS, height=\HeightS, trim=5 0 5 0]{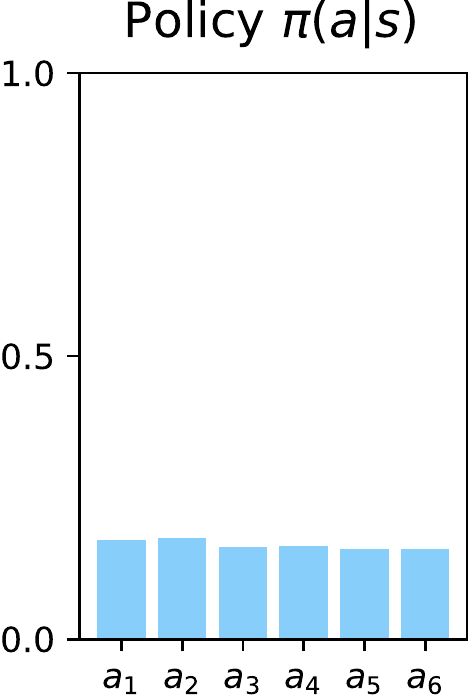} & 
%\caption{\centering \small $D_{KL}, \beta = 0.1$}\label{fig:taba}\end{subfigure}& \qquad \hspace*{.2cm}
%\begin{subfigure}{0.33\columnwidth} 
\includegraphics[width=\WidthM, height=\HeightM, trim=5 0 5 0]{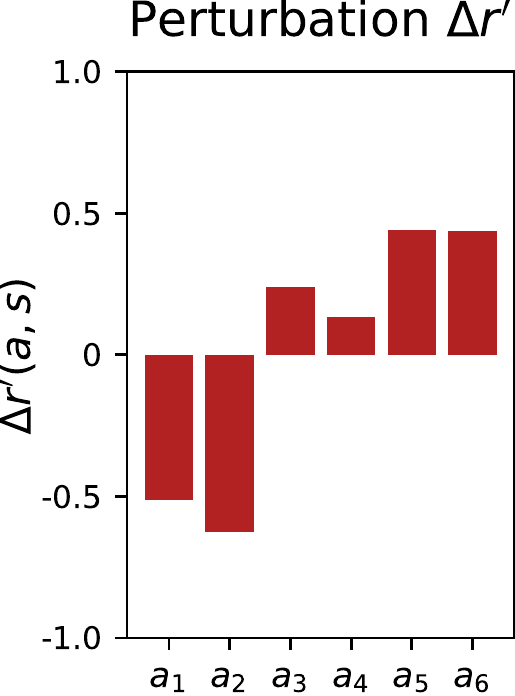} & 
%\caption{\centering  $D_{KL}, \beta = 1.0$}\label{fig:tabb}\end{subfigure}&\qquad \hspace*{.2cm}
%\begin{subfigure}{0.33\columnwidth} 
\includegraphics[width=\WidthM, height=\HeightM, trim=5 0 5 0]{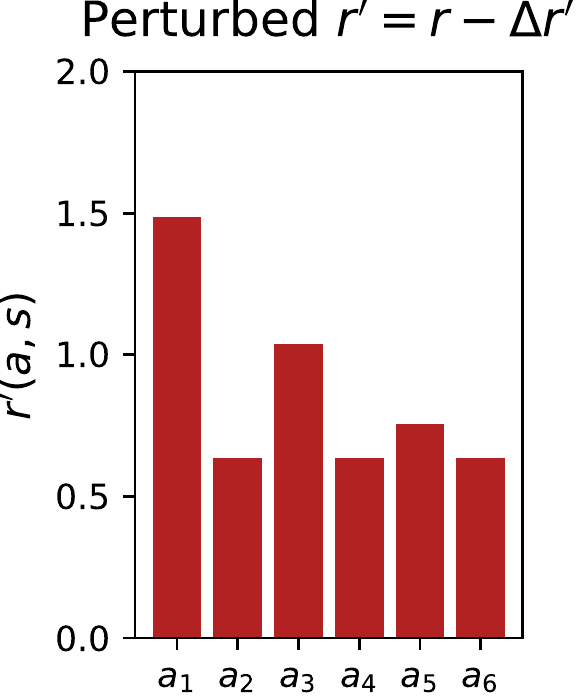}  \\[.25ex]
 & \multicolumn{3}{c}{\text{(ii) } \alpha=0,  \beta =1.0} \\[.5ex]
%\caption{\centering \small $D_{KL}, \beta = 10$}\label{fig:tabc}\end{subfigure}&\hspace*{.2cm}\\
& % NEXT LINE for multi-row
%\includegraphics[width=\WidthM, height=\HeightS, trim=5 0 5 0]{figs/perturbed/agent.pdf} &
%\end{subfigure}&\qquad  \hspace*{.2cm}
%\begin{subfigure}{0.33\columnwidth} 
\includegraphics[width=\WidthS, height=\HeightS, trim=5 0 5 0]{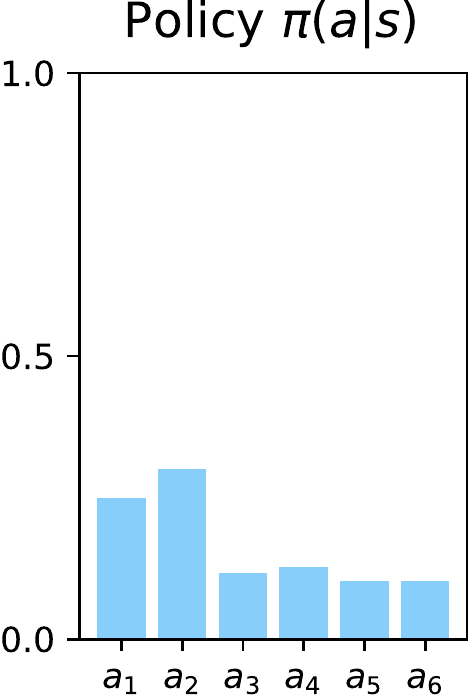} & 
%\caption{\centering \small $D_{KL}, \beta = 0.1$}\label{fig:taba}\end{subfigure}& \qquad \hspace*{.2cm}
%\begin{subfigure}{0.33\columnwidth} 
\includegraphics[width=\WidthM, height=\HeightM, trim=5 0 5 0]{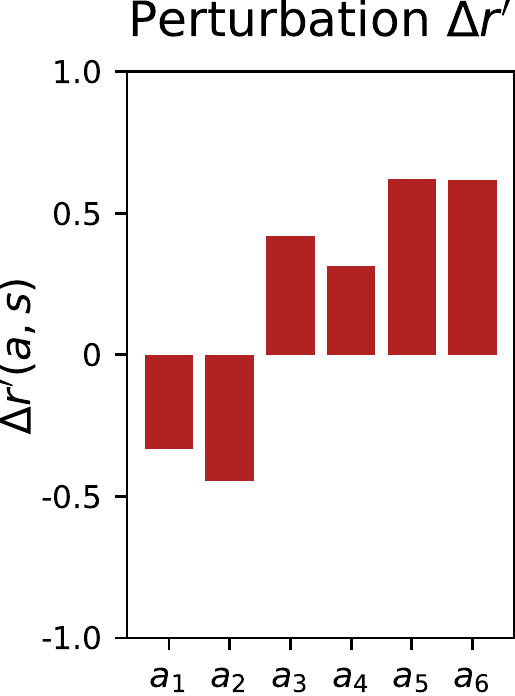} & 
%\caption{\centering  $D_{KL}, \beta = 1.0$}\label{fig:tabb}\end{subfigure}&\qquad \hspace*{.2cm}
%\begin{subfigure}{0.33\columnwidth} 
\includegraphics[width=\WidthM, height=\HeightM, trim=5 0 5 0]{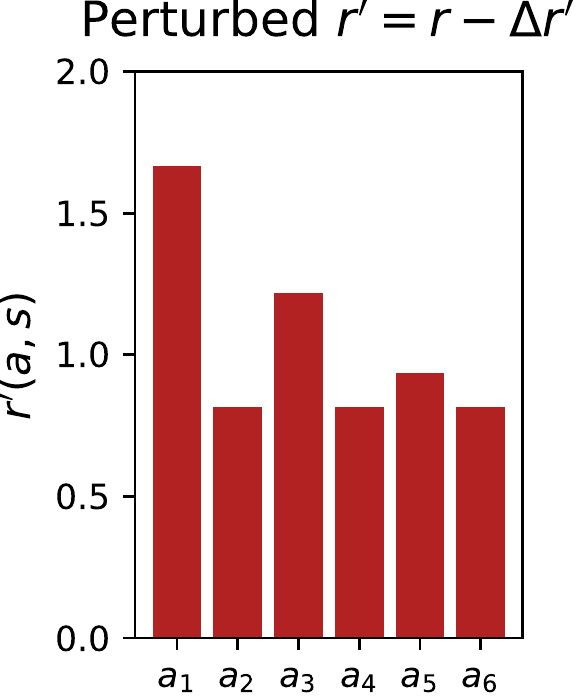} \\[.25ex]
 & \multicolumn{3}{c}{\text{(iii) } \alpha=0,  \beta =10} \\[.5ex]
&
%\end{subfigure}&\qquad  \hspace*{.2cm}
%\begin{subfigure}{0.33\columnwidth} 
\includegraphics[width=\WidthS, height=\HeightS, trim=5 0 5 0]{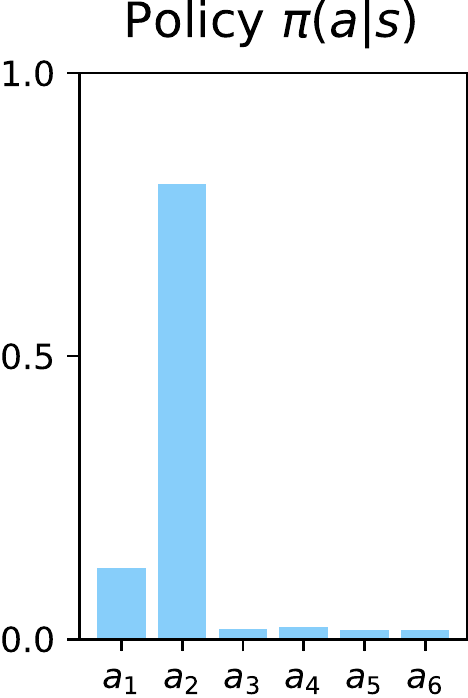} & 
%\caption{\centering \small $D_{KL}, \beta = 0.1$}\label{fig:taba}\end{subfigure}& \qquad \hspace*{.2cm}
%\begin{subfigure}{0.33\columnwidth} 
\includegraphics[width=\WidthM, height=\HeightM, trim=5 0 5 0]{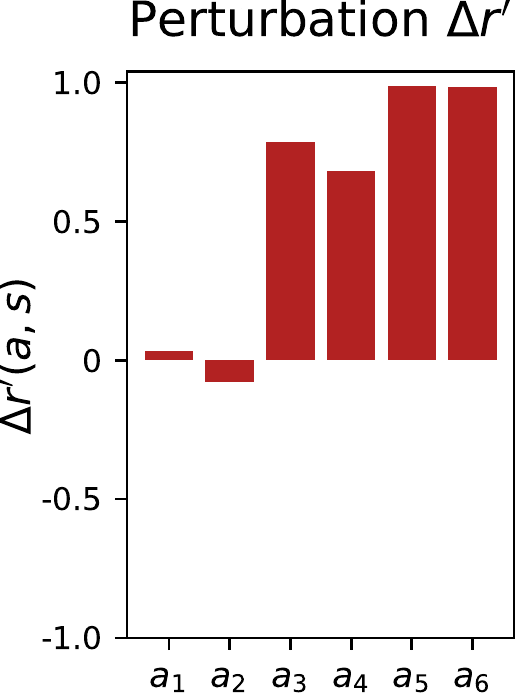} & 
%\caption{\centering  $D_{KL}, \beta = 1.0$}\label{fig:tabb}\end{subfigure}&\qquad \hspace*{.2cm}
%\begin{subfigure}{0.33\columnwidth} 
\includegraphics[width=\WidthM, height=\HeightM, trim=5 0 5 0]{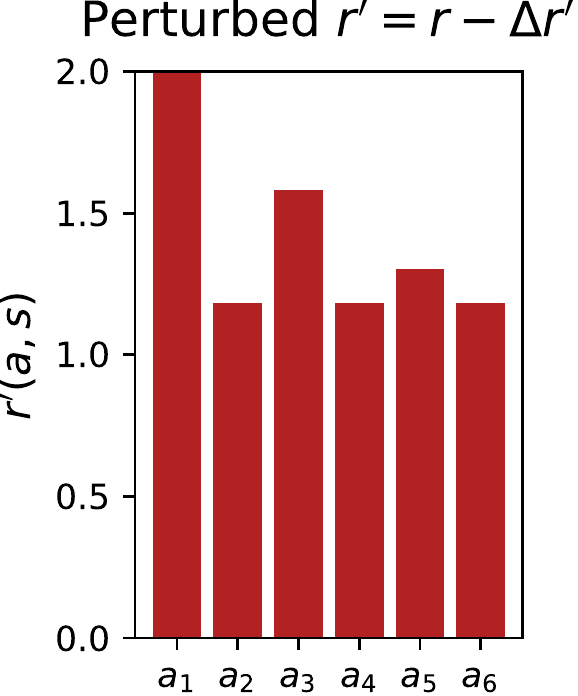} \\[.25ex]
\end{array}
\]
}
\end{minipage}
\caption{ Single-Step Reward Perturbations for $\alpha = 0$.  Agent $Q$-values are used for each $\beta$ in columns 2-4.  }\label{fig:perturb_opt_alpha05}
\end{figure*}%
\begin{figure*}[h]
\centering
\begin{minipage}{.48\textwidth}
\subfloat[Optimal Policy]{
\[\arraycolsep=.005\textwidth
\begin{array}{cccc} %[width=40mm]
%\begin{subfigure}{.16\columnwidth}
 & \multicolumn{3}{c}{\text{(i) }\alpha=3,  \beta =0.1} \\[.5ex]
\multirow{3}{\WidthMM}{\includegraphics[width=\WidthM, height=\HeightS, trim=5 0 5 0]{figs/perturbed/env.pdf} \\[4ex] \includegraphics[width=\WidthM, height=\HeightS, trim=5 0 5 0]{figs/perturbed/opt_agent.pdf}} &
%\end{subfigure}&\qquad  \hspace*{.2cm}
%\begin{subfigure}{0.33\columnwidth} 
\includegraphics[width=\WidthS, height=\HeightS, trim=5 0 5 0]{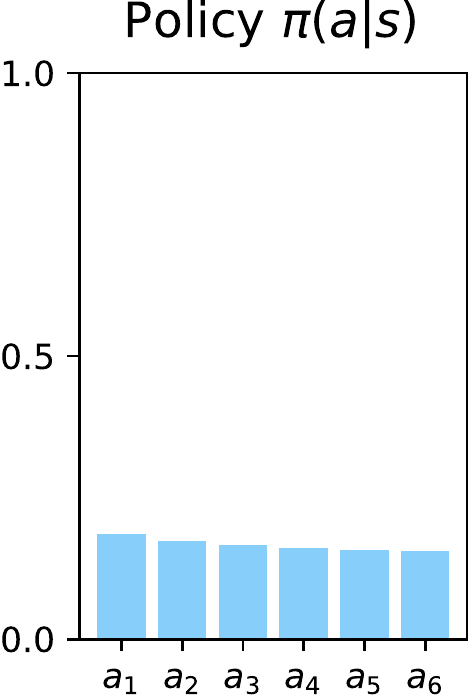} & 
%\caption{\centering \small $D_{KL}, \beta = 0.1$}\label{fig:taba}\end{subfigure}& \qquad \hspace*{.2cm}
%\begin{subfigure}{0.33\columnwidth} 
\includegraphics[width=\WidthM, height=\HeightM, trim=5 0 5 0]{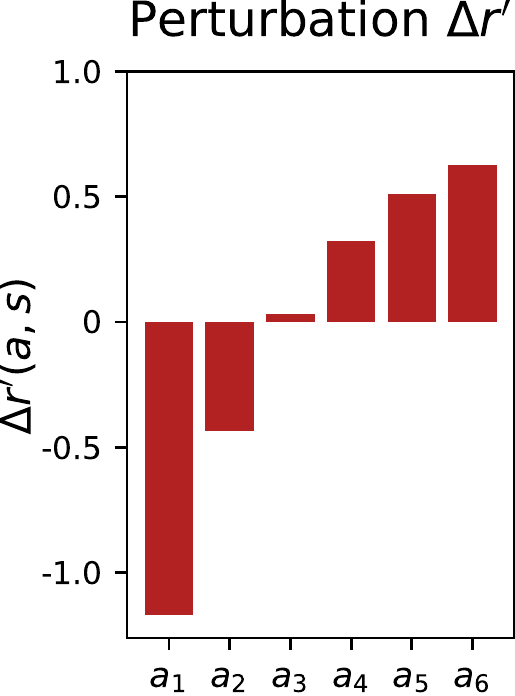} & 
%\caption{\centering  $D_{KL}, \beta = 1.0$}\label{fig:tabb}\end{subfigure}&\qquad \hspace*{.2cm}
%\begin{subfigure}{0.33\columnwidth} 
\includegraphics[width=\WidthM, height=\HeightM, trim=5 0 5 0]{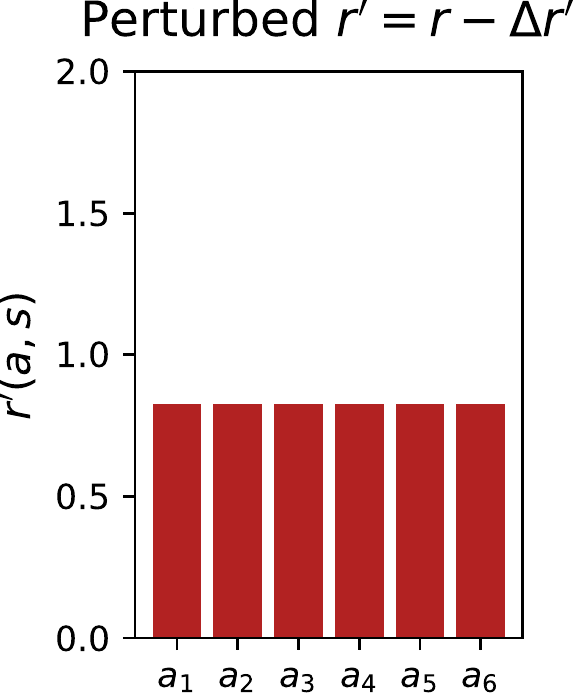}  \\[.25ex]
 & \multicolumn{3}{c}{\text{(ii) }\alpha=3,  \beta =1.0} \\[.5ex]
%\caption{\centering \small $D_{KL}, \beta = 10$}\label{fig:tabc}\end{subfigure}&\hspace*{.2cm}\\
& % NEXT LINE for multi-row
%\includegraphics[width=\WidthM, height=\HeightS, trim=5 0 5 0]{figs/perturbed/opt_agent.pdf} &
%\end{subfigure}&\qquad  \hspace*{.2cm}
%\begin{subfigure}{0.33\columnwidth} 
\includegraphics[width=\WidthS, height=\HeightS, trim=5 0 5 0]{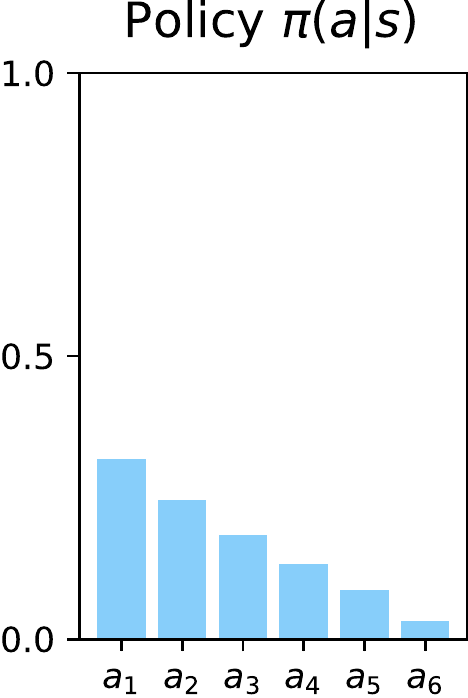} & 
%\caption{\centering \small $D_{KL}, \beta = 0.1$}\label{fig:taba}\end{subfigure}& \qquad \hspace*{.2cm}
%\begin{subfigure}{0.33\columnwidth} 
\includegraphics[width=\WidthM, height=\HeightM, trim=5 0 5 0]{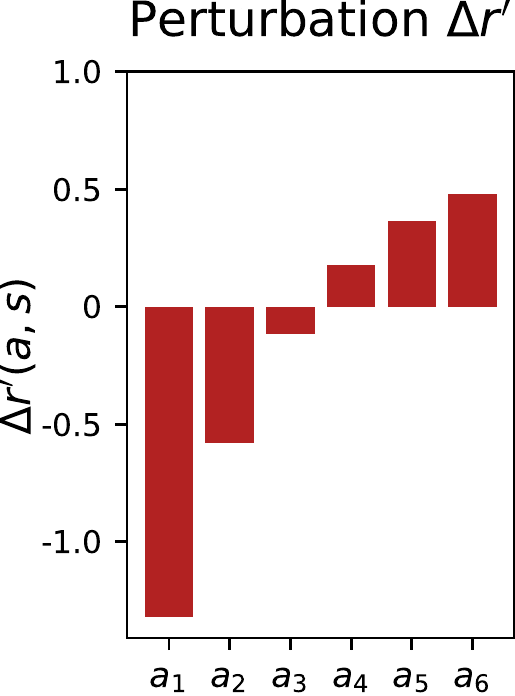} & 
%\caption{\centering  $D_{KL}, \beta = 1.0$}\label{fig:tabb}\end{subfigure}&\qquad \hspace*{.2cm}
%\begin{subfigure}{0.33\columnwidth} 
\includegraphics[width=\WidthM, height=\HeightM, trim=5 0 5 0]{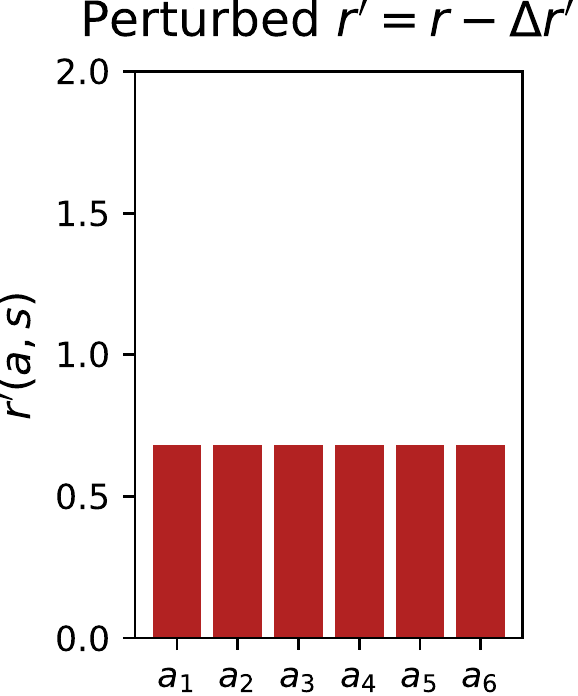} \\[.25ex]
 & \multicolumn{3}{c}{\text{(iii) } \alpha=3,  \beta =10} \\[.25ex]
&
%\end{subfigure}&\qquad  \hspace*{.2cm}
%\begin{subfigure}{0.33\columnwidth} 
\includegraphics[width=\WidthS, height=\HeightS, trim=5 0 5 0]{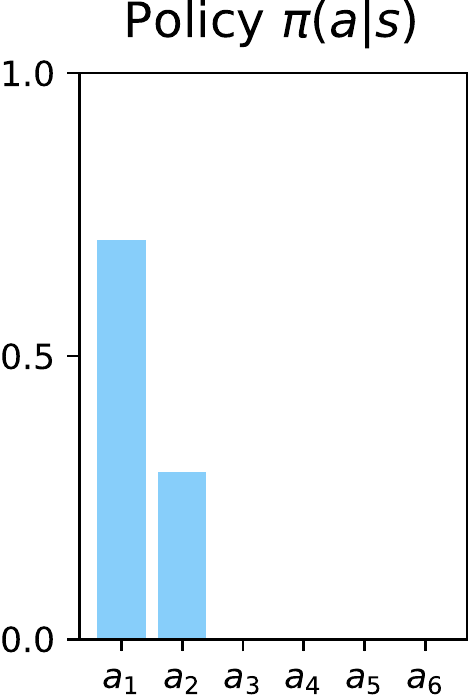} & 
%\caption{\centering \small $D_{KL}, \beta = 0.1$}\label{fig:taba}\end{subfigure}& \qquad \hspace*{.2cm}
%\begin{subfigure}{0.33\columnwidth} 
\includegraphics[width=\WidthM, height=\HeightM, trim=5 0 5 0]{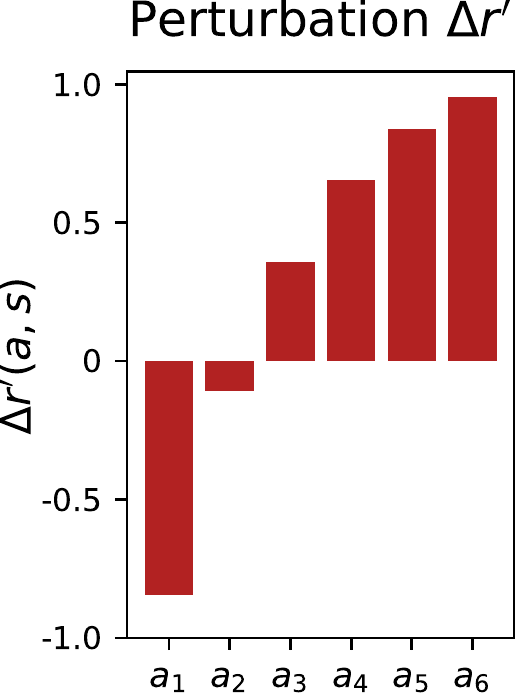} & 
%\caption{\centering  $D_{KL}, \beta = 1.0$}\label{fig:tabb}\end{subfigure}&\qquad \hspace*{.2cm}
%\begin{subfigure}{0.33\columnwidth} 
\includegraphics[width=\WidthM, height=\HeightM, trim=5 0 5 0]{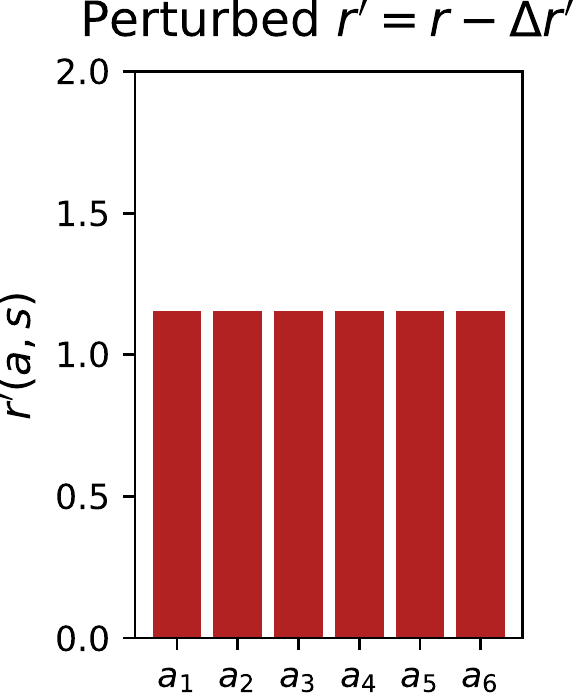} \\[.25ex]
\end{array}
\]
} %\hspace*{0.25cm}
%\label{subfig:subfig}
\end{minipage}\hspace{.02\textwidth} %{\quad \vline width 1pt}&
%&\\[2ex] \midrule
\begin{minipage}{.48\textwidth}
\subcaptionbox{Suboptimal Policy}{
\[\arraycolsep=.005\textwidth
\begin{array}{cccc} %[width=40mm]
%\begin{subfigure}{.16\columnwidth}
 & \multicolumn{3}{c}{\text{(i) } \alpha=3,  \beta =0.1} \\[.5ex]
\multirow{3}{\WidthMM}{\includegraphics[width=\WidthM, height=\HeightS, trim=5 0 5 0]{figs/perturbed/env.pdf} \\[4ex] \includegraphics[width=\WidthM, height=\HeightS, trim=5 0 5 0]{figs/perturbed/subopt_agent.pdf}} &
%\end{subfigure}&\qquad  \hspace*{.2cm}
%\begin{subfigure}{0.33\columnwidth} 
\includegraphics[width=\WidthS, height=\HeightS, trim=5 0 5 0]{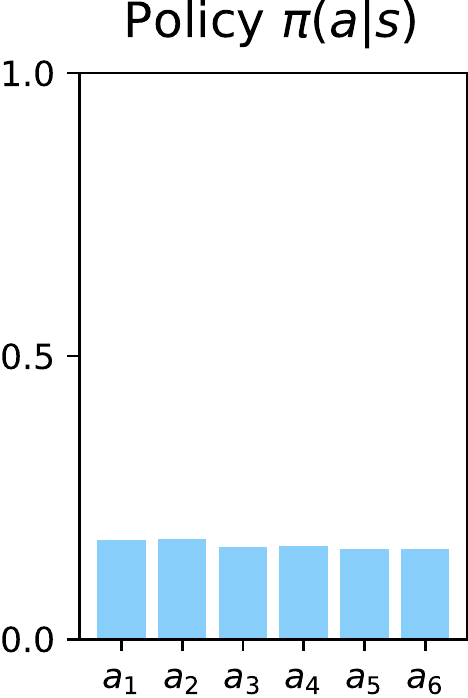} & 
%\caption{\centering \small $D_{KL}, \beta = 0.1$}\label{fig:taba}\end{subfigure}& \qquad \hspace*{.2cm}
%\begin{subfigure}{0.33\columnwidth} 
\includegraphics[width=\WidthM, height=\HeightM, trim=5 0 5 0]{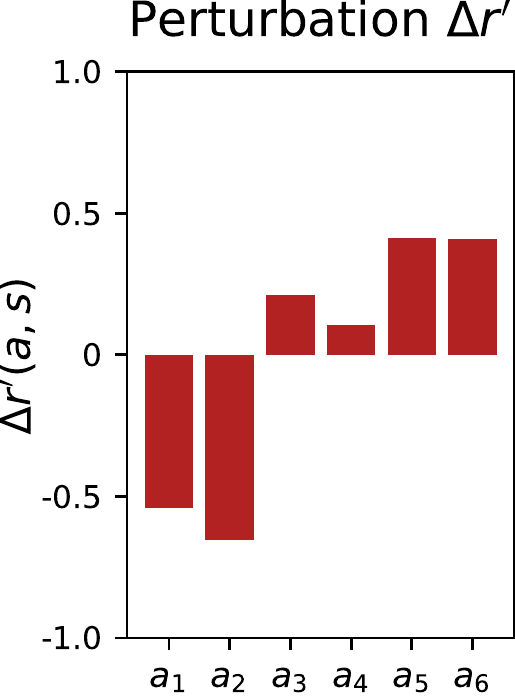} & 
%\caption{\centering  $D_{KL}, \beta = 1.0$}\label{fig:tabb}\end{subfigure}&\qquad \hspace*{.2cm}
%\begin{subfigure}{0.33\columnwidth} 
\includegraphics[width=\WidthM, height=\HeightM, trim=5 0 5 0]{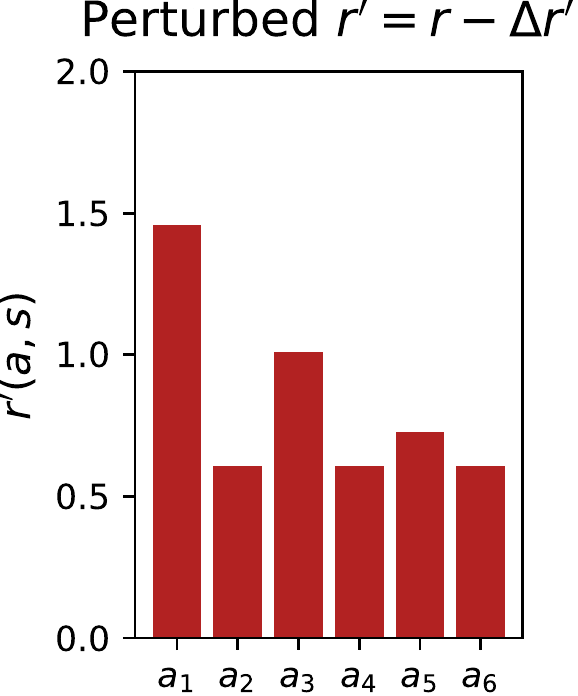}  \\[.25ex]
 & \multicolumn{3}{c}{\text{(ii) } \alpha=3,  \beta =1.0} \\[.5ex]
%\caption{\centering \small $D_{KL}, \beta = 10$}\label{fig:tabc}\end{subfigure}&\hspace*{.2cm}\\
& % NEXT LINE for multi-row
%\includegraphics[width=\WidthM, height=\HeightS, trim=5 0 5 0]{figs/perturbed/agent.pdf} &
%\end{subfigure}&\qquad  \hspace*{.2cm}
%\begin{subfigure}{0.33\columnwidth} 
\includegraphics[width=\WidthS, height=\HeightS, trim=5 0 5 0]{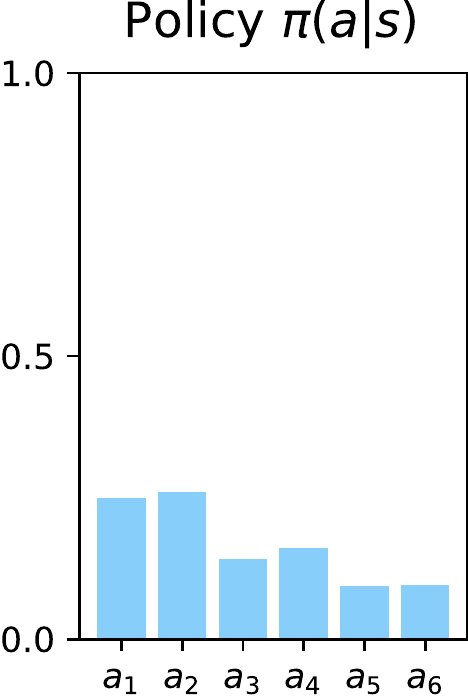} & 
%\caption{\centering \small $D_{KL}, \beta = 0.1$}\label{fig:taba}\end{subfigure}& \qquad \hspace*{.2cm}
%\begin{subfigure}{0.33\columnwidth} 
\includegraphics[width=\WidthM, height=\HeightM, trim=5 0 5 0]{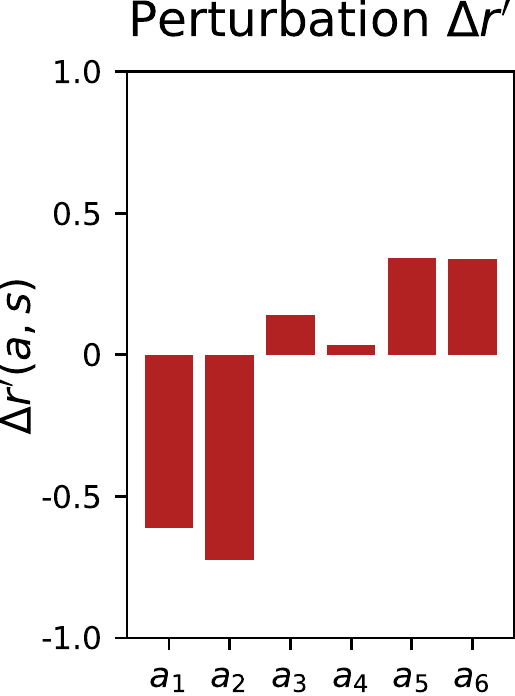} & 
%\caption{\centering  $D_{KL}, \beta = 1.0$}\label{fig:tabb}\end{subfigure}&\qquad \hspace*{.2cm}
%\begin{subfigure}{0.33\columnwidth} 
\includegraphics[width=\WidthM, height=\HeightM, trim=5 0 5 0]{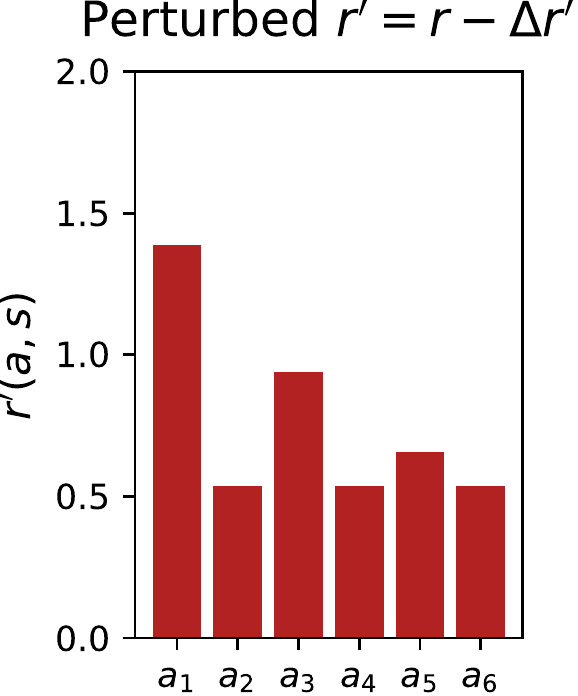} \\[.25ex]
 & \multicolumn{3}{c}{\text{(iii) } \alpha=3,  \beta =10} \\[.5ex]
&
%\end{subfigure}&\qquad  \hspace*{.2cm}
%\begin{subfigure}{0.33\columnwidth} 
\includegraphics[width=\WidthS, height=\HeightS, trim=5 0 5 0]{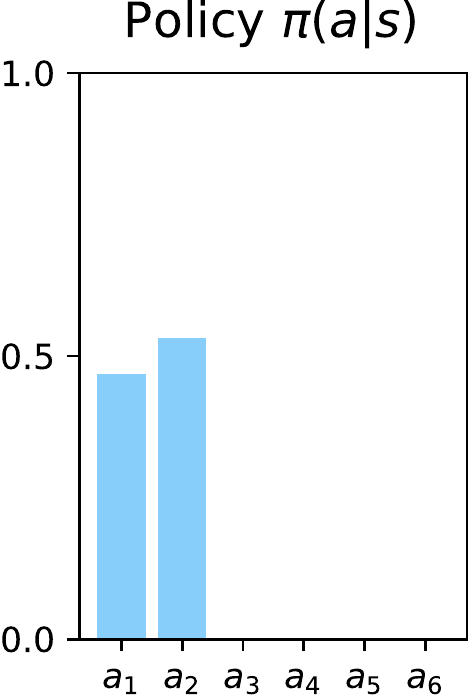} & 
%\caption{\centering \small $D_{KL}, \beta = 0.1$}\label{fig:taba}\end{subfigure}& \qquad \hspace*{.2cm}
%\begin{subfigure}{0.33\columnwidth} 
\includegraphics[width=\WidthM, height=\HeightM, trim=5 0 5 0]{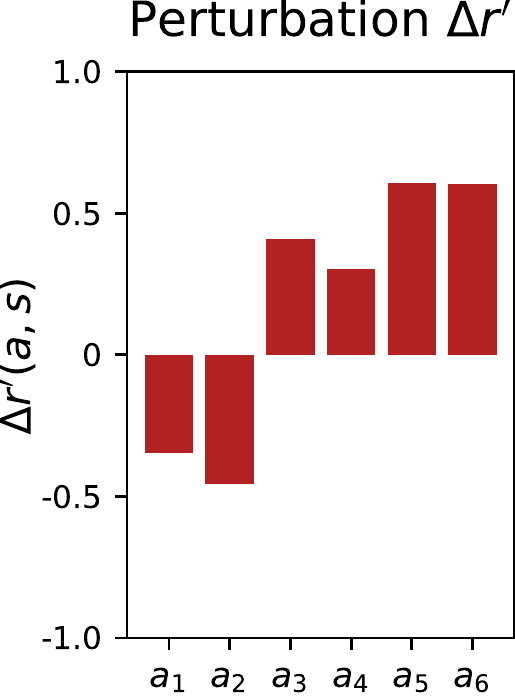} & 
%\caption{\centering  $D_{KL}, \beta = 1.0$}\label{fig:tabb}\end{subfigure}&\qquad \hspace*{.2cm}
%\begin{subfigure}{0.33\columnwidth} 
\includegraphics[width=\WidthM, height=\HeightM, trim=5 0 5 0]{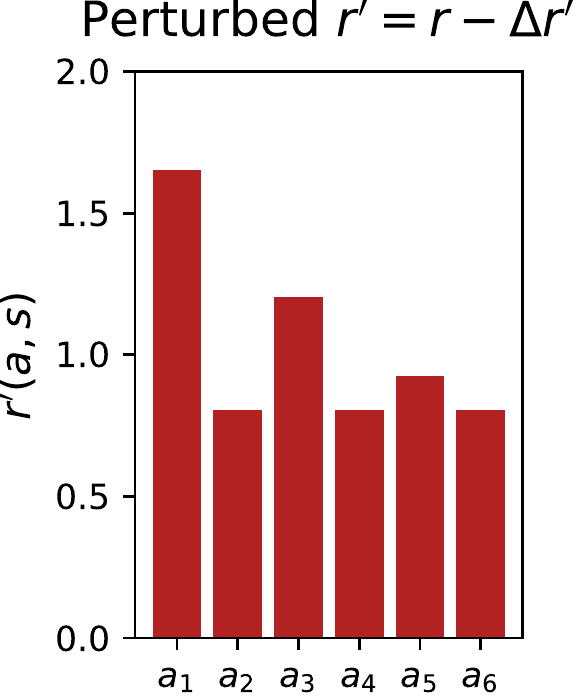} \\[.25ex]
\end{array}
\]
}
\end{minipage}
\caption{ Single-Step Reward Perturbations for $\alpha = 3$.  Agent $Q$-values are used for each $\beta$ in columns 2-4.  }\label{fig:perturb_opt_alpha3}
\end{figure*}
