# Supplementary material for: Your Policy Regularizer is Secretly an Adversary
Source: arXiv:2203.12592 source file (2022-07-08)
Supplement: Supplementary file 7 [file path_consistency.tex]

\begin{figure*}[t]
\vspace*{-.3cm}
\begin{subfigure}{.2\textwidth}
\includegraphics[width=\textwidth]{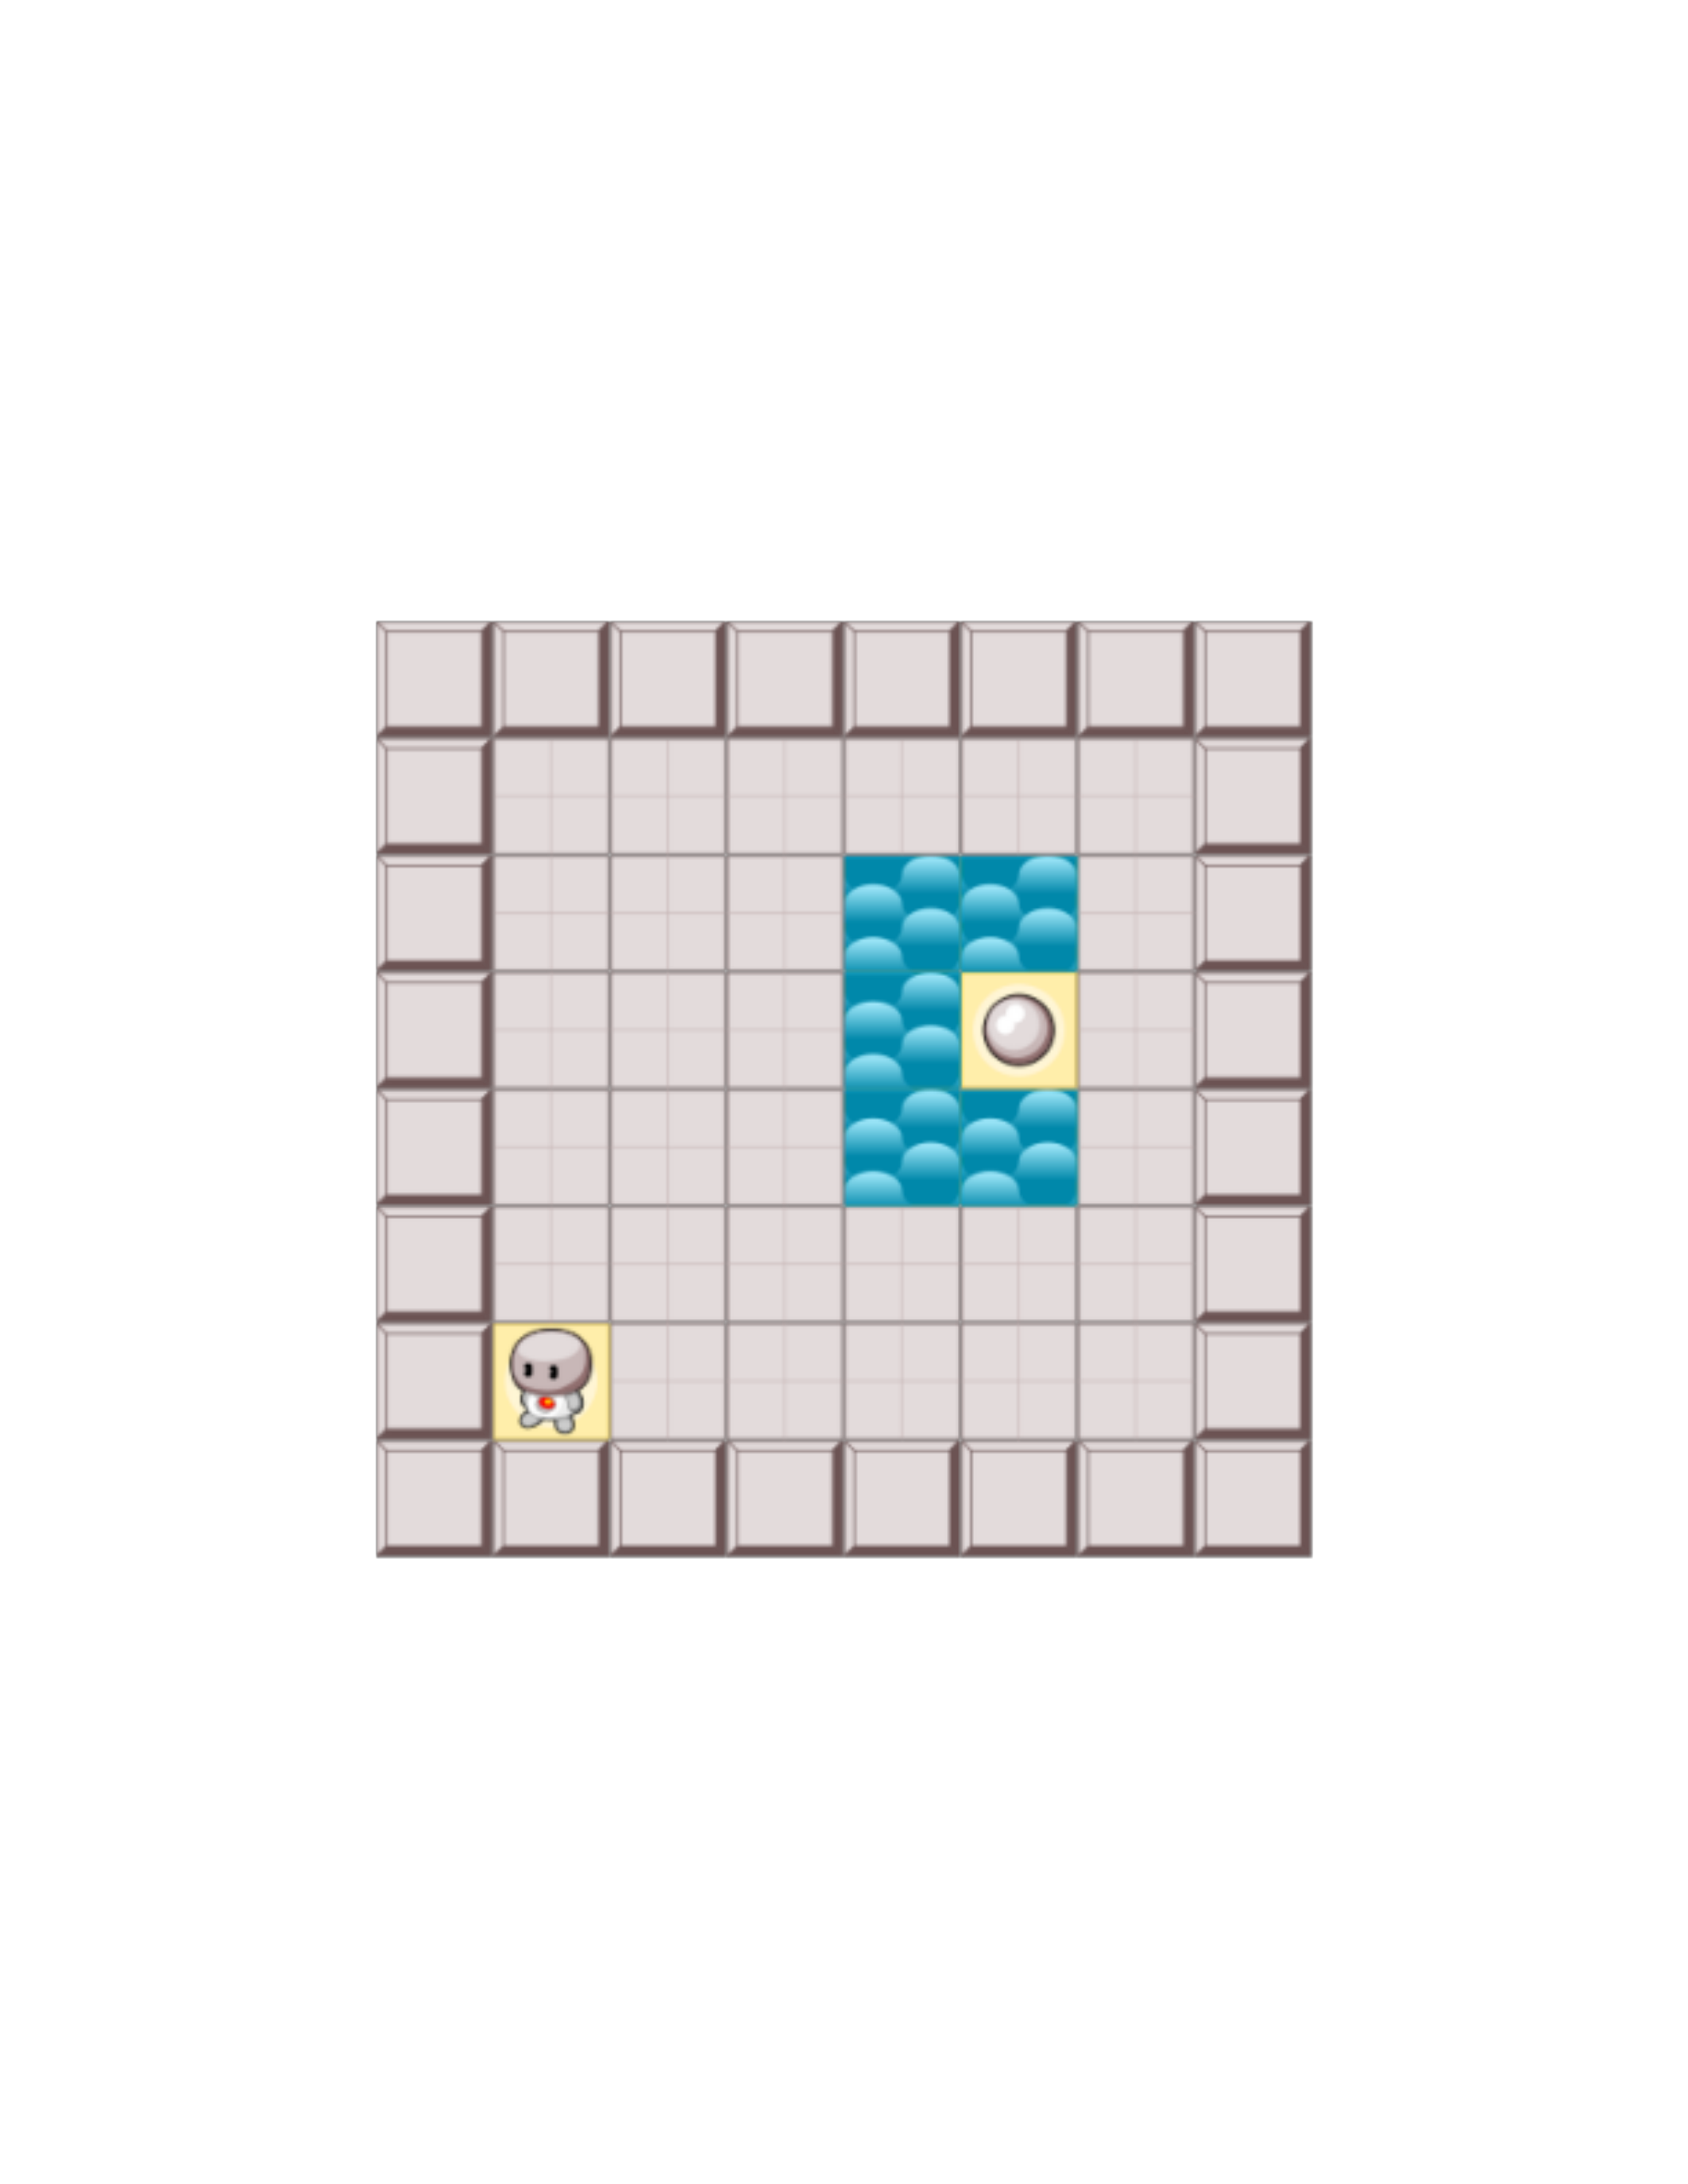}\vspace*{.2cm}
\caption{Environment \\
($r(a,s) = -1$ for water, \\
$r(a,s) = 5$ for goal)}\label{fig:pyco_env2}
\end{subfigure}
\begin{subfigure}{.26\textwidth}
\includegraphics[width=\textwidth]{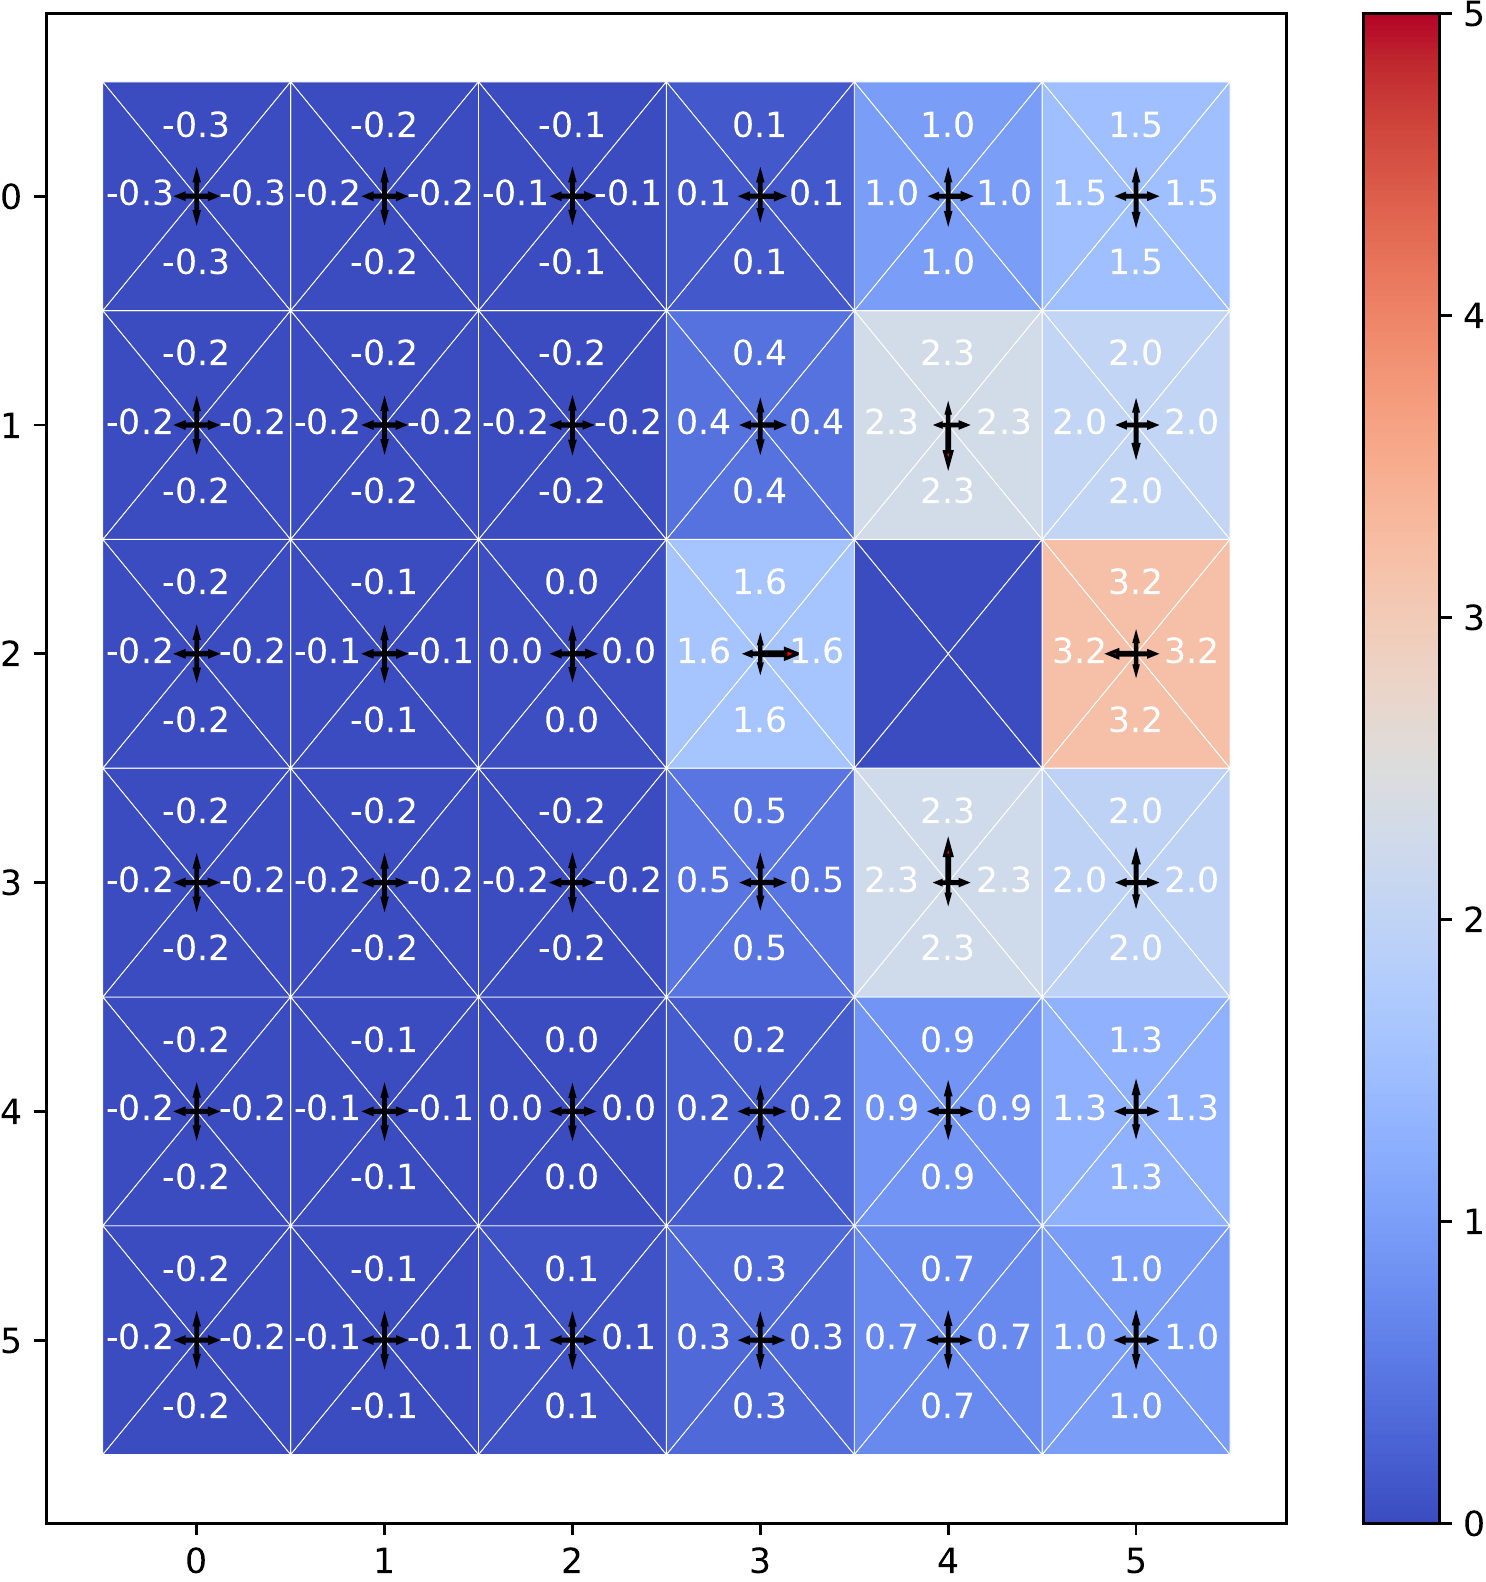}
\caption{$\beta = 0.2$ (High Reg.)}\label{fig:pyco_beta02}
\end{subfigure}
\begin{subfigure}{.26\textwidth}
\includegraphics[width=\textwidth]{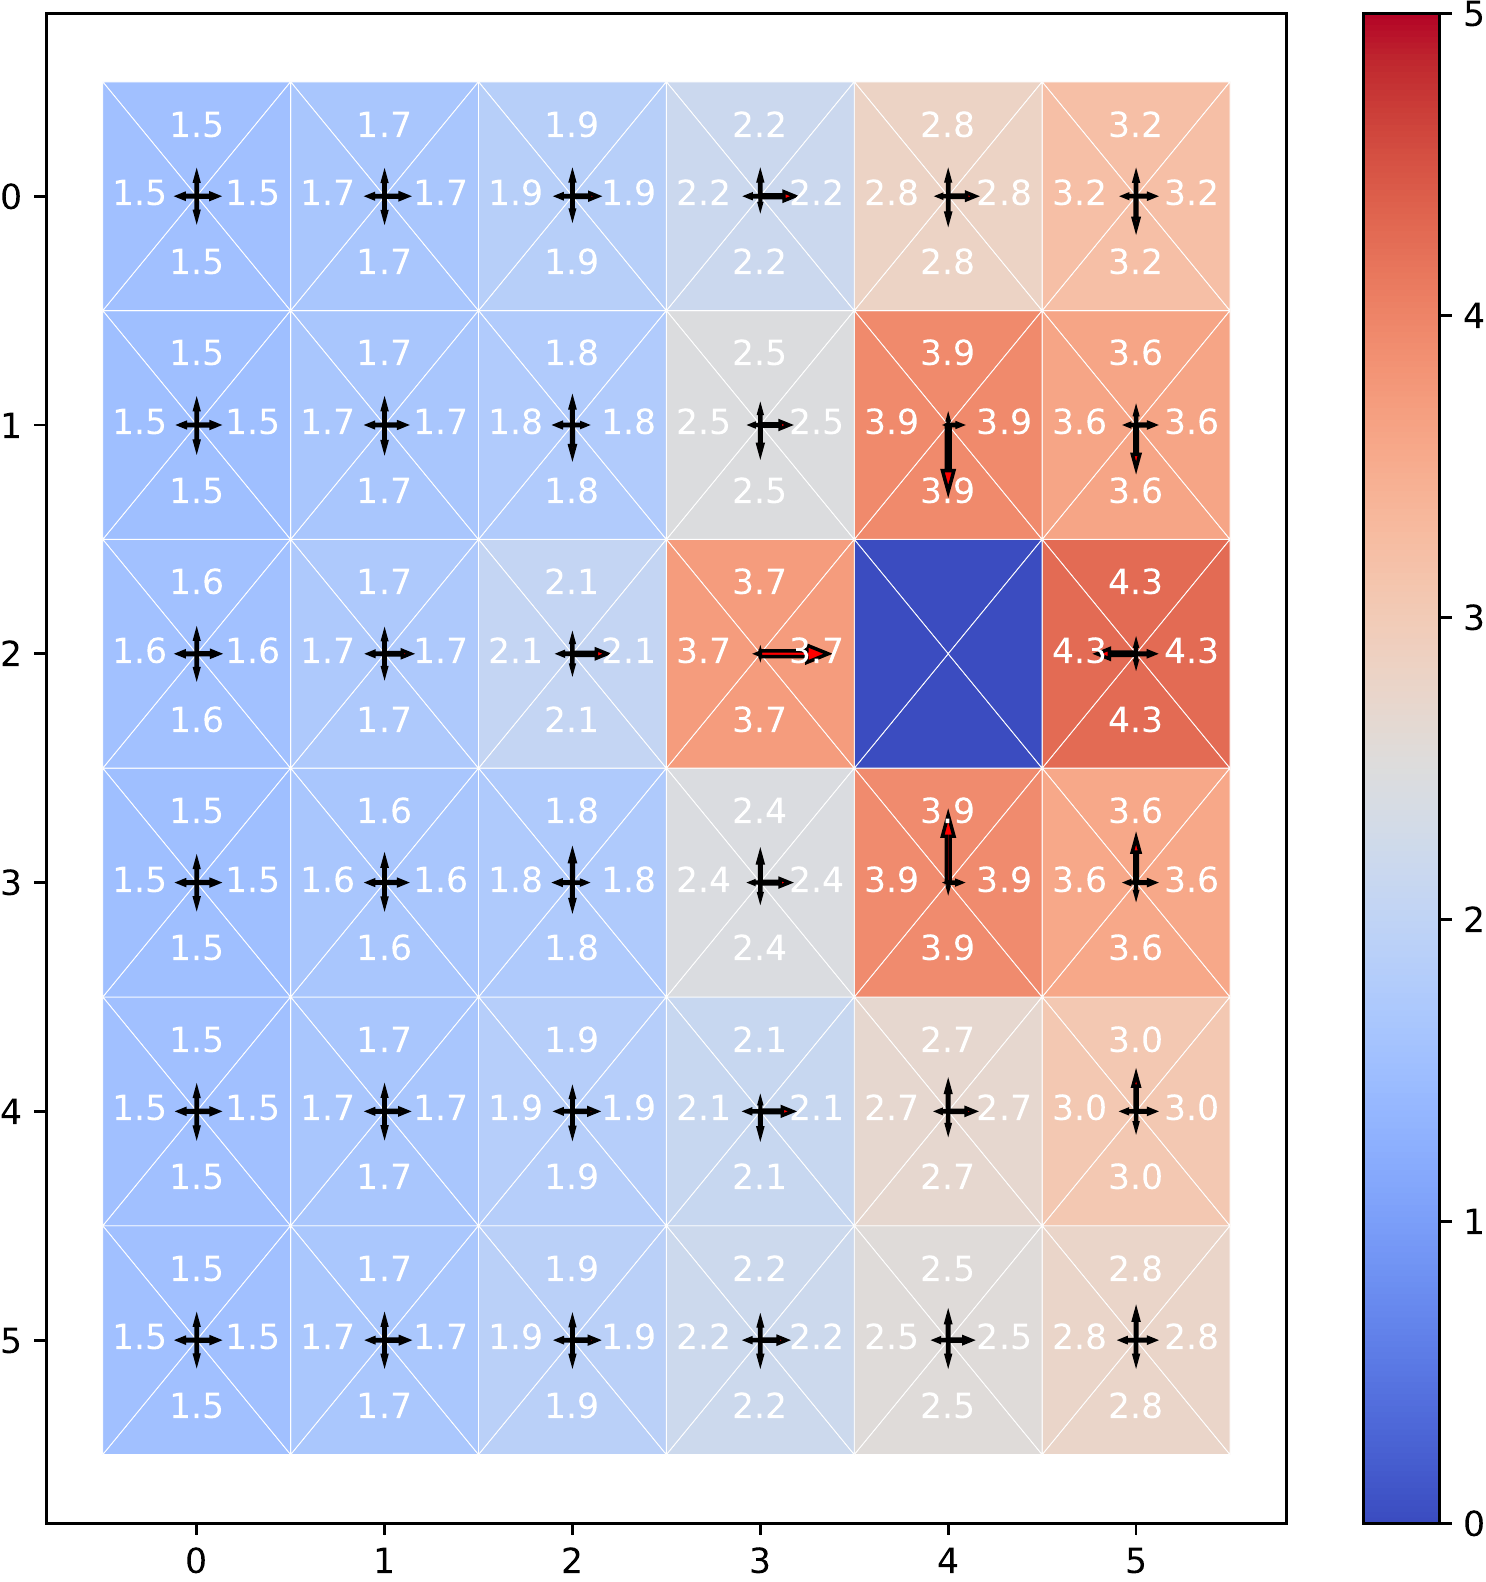}
\caption{$\beta = 1$}\label{fig:pyco_beta1}
\end{subfigure}
\begin{subfigure}{.26\textwidth}
\includegraphics[width=\textwidth]{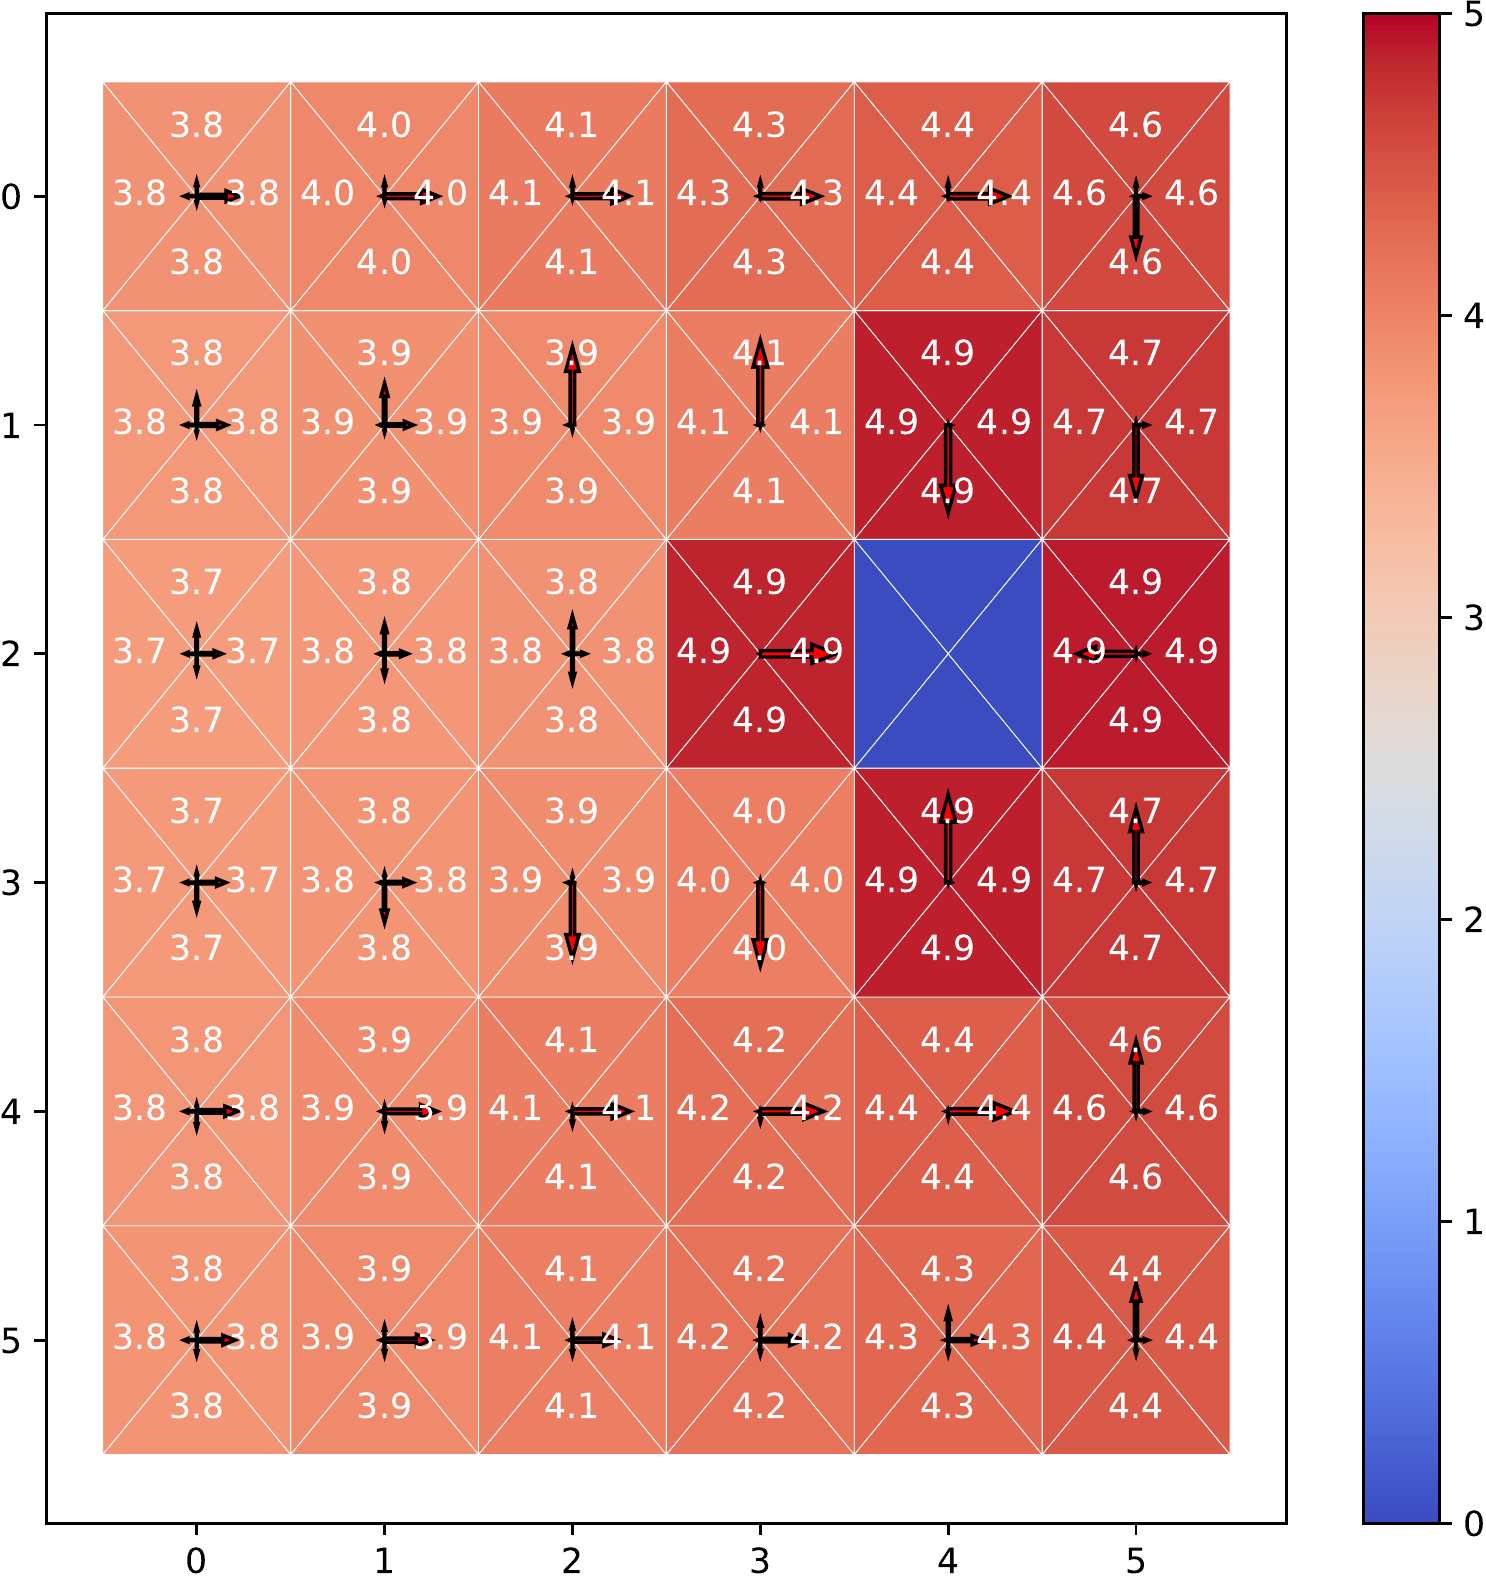}
\caption{$\beta = 10$ (Low Reg.)}\label{fig:pyco_beta02}
\end{subfigure}
\caption{\label{fig:pyco_indifference} \textbf{Confirming Optimality of the Policy.}  We show the perturbed rewards $\mr(a,s) = Q(a,s) - \pr(a,s)$ for policies trained with \textsc{kl} divergence regularization.  The indifference condition holds in all cases, with $\mr(a,s) = c(s)$ for each state-action pair, with $c(s) = V(s)$ for \textsc{kl} regularization.  This confirms that the policy is optimal \citep{ortega2014adversarial, nachum2017bridging}.}
\end{figure*}
