# Supplementary material for: Your Policy Regularizer is Secretly an Adversary
Source: arXiv:2203.12592 source file (2022-07-08)
Supplement: Supplementary file 8 [file psi_comparison.tex]

\begin{figure*}
\begin{minipage}{\textwidth}
\vspace*{-.2cm}
% \begin{subfigure}{0.25\textwidth}\includegraphics[width=\textwidth]{figs/conj_by_alpha_confirm/value_norm_beta01_vert.pdf}
% \caption{$\beta=0.1$}\label{fig:value_agg}\end{subfigure}
\begin{subfigure}{0.24\textwidth}\includegraphics[width=\textwidth]{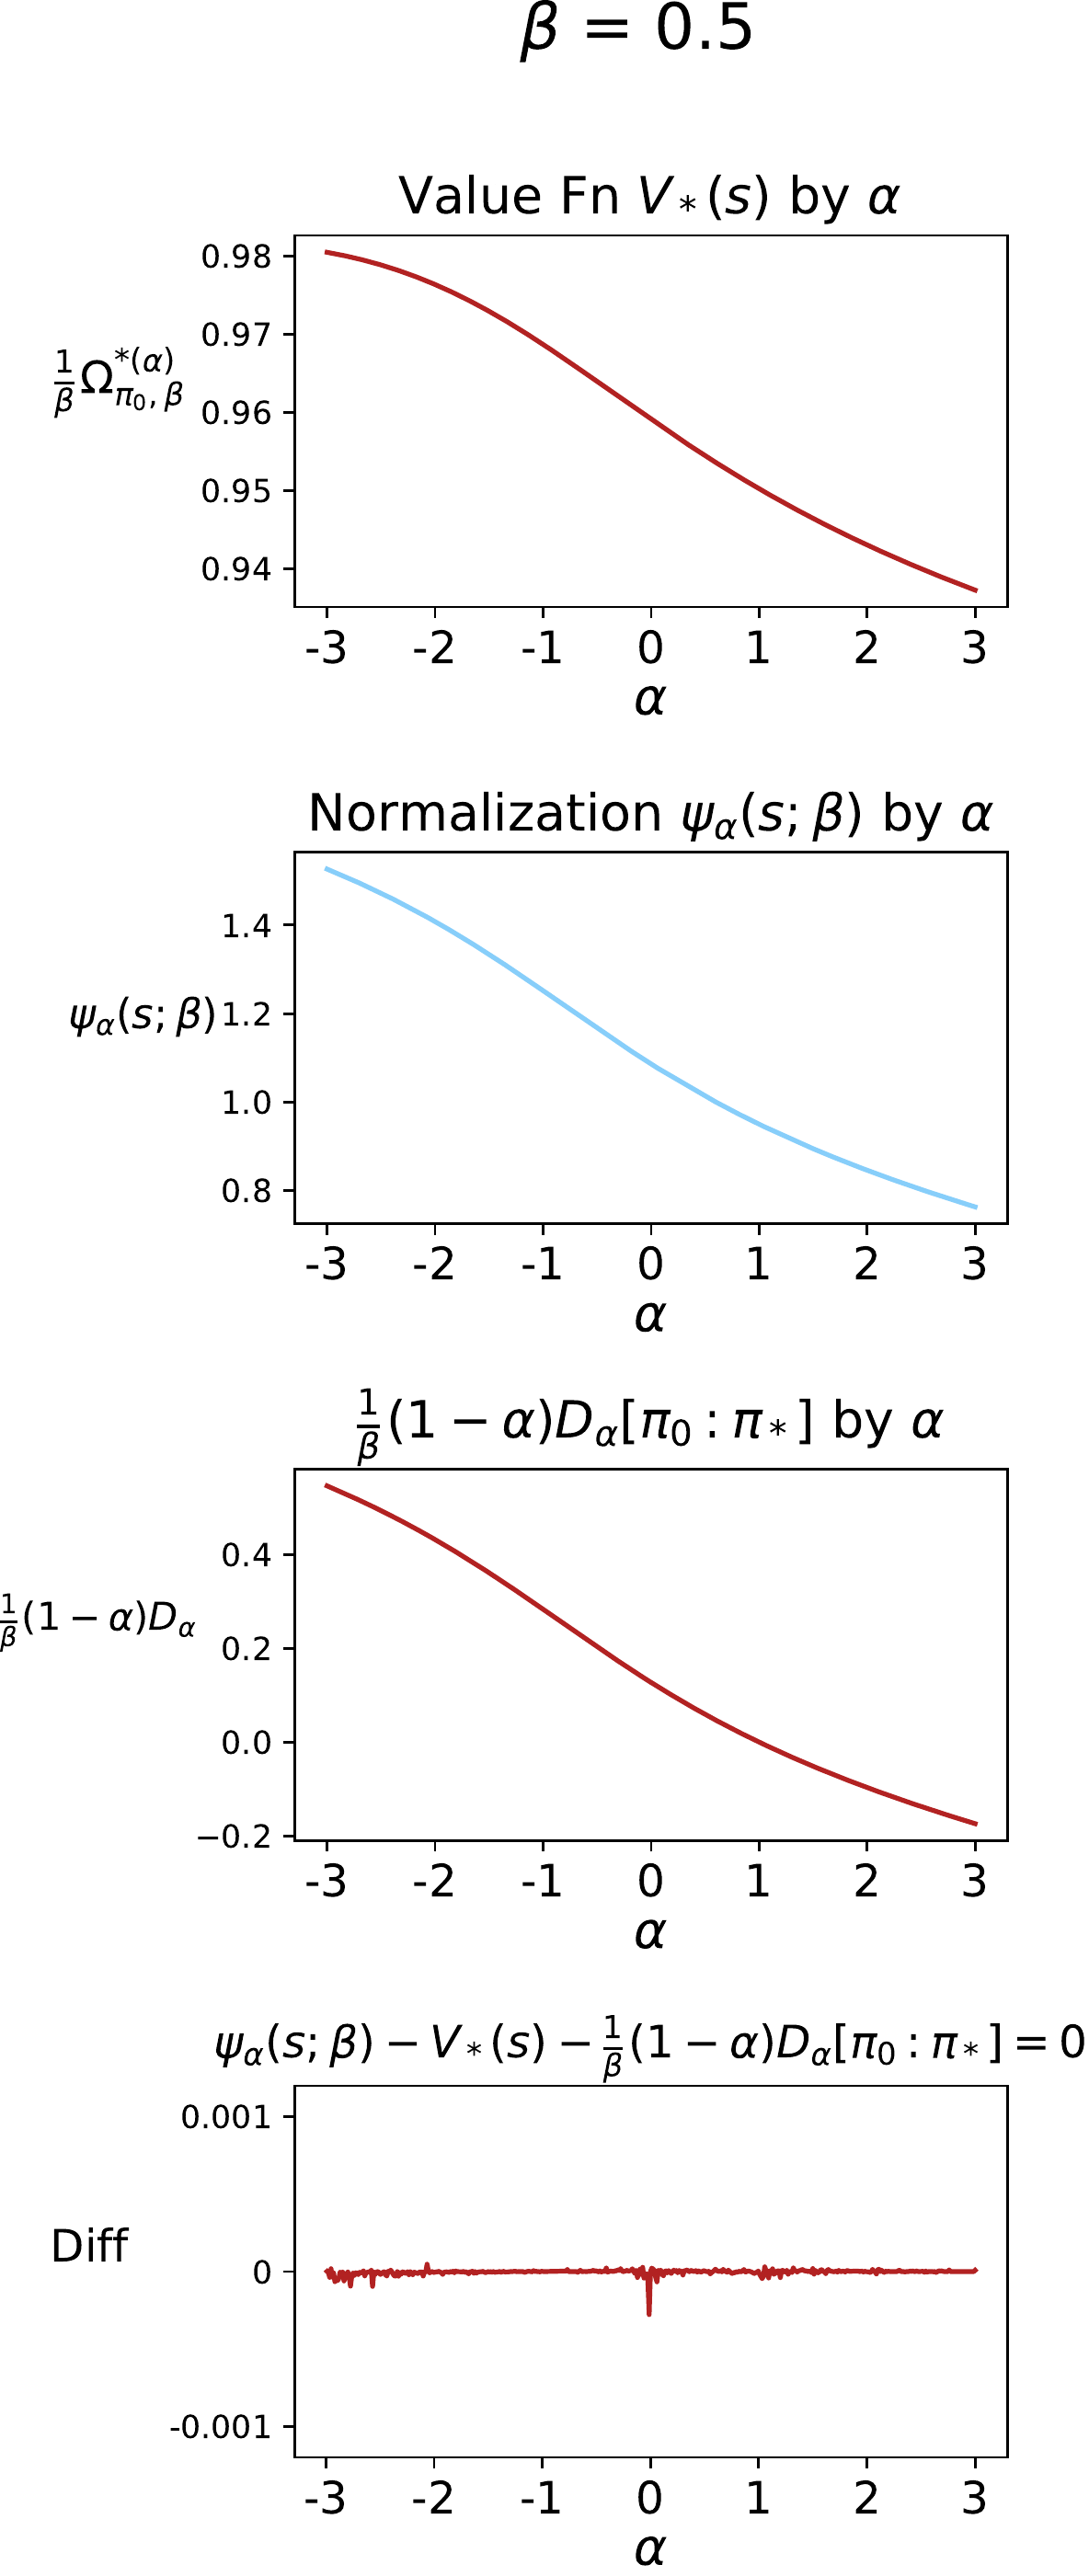}
\caption{$\beta=0.5$}\end{subfigure}
\begin{subfigure}{0.24\textwidth}\includegraphics[width=\textwidth]{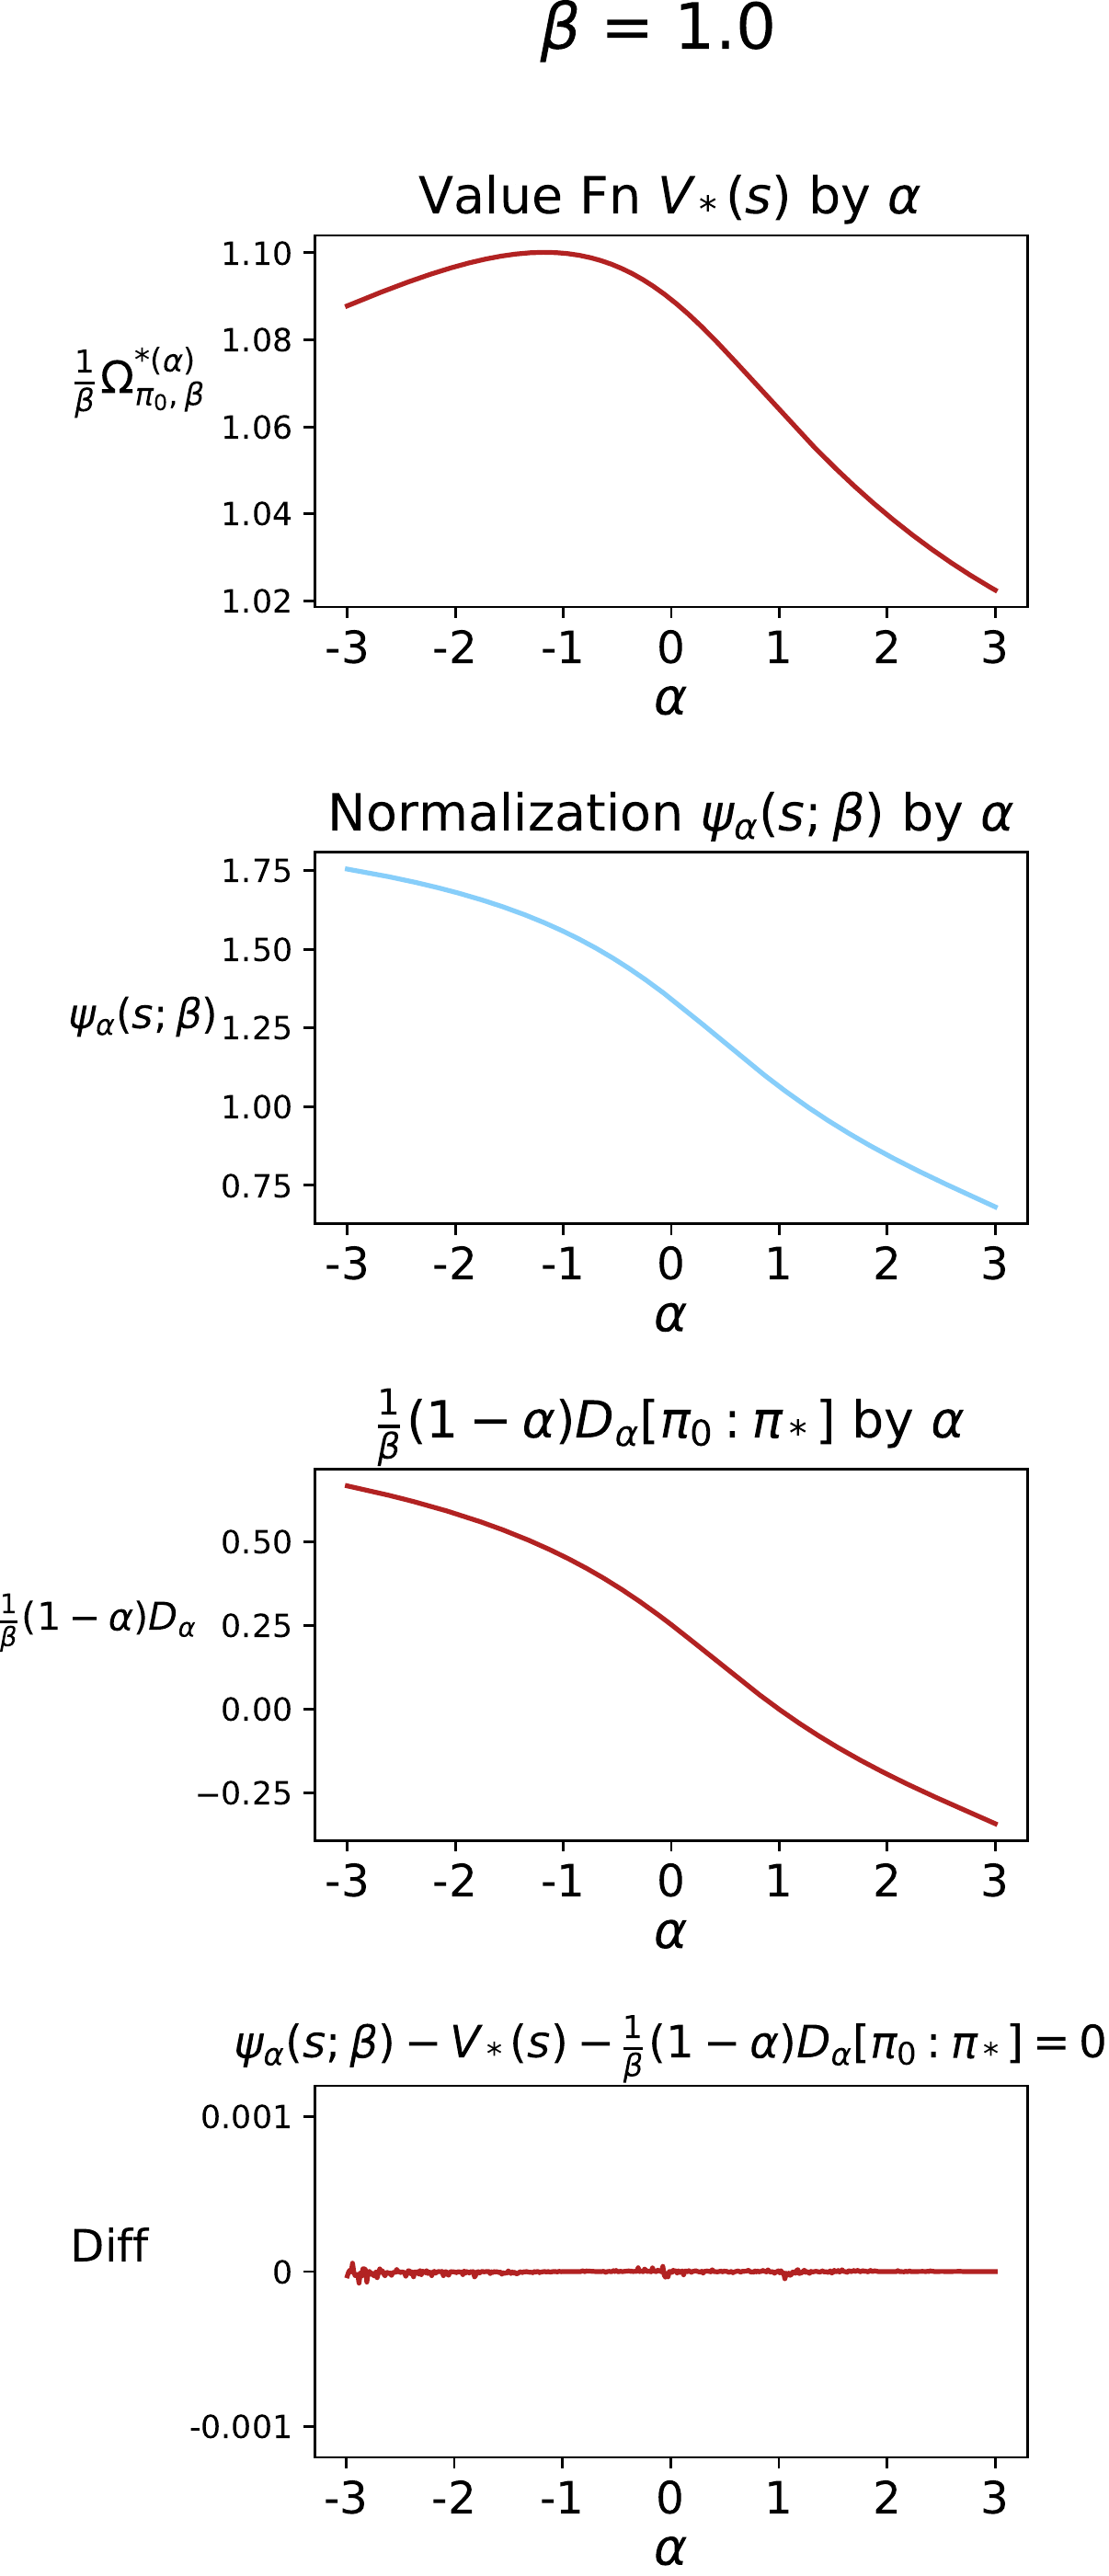}
\caption{$\beta=1$}\end{subfigure}
\begin{subfigure}{0.24\textwidth}\includegraphics[width=\textwidth]{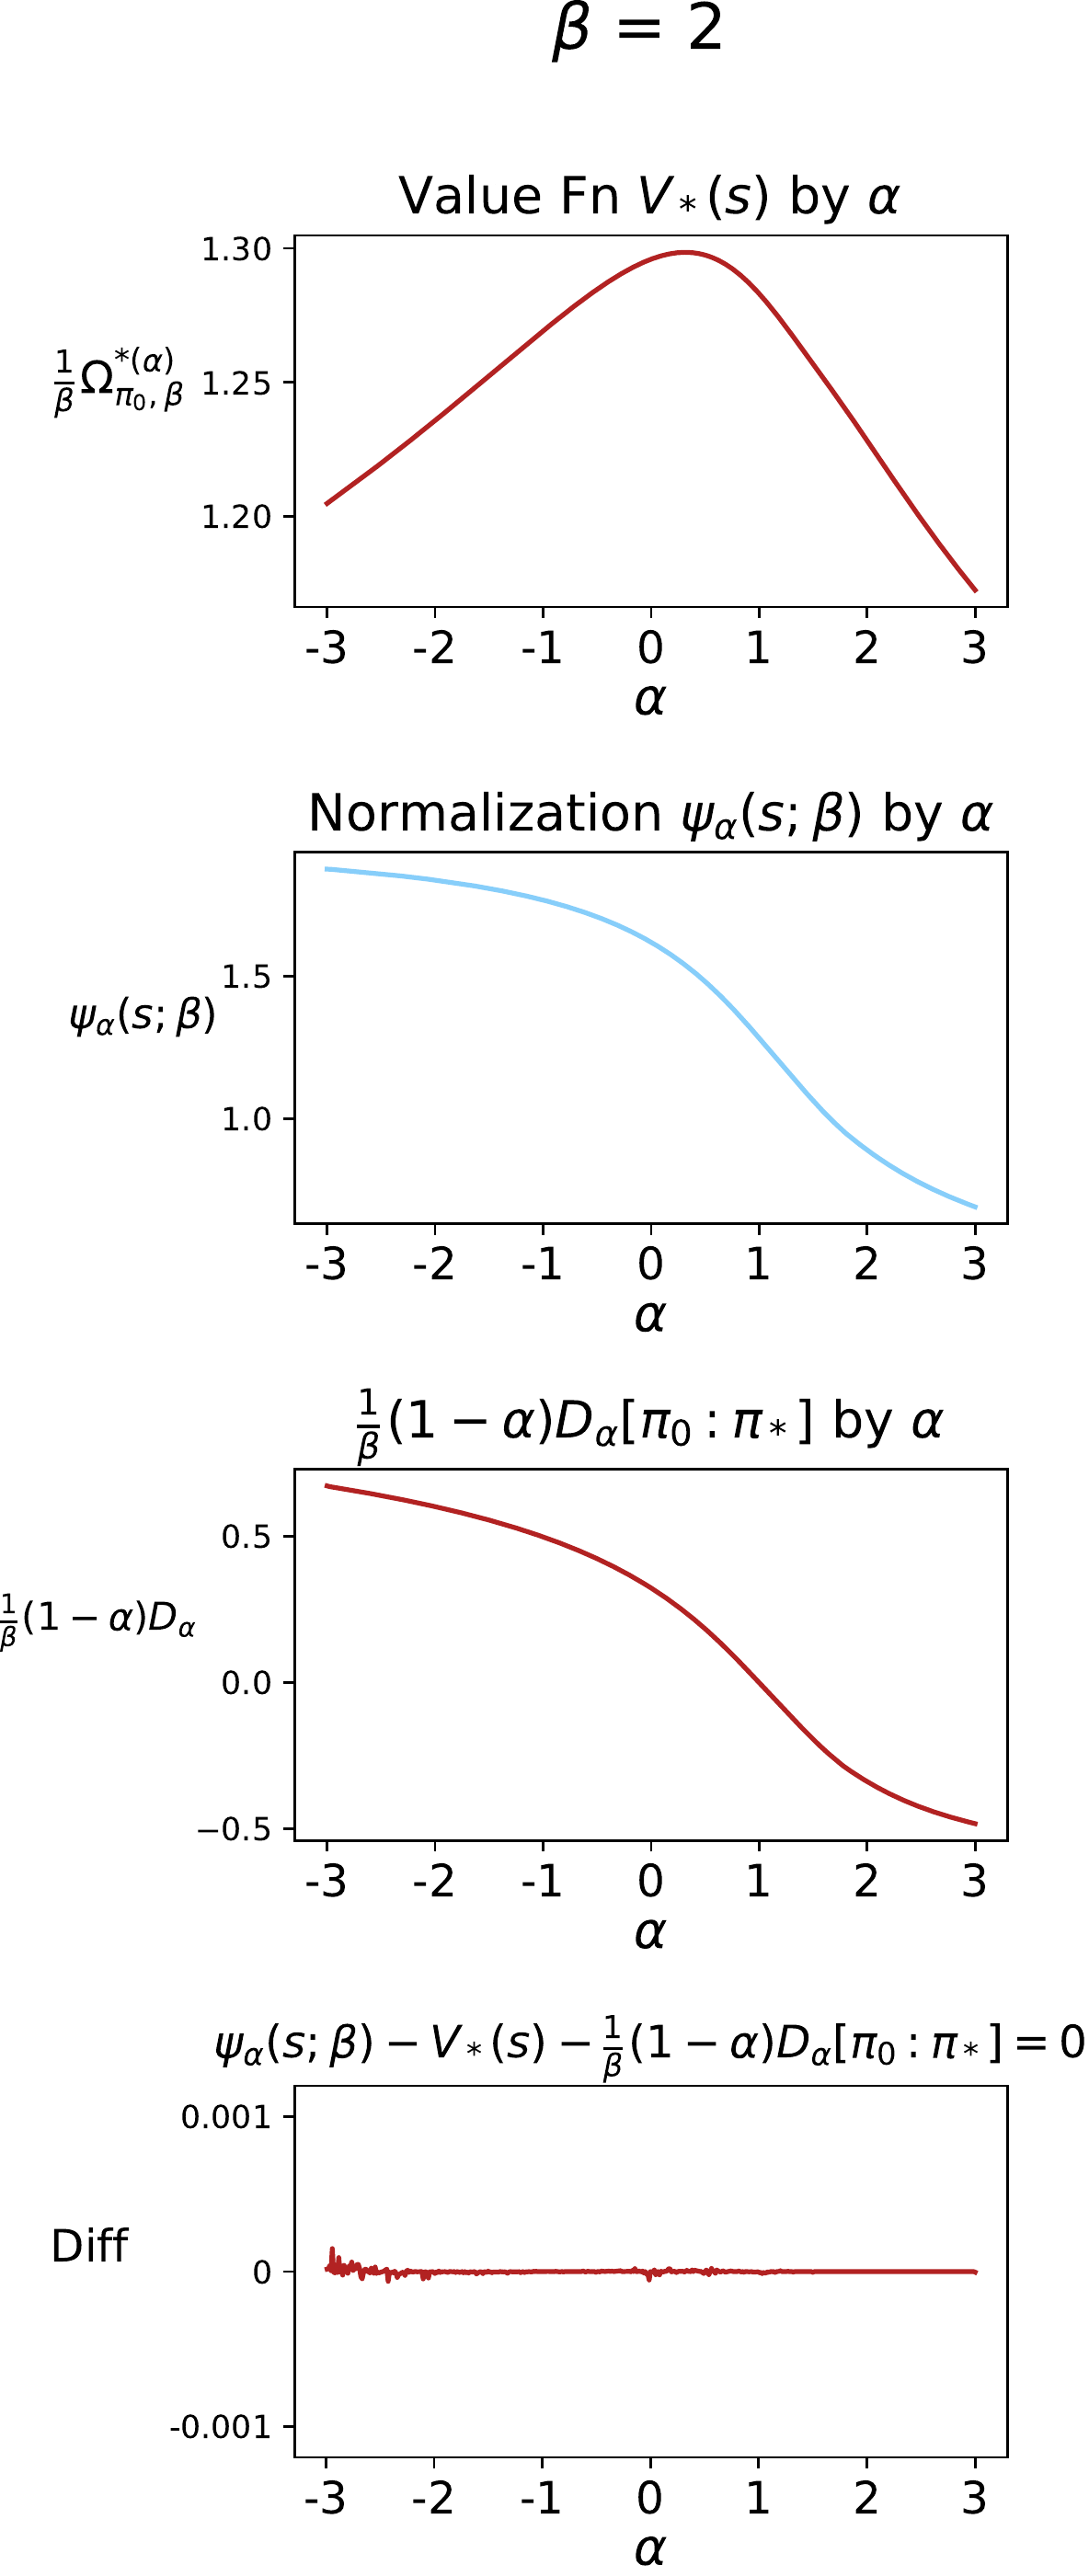}
\caption{$\beta=2$}\end{subfigure}
\begin{subfigure}{0.24\textwidth}\includegraphics[width=\textwidth]{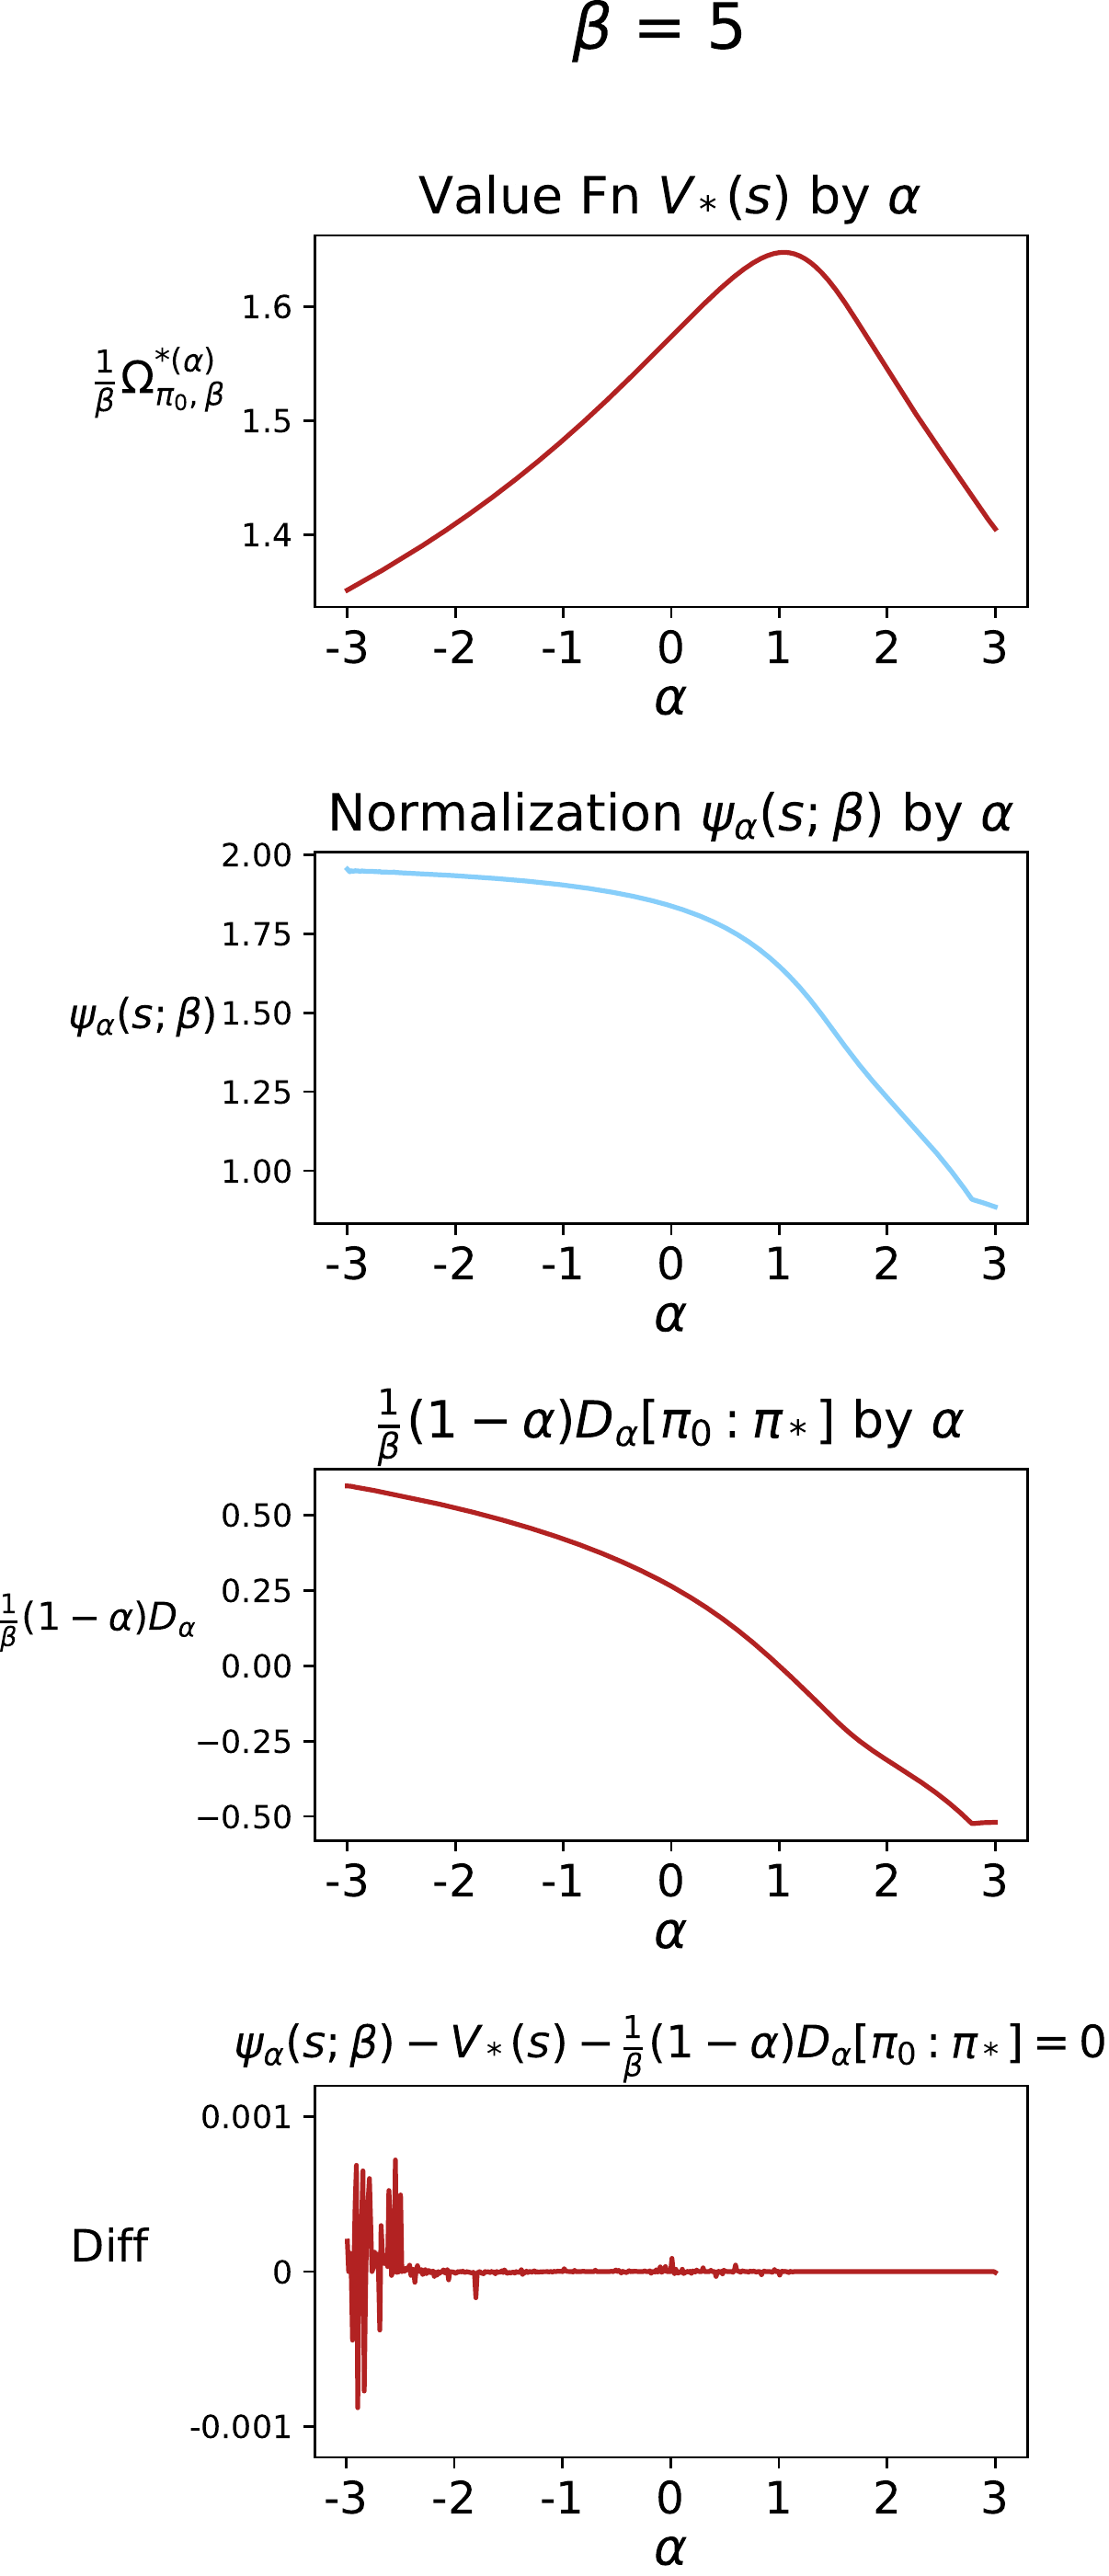}
\caption{$\beta=5$}\end{subfigure}
\caption{ Value Function $V_*(s) = \alphaconjn(Q_*)$ (first row) and Normalization Constant $\psiqopt$ (second row) as a function of $\alpha$ for various regularization strengths $\beta$.   We use the same rewards as in  \myfig{perturb_opt} and \myfig{value_agg_main} and a uniform reference.
We plot $\psipr = \frac{1}{\beta}(1-\alpha)D_{\alpha}[\pi_0:\piopt]$ in the third row, and confirm the identity $V_*(s) = \psiqopt - \psipr$ from \cref{eq:value_and_normalizers} and (\ref{eq:subtractive_relationship}) in the last row.   We find that this equality holds for all $\alpha$ up to small optimization errors on the order of $10^{-3}$.
% Recall that $V(s)= \alphaconjn(Q) = \frac{\alpha-1}{\alpha}   \langle \piopt(a|s), \, Q(a,s)  \rangle   +  \textcolor{red}{\psi_Q(s;\beta)}$ where $\psi_Q(s;\beta)$ is the normalization constant for the optimizing argument $\piopt(a|s) = \pi_0(a|s)[1+(\alpha-1) \beta \big(Q(a,s) - \psi_Q(s;\beta) \big)]_+^{\frac{1}{\alpha-1}}$.  For $\alpha =1$, $V_*(s) = \psi(s;\beta)$ and $\piopt(a|s) = \pi_0(a|s)\exp\{\beta \big(r(a,s) - \normalizerexp \big)\}$. We use the same rewards as in \cref{fig:perturb_opt} and \cref{fig:value_agg_main}.  We emphasize the smaller scale of the $y$-axis in the top row for $V_*(s)$ plots and in the fourth row for confirming \textcolor{red}{$V_*(s) - \normalizeralpha = \frac{1}{\beta}(1-\alpha)D_{\alpha}[\pi_0:\piopt]$.}   We find that this equality holds for all $\alpha$, apart from numerical optimization errors on the order of $10^{-3}$ for $\beta =5$ and $\alpha \approx -3$.
}\label{fig:conj_by_alpha_app}
\end{minipage}
\begin{minipage}{\textwidth}
\vspace*{1cm}
\centering
\begin{subfigure}{0.4\columnwidth}\includegraphics[width=.676\textwidth]{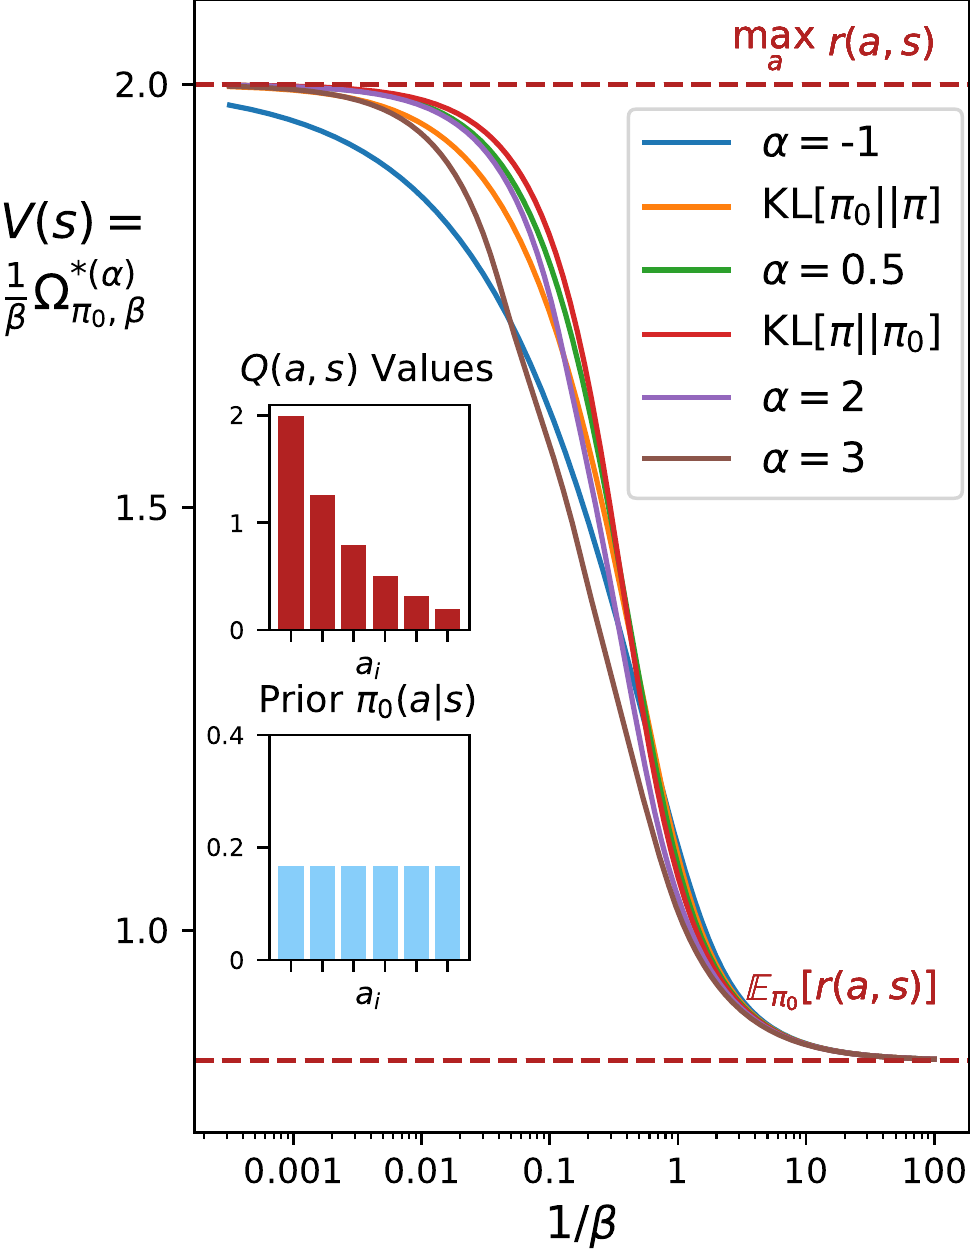}
\caption{Uniform $\pi_0(a|s)$}
% \label{fig:value_agga}
\end{subfigure}\hspace*{.01\columnwidth}
\begin{subfigure}{0.4\columnwidth} 
% \vspace*{-.12cm}\includegraphics[scale=.3]{figs/conj_by_alpha/value_norm_beta1_vert.pdf}
% \vspace*{-.1cm}\includegraphics[width=.96\textwidth]{figs/conj_by_alpha/value_norm_beta1_vert_thin.pdf}
% \caption{$V(s)$ and $\psi_{\alpha}(s)$ as a function of $\alpha$ for $\beta=1$}\label{fig:value_aggb}\end{subfigure}
\vspace*{-.1cm}\includegraphics[width=.676\textwidth]{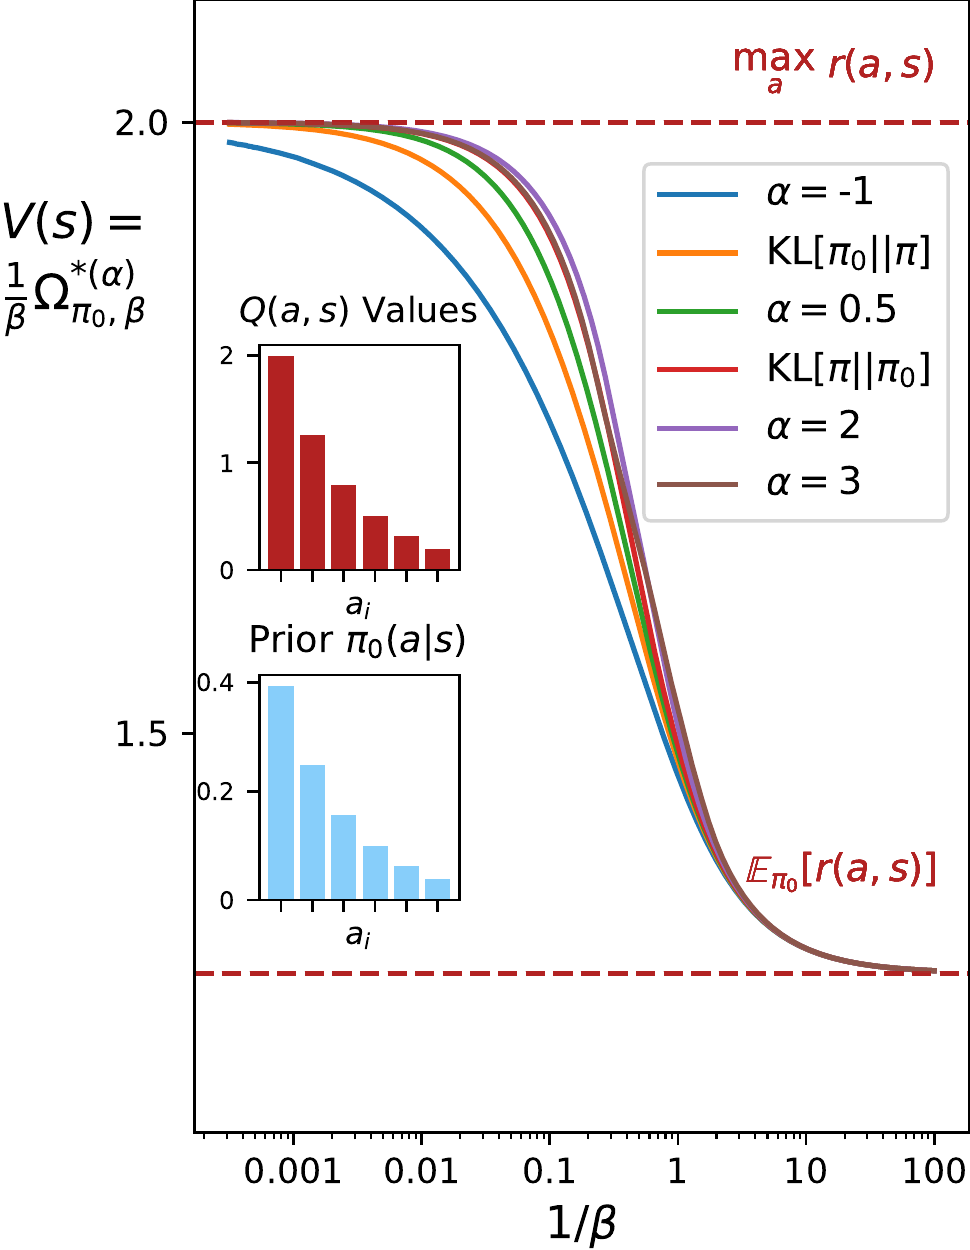}
\caption{$\pi_0(a|s) \propto r(a,s) $}
% \label{fig:value_agga}
\end{subfigure}
\captionof{figure}{Value function $V(s) = \alphaconjm(Q)$ as a function of $\beta$ (x-axis) and $\alpha$ (colored lines), using $Q(a,s)$ and $\pi_0(a|s)$ from the left inset.   See \cref{eq:kl_bellman} and \cref{eq:alpha_bellman} for closed forms.}\label{fig:value_agg_main} %and normalization constant $\psi_{\alpha}(s)$
\end{minipage}
\end{figure*}
