# Supplementary material for: Your Policy Regularizer is Secretly an Adversary
Source: arXiv:2203.12592 source file (2022-07-08)
Supplement: Supplementary file 9 [file value_agg.tex]

\begin{figure}[h]
\centering
\begin{subfigure}{0.4\columnwidth}\includegraphics[width=.676\textwidth]{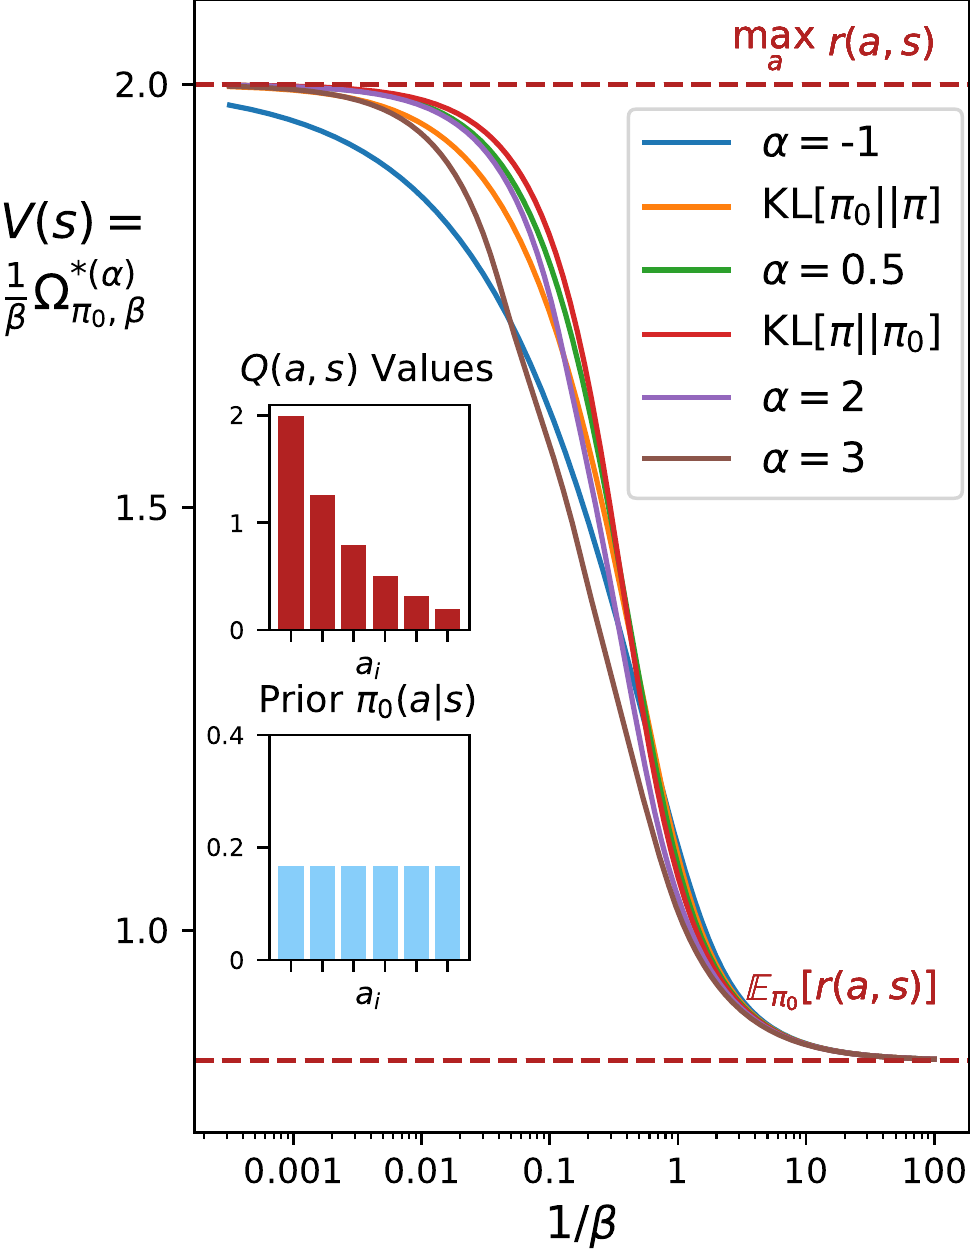}
%\vspace*{.15cm}
\caption{Uniform $\pi_0(a|s)$}\label{fig:value_agga}\end{subfigure}\hspace*{.01\columnwidth}
\begin{subfigure}{0.4\columnwidth} 
% \vspace*{-.12cm}\includegraphics[scale=.3]{figs/conj_by_alpha/value_norm_beta1_vert.pdf}
% \vspace*{-.1cm}\includegraphics[width=.96\textwidth]{figs/conj_by_alpha/value_norm_beta1_vert_thin.pdf}
% \caption{$V(s)$ and $\psi_{\alpha}(s)$ as a function of $\alpha$ for $\beta=1$}\label{fig:value_aggb}\end{subfigure}
\vspace*{-.1cm}\includegraphics[width=.676\textwidth]{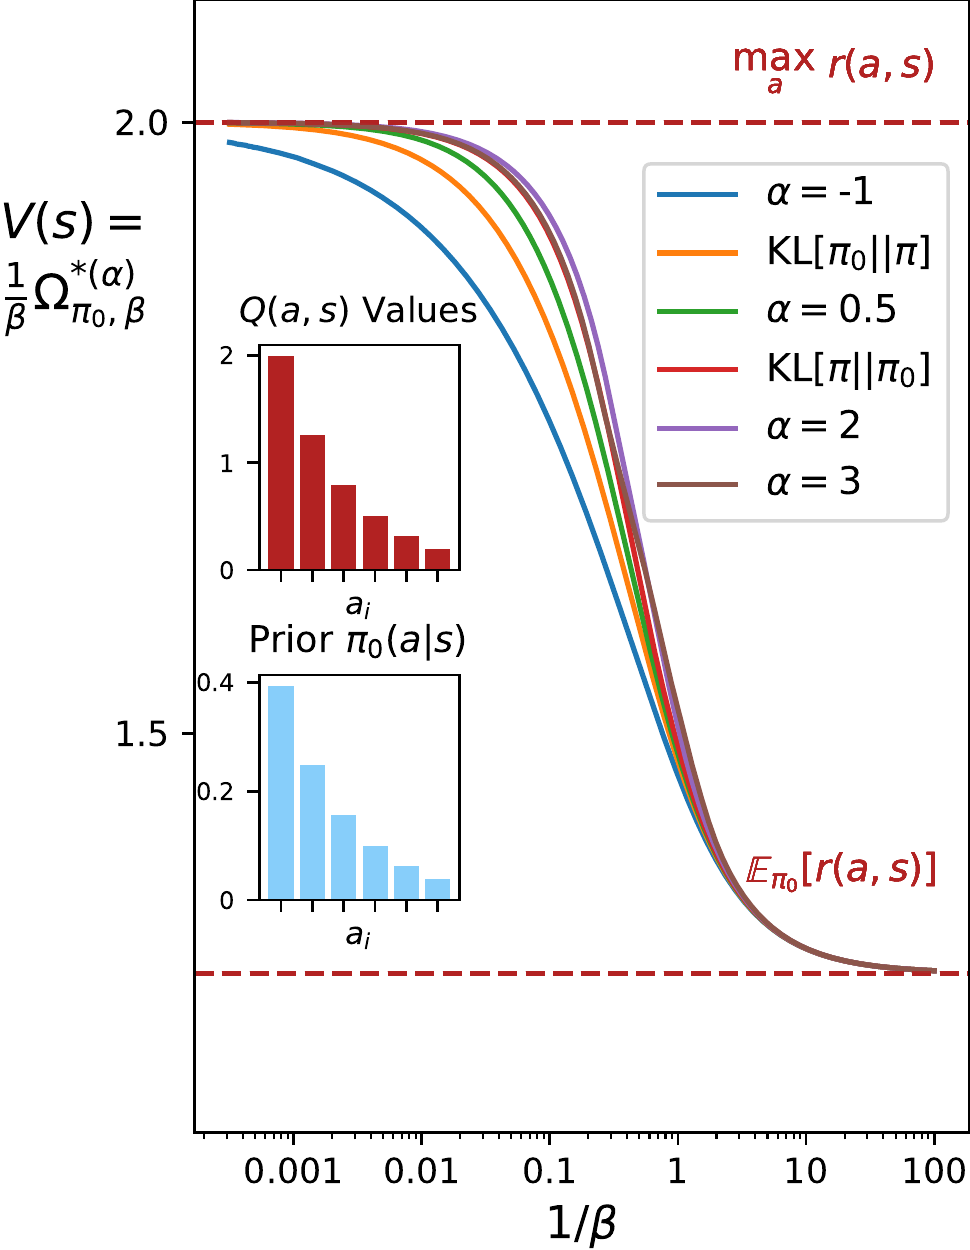}
\caption{$\pi_0(a|s) \propto r(a,s) $}\label{fig:value_agga}
\end{subfigure}
\caption{Value function $V(s) = \alphaconjm(Q)$ as a function of $\beta$ (x-axis) and $\alpha$ (colored lines), using $Q(a,s)$ and $\pi_0(a|s)$ from the left inset.   See \cref{eq:kl_bellman} and \cref{eq:alpha_bellman} for closed forms. }\label{fig:value_agg_main} %and normalization constant $\psi_{\alpha}(s)$
\end{figure}
