# Supplementary material for: Your Policy Regularizer is Secretly an Adversary
Source: arXiv:2203.12592 source file (2022-07-08)
Supplement: Supplementary file 11 [file 1_normalized_mu.tex]

\section{Bellman Flow Constraints Imply Normalized $\mu(a,s)$}\label{app:normalized_mu}
In this section, we show that a state-action occupancy measure which satisfies the Bellman flow constraints is normalized as a joint distribution, assuming that the initial state $\nu_0(s)$ and transition $P(s\tick|a,s)$ distributions are normalized.   More formally, if $\sum_s \nu_0(s) = 1$ and $\sum_{s\tick} P(s\tick|a,s) = 1$  $\forall a \in \mathcal{A},s \in \mathcal{S}$, then $\mu(a,s) \in \mathcal{M} \implies \mu(a,s) \in \Delta^{|\mathcal{A}| \times |\mathcal{S}|}$.

Starting from the Bellman flow constraints
\begin{align}
    \sum \limits_{a} \mu(a,s) = (1-\gamma) \nu_0(s) + \gamma \sum \limits_{a\tick,s\tick} P(s|a\tick,s\tick) \mu(a\tick, s\tick)
\end{align}
we consider taking the summation over states $s \in \mathcal{S}$,
\begin{align}
       \sum \limits_{a, s} \mu(a,s) &= (1-\gamma) \sum \limits_{s} \nu_0(s) + \gamma \sum \limits_{s} \sum \limits_{a\tick,s\tick} P(s|a\tick,s\tick) \mu(a\tick, s\tick) \\
       \sum \limits_{a, s} \mu(a,s) &\overset{(1)}{=} (1-\gamma) \cdot 1 + \gamma \sum \limits_{s} P(s|a\tick,s\tick) \sum \limits_{a\tick,s\tick}  \mu(a\tick, s\tick) \\
        \sum \limits_{a, s} \mu(a,s) &\overset{(2)}{=} (1-\gamma) \cdot 1 + \gamma \sum \limits_{a\tick,s\tick}  \mu(a\tick, s\tick) 
\end{align}
where $(1)$ uses the normalization assumption on $\nu_0(s)$ and the distributive law, and $(2)$ uses the normalization assumption on $P(s|a\tick,s\tick)$.  Finally, we rearrange to obtain
\begin{align}
  (1-\gamma)  \sum \limits_{a, s} \mu(a,s)  = (1-\gamma) \quad \implies \quad \sum \limits_{a, s} \mu(a,s) = 1
\end{align}
which shows that $\mu(a,s)$ is normalized as a joint distribution over $a \in \mathcal{A},s \in \mathcal{S}$, as desired.

% ($\mu(a,s) \in \mathcal{M}$) is normalized as a joint distribution over states and actions ($\mu(a,s) \in \Delta^{|\mathcal{A}| \times |\mathcal{S}|}$).   a normalized initial state distribution $\nu_0(\vz)$
