# Supplementary material for: Your Policy Regularizer is Secretly an Adversary
Source: arXiv:2203.12592 source file (2022-07-08)
Supplement: Supplementary file 12 [file 1_reg_mu.tex]

\section{Regularizing the Joint State-Action Occupancy Measure $\mu(a,s)$}\label{app:mu_results}

\begin{align}
    \alphaconjm &= \max \limits_{\mu} \blangle \mu(a,s), \pr(a,s) \brangle - \alphaomegamu \label{eq:conj_mu} \\
    &= \frac{1}{\beta}\frac{1}{\alpha} \sum \limits_{a,s} \mu_0(a,s)\big[1+\beta(\alpha-1)\pr(a,s)\big]^{\frac{\alpha}{\alpha-1}} - \frac{1}{\beta}\frac{1}{\alpha} \sum \limits_{a,s}\mu_0(a,s) \label{eq:conj_mu_result}
\end{align}

Result
\begin{align}
    \alphaconjm &= \frac{1}{\beta}\frac{1}{\alpha} \sum \limits_{a,s} \mu_0(a,s)\big[1+\beta(\alpha-1)\pr(a,s)\big]^{\frac{\alpha}{\alpha-1}} - \frac{1}{\beta}\frac{1}{\alpha} \sum \limits_{a,s}\mu_0(a,s) \label{eq:conj_mu_result}
\end{align}

\begin{align}
    % \alphaconjm &= \max \limits_{\mu} \blangle \mu(a,s), \pr(a,s) \brangle - \alphaomegamu \\
    \pr(a,s) &= \frac{1}{\beta} \frac{1}{\alpha(1-\alpha)} \nabla_{\mu} \left( (1-\alpha) \sum \limits_{a,s} \mu_0(a,s) + \alpha \sum \limits_{a,s} \mu(a,s) - \sum \limits_{a,s} \mu_0(a,s)^{1-\alpha} \mu(a,s)^{\alpha} \right) \\
    &= \frac{1}{\beta} \frac{1}{1-\alpha} - \frac{1}{\beta} \frac{1}{1-\alpha} \mu_0(a,s)^{1-\alpha} \mu(a,s)^{\alpha-1} \\
    \implies \mu_{\pr}(a,s) &= \mu_0(a,s) [1 + \beta(1-\alpha)\pr(a,s)]^{ \frac{1}{\alpha-1}}
\end{align}
Plugging this back into the conjugate function \cref{eq:conj_mu},
\footnotesize
\begin{align}
    \alphaconjm &= \blangle \mu_{\pr}(a,s), \pr(a,s) \brangle - \frac{1}{\beta} \frac{1}{\alpha(1-\alpha)}\bigg( (1-\alpha) \sum \limits_{a,s} \mu_0(a,s) + \alpha \sum \limits_{a,s} \mu_{\pr}(a,s)  - \sum \limits_{a,s} \mu_{\pr}(a,s)  \underbrace{\left(\frac{\mu_{\pr}(a,s) }{\mu_0(a,s)}\right)^{\alpha-1}}_{1 + \beta(\alpha-1) \pr(a,s)} \bigg) \nonumber \\
    &= \left(1- \frac{1}{\alpha} \right) \blangle \mu_{\pr}(a,s), \pr(a,s) \brangle - \frac{1}{\beta} \frac{1}{\alpha}\sum \limits_{a,s} \mu_0(a,s) +  \left( \frac{1}{\beta}\frac{1}{\alpha(1-\alpha)} - \frac{1}{\beta}\frac{1}{1-\alpha} \right) \sum \limits_{a,s} \mu_{\pr}(a,s) \\
    &= \text{ \footnotesize $\frac{\alpha -1}{\alpha}  \blangle \mu_{0}(a,s)
    \big[1+\beta(\alpha-1)\pr(a,s)\big]^{\frac{1}{\alpha-1}}, \pr(a,s) \brangle + \frac{1}{\beta} \frac{1}{\alpha} \sum \limits_{a,s} \mu_{0}(a,s)\big[1+\beta(\alpha-1)\pr(a,s)\big]^{\frac{1}{\alpha-1}} - \frac{1}{\beta} \frac{1}{\alpha} \sum \limits_{a,s} \mu_{0}(a,s)$} \nonumber \\
    % &= \frac{\alpha -1}{\alpha}  \blangle \mu_{0}(a,s)[1+\beta(\alpha-1)\pr(a,s)]^{\frac{1}{\alpha-1}}, \pr(a,s) \brangle \\[1.5ex]
    % &\phantom{====} + \frac{1}{\beta} \frac{1}{\alpha} \sum \limits_{a,s} \mu_{0}(a,s)[1+\beta(\alpha-1)\pr(a,s)]^{\frac{1}{\alpha-1}} - \frac{1}{\beta} \frac{1}{\alpha} \sum \limits_{a,s} \mu_{0}(a,s) \nonumber \\
    &=  \sum \limits_{a,s} \mu_0(a,s)\mu_{0}(a,s)\big[1+\beta(\alpha-1)\pr(a,s)\big]^{\frac{1}{\alpha-1}}\cdot \frac{1}{\beta}\frac{1}{\alpha} \big( 1 + \beta (\alpha-1) \pr(a,s) \big) - \frac{1}{\beta}\frac{1}{\alpha} \sum \limits_{a,s}\mu_0(a,s) \\
    &=  \frac{1}{\beta}\frac{1}{\alpha} \sum \limits_{a,s} \mu_0(a,s)\big[1+\beta(\alpha-1)\pr(a,s)\big]^{\frac{\alpha}{\alpha-1}} - \frac{1}{\beta}\frac{1}{\alpha} \sum \limits_{a,s}\mu_0(a,s)
\end{align}
\normalsize
where, in the last line, note that $\frac{1}{\alpha-1}+1=\frac{\alpha}{\alpha-1}$.

\subsection{KL Divergence Conjugate with $\mu(a,s)$ Optimization}\label{app:kl_mu}
\begin{restateable} 
The conjugate function for \kl divergence regularization of the state-action occupancy $\mu(a,s)$ to a reference $\mu_0(a,s)$ has the following closed form.
\begin{align}
    \frac{1}{\beta} \Omega^{*}(\pr) &= \frac{1}{\beta} \sum \limits_{a,s} \mu(s)\pi_0(a|s) \expof{\beta \cdot \pr(a,s)}  - \frac{1}{\beta} \sum \limits_{a,s} \mu(s) \pi_0(a|s)
\end{align}
\end{restateable}

\begin{align}
    \frac{1}{\beta} \Omega^{*}(\pr) = \max \limits_{\mu(a,s)} \blangle \mu(a,s), \pr(a,s) \brangle - \frac{1}{\beta} \blangle \mu(a,s) \log \frac{\mu(a,s)}{\mu(s) \pi_0(a|s)} \brangle + \frac{1}{\beta} \sum \limits_{a,s} \mu(a,s) - \frac{1}{\beta} \sum \limits_{a,s} \mu(s) \pi_0(a|s)
\end{align}

\begin{align}
    \pr(a,s) &\overset{(1)}{=} \frac{1}{\beta} \log \frac{\mu(a,s)}{\mu(s) \pi_0(a|s)} - \frac{1}{\beta}  
    % \sum \limits_{a,s} \frac{d \mu(a,s)}{d \mu(a^\prime, s^\prime)} 
    + \frac{1}{\beta}  \sum \limits_{a,s} \frac{\mu(a,s)}{\mu(s)} \underbrace{ 
    \frac{d \sum_{a^{\prime\prime}} \mu(a^{\prime\prime},s)}{d \mu(a^\prime, s^\prime)}}
    _{\delta(s=s^{\prime})} 
    + \frac{1}{\beta} -  \frac{1}{\beta}  \sum \limits_{a,s}  
    \underbrace{
    \frac{d \sum_{a^{\prime\prime}} \mu(a^{\prime\prime},s)}{d \mu(a^\prime, s^\prime)}
    }_{\delta(s=s^{\prime})} \pi_0(a|s) \\
    &= \frac{1}{\beta} \log \frac{\mu(a,s)}{\mu(s) \pi_0(a|s)} +  \frac{1}{\beta}  \sum \limits_{a} \frac{\mu(a,s)}{\mu(s)}  
    % \textcolor{red}{\pi(a|s) \footnote{Notation?}}
    - \frac{1}{\beta} \sum \limits_{a} \pi_0(a|s) \\
     &\overset{(2)}{=} \frac{1}{\beta} \log \frac{\mu(a,s)}{\mu(s) \pi_0(a|s)} 
\end{align}
where in $(1)$ we take care to differentiate $\mu(s)$ with respect to $\mu(a,s)$.
In $(2)$ we assume that $\sum_a \pi_0(a|s) = 1$ and note that $\sum_a \frac{\mu(a,s)}{\mu(s)} = \frac{\sum_a \mu(a,s)}{\mu(s)} = \frac{\mu(s)}{\mu(s)} =1 $.

\textcolor{red}{Defining $\pi_{\pr}(a|s) = \frac{\mu(a,s)}{\mu(s)}$},
\begin{align}
    \pi_{\pr}(a|s) = \pi_0(a|s) \expof{\beta \cdot \pr(a,s)}
\end{align}
Plugging this back into the conjugate optimization, we have
\begin{align}
    \frac{1}{\beta} \Omega^{*}(\pr) &=  \blangle \mu(s) \pi_{\pr}(a,s), \pr(a,s) \brangle - \frac{1}{\beta} \blangle \mu(s) \pr(a,s) 
\cancel{\log \exp} \{ \beta \cdot \pr(a,s) \} \brangle \\
&\phantom{= \mu(s) \pr(a,s), \pr(a,s) \pr(} + \frac{1}{\beta} \sum \limits_{a,s} \mu(s)\pi_0(a|s) \expof{\beta \cdot \pr(a,s)}  - \frac{1}{\beta} \sum \limits_{a,s} \mu(s) \pi_0(a|s) \nonumber \\
&= \frac{1}{\beta} \sum \limits_{a,s} \mu(s)\pi_0(a|s) \expof{\beta \cdot \pr(a,s)}  - \frac{1}{\beta} \sum \limits_{a,s} \mu(s) \pi_0(a|s)
\end{align}

\subsection{Feasible Set for State-Action Occupancy Regularization}\label{app:mu_feasible}
