# Supplementary material for: Your Policy Regularizer is Secretly an Adversary
Source: arXiv:2203.12592 source file (2022-07-08)
Supplement: Supplementary file 13 [file 2_soft_value.tex]

\section{Soft Value Aggregation}\label{app:soft_value}
In this section, we provide background on soft value aggregation \citep{fox2016taming, haarnoja17a} and the regularized Bellman optimality operator \citep{neu2017unified, geist2019theory}, which rely on the convex conjugate functions derived in \mysec{conj_examples} and \myapp{conjugates}.  

% Our main object of interest in the rest of the paper will be an alternative decomposition of the Lagrangian %dual 
% Starting from the Lagrangian in \cref{eq:dual_lagrangian},
We give a non-standard derivation of the regularized Bellman optimality operator.   Factorizing $\mu(a,s) = \mu(s) \pi(a|s)$, we can imagine optimizing over $\mu(s)$ and $\pi(a|s) \in \simplex$ separately,
\begin{align}
%   \mathcal{L}:= 
   \max \limits_{\mu(s)\rightarrow \mathcal{M}} \max \limits_{\pi(a|s)} \min \limits_{V(s)}  \, 
     (1-\gamma) \big\langle \nu_0(s), V(s) \big  \rangle
     + &\blangle \mu(a,s), r(a,s) +  \gamma \transitionv -V(s)\brangle - \frac{1}{\beta} \Omega_{\pi_0}(\mu)  \label{eq:dual_lagrangian_app}
\end{align}
%mention a further decomposition the Lagrangian dual in \cref{eq:dual_lagrangian}.
%We mention a further decomposition of the Lagrangian dual to highlight an approach used later in the paper.  
% from \cref{eq:dual_lagrangian}
% Note that both $\mu(s)$ and $V(s)$ have the role of enforcing the Bellman flow constraints.
Eliminating $\mu(s)$ by setting $d/d\mu(s) = 0$, we obtain the regularized Bellman operator 
%\resizebox{\columnwidth}{!}{\parbox{\columnwidth}{
\begin{align}
    V(s)  = \blangle \pi(a|s), \, r(s,a) + \gamma \transitionv \brangle - \frac{1}{\beta} \Omega_{\pi_0}(\pi) \nonumber . % \label{eq:reg_bell}
\end{align}
\normalsize
%}}
% using fact that $V(s)$ is not a function of the action $a$. % $\pi(a|s)$.  
Eliminating $\mu(s)$ thus leads to a constraint on the form of $V(s)$, since both may be viewed as enforcing the Bellman flow constraints.  Plugging this expression back into the Lagrangian \cref{eq:dual_lagrangian_app} and removing the minimization over $V(s)$, we are left with only the initial state term and a maximization over $\pi(a|s) \in \Delta^{|\mathcal{A}|}$.
%, where the policy appears in the above expression for the value function $V(s)$.  

%This translates to a constraint of $V(s)$, so that we can remove minimization over the value function and plug this expression back into the Lagrangian \cref{eq:dual_lagrangian}.   We are left with only the initial state term and a maximization over $\pi(a|s) \in \Delta^{|\mathcal{A}|}$, where the policy appears in the above expression for the value function $V(s)$.  
%However, the above expression for the value function $V(s)$. %in \cref{eq:reg_bell} still depends on the policy, with a maximization over $\pi(a|s) \in \Delta^{|\mathcal{A}|}$.  

Recalling the definition of the optimal state-action value, or $Q$ function, ${Q_*(s,a)= r(s,a) + \gamma \transitionv}$, which is recursively defined in terms of value function estimates $V(s\tick)$, we obtain the following optimization %\gamma \mathbb{E}_{P(s'|s,a)}[V(s')]
% \resizebox{\columnwidth}{!}{\parbox{\columnwidth}{
\begin{align}
\mathcal{R}_{\Omega, \beta}^{*}(r) &= \, \max \limits_{\pi(a|s) \in \Delta^{|\mathcal{A}|}} (1-\gamma) \, \blangle \nu_0(s) , V(s) \brangle  \,\, \text{subj. $ V(s)= \blangle \pi(a|s), r(s,a) + \gamma \transitionv \brangle -  \klomegapi$} \label{eq:bellman_reg} \\
    &=(1-\gamma) \, \mathbb{E}_{\nu_0} \big[\max \limits_{\pi \in \Delta^{|\mathcal{A}|}} \langle \pi(a|s), Q_*(s,a)  \rangle - \klomegapi \big]  \label{eq:soft_bellman}
    % \frac{1}{\beta} \Omega_{\pi_0}(\pi)
\end{align}
% }}
\normalsize
This conveniently involves expectations under $\nu_0(s)$, and leads to `soft' or regularized versions of algorithms such as value iteration (\citet{fox2016taming, haarnoja17a}) and modified policy iteration \citep{geist2019theory}.
% (e.g. \citet{haarnoja17a, geist2019theory}).

Maximizing over $\pi \in \simplex$ in \cref{eq:soft_bellman}, we can recognize the optimal value function $V_*(s) = \alphaconjn$ as the conjugate function, also known as the regularized Bellman optimality operator \citep{geist2019theory}.
We derived closed forms for $V_*(s)$ and the optimal policy $\piopt(a|s)$ in \myapp{conjugates} and \mysec{conj_examples}.  
% Similarly to \mysec{adversarial_perturb}, we can interpret the regularized policy optimization in \cref{eq:soft_bellman} as hedging against an imaginary adversary.  which corresponds to the conjugate function $\frac{1}{\beta}\Omega^{*}_{\pi_0,\beta}(Q)$, as a two player game between an agent and an imagined adversary \citep{ortega2014adversarial}.

\subsection{Soft Value Function by $\alpha$-Divergence}\label{app:alpha_results}
\begin{figure}[h]
\centering
\begin{subfigure}{0.4\columnwidth}\includegraphics[width=.676\textwidth]{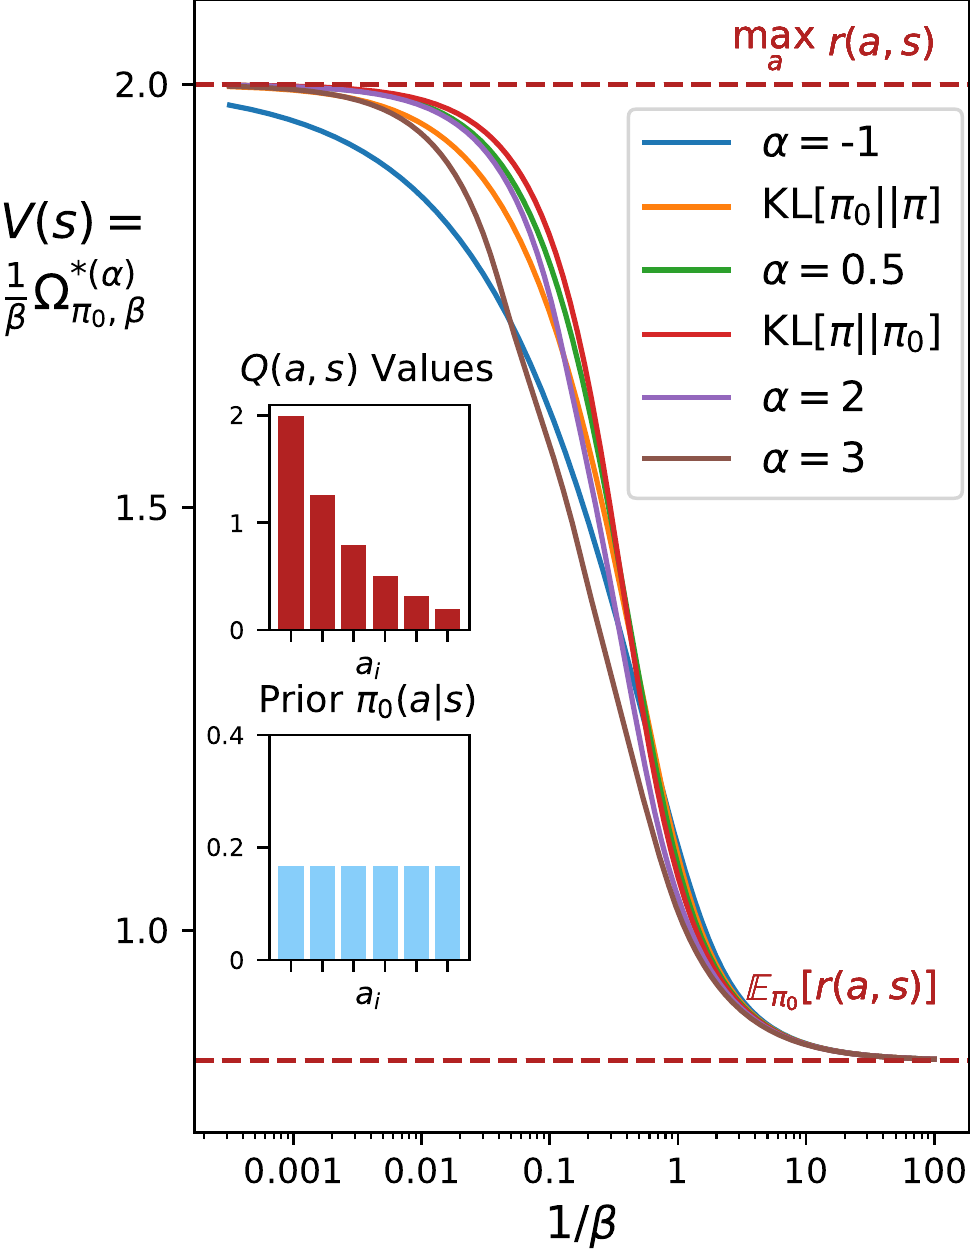}
%\vspace*{.15cm}
\caption{Uniform $\pi_0(a|s)$}\label{fig:value_agga}\end{subfigure}\hspace*{.01\columnwidth}
\begin{subfigure}{0.4\columnwidth} 
% \vspace*{-.12cm}\includegraphics[scale=.3]{figs/conj_by_alpha/value_norm_beta1_vert.pdf}
% \vspace*{-.1cm}\includegraphics[width=.96\textwidth]{figs/conj_by_alpha/value_norm_beta1_vert_thin.pdf}
% \caption{$V(s)$ and $\psi_{\alpha}(s)$ as a function of $\alpha$ for $\beta=1$}\label{fig:value_aggb}\end{subfigure}
\vspace*{-.1cm}\includegraphics[width=.676\textwidth]{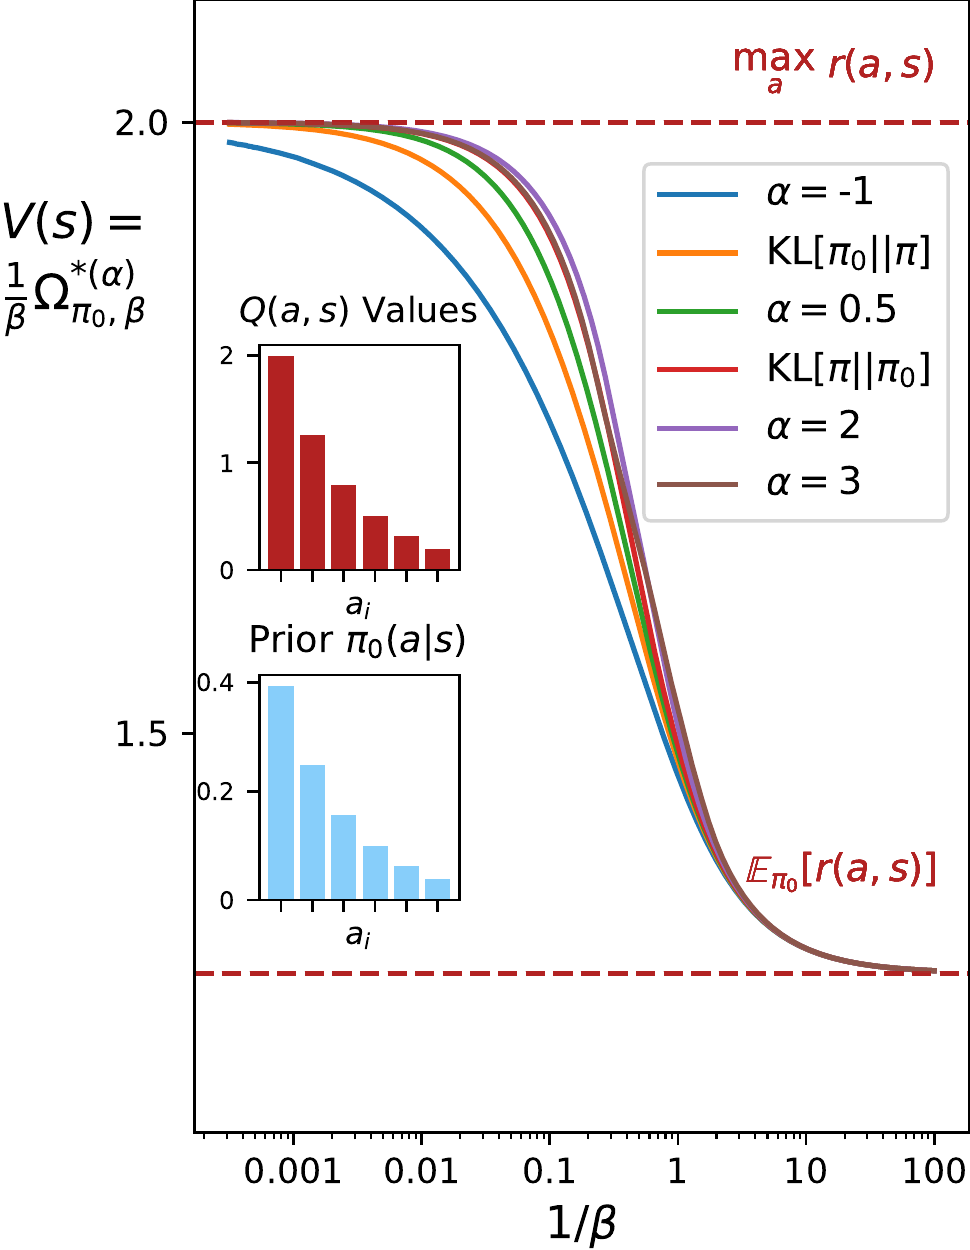}
\caption{$\pi_0(a|s) \propto r(a,s) $}\label{fig:value_agga}
\end{subfigure}
\caption{Value function $V(s) = \alphaconjm(Q)$ as a function of $\beta$ (x-axis) and $\alpha$ (colored lines), using $Q(a,s)$ and $\pi_0(a|s)$ from the left inset.   See \cref{eq:kl_bellman} and \cref{eq:alpha_bellman} for closed forms. }\label{fig:value_agg_main} %and normalization constant $\psi_{\alpha}(s)$
\end{figure}

% \subsection{Value Function and Normalization Constant by $\beta$ and $\alpha$}\label{app:alpha_results}
% \paragraph{Soft Value Aggregation using Various $\alpha$-Divergences}
In \cref{fig:value_agga}, we visualize the optimal value function $V_*(s) = \frac{1}{\beta}\Omega^{*}_{\pi_0,\beta}(Q)$, for \textsc{kl} or $\alpha$-divergence regularization and different choices of regularization strength $1/\beta$.   
The choice of divergence particularly affects the aggregated value for low regularization, although we do not observe a clear pattern with respect to $\alpha$.\footnote{See \citet{belousov2019entropic, lee2018sparse, lee2019tsallis}, or \cref{app:alpha_results} for additional discussion of the effect of $\alpha$-divergence regularization on learned policies.}
In all cases, the value function ranges between $\max_a Q(a,s)$ for an unregularized deterministic policy as $\beta \rightarrow \infty$, and the expectation under the reference policy $\mathbb{E}_{\pi_0}[Q(a,s)]$ for strong regularization as $\beta \rightarrow 0$.   We further discuss this property in \mysec{entropy_vs_div}.

% \paragraph{Value Function $V_*(s)$ and Normalization Constant $\normalizeralpha$ as a function of $\alpha$}
% Recall the expression for the optimal value function $V_*(s) = \alphaconjpi$ from \cref{eq:alpha_conj_norm_main} or \myprop{alpha_conj_app} 
% \begin{align}
%     V_*(s) = \frac{\alpha-1}{\alpha}  \big \langle \pi_0(a|s) \big[  \beta (\alpha-1) \cdot \big(\dualvar(a,s) - \psi_{\alpha}(s;\beta)\big)  \big]_+^{\frac{1}{\alpha-1}}, \, \dualvar(a,s) \big \rangle   +  \frac{1}{\alpha}  \psi_{\alpha}(s;\beta) 
% \end{align}
% where $\piopt(a|s) = pi_0(a|s) \big[  \beta (\alpha-1) \cdot \big(\dualvar(a,s) - \psi_{\alpha}(s;\beta)\big)  \big]_+^{\frac{1}{\alpha-1}}$ is the optimal policy.    

% To understand the relationship between
