# Supplementary material for: Your Policy Regularizer is Secretly an Adversary
Source: arXiv:2203.12592 source file (2022-07-08)
Supplement: Supplementary file 15 [file 4_husain.tex]

\section{Derivations of \citet{husain2021regularized}}\label{app:husain_conjugate}
We rewrite the derivations of \citet{husain2021regularized} where $\Omega \big( \mu(a,s) \big)$ represents a convex regularizer
\begin{align}
    \obj_{\Omega, \beta}(r) = \max \limits_{\mu(a,s)} \obj_{\Omega, \beta}(\mu) &= \max \limits_{\mu(a,s)} \,\,  \langle \mu(a,s), r(a,s) \rangle - \frac{1}{\beta} \Omega \big( \mu(a,s) \big)  \label{eq:reg_rl} \\ 
    \text{subj. to: } \, \, & \int \mu(a,s) \, da = (1-\gamma) \nu_0(s) + \gamma \int p(s|s',a') \, \mu(s',a')  ds \, da \, \, \forall s \in \mathcal{S} \nonumber
\end{align}
   We can let $\Omega$ regularize the full state-action distribution, or the conditional policy $\pi(a|s) = \mu(a,s) / \sum_a \mu(a,s)$), and denote the feasible set for the above constraints as $\mudomain$, so that we can write 
   \begin{align}
        \max \limits_{\mu(a,s) \in \mudomain} \obj_{\Omega, \beta}(\mu) &= \max \limits_{\mu(a,s) \in \mudomain} \,\,  \big\langle \mu(a,s), r(a,s)\rangle - \frac{1}{\beta} \Omega \big( \mu(a,s) \big) := \Omega^{*}\big( r(a,s) \big) \label{eq:reg_rl2} 
   \end{align}
 Note that the objective is \textit{concave}, as the sum of a linear term and the concave $-\Omega$.  Since the conjugate is an involution for convex functions, we can rewrite  $ \obj_{\Omega, \beta}(r) = -(-\obj_{\Omega, \beta}(r)) = - ((-\obj_{\Omega, \beta})^*)^* $, which yields
 \begin{align}
     \obj_{\Omega, \beta}(r) &= \sup \limits_{\mu(a,s) \in \mudomain} - ((-\obj_{\Omega, \beta})^*)^* \nonumber \\
     &\overset{(1)}{=}\sup \limits_{\mu(a,s) \in \mudomain} -\bigg( \sup \limits_{r^\prime(a,s) \in \mathcal{F}} \langle \mu(a,s), r^{\prime}(a,s) \rangle -  (-\obj_{\Omega, \beta})^*(r^{\prime}) \bigg) \nonumber \\[1.25ex]
     %- \big(-\langle \mu(a,s), r(a,s) \rangle + \obj \big) \bigg) \\
     &= \sup \limits_{\mu(a,s) \in \mudomain}   \inf \limits_{r^\prime(a,s) \in \mathcal{F}}  \langle \mu(a,s), -r^{\prime}(a,s) \rangle +  (-\obj_{\Omega, \beta})^*(r^{\prime})  \nonumber \\
      &\overset{(2)}{=}  \sup \limits_{\mu(a,s) \in \mudomain} \inf \limits_{r^\prime(a,s) \in \mathcal{F}}  \langle \mu(a,s), r^{\prime}(a,s) \rangle +  (-\obj_{\Omega, \beta})^*(-r^{\prime})  \nonumber\\
     &\overset{(3)}{=} \sup \limits_{\mu(a,s) \in \mudomain}  \inf \limits_{r^\prime(a,s) \in \mathcal{F}}  \langle \mu(a,s), r^{\prime}(a,s) \rangle +  \bigg( \sup \limits_{\mu^{\prime}} \, \langle \mu^{\prime}(a,s), -r^{\prime}(a,s) \rangle + \obj_{\Omega, \beta}(\mu^{\prime}) \bigg) \nonumber \\
     &\overset{(4)}{=}  \sup \limits_{\mu(a,s) \in \mudomain}  \inf \limits_{r^\prime(a,s) \in \mathcal{F}}  \langle \mu(a,s), r^{\prime}(a,s) \rangle +  \bigg( \sup \limits_{\mu^{\prime}} \, \langle \mu^{\prime}(a,s), -r^{\prime}(a,s) \rangle + \langle \mu^{\prime}(a,s), r(a,s)\rangle - \frac{1}{\beta} \Omega(\mu^{\prime})   \bigg) \nonumber \\
     &=  \sup \limits_{\mu(a,s) \in \mudomain}  \inf \limits_{r^\prime(a,s) \in \mathcal{F}}  \langle \mu(a,s), r^{\prime}(a,s) \rangle + \frac{1}{\beta}  \bigg( \sup \limits_{\mu^{\prime}}  \, \langle \mu^{\prime}(a,s), \beta \cdot \big( r(a,s) - r^{\prime}(a,s) \big)  \rangle -  \Omega(\mu^{\prime})   \bigg) \nonumber \\[1.25ex]
      &\overset{(5)}{=} \sup \limits_{\mu(a,s) \in \mudomain}  \inf \limits_{r^\prime(a,s) \in \mathcal{F}}  \langle \mu(a,s), r^{\prime}(a,s) \rangle +  \frac{1}{\beta} \Omega^{*} \big( \beta \cdot ( r - r^{\prime} ) \big)   \\
      &\overset{(6)}{=}  \inf \limits_{r^\prime(a,s) \in \mathcal{F}}  \sup \limits_{\mu(a,s) \in \mudomain}  \langle \mu(a,s), r^{\prime}(a,s) \rangle +  \frac{1}{\beta}  \Omega^{*} \big( \beta \cdot ( r - r^{\prime} ) \big)  \label{eq:end}
 \end{align}
 where $(1)$ applies the definition of the conjugate of $(-\obj_{\Omega, \beta})^*$, $(2)$ reparameterizes the optimization in terms of $r^{\prime} \rightarrow -r^{\prime}$, $(3)$ is the conjugate for $(-\obj_{\Omega, \beta})$, and $(4)$ uses the definition of the regularized RL objective for measure $\mu^{\prime}(a,s)$ with the reward $r(a,s)$.  Finally, $(5)$ recognizes the inner maximization as the conjugate function for a modified reward and $(6)$ swaps the order of $\inf$ and $\sup$ assuming the problem is feasible.   
 
%  To summarize, we have the following (where the last line follows from conditions of the stationary distribution and form of adversarial rewards (see proof of Lemma 1 on \citet{husain2021regularized} pg. 17).
%       \begin{align}
%      \sup \limits_{\mu(a,s) \in \mudomain} \,  &\big\langle \mu(a,s), r(a,s) - \frac{1}{\beta} \Omega \big( \mu(a,s) \big) \big \rangle \nonumber \\[.5ex]
%      &= \inf \limits_{r^\prime(a,s) \in \mathcal{F}} \sup \limits_{\mu(a,s) \in \mudomain} \,\,  \big\langle \mu(a,s), r^{\prime}(a,s) \big \rangle    + \frac{1}{\beta} \Omega^{*} \bigg( \beta \cdot (r(a,s) - r^{\prime}(a,s)) \bigg) \label{eq:full_rl_conj} 
%      \\[.5ex]
%      &=  \inf \limits_{Q(a,s) \in \mathcal{F}} \, (1-\gamma) \langle \nu_0(s), V(s) \rangle \, + \frac{1}{\beta} \Omega^{*}\bigg( \beta \cdot\big(r(a,s) +  \transitionv - Q(a,s)) \big)      \bigg) %\int P(s'|a,s) V(s') ds'
%  \end{align}

To derive the optimal reward perturbations, consider introducing $V(s)$ to enforce the flow constraints.
\begin{align}
 \obj_{\Omega, \beta}(r)=   \inf \limits_{r^\prime(a,s) \in \mathcal{F}}  \sup \limits_{\mu(a,s)} \inf \limits_{V(s)} \langle \mu(a,s), r^{\prime}(a,s) + \gamma \transitionv - V(s) \rangle +  \frac{1}{\beta}  \Omega^{*} \big( \beta \cdot ( r - r^{\prime} ) \big) + (1-\gamma) \langle \nu_0(s), V(s) \rangle \label{eq:husain_lagr}
\end{align}
Now, eliminating $\mu(a,s)$ yields the condition 
\begin{align}
     r^{\prime}(a,s) + \gamma \transitionv - V(s) = 0 \quad \implies \quad r^{\prime}(a,s) = V(s) - \gamma \transitionv \label{eq:husain_result}
\end{align}
which matches \citet{husain2021regularized}.  
% See \citet{husain2021regularized} for alternative derivations.  
Recognizing that $r^{\prime}(a,s) = r(a,s)- \pr(a,s)$, we can rearrange \cref{eq:husain_result} to obtain $\pr(a,s) = r(a,s) + \gamma \transitionv - V(s)$ which matches the advantage function.

Finally, note that the term involving $\mu(a,s)$ vanishes when substituting the expression for $\mr(a,s)$ in \cref{eq:husain_result} into \cref{eq:husain_lagr}.  This yields Theorem 1 of \citet{husain2021regularized},
\begin{align}
 \obj_{\Omega, \beta}(r)=    \inf \limits_{V(s)}  \, (1-\gamma) \blangle \nu_0(s), V(s) \brangle + \frac{1}{\beta}  \Omega^{*} \big( \beta \cdot ( r(a,s) + \gamma \transitionv - V(s) ) \big)
\end{align}
% \textcolor{red}{Taking $r^{\prime}(a,s) = r(a,s)- \pr(a,s)$, we have $r(a,s)- \pr(a,s) = V(s) - \gamma \transitionv$.} \RB{Other way around}
