# Supplementary material for: Your Policy Regularizer is Secretly an Adversary
Source: arXiv:2203.12592 source file (2022-07-08)
Supplement: Supplementary file 20 [file 9_submission_placeholder.tex]

% \section{Relationship between $V_*(s)$ and $\normalizeralpha$ (Redirect to \myapp{perturb_pf})}
% See \myapp{advantage_pf} and \myapp{advantage_confirm}.

\section{Consistency Implies Optimality}
Consistency equation implies
\begin{align}
    r(a,s) + \gamma \transitionv - V(s) = \frac{1}{\beta} \log_{\alpha}\frac{\piopt(a|s)}{\pi_0(a|s)} + \psi_{\prpi} 
\end{align}
Recall that $\frac{1}{\beta} \nabla_{\mu} \Omega_{\pi_0}(\mu) = \log_{\alpha}\frac{\piopt(a|s)}{\pi_0(a|s)} + \psi_{\prpi}$.
Thus, we can rewrite the consistency condition as 
\begin{align}
    r(a,s) + \gamma \transitionv  = V(s) + \frac{1}{\beta} \nabla_{\mu} \Omega_{\pi_0}(\mu)
\end{align}

This condition is identical to showing that that the maximization in the Bellman optimality operator is tight, 
\begin{align}
    \mathcal{T}V(s) &= \max \limits_{\pi(a|s) \in \Delta^{|\mathcal{A}|}} \blangle \pi(a|s), r(a,s) + \gamma \transitionv \brangle - \omegapi \\
    &= \blangle \piopt(a|s), r(a,s) + \gamma \transitionv \brangle - \omegapiopt
\end{align}
