# Supplementary material for: Your Policy Regularizer is Secretly an Adversary
Source: arXiv:2203.12592 source file (2022-07-08)
Supplement: Supplementary file 22 [file 00_prelim.tex]

\section{Proofs from Preliminaries (\mysec{prelim})}
In this section, we show that a state-action occupancy measure $\mu(a,s)$ which satisfies the Bellman flow constraints in \cref{eq:primal_lp} is normalized as a joint distribution.   
We also provide background on the various conjugate optimizations which appear in the regularized \gls{MDP} setting, which provides context for our conjugate function derivations in \myapp{conjugates} and \myapp{soft_value}.   In particular, we compare the dual optimization in \cref{eq:dual_reg} with the regularized Bellman optimality operator \citep{geist2019theory}, which underlies common iterative algorithms.
% \citep{geist2019theory}, which we also discuss in \myapp{} and \myapp{}.

\subsection{Bellman Flow Constraints Imply Normalized $\mu(a,s)$}\label{app:normalized_mu}
Assuming that the initial state $\nu_0(s)$ and transition $P(s\tick|a,s)$ distributions are normalized ($\sum_s \nu_0(s) = 1$ and $\sum_{s} P(s|a\tick,s\tick) = 1$   $\forall s \in \mathcal{S}$), we would like to show that any $\mu(a,s) \in \mathcal{M}$ which satisfies the Bellman flow constraints is normalized as a joint distribution, $\mu(a,s) \in \Delta^{|\mathcal{A}| \times |\mathcal{S}|}$.
% We briefly show that a state-action occupancy measure which satisfies the Bellman flow constraints is normalized as a joint distribution, assuming that the initial state $\nu_0(s)$ and transition $P(s\tick|a,s)$ distributions are normalized.   More formally, if $\sum_s \nu_0(s) = 1$ and $\sum_{s\tick} P(s\tick|a,s) = 1$  $\forall a \in \mathcal{A},s \in \mathcal{S}$, then $\mu(a,s) \in \mathcal{M} \implies \mu(a,s) \in \Delta^{|\mathcal{A}| \times |\mathcal{S}|}$.
Starting from the Bellman flow constraints $ \sum_{a} \mu(a,s) = (1-\gamma) \nu_0(s) + \gamma \sum_{a\tick,s\tick} P(s|a\tick,s\tick) \mu(a\tick, s\tick)$,
% \begin{align}
%     \sum \limits_{a} \mu(a,s) = (1-\gamma) \nu_0(s) + \gamma \sum \limits_{a\tick,s\tick} P(s|a\tick,s\tick) \mu(a\tick, s\tick)
% \end{align}
we consider taking the summation over states $s \in \mathcal{S}$,
% \small
% \begin{align}
%       \sum \limits_{a, s} \mu(a,s) &= (1-\gamma) \sum \limits_{s} \nu_0(s) + \gamma \sum \limits_{s} \sum \limits_{a\tick,s\tick} P(s|a\tick,s\tick) \mu(a\tick, s\tick) \\
%       \sum \limits_{a, s} \mu(a,s) &\overset{(1)}{=} (1-\gamma) \cdot 1 + \gamma \sum \limits_{s} P(s|a\tick,s\tick) \sum \limits_{a\tick,s\tick}  \mu(a\tick, s\tick) \\
%         \sum \limits_{a, s} \mu(a,s) &\overset{(2)}{=} (1-\gamma) \cdot 1 + \gamma \sum \limits_{a\tick,s\tick}  \mu(a\tick, s\tick) 
% \end{align}
% \normalsize
\scriptsize
\begin{align}
       \sum \limits_{a, s} \mu(a,s) &= (1-\gamma) \sum \limits_{s} \nu_0(s) + \gamma \sum \limits_{s} \sum \limits_{a\tick,s\tick} P(s|a\tick,s\tick) \mu(a\tick, s\tick) \overset{(1)}{=} (1-\gamma) + \gamma \sum \limits_{s} P(s|a\tick,s\tick) \sum \limits_{a\tick,s\tick}  \mu(a\tick, s\tick) \overset{(2)}{=} (1-\gamma) + \gamma \sum \limits_{a\tick,s\tick}  \mu(a\tick, s\tick) \nonumber
\end{align}
\normalsize
where $(1)$ uses the normalization assumption on $\nu_0(s)$ and the distributive law, and $(2)$ uses the normalization assumption on $P(s|a\tick,s\tick)$.  Finally, we rearrange to obtain
\small
\begin{align}
  (1-\gamma)  \sum \limits_{a, s} \mu(a,s)  = (1-\gamma) \qquad \implies \qquad \sum \limits_{a, s} \mu(a,s) = 1
\end{align}
\normalsize
which shows that $\mu(a,s)$ is normalized as a joint distribution over $a \in \mathcal{A},s \in \mathcal{S}$, as desired.

% ($\mu(a,s) \in \mathcal{M}$) is normalized as a joint distribution over states and actions ($\mu(a,s) \in \Delta^{|\mathcal{A}| \times |\mathcal{S}|}$).   a normalized initial state distribution $\nu_0(\vz)$

\subsection{Optimal Policy in a Regularized MDP}\label{app:optimal_policy}
% In \cref{eq:dual_lagrangian}, we have eliminated $\mu(a,s)$ to move from the 
In \mysec{mdp_regularized}, we moved from the regularized primal optimization (\cref{eq:primal_reg}) to the dual optimization (\cref{eq:dual_reg}) via the regularized Lagrangian
\small
\begin{align}
  \min \limits_{V(s), \lambdaplus} \max \limits_{\mu(a,s)}  \, 
     (1-\gamma) \big\langle \nu_0(s), V(s) \big  \rangle + \langle \mu(a,s), r(a,s) + \gamma \transitionv -V(s) + \lambdaplus \rangle - \frac{1}{\beta} \Omega_{\pi_0}(\mu) 
\end{align}
\normalsize
where we recognized the final two terms as a conjugate optimization
\small
\begin{align}
   \hspace*{-.25cm} \frac{1}{\beta} \Omega^*_{\pi_0,\beta}\Big( r(a,s) + \gamma \transitionv -V(s) + \lambdaplus \Big) = \max \limits_{\mu(a,s)} \blangle \mu(a,s), r(a,s) + \gamma \transitionv -V(s) + \lambdaplus \brangle - \frac{1}{\beta} \Omega_{\pi_0}(\mu) \label{eq:conj_opt_mdp}
\end{align}
\normalsize
% , we have eliminated the optimization over $\mu(a,s)$ by writing the conjugate function $\frac{1}{\beta} \Omega^{*}_{\pi_0, \beta}$
to yield a dual optimization over $V(s)$ and $\lambdaplus$ only in \cref{eq:dual_reg}.   After solving the dual optimization for $V_*(s)$, $\lambda_*(a,s)$, we can recover the optimal policy in the \textsc{mdp} using the optimizing argument of \cref{eq:conj_opt_mdp}.

We have not explicitly written the form of the optimizing argument $\mu(a,s)$ in the main text until \cref{eq:optimal_policy}, but we will see that this expression arises from our convex conjugate derivations for $\pr(a,s)$ in \cref{table:conj_table} and \myapp{conjugates}.   Note that we optimize over $\mu(a,s)$ and do not enforce normalization explicitly, since the optimal $V_*(s)$ will enforce this constraint by the reasoning above (\myapp{normalized_mu}). 
For $\alpha$-divergence regularization of the policy (to reference $\pi_0$) or state-action occupancy (to reference $\mu_0$), we can write
\small
\begin{align}
  \hspace*{-.2cm}  \mu(a,s) &= \mu(s) \pi_0(a|s) \exp_{\alpha} \left\{r(a,s) + \gamma \transitionvstar - V_*(s) + \lambdaplus - \psi(s;\beta) \right\}  \,\, \qquad (\text{Policy Reg., \myapp{conj3} \cref{eq:opt_pi_alpha}}) \nonumber \\
  \hspace*{-.2cm}    \mu(a,s) &= \mu_0(a,s) \exp_{\alpha} \left\{r(a,s) + \gamma \transitionvstar - V_*(s) + \lambdaplus \right\} \hfill \qquad \qquad \qquad (\text{Occupancy Reg., \myapp{conj4} \cref{eq:opt_mu_alpha}}) \nonumber
\end{align}
\normalsize
where $\psi(s;\beta)$ is identical to $\psi_{\pr}(s;\beta)$ (see \myapp{conj3}).   

We derive these expressions in \cref{table:conj_table} and \myapp{conjugates} using $\pr(a,s)$ as the argument of the conjugate function.  Our result in \cref{prop:advantage} (proof in \myapp{advantage_pf}) links these two results at optimality, with
\begin{align}
\pr_{*}(a,s) = \underbrace{r(a,s) + \gamma \transitionv}_{Q_*(a,s)} -V_*(s) + \lambdaplus \label{eq:expression_for_advantage_app}
\end{align}

% See \citet{lee2019tsallis} for full proofs regarding optimality.

\subsection{Soft Value Aggregation}\label{app:sv_background}
Soft value aggregation \citep{fox2016taming, haarnoja17a} and the regularized Bellman optimality operator \citep{neu2017unified, geist2019theory} also rely on the convex conjugate function, but with a slightly different setting than our derivations for the optimal regularized policy or reward perturbations.  In particular, the optimization is over the policy in each state $\pi(a|s) \in \Delta^{|\mathcal{A}|}$ with an explicit normalization constraint (\cref{eq:soft_value_app}).

% In this section, we provide background on 
% derived in \mytab{conj_table} and \myapp{conjugates}.  
We derive the regularized Bellman optimality operator from the primal objective in \cref{eq:primal_reg}.   Factorizing $\mu(a,s) = \mu(s) \pi(a|s)$, we can imagine optimizing over $\mu(s)$ and $\pi(a|s) \in \simplex$ separately,
\begin{align}
%   \mathcal{L}:= 
   \max \limits_{\mu(s)\rightarrow \mathcal{M}} \max \limits_{\pi(a|s)} \min \limits_{V(s)}  \, 
     (1-\gamma) \big\langle \nu_0(s), V(s) \big  \rangle
     + &\blangle \mu(a,s), r(a,s) +  \gamma \transitionv -V(s)\brangle - \frac{1}{\beta} \Omega_{\pi_0}(\mu) . \label{eq:dual_lagrangian_app}
\end{align}
%mention a further decomposition the Lagrangian dual in \cref{eq:dual_lagrangian}.
%We mention a further decomposition of the Lagrangian dual to highlight an approach used later in the paper.  
% from \cref{eq:dual_lagrangian}
% Note that both $\mu(s)$ and $V(s)$ have the role of enforcing the Bellman flow constraints.
Eliminating $\mu(s)$ (by setting $d/d\mu(s) = 0$) leads to a constraint on the form of $V(s)$, since both may be viewed as enforcing the Bellman flow constraints.  
% Eliminating $\mu(s)$ by setting $d/d\mu(s) = 0$, we obtain a condition on $V(s)$.   This is ince 
% obtain the regularized Bellman operator 
%\resizebox{\columnwidth}{!}{\parbox{\columnwidth}{
\begin{align}
    V(s)  &= \blangle \pi(a|s), \, r(s,a) + \gamma \transitionv \brangle - \frac{1}{\beta} \Omega_{\pi_0}(\pi) \label{eq:bellman_opt} . % \label{eq:reg_bell}
\end{align}
\normalsize
We define $Q(s,a) \coloneqq r(s,a) + \gamma \transitionv$ and write $V(s) = \langle \pi(a|s), \, Q(a,s) \rangle - \frac{1}{\beta} \Omega_{\pi_0}(\pi)$ moving forward.

As an operator for iteratively updating $V(s)$, \cref{eq:bellman_opt} corresponds to the regularized Bellman operator $\mathcal{T}_{\Omega_{\pi_0}, \beta}$ and may be used to perform policy evaluation for a given $\pi(a|s)$ \citep{geist2019theory}.    
The regularized Bellman \textit{optimality} operator $\mathcal{T}^*_{\Omega_{\pi_0}, \beta}$, which can be used for value iteration or modified policy iteration \citep{geist2019theory}, arises from including the maximization over $\pi(a|s) \in \simplex$ in \cref{eq:dual_lagrangian_app}
\begin{align}
   V(s)  \leftarrow \frac{1}{\beta} \Omega^{*}_{\pi_0,\beta}(Q) = \max \limits_{\pi \in \Delta^{|\mathcal{A}|}} \blangle \pi(a|s), Q(a,s) \brangle - \frac{1}{\beta} \Omega_{\pi_0}(\pi) \, . \label{eq:soft_value_app} 
\end{align}  
This has the form of a conjugate optimization $\frac{1}{\beta} \Omega^{*}_{\pi_0,\beta}(Q)$ \citep{geist2019theory}, albeit with a normalization constraint which can be enforced using a Lagrange multiplier $\psi_Q(s;\beta)$. 

Also note that the argument of the conjugate function \textit{does not} include the value function $V(s)$ compared with the optimization for the optimal policy in \cref{eq:conj_opt_mdp}.   We will highlight relationship between the normalization constants $\psi_Q(s;\beta)$, $\psi_{\pr}(s;\beta)$, and $V_*(s)$ in \myapp{advantage_confirm}, where $V_*(s) = \psi_Q(s;\beta) + \psi_{\pr}(s;\beta)$ as in \citet{lee2019tsallis}.

See \myapp{soft_value} for detailed discussion of soft value aggregation along with conjugate derivations for $\frac{1}{\beta} \Omega^{*}_{\pi_0,\beta}(Q)$ (\ref{table:table_refs_q}).   
% We also highlight a relationship between the normalization constants $\psi_Q(s;\beta)$, $\psi_{\pr}(s;\beta)$, and $V_*(s)$ in \myapp{advantage_confirm}, where $V_*(s) = \psi_Q(s;\beta)- \psi_{\pr}(s;\beta)$.

% \paragraph{Normalization Constraints in Conjugate Optimization}
% Note that the conjugate optimization in \cref{eq:soft_value_app} involves a normalization constraint for each $\pi(a|s)$, which we can enforce using a Lagrange multiplier $\psi_Q(s;\beta)$.   We derive expressions for the conjugate function with normalization constraint for the \textsc{kl} divergence in \myapp{kl_norm_conj} and $\alpha$-divergence in \myapp{alpha_norm_conj}.

% By contrast, when reasoning about the reward perturbations $\pr$ and the conjugate function $\frac{1}{\beta} \Omega^{*}_{\pi_0,\beta}(\pr)$, we will optimize over $\mu(a,s)$ jointly and do not include an explicit normalization constraint (see \cref{eq:conj_app} below).   

% In the following sections, we use the convention that the conjugate $\frac{1}{\beta} \Omega^{*}_{\pi_0,\beta}(Q)$ involves optimization over normalized $\pi(a|s) \in \simplex$ as in \cref{eq:soft_value_app}, while $\frac{1}{\beta} \Omega^{*}_{\pi_0,\beta}(\pr)$ optimizes over $\mu(a,s)$ without normalization.    We comment on the relationship between these two formulations in \myapp{advantage_confirm}.

% % For defining the conjugate $\frac{1}{\beta} \Omega^{*}_{\pi_0,\beta}(\pr)$, we instead in contrast to our conjugate optimization over $\mu(a,s)$ without normalization 
