# Supplementary material for: Your Policy Regularizer is Secretly an Adversary
Source: arXiv:2203.12592 source file (2022-07-08)
Supplement: Supplementary file 24 [file 02_optimal_primal.tex]

\section{Proofs from Preliminaries (\mysec{prelim})}
In this section, we show that a state-action occupancy measure $\mu(a,s$ which satisfies the Bellman flow constraints in \cref{eq:primal_lp} is normalized as a joint distribution, and provide background on soft value aggregation and the regularized Bellman optimality operator \citep{geist2019theory}.
% \citep{geist2019theory}, which we also discuss in \myapp{} and \myapp{}.

\subsection{Bellman Flow Constraints Imply Normalized $\mu(a,s)$}\label{app:normalized_mu}
Assuming that the initial state $\nu_0(s)$ and transition $P(s\tick|a,s)$ distributions are normalized ($\sum_s \nu_0(s) = 1$ and $\sum_{s} P(s|a\tick,s\tick) = 1$   $\forall s \in \mathcal{S}$), we would like to show that any $\mu(a,s) \in \mathcal{M}$ which satisfies the Bellman flow constraints is normalized as a joint distribution, $\mu(a,s) \in \Delta^{|\mathcal{A}| \times |\mathcal{S}|}$.
% We briefly show that a state-action occupancy measure which satisfies the Bellman flow constraints is normalized as a joint distribution, assuming that the initial state $\nu_0(s)$ and transition $P(s\tick|a,s)$ distributions are normalized.   More formally, if $\sum_s \nu_0(s) = 1$ and $\sum_{s\tick} P(s\tick|a,s) = 1$  $\forall a \in \mathcal{A},s \in \mathcal{S}$, then $\mu(a,s) \in \mathcal{M} \implies \mu(a,s) \in \Delta^{|\mathcal{A}| \times |\mathcal{S}|}$.
Starting from the Bellman flow constraints $ \sum_{a} \mu(a,s) = (1-\gamma) \nu_0(s) + \gamma \sum_{a\tick,s\tick} P(s|a\tick,s\tick) \mu(a\tick, s\tick)$,
% \begin{align}
%     \sum \limits_{a} \mu(a,s) = (1-\gamma) \nu_0(s) + \gamma \sum \limits_{a\tick,s\tick} P(s|a\tick,s\tick) \mu(a\tick, s\tick)
% \end{align}
we consider taking the summation over states $s \in \mathcal{S}$,
\begin{align}
       \sum \limits_{a, s} \mu(a,s) &= (1-\gamma) \sum \limits_{s} \nu_0(s) + \gamma \sum \limits_{s} \sum \limits_{a\tick,s\tick} P(s|a\tick,s\tick) \mu(a\tick, s\tick) \\
       \sum \limits_{a, s} \mu(a,s) &\overset{(1)}{=} (1-\gamma) \cdot 1 + \gamma \sum \limits_{s} P(s|a\tick,s\tick) \sum \limits_{a\tick,s\tick}  \mu(a\tick, s\tick) \\
        \sum \limits_{a, s} \mu(a,s) &\overset{(2)}{=} (1-\gamma) \cdot 1 + \gamma \sum \limits_{a\tick,s\tick}  \mu(a\tick, s\tick) 
\end{align}
where $(1)$ uses the normalization assumption on $\nu_0(s)$ and the distributive law, and $(2)$ uses the normalization assumption on $P(s|a\tick,s\tick)$.  Finally, we rearrange to obtain
\begin{align}
  (1-\gamma)  \sum \limits_{a, s} \mu(a,s)  = (1-\gamma) \qquad \implies \qquad \sum \limits_{a, s} \mu(a,s) = 1
\end{align}
which shows that $\mu(a,s)$ is normalized as a joint distribution over $a \in \mathcal{A},s \in \mathcal{S}$, as desired.

\subsection{Optimal Policy in a Regularized \gls{MDP}}\label{app:optimal_policy}

% ($\mu(a,s) \in \mathcal{M}$) is normalized as a joint distribution over states and actions ($\mu(a,s) \in \Delta^{|\mathcal{A}| \times |\mathcal{S}|}$).   a normalized initial state distribution $\nu_0(\vz)$

\subsection{Soft Value Aggregation}\label{app:sv_background}
In this section, we provide background on soft value aggregation \citep{fox2016taming, haarnoja17a} and the regularized Bellman optimality operator \citep{neu2017unified, geist2019theory}, which rely on the convex conjugate function. 
% derived in \mytab{conj_table} and \myapp{conjugates}.  
We derive the regularized Bellman optimality operator from the primal objective in \cref{eq:primal_reg}.   Factorizing $\mu(a,s) = \mu(s) \pi(a|s)$, we can imagine optimizing over $\mu(s)$ and $\pi(a|s) \in \simplex$ separately,
\begin{align}
%   \mathcal{L}:= 
   \max \limits_{\mu(s)\rightarrow \mathcal{M}} \max \limits_{\pi(a|s)} \min \limits_{V(s)}  \, 
     (1-\gamma) \big\langle \nu_0(s), V(s) \big  \rangle
     + &\blangle \mu(a,s), r(a,s) +  \gamma \transitionv -V(s)\brangle - \frac{1}{\beta} \Omega_{\pi_0}(\mu)  \label{eq:dual_lagrangian_app}
\end{align}
%mention a further decomposition the Lagrangian dual in \cref{eq:dual_lagrangian}.
%We mention a further decomposition of the Lagrangian dual to highlight an approach used later in the paper.  
% from \cref{eq:dual_lagrangian}
% Note that both $\mu(s)$ and $V(s)$ have the role of enforcing the Bellman flow constraints.
Eliminating $\mu(s)$ (by setting $d/d\mu(s) = 0$) leads to a constraint on the form of $V(s)$, since both may be viewed as enforcing the Bellman flow constraints.  
% Eliminating $\mu(s)$ by setting $d/d\mu(s) = 0$, we obtain a condition on $V(s)$.   This is ince 
% obtain the regularized Bellman operator 
%\resizebox{\columnwidth}{!}{\parbox{\columnwidth}{
\begin{align}
    V(s)  &= \blangle \pi(a|s), \, r(s,a) + \gamma \transitionv \brangle - \frac{1}{\beta} \Omega_{\pi_0}(\pi) = \blangle \pi(a|s), \, Q(s,a)  \brangle - \frac{1}{\beta} \Omega_{\pi_0}(\pi) \label{eq:bellman_opt} . % \label{eq:reg_bell}
\end{align}
\normalsize
where we define $Q(s,a) \coloneqq r(s,a) + \gamma \transitionv$.
As an operator for iteratively updating $V(s)$, \cref{eq:bellman_opt} corresponds to the regularized Bellman operator $\mathcal{T}_{\Omega_{\pi_0}, \beta}$ and may be used to perform policy evaluation for a given $\pi(a|s)$ \citep{geist2019theory}.    
The regularized Bellman \textit{optimality} operator $\mathcal{T}^*_{\Omega_{\pi_0}, \beta}$, which can be used for value iteration or modified policy iteration \citep{geist2019theory}, arises from including the maximization over $\pi(a|s) \in \simplex$ in \cref{eq:dual_lagrangian_app}
\begin{align}
   V(s)  \leftarrow \frac{1}{\beta} \Omega^{*}_{\pi_0,\beta}(Q) = \max \limits_{\pi \in \Delta^{|\mathcal{A}|}} \blangle \pi(a|s), Q(a,s) \brangle - \frac{1}{\beta} \Omega_{\pi_0}(\pi) \, . \label{eq:soft_value_app} 
\end{align}
\paragraph{Normalization Constraints in Conjugate Optimization}
Note that the conjugate optimization in \cref{eq:soft_value_app} involves a normalization constraint for each $\pi(a|s)$, which we can enforce using a Lagrange multiplier $\psi_Q(s;\beta)$.   We derive expressions for the conjugate function with normalization constraint for the \textsc{kl} divergence in \myapp{kl_norm_conj} and $\alpha$-divergence in \myapp{alpha_norm_conj}.

By contrast, when reasoning about the reward perturbations $\pr$ and the conjugate function $\frac{1}{\beta} \Omega^{*}_{\pi_0,\beta}(\pr)$, we will optimize over $\mu(a,s)$ jointly and do not include an explicit normalization constraint (see \cref{eq:conj_app} below).   

In the following sections, we use the convention that the conjugate $\frac{1}{\beta} \Omega^{*}_{\pi_0,\beta}(Q)$ involves optimization over normalized $\pi(a|s) \in \simplex$ as in \cref{eq:soft_value_app}, while $\frac{1}{\beta} \Omega^{*}_{\pi_0,\beta}(\pr)$ optimizes over $\mu(a,s)$ without normalization.    We comment on the relationship between these two formulations in \myapp{advantage_confirm}.

% For defining the conjugate $\frac{1}{\beta} \Omega^{*}_{\pi_0,\beta}(\pr)$, we instead in contrast to our conjugate optimization over $\mu(a,s)$ without normalization 

\subsection{Soft Value Aggregation with KL Divergence}

\subsection{Soft Value Aggregation with $\alpha$-Divergence}

\subsection{Confirming the Relationship between Normalization and Value Function}
